# Supplementary material for: Demand Modeling, Forecasting, and Counterfactuals, Part I
Source: arXiv:1401.7359 ancillary file (2015-01-14)
Supplement: Supplementary file 1 [file new-market-shares.pdf]

# Supplementary Data to Demand Modeling, Forecasting, and Counterfactuals, Part I

Parag A. Pathak and Peng Shi*

First draft: January 2014
This draft: December 2014

## Contents

**D Detailed Market Shares** **1**
D.1 Back Testing . . . 1
D.1.1 K2 . . . 1
D.1.2 K1 . . . 27
D.2 Predictions for 2014 . . . 51
D.2.1 K2 . . . 51
D.2.2 K1 . . . 72

## D Detailed Market Shares

This is an appendix to the article "Demand Modeling, Forecasting, and Counterfactuals, Part I," available at `http://arxiv.org/abs/1401.7359`. This appendix contains detailed estimates of school market shares using the Naive, Logit, and Mixed Logit models. It contains both backtesting and future predictions. We show both the mean forecasts and the 95% confidence intervals.

### D.1 Back Testing

This section compares predictions of models calibrated using 2012 data with the actual outcomes in 2013.

#### D.1.1 K2

Table 1: Top Choice Market Share Predictions for 2013 K2

| | | Naive | | Logit | | Mixed Logit | | |
|---|---|---|---|---|---|---|---|---|
| Neighborhood | School | mean | (95% C.I.) | mean | (95% C.I.) | mean | (95% C.I.) | Actual |
| Allston-Brighton | Baldwin | 0.15 | (0.11,0.19) | 0.20 | (0.15,0.24) | 0.19 | (0.14,0.24) | 0.16 |
| Allston-Brighton | Blackstone | 0.01 | (0.00,0.03) | 0.01 | (0.00,0.02) | 0.01 | (0.00,0.02) | |
| Allston-Brighton | Bradley | 0.01 | (0.00,0.02) | | | 0.00 | (0.00,0.01) | |
| Allston-Brighton | East Boston EEC | | | 0.00 | (0.00,0.01) | 0.01 | (0.00,0.02) | |

Continued on next page

*Pathak: Massachusetts Institute of Technology and NBER, Department of Economics, email: ppathak@mit.edu and Shi: Massachusetts Institute of Technology, Operations Research Center, email: pengshi@mit.edu.

**Table 1 – continued from previous page**

| Neighborhood | School | Naive mean | Naive (95% C.I.) | Logit mean | Logit (95% C.I.) | Mixed Logit mean | Mixed Logit (95% C.I.) | Actual |
|---|---|---|---|---|---|---|---|---|
| Allston-Brighton | Edison | 0.06 | (0.04,0.08) | 0.09 | (0.06,0.13) | 0.08 | (0.05,0.12) | 0.15 |
| Allston-Brighton | Eliot | 0.01 | (0.00,0.01) | 0.02 | (0.00,0.04) | 0.01 | (0.00,0.03) | 0.01 |
| Allston-Brighton | Gardner | 0.09 | (0.06,0.11) | 0.16 | (0.12,0.21) | 0.17 | (0.12,0.21) | 0.22 |
| Allston-Brighton | Guild | | | | | 0.00 | (0.00,0.01) | |
| Allston-Brighton | Harvard/Kent | 0.01 | (0.00,0.02) | 0.01 | (0.00,0.02) | 0.01 | (0.00,0.02) | |
| Allston-Brighton | Hernandez | | | 0.01 | (0.00,0.02) | 0.01 | (0.00,0.02) | |
| Allston-Brighton | Hurley | 0.06 | (0.03,0.10) | 0.01 | (0.00,0.03) | 0.01 | (0.00,0.02) | |
| Allston-Brighton | Jackson/Mann | 0.12 | (0.10,0.15) | 0.15 | (0.11,0.20) | 0.13 | (0.09,0.17) | 0.15 |
| Allston-Brighton | Kennedy Patrick | | | 0.00 | (0.00,0.01) | 0.00 | (0.00,0.01) | |
| Allston-Brighton | Kenny | 0.01 | (0.00,0.02) | | | | | |
| Allston-Brighton | Kilmer | 0.01 | (0.00,0.02) | | | | | |
| Allston-Brighton | Lyon K-8 | 0.20 | (0.14,0.28) | 0.11 | (0.06,0.17) | 0.15 | (0.09,0.21) | 0.11 |
| Allston-Brighton | Mario Umana | | | | | 0.00 | (0.00,0.01) | |
| Allston-Brighton | Mason | | | 0.00 | (0.00,0.01) | 0.00 | (0.00,0.01) | |
| Allston-Brighton | McKay | | | 0.00 | (0.00,0.01) | 0.00 | (0.00,0.01) | |
| Allston-Brighton | O'Donnell | | | 0.00 | (0.00,0.01) | 0.00 | (0.00,0.01) | |
| Allston-Brighton | Orchard Gardens | | | 0.01 | (0.00,0.02) | 0.01 | (0.00,0.02) | |
| Allston-Brighton | Otis | 0.05 | (0.02,0.09) | | | 0.00 | (0.00,0.01) | |
| Allston-Brighton | Perkins | 0.01 | (0.00,0.02) | | | | | |
| Allston-Brighton | Quincy | 0.06 | (0.03,0.10) | 0.02 | (0.00,0.04) | 0.02 | (0.00,0.04) | 0.05 |
| Allston-Brighton | Roosevelt | 0.01 | (0.00,0.02) | | | | | |
| Allston-Brighton | Tobin | | | 0.01 | (0.00,0.02) | 0.01 | (0.00,0.02) | |
| Allston-Brighton | Warren/Prescott | | | 0.01 | (0.00,0.02) | 0.01 | (0.00,0.03) | |
| Allston-Brighton | Winship | 0.11 | (0.08,0.14) | 0.17 | (0.13,0.22) | 0.16 | (0.11,0.20) | 0.11 |
| Allston-Brighton | Winthrop | 0.01 | (0.01,0.02) | 0.00 | (0.00,0.01) | 0.00 | (0.00,0.01) | |
| Charlestown | Adams | | | 0.00 | (0.00,0.01) | 0.00 | (0.00,0.01) | |
| Charlestown | Baldwin | 0.02 | (0.01,0.02) | 0.01 | (0.00,0.03) | 0.02 | (0.00,0.04) | |
| Charlestown | Blackstone | 0.01 | (0.00,0.02) | 0.02 | (0.00,0.04) | 0.02 | (0.00,0.04) | |
| Charlestown | Bradley | | | 0.01 | (0.00,0.02) | 0.00 | (0.00,0.02) | |
| Charlestown | East Boston EEC | | | 0.02 | (0.00,0.04) | 0.02 | (0.00,0.04) | |
| Charlestown | Edison | | | 0.01 | (0.00,0.02) | 0.01 | (0.00,0.02) | |
| Charlestown | Eliot | 0.01 | (0.00,0.02) | 0.19 | (0.12,0.27) | 0.16 | (0.11,0.23) | 0.12 |
| Charlestown | Gardner | | | 0.02 | (0.00,0.04) | 0.02 | (0.00,0.04) | |
| Charlestown | Guild | | | 0.01 | (0.00,0.02) | 0.00 | (0.00,0.01) | |
| Charlestown | Harvard/Kent | 0.38 | (0.32,0.46) | 0.21 | (0.15,0.27) | 0.21 | (0.15,0.28) | 0.24 |
| Charlestown | Hernandez | | | 0.01 | (0.00,0.03) | 0.01 | (0.00,0.03) | |
| Charlestown | Hurley | 0.07 | (0.04,0.10) | 0.03 | (0.01,0.06) | 0.03 | (0.01,0.05) | 0.04 |
| Charlestown | Jackson/Mann | | | 0.01 | (0.00,0.03) | 0.01 | (0.00,0.02) | |
| Charlestown | Kennedy Patrick | | | 0.01 | (0.00,0.04) | 0.01 | (0.00,0.03) | |
| Charlestown | Lyon K-8 | | | 0.01 | (0.00,0.03) | 0.01 | (0.00,0.03) | |
| Charlestown | Mario Umana | | | 0.01 | (0.00,0.03) | 0.01 | (0.00,0.03) | |
| Charlestown | Mason | 0.01 | (0.00,0.04) | 0.01 | (0.00,0.02) | 0.01 | (0.00,0.02) | |
| Charlestown | Mather | 0.01 | (0.00,0.02) | | | | | |
| Charlestown | McKay | | | 0.01 | (0.00,0.03) | 0.01 | (0.00,0.03) | |
| Charlestown | O'Donnell | | | 0.02 | (0.00,0.04) | 0.01 | (0.00,0.04) | |
| Charlestown | Orchard Gardens | | | 0.01 | (0.00,0.03) | 0.01 | (0.00,0.03) | 0.02 |
| Charlestown | Otis | 0.02 | (0.00,0.05) | 0.01 | (0.00,0.03) | 0.01 | (0.00,0.02) | |
| Charlestown | Quincy | 0.01 | (0.00,0.02) | 0.04 | (0.01,0.08) | 0.04 | (0.01,0.07) | 0.04 |
| Charlestown | Tobin | | | 0.01 | (0.00,0.02) | 0.01 | (0.00,0.02) | |
| Charlestown | Warren/Prescott | 0.43 | (0.34,0.51) | 0.31 | (0.24,0.39) | 0.37 | (0.29,0.45) | 0.49 |
| Charlestown | Winship | 0.01 | (0.00,0.01) | 0.01 | (0.00,0.03) | 0.01 | (0.00,0.02) | |
| Charlestown | Winthrop | | | 0.00 | (0.00,0.01) | 0.00 | (0.00,0.01) | |
| Downtown | Baldwin | 0.01 | (0.00,0.02) | 0.03 | (0.01,0.06) | 0.03 | (0.00,0.06) | 0.01 |
| Downtown | Blackstone | 0.03 | (0.01,0.05) | 0.03 | (0.01,0.06) | 0.04 | (0.01,0.07) | |
| Downtown | Bradley | | | 0.00 | (0.00,0.01) | 0.00 | (0.00,0.01) | |

Continued on next page

**Table 1 – continued from previous page**

| Neighborhood | School | Naive mean | Naive (95% C.I.) | Logit mean | Logit (95% C.I.) | Mixed Logit mean | Mixed Logit (95% C.I.) | Actual |
|---|---|---|---|---|---|---|---|---|
| Downtown | Condon | | | 0.01 | (0.00,0.03) | 0.01 | (0.00,0.04) | |
| Downtown | East Boston EEC | | | 0.00 | (0.00,0.02) | 0.01 | (0.00,0.03) | |
| Downtown | Edison | 0.01 | (0.00,0.02) | 0.01 | (0.00,0.03) | 0.01 | (0.00,0.03) | 0.02 |
| Downtown | Eliot | 0.26 | (0.20,0.33) | 0.26 | (0.20,0.33) | 0.26 | (0.20,0.33) | 0.36 |
| Downtown | Gardner | 0.01 | (0.00,0.02) | 0.02 | (0.00,0.05) | 0.02 | (0.00,0.04) | |
| Downtown | Hale | 0.01 | (0.00,0.03) | 0.00 | (0.00,0.02) | 0.01 | (0.00,0.02) | |
| Downtown | Harvard/Kent | 0.05 | (0.03,0.07) | 0.08 | (0.04,0.11) | 0.07 | (0.03,0.12) | 0.01 |
| Downtown | Hennigan | | | 0.00 | (0.00,0.01) | 0.00 | (0.00,0.01) | |
| Downtown | Hernandez | | | 0.02 | (0.00,0.04) | 0.01 | (0.00,0.04) | |
| Downtown | Hurley | 0.15 | (0.10,0.22) | 0.04 | (0.01,0.08) | 0.05 | (0.01,0.08) | 0.07 |
| Downtown | Jackson/Mann | 0.02 | (0.01,0.04) | 0.02 | (0.00,0.05) | 0.02 | (0.00,0.04) | 0.02 |
| Downtown | Kennedy Patrick | 0.01 | (0.00,0.03) | 0.00 | (0.00,0.02) | 0.00 | (0.00,0.02) | |
| Downtown | Lyon K-8 | | | 0.01 | (0.00,0.04) | 0.01 | (0.00,0.04) | |
| Downtown | Mario Umana | | | 0.00 | (0.00,0.02) | 0.00 | (0.00,0.02) | |
| Downtown | Mason | 0.01 | (0.00,0.02) | 0.02 | (0.01,0.05) | 0.02 | (0.01,0.04) | 0.01 |
| Downtown | McKay | | | 0.00 | (0.00,0.02) | 0.00 | (0.00,0.02) | |
| Downtown | Mission Hill | | | | | 0.01 | | |
| Downtown | O'Donnell | | | 0.00 | (0.00,0.02) | 0.00 | (0.00,0.01) | |
| Downtown | Orchard Gardens | 0.03 | (0.01,0.06) | 0.03 | (0.01,0.07) | 0.03 | (0.01,0.06) | 0.01 |
| Downtown | Otis | 0.01 | (0.00,0.03) | | | 0.00 | (0.00,0.01) | |
| Downtown | Quincy | 0.33 | (0.26,0.41) | 0.27 | (0.21,0.34) | 0.29 | (0.22,0.36) | 0.39 |
| Downtown | Russell | 0.01 | (0.00,0.03) | | | 0.00 | (0.00,0.01) | |
| Downtown | Tobin | | | 0.02 | (0.00,0.04) | 0.02 | (0.00,0.05) | |
| Downtown | Warren/Prescott | 0.01 | (0.00,0.03) | 0.05 | (0.02,0.09) | 0.05 | (0.02,0.10) | 0.03 |
| Downtown | West Zone ELC | | | 0.00 | (0.00,0.01) | 0.00 | (0.00,0.02) | |
| Downtown | Winship | 0.02 | (0.01,0.03) | 0.02 | (0.01,0.04) | 0.02 | (0.00,0.04) | |
| Downtown | Winthrop | 0.02 | (0.00,0.04) | 0.01 | (0.00,0.02) | 0.01 | (0.00,0.02) | |
| East Boston | Adams | 0.07 | (0.06,0.09) | 0.09 | (0.06,0.11) | 0.08 | (0.07,0.10) | 0.08 |
| East Boston | Baldwin | | | | | 0.01 | (0.00,0.01) | |
| East Boston | Blackstone | 0.03 | (0.02,0.04) | 0.01 | (0.00,0.02) | 0.01 | (0.01,0.03) | 0.02 |
| East Boston | Bradley | 0.07 | (0.05,0.09) | 0.06 | (0.05,0.08) | 0.07 | (0.05,0.09) | 0.08 |
| East Boston | East Boston EEC | 0.05 | (0.04,0.06) | 0.13 | (0.10,0.16) | 0.13 | (0.10,0.16) | 0.15 |
| East Boston | Edison | | | | | 0.01 | (0.00,0.01) | |
| East Boston | Eliot | 0.01 | (0.00,0.01) | 0.02 | (0.01,0.03) | 0.01 | (0.01,0.03) | 0.02 |
| East Boston | Gardner | | | 0.01 | (0.00,0.02) | 0.02 | (0.01,0.03) | |
| East Boston | Guild | 0.01 | (0.01,0.02) | 0.05 | (0.03,0.08) | 0.04 | (0.03,0.06) | 0.04 |
| East Boston | Harvard/Kent | 0.03 | (0.02,0.04) | 0.02 | (0.01,0.03) | 0.01 | (0.01,0.02) | 0.01 |
| East Boston | Hernandez | | | | | 0.01 | (0.00,0.02) | |
| East Boston | Hurley | 0.33 | (0.29,0.38) | 0.01 | (0.00,0.02) | 0.01 | (0.00,0.02) | 0.01 |
| East Boston | Jackson/Mann | | | | | 0.00 | (0.00,0.01) | |
| East Boston | Kennedy Patrick | 0.06 | (0.05,0.07) | 0.17 | (0.13,0.20) | 0.15 | (0.12,0.18) | 0.14 |
| East Boston | Lyon K-8 | | | | | 0.00 | (0.00,0.01) | |
| East Boston | Mario Umana | 0.03 | (0.02,0.05) | 0.04 | (0.02,0.06) | 0.05 | (0.03,0.07) | 0.03 |
| East Boston | McKay | 0.05 | (0.03,0.07) | 0.15 | (0.12,0.18) | 0.14 | (0.11,0.17) | 0.11 |
| East Boston | O'Donnell | 0.05 | (0.04,0.06) | 0.14 | (0.11,0.17) | 0.11 | (0.09,0.14) | 0.10 |
| East Boston | Orchard Gardens | 0.01 | (0.01,0.02) | 0.01 | (0.00,0.01) | 0.01 | (0.00,0.02) | |
| East Boston | Otis | 0.16 | (0.13,0.19) | 0.08 | (0.06,0.11) | 0.08 | (0.06,0.10) | 0.15 |
| East Boston | Quincy | | | | | 0.00 | (0.00,0.01) | 0.01 |
| East Boston | Tobin | | | | | 0.01 | (0.00,0.01) | |
| East Boston | Warren/Prescott | | | 0.01 | (0.00,0.02) | 0.01 | (0.00,0.02) | |
| East Boston | Winship | | | | | 0.01 | (0.00,0.01) | |
| East Boston | Winthrop | 0.01 | (0.00,0.01) | | | | | |
| Hyde Park | BTU | | | 0.01 | (0.00,0.02) | 0.01 | (0.00,0.02) | |
| Hyde Park | Bates | | | 0.01 | (0.00,0.03) | 0.01 | (0.00,0.02) | 0.02 |
| Hyde Park | Beethoven | 0.03 | (0.02,0.04) | 0.07 | (0.04,0.10) | 0.06 | (0.04,0.09) | 0.04 |

Continued on next page

**Table 1 – continued from previous page**

| | | Naive | | Logit | | Mixed Logit | | |
|---|---|---|---|---|---|---|---|---|
| Neighborhood | School | mean | (95% C.I.) | mean | (95% C.I.) | mean | (95% C.I.) | Actual |
| Hyde Park | Channing | 0.05 | (0.03,0.08) | 0.09 | (0.05,0.13) | 0.08 | (0.05,0.12) | 0.05 |
| Hyde Park | Chittick | 0.07 | (0.05,0.09) | 0.06 | (0.03,0.09) | 0.05 | (0.03,0.08) | 0.08 |
| Hyde Park | Clap | | | 0.00 | (0.00,0.01) | 0.00 | (0.00,0.01) | |
| Hyde Park | Condon | 0.01 | (0.00,0.01) | 0.00 | (0.00,0.01) | 0.01 | (0.00,0.02) | |
| Hyde Park | Conley | 0.15 | (0.11,0.20) | 0.03 | (0.01,0.05) | 0.03 | (0.01,0.06) | 0.02 |
| Hyde Park | Dever | 0.01 | (0.00,0.02) | 0.01 | (0.00,0.02) | 0.01 | (0.00,0.02) | 0.01 |
| Hyde Park | E Greenwood | 0.01 | (0.00,0.03) | 0.07 | (0.04,0.11) | 0.07 | (0.04,0.11) | 0.06 |
| Hyde Park | Ellis | 0.01 | (0.00,0.02) | | | | | |
| Hyde Park | Ellison/Parks | 0.02 | (0.01,0.02) | 0.05 | (0.02,0.07) | 0.04 | (0.02,0.07) | 0.06 |
| Hyde Park | Everett | | | 0.00 | (0.00,0.02) | 0.00 | (0.00,0.01) | |
| Hyde Park | Grew | 0.01 | (0.00,0.03) | 0.05 | (0.02,0.08) | 0.04 | (0.02,0.07) | 0.05 |
| Hyde Park | Haley | 0.01 | (0.00,0.02) | 0.01 | (0.00,0.03) | 0.01 | (0.00,0.03) | |
| Hyde Park | Henderson | 0.03 | (0.01,0.06) | 0.01 | (0.00,0.02) | 0.01 | (0.00,0.02) | 0.01 |
| Hyde Park | Hernandez | 0.01 | (0.00,0.01) | 0.02 | (0.01,0.04) | 0.02 | (0.00,0.03) | 0.02 |
| Hyde Park | Holland | | | 0.01 | (0.00,0.02) | 0.01 | (0.00,0.02) | |
| Hyde Park | Holmes | 0.01 | (0.00,0.01) | 0.00 | (0.00,0.01) | 0.00 | (0.00,0.01) | |
| Hyde Park | Kenny | | | 0.01 | (0.00,0.03) | 0.01 | (0.00,0.02) | |
| Hyde Park | Kilmer | 0.01 | (0.00,0.01) | 0.01 | (0.00,0.02) | 0.01 | (0.00,0.03) | 0.02 |
| Hyde Park | Lyndon | 0.01 | (0.00,0.02) | 0.01 | (0.00,0.03) | 0.01 | (0.00,0.02) | |
| Hyde Park | Mather | 0.01 | (0.00,0.01) | 0.01 | (0.00,0.03) | 0.01 | (0.00,0.02) | |
| Hyde Park | Mattahunt | 0.04 | (0.02,0.05) | 0.03 | (0.01,0.05) | 0.03 | (0.01,0.05) | 0.04 |
| Hyde Park | Mission Hill | | | 0.00 | (0.00,0.01) | | | |
| Hyde Park | Mozart | | | 0.01 | (0.00,0.02) | 0.00 | (0.00,0.01) | |
| Hyde Park | Murphy | 0.02 | (0.00,0.04) | 0.02 | (0.01,0.04) | 0.02 | (0.01,0.05) | 0.02 |
| Hyde Park | Perry | | | 0.00 | (0.00,0.02) | 0.01 | (0.00,0.02) | |
| Hyde Park | Philbrick | 0.01 | (0.00,0.02) | 0.01 | (0.00,0.02) | 0.00 | (0.00,0.01) | |
| Hyde Park | Roosevelt | 0.30 | (0.26,0.37) | 0.26 | (0.21,0.32) | 0.28 | (0.23,0.33) | 0.29 |
| Hyde Park | Russell | | | 0.01 | (0.00,0.02) | 0.01 | (0.00,0.02) | |
| Hyde Park | S. Greenwood | 0.06 | (0.04,0.09) | 0.02 | (0.01,0.04) | 0.02 | (0.01,0.04) | 0.02 |
| Hyde Park | Sumner | 0.02 | (0.01,0.03) | 0.01 | (0.00,0.02) | 0.01 | (0.00,0.03) | |
| Hyde Park | Taylor | 0.06 | (0.03,0.08) | 0.02 | (0.01,0.04) | 0.02 | (0.01,0.03) | 0.02 |
| Hyde Park | Young Achievers | 0.01 | (0.00,0.01) | 0.05 | (0.02,0.07) | 0.05 | (0.03,0.08) | 0.07 |
| Jamaica Plain | BTU | 0.03 | (0.03,0.04) | 0.07 | (0.05,0.10) | 0.07 | (0.04,0.09) | 0.08 |
| Jamaica Plain | Baldwin | | | 0.01 | (0.00,0.03) | 0.01 | (0.00,0.03) | 0.02 |
| Jamaica Plain | Bates | | | 0.01 | (0.00,0.02) | 0.01 | (0.00,0.02) | |
| Jamaica Plain | Beethoven | 0.01 | (0.00,0.02) | 0.02 | (0.01,0.04) | 0.02 | (0.00,0.04) | 0.02 |
| Jamaica Plain | Blackstone | 0.01 | (0.01,0.01) | 0.01 | (0.00,0.03) | 0.01 | (0.00,0.02) | |
| Jamaica Plain | Conley | | | 0.01 | (0.00,0.02) | 0.00 | (0.00,0.01) | |
| Jamaica Plain | Curley | 0.08 | (0.06,0.09) | 0.13 | (0.10,0.17) | 0.14 | (0.11,0.18) | 0.16 |
| Jamaica Plain | East Boston EEC | | | | | 0.00 | (0.00,0.01) | |
| Jamaica Plain | Edison | 0.01 | (0.00,0.01) | 0.01 | (0.00,0.02) | 0.01 | (0.00,0.02) | 0.01 |
| Jamaica Plain | Eliot | | | 0.01 | (0.00,0.02) | 0.01 | (0.00,0.02) | |
| Jamaica Plain | Ellis | 0.01 | (0.01,0.01) | 0.01 | (0.00,0.03) | 0.01 | (0.00,0.03) | 0.01 |
| Jamaica Plain | Gardner | | | 0.01 | (0.00,0.02) | 0.01 | (0.00,0.02) | |
| Jamaica Plain | Hale | 0.20 | (0.16,0.25) | 0.02 | (0.01,0.04) | 0.02 | (0.01,0.04) | 0.01 |
| Jamaica Plain | Haley | 0.02 | (0.01,0.02) | 0.02 | (0.01,0.04) | 0.02 | (0.01,0.04) | 0.02 |
| Jamaica Plain | Harvard/Kent | 0.02 | (0.01,0.03) | 0.01 | (0.00,0.03) | 0.01 | (0.00,0.02) | |
| Jamaica Plain | Haynes | | | 0.01 | (0.00,0.02) | 0.01 | (0.00,0.03) | 0.03 |
| Jamaica Plain | Hennigan | 0.04 | (0.02,0.07) | 0.06 | (0.03,0.09) | 0.05 | (0.03,0.08) | 0.05 |
| Jamaica Plain | Hernandez | 0.03 | (0.02,0.03) | 0.05 | (0.03,0.07) | 0.05 | (0.03,0.08) | 0.05 |
| Jamaica Plain | Higginson/Lewis | 0.02 | (0.01,0.02) | 0.01 | (0.00,0.03) | 0.01 | (0.00,0.03) | 0.01 |
| Jamaica Plain | Hurley | 0.00 | (0.00,0.02) | 0.01 | (0.00,0.03) | 0.01 | (0.00,0.03) | |
| Jamaica Plain | J.F. Kennedy | 0.05 | (0.04,0.07) | 0.06 | (0.03,0.10) | 0.06 | (0.03,0.08) | 0.08 |
| Jamaica Plain | Jackson/Mann | 0.01 | (0.00,0.02) | 0.01 | (0.00,0.03) | 0.01 | (0.00,0.03) | |
| Jamaica Plain | Kilmer | | | 0.02 | (0.01,0.04) | 0.03 | (0.01,0.05) | 0.02 |

Continued on next page

**Table 1 – continued from previous page**

| Neighborhood | School | Naive mean | Naive (95% C.I.) | Logit mean | Logit (95% C.I.) | Mixed Logit mean | Mixed Logit (95% C.I.) | Actual |
|---|---|---|---|---|---|---|---|---|
| Jamaica Plain | Lyndon | 0.00 | (0.00,0.01) | 0.02 | (0.00,0.04) | 0.02 | (0.00,0.03) | |
| Jamaica Plain | Lyon K-8 | 0.00 | (0.00,0.02) | 0.01 | (0.00,0.02) | 0.01 | (0.00,0.02) | |
| Jamaica Plain | Manning | 0.08 | (0.05,0.12) | 0.03 | (0.01,0.05) | 0.03 | (0.01,0.06) | 0.05 |
| Jamaica Plain | Mario Umana | 0.00 | (0.00,0.01) | | | | | |
| Jamaica Plain | Mason | 0.00 | (0.00,0.01) | 0.01 | (0.00,0.02) | 0.01 | (0.00,0.02) | |
| Jamaica Plain | Mendell | 0.07 | (0.06,0.08) | 0.06 | (0.04,0.09) | 0.06 | (0.04,0.09) | 0.04 |
| Jamaica Plain | Mission Hill | 0.02 | (0.01,0.04) | 0.04 | (0.02,0.07) | 0.04 | (0.02,0.06) | 0.09 |
| Jamaica Plain | Mozart | | | 0.01 | (0.00,0.03) | 0.01 | (0.00,0.02) | |
| Jamaica Plain | Orchard Gardens | 0.03 | (0.02,0.03) | 0.03 | (0.01,0.05) | 0.02 | (0.01,0.04) | 0.02 |
| Jamaica Plain | Otis | 0.00 | (0.00,0.01) | | | | | |
| Jamaica Plain | Philbrick | 0.00 | (0.00,0.01) | 0.01 | (0.00,0.02) | 0.01 | (0.00,0.02) | 0.01 |
| Jamaica Plain | Quincy | 0.03 | (0.01,0.05) | 0.02 | (0.00,0.03) | 0.02 | (0.00,0.04) | 0.04 |
| Jamaica Plain | Sumner | 0.06 | (0.03,0.09) | 0.01 | (0.00,0.03) | 0.01 | (0.00,0.03) | 0.01 |
| Jamaica Plain | Taylor | 0.00 | (0.00,0.01) | | | | | |
| Jamaica Plain | Tobin | 0.01 | (0.00,0.02) | 0.03 | (0.01,0.05) | 0.03 | (0.01,0.06) | 0.02 |
| Jamaica Plain | Trotter | 0.02 | (0.01,0.02) | 0.01 | (0.00,0.03) | 0.01 | (0.00,0.03) | 0.02 |
| Jamaica Plain | Tynan | 0.00 | (0.00,0.02) | | | | | |
| Jamaica Plain | Warren/Prescott | | | 0.00 | (0.00,0.01) | 0.00 | (0.00,0.01) | |
| Jamaica Plain | West Zone ELC | 0.04 | (0.03,0.05) | 0.07 | (0.04,0.10) | 0.08 | (0.05,0.11) | 0.05 |
| Jamaica Plain | Winship | | | 0.01 | (0.00,0.02) | 0.01 | (0.00,0.02) | |
| Jamaica Plain | Winthrop | 0.02 | (0.01,0.02) | 0.01 | (0.00,0.02) | 0.01 | (0.00,0.02) | 0.01 |
| Mattapan | BTU | | | 0.01 | (0.00,0.02) | 0.01 | (0.00,0.02) | |
| Mattapan | Beethoven | | | 0.00 | (0.00,0.01) | 0.00 | (0.00,0.01) | |
| Mattapan | Channing | 0.01 | (0.00,0.03) | 0.02 | (0.01,0.04) | 0.02 | (0.00,0.03) | 0.01 |
| Mattapan | Chittick | 0.04 | (0.02,0.05) | 0.04 | (0.02,0.06) | 0.04 | (0.02,0.06) | 0.04 |
| Mattapan | Clap | 0.02 | (0.01,0.04) | 0.02 | (0.00,0.03) | 0.01 | (0.00,0.03) | 0.03 |
| Mattapan | Condon | 0.01 | (0.00,0.02) | 0.01 | (0.00,0.02) | 0.01 | (0.00,0.02) | 0.02 |
| Mattapan | Curley | | | 0.01 | (0.00,0.02) | 0.01 | (0.00,0.01) | |
| Mattapan | Dever | 0.02 | (0.00,0.03) | 0.02 | (0.01,0.04) | 0.02 | (0.01,0.04) | 0.03 |
| Mattapan | E Greenwood | 0.00 | (0.00,0.01) | 0.03 | (0.01,0.05) | 0.02 | (0.01,0.04) | 0.04 |
| Mattapan | Ellison/Parks | 0.04 | (0.02,0.05) | 0.09 | (0.06,0.13) | 0.10 | (0.07,0.14) | 0.13 |
| Mattapan | Everett | 0.00 | (0.00,0.01) | 0.01 | (0.00,0.03) | 0.01 | (0.00,0.02) | 0.01 |
| Mattapan | Grew | | | 0.02 | (0.00,0.03) | 0.01 | (0.00,0.03) | |
| Mattapan | Haley | | | 0.03 | (0.01,0.05) | 0.03 | (0.01,0.05) | 0.02 |
| Mattapan | Henderson | 0.29 | (0.23,0.34) | 0.02 | (0.00,0.03) | 0.02 | (0.01,0.04) | |
| Mattapan | Hernandez | 0.03 | (0.02,0.04) | 0.05 | (0.03,0.07) | 0.04 | (0.03,0.06) | 0.05 |
| Mattapan | Holland | 0.03 | (0.02,0.04) | 0.03 | (0.01,0.05) | 0.03 | (0.01,0.05) | 0.04 |
| Mattapan | Holmes | 0.02 | (0.01,0.03) | 0.02 | (0.00,0.04) | 0.02 | (0.01,0.04) | 0.03 |
| Mattapan | J.F. Kennedy | 0.01 | (0.00,0.02) | 0.00 | (0.00,0.01) | 0.00 | (0.00,0.01) | 0.01 |
| Mattapan | Kenny | 0.00 | (0.00,0.01) | 0.02 | (0.01,0.04) | 0.02 | (0.01,0.04) | 0.01 |
| Mattapan | Lyndon | 0.01 | (0.00,0.02) | 0.01 | (0.00,0.02) | 0.01 | (0.00,0.02) | |
| Mattapan | Mather | 0.03 | (0.02,0.04) | 0.03 | (0.01,0.04) | 0.02 | (0.01,0.04) | 0.02 |
| Mattapan | Mattahunt | 0.04 | (0.02,0.05) | 0.04 | (0.02,0.06) | 0.03 | (0.01,0.06) | 0.07 |
| Mattapan | Mission Hill | 0.00 | (0.00,0.01) | 0.00 | (0.00,0.01) | 0.00 | (0.00,0.01) | |
| Mattapan | Mozart | | | 0.00 | (0.00,0.01) | | | |
| Mattapan | Murphy | 0.02 | (0.01,0.04) | 0.04 | (0.02,0.07) | 0.06 | (0.03,0.09) | 0.06 |
| Mattapan | Orchard Gardens | 0.01 | (0.00,0.02) | | | | | |
| Mattapan | Perkins | | | 0.01 | (0.00,0.02) | 0.00 | (0.00,0.01) | |
| Mattapan | Perry | | | 0.01 | (0.00,0.03) | 0.01 | (0.00,0.03) | |
| Mattapan | Philbrick | 0.04 | (0.02,0.06) | 0.00 | (0.00,0.01) | 0.00 | (0.00,0.01) | |
| Mattapan | Quincy | 0.00 | (0.00,0.01) | | | | | |
| Mattapan | Roosevelt | 0.03 | (0.02,0.04) | 0.05 | (0.03,0.08) | 0.05 | (0.03,0.08) | 0.03 |
| Mattapan | Russell | 0.03 | (0.02,0.04) | 0.03 | (0.01,0.04) | 0.03 | (0.01,0.04) | 0.03 |
| Mattapan | S. Greenwood | 0.08 | (0.05,0.11) | 0.06 | (0.04,0.09) | 0.06 | (0.04,0.09) | 0.06 |
| Mattapan | Sumner | 0.02 | (0.01,0.04) | 0.01 | (0.00,0.02) | 0.01 | (0.00,0.02) | 0.01 |

Continued on next page

**Table 1 – continued from previous page**

| Neighborhood | School | Naive mean | Naive (95% C.I.) | Logit mean | Logit (95% C.I.) | Mixed Logit mean | Mixed Logit (95% C.I.) | Actual |
|---|---|---|---|---|---|---|---|---|
| Mattapan | Taylor | 0.06 | (0.04,0.08) | 0.06 | (0.03,0.08) | 0.05 | (0.03,0.07) | 0.07 |
| Mattapan | Tobin | 0.00 | (0.00,0.01) | | | | | |
| Mattapan | Trotter | 0.01 | (0.00,0.02) | 0.01 | (0.00,0.02) | 0.01 | (0.00,0.02) | 0.01 |
| Mattapan | Tynan | 0.00 | (0.00,0.01) | 0.01 | (0.00,0.02) | 0.00 | (0.00,0.01) | |
| Mattapan | West Zone ELC | 0.01 | (0.00,0.02) | 0.00 | (0.00,0.01) | 0.00 | (0.00,0.01) | |
| Mattapan | Winthrop | 0.01 | (0.00,0.02) | | | | | |
| Mattapan | Young Achievers | 0.04 | (0.03,0.06) | 0.16 | (0.11,0.21) | 0.19 | (0.14,0.23) | 0.13 |
| North Dorchester | Baldwin | | | 0.00 | (0.00,0.01) | 0.00 | (0.00,0.01) | |
| North Dorchester | Bates | 0.01 | (0.00,0.02) | | | | | |
| North Dorchester | Blackstone | | | 0.01 | (0.00,0.02) | 0.01 | (0.00,0.02) | |
| North Dorchester | Channing | | | 0.01 | (0.00,0.02) | 0.01 | (0.00,0.02) | |
| North Dorchester | Chittick | | | 0.00 | (0.00,0.01) | 0.00 | (0.00,0.01) | |
| North Dorchester | Clap | 0.03 | (0.01,0.05) | 0.06 | (0.04,0.09) | 0.06 | (0.03,0.09) | 0.08 |
| North Dorchester | Condon | 0.04 | (0.02,0.06) | 0.04 | (0.01,0.07) | 0.03 | (0.01,0.07) | 0.04 |
| North Dorchester | Dever | 0.05 | (0.02,0.07) | 0.08 | (0.04,0.13) | 0.08 | (0.04,0.12) | 0.04 |
| North Dorchester | E Greenwood | | | 0.01 | (0.00,0.02) | 0.01 | (0.00,0.02) | |
| North Dorchester | East Boston EEC | | | | | 0.00 | (0.00,0.01) | |
| North Dorchester | Eliot | 0.01 | (0.00,0.02) | 0.01 | (0.00,0.02) | 0.01 | (0.00,0.02) | |
| North Dorchester | Ellison/Parks | | | 0.01 | (0.00,0.03) | 0.01 | (0.00,0.03) | |
| North Dorchester | Everett | 0.01 | (0.00,0.02) | 0.06 | (0.03,0.09) | 0.06 | (0.03,0.10) | 0.10 |
| North Dorchester | Gardner | | | 0.00 | (0.00,0.01) | 0.00 | (0.00,0.01) | |
| North Dorchester | Grew | 0.01 | (0.00,0.02) | 0.00 | (0.00,0.01) | 0.00 | (0.00,0.02) | |
| North Dorchester | Haynes | 0.02 | (0.01,0.03) | 0.04 | (0.01,0.07) | 0.04 | (0.02,0.07) | 0.04 |
| North Dorchester | Henderson | 0.09 | (0.04,0.14) | 0.02 | (0.00,0.04) | 0.02 | (0.00,0.04) | |
| North Dorchester | Hernandez | | | 0.02 | (0.00,0.04) | 0.02 | (0.00,0.04) | |
| North Dorchester | Higginson/Lewis | | | 0.00 | (0.00,0.01) | 0.00 | (0.00,0.01) | |
| North Dorchester | Holland | 0.05 | (0.02,0.07) | 0.05 | (0.03,0.09) | 0.05 | (0.02,0.08) | 0.04 |
| North Dorchester | Holmes | | | 0.01 | (0.00,0.02) | 0.01 | (0.00,0.02) | 0.01 |
| North Dorchester | Hurley | 0.01 | (0.00,0.02) | 0.01 | (0.00,0.02) | 0.01 | (0.00,0.02) | |
| North Dorchester | Jackson/Mann | | | 0.01 | (0.00,0.02) | 0.00 | (0.00,0.01) | |
| North Dorchester | Kenny | | | 0.01 | (0.00,0.03) | 0.01 | (0.00,0.02) | |
| North Dorchester | King | | | 0.01 | (0.00,0.03) | 0.01 | (0.00,0.02) | 0.01 |
| North Dorchester | Mason | 0.24 | (0.17,0.32) | 0.05 | (0.02,0.08) | 0.05 | (0.02,0.08) | 0.04 |
| North Dorchester | Mather | 0.09 | (0.06,0.13) | 0.09 | (0.06,0.13) | 0.10 | (0.06,0.13) | 0.12 |
| North Dorchester | Mattahunt | 0.02 | (0.00,0.04) | 0.00 | (0.00,0.02) | 0.00 | (0.00,0.01) | 0.01 |
| North Dorchester | Murphy | 0.06 | (0.03,0.10) | 0.07 | (0.04,0.11) | 0.09 | (0.05,0.14) | 0.15 |
| North Dorchester | Orchard Gardens | 0.06 | (0.03,0.10) | 0.03 | (0.01,0.05) | 0.03 | (0.01,0.06) | 0.01 |
| North Dorchester | Otis | 0.01 | (0.00,0.03) | | | | | |
| North Dorchester | Perkins | | | 0.01 | (0.00,0.04) | 0.01 | (0.00,0.03) | |
| North Dorchester | Perry | | | 0.03 | (0.01,0.06) | 0.03 | (0.01,0.06) | 0.02 |
| North Dorchester | Quincy | 0.02 | (0.00,0.04) | 0.01 | (0.00,0.03) | 0.01 | (0.00,0.03) | |
| North Dorchester | Roosevelt | 0.02 | (0.01,0.04) | 0.01 | (0.00,0.03) | 0.02 | (0.01,0.04) | |
| North Dorchester | Russell | 0.07 | (0.04,0.10) | 0.10 | (0.07,0.14) | 0.11 | (0.07,0.15) | 0.11 |
| North Dorchester | S. Greenwood | 0.02 | (0.00,0.04) | 0.01 | (0.00,0.03) | 0.01 | (0.00,0.03) | 0.01 |
| North Dorchester | Taylor | | | 0.00 | (0.00,0.02) | 0.00 | (0.00,0.01) | |
| North Dorchester | Tobin | | | 0.00 | (0.00,0.01) | 0.00 | (0.00,0.01) | |
| North Dorchester | Trotter | | | 0.00 | (0.00,0.02) | 0.00 | (0.00,0.01) | 0.02 |
| North Dorchester | Tynan | 0.01 | (0.00,0.02) | 0.01 | (0.00,0.03) | 0.01 | (0.00,0.03) | |
| North Dorchester | Warren/Prescott | | | 0.00 | (0.00,0.01) | | | |
| North Dorchester | Winship | | | 0.00 | (0.00,0.01) | 0.00 | (0.00,0.01) | |
| North Dorchester | Winthrop | 0.03 | (0.02,0.05) | 0.04 | (0.01,0.06) | 0.03 | (0.01,0.05) | 0.03 |
| North Dorchester | Young Achievers | 0.01 | (0.00,0.02) | 0.02 | (0.00,0.04) | 0.02 | (0.00,0.04) | |
| Roslindale | BTU | 0.03 | (0.02,0.05) | 0.10 | (0.07,0.13) | 0.10 | (0.07,0.13) | 0.08 |
| Roslindale | Bates | 0.01 | (0.00,0.03) | 0.04 | (0.02,0.07) | 0.05 | (0.02,0.07) | 0.06 |
| Roslindale | Beethoven | 0.06 | (0.04,0.08) | 0.11 | (0.08,0.15) | 0.11 | (0.08,0.15) | 0.09 |

Continued on next page

**Table 1 – continued from previous page**

| Neighborhood | School | Naive mean | Naive (95% C.I.) | Logit mean | Logit (95% C.I.) | Mixed Logit mean | Mixed Logit (95% C.I.) | Actual |
|---|---|---|---|---|---|---|---|---|
| Roslindale | Channing | | | 0.00 | (0.00,0.01) | 0.00 | (0.00,0.01) | |
| Roslindale | Chittick | | | 0.00 | (0.00,0.01) | | | |
| Roslindale | Condon | 0.01 | (0.00,0.02) | | | | | |
| Roslindale | Conley | 0.09 | (0.06,0.12) | 0.03 | (0.01,0.05) | 0.03 | (0.01,0.04) | 0.05 |
| Roslindale | Curley | 0.02 | (0.01,0.04) | 0.03 | (0.01,0.06) | 0.03 | (0.02,0.05) | 0.03 |
| Roslindale | E Greenwood | | | 0.01 | (0.00,0.03) | 0.01 | (0.00,0.03) | |
| Roslindale | Ellis | 0.02 | (0.01,0.03) | 0.01 | (0.00,0.02) | 0.01 | (0.00,0.02) | |
| Roslindale | Grew | 0.00 | (0.00,0.01) | 0.01 | (0.00,0.02) | 0.01 | (0.00,0.02) | |
| Roslindale | Hale | 0.01 | (0.00,0.02) | 0.00 | (0.00,0.01) | 0.00 | (0.00,0.01) | |
| Roslindale | Haley | 0.04 | (0.03,0.05) | 0.06 | (0.04,0.08) | 0.06 | (0.04,0.09) | 0.08 |
| Roslindale | Haynes | | | 0.01 | (0.00,0.02) | 0.01 | (0.00,0.02) | 0.01 |
| Roslindale | Hennigan | 0.01 | (0.00,0.02) | 0.01 | (0.00,0.03) | 0.01 | (0.00,0.02) | |
| Roslindale | Hernandez | 0.03 | (0.01,0.04) | 0.04 | (0.02,0.06) | 0.03 | (0.02,0.05) | 0.05 |
| Roslindale | Higginson/Lewis | 0.01 | (0.00,0.03) | 0.00 | (0.00,0.01) | 0.00 | (0.00,0.01) | |
| Roslindale | J.F. Kennedy | 0.02 | (0.01,0.03) | 0.01 | (0.00,0.03) | 0.01 | (0.00,0.02) | |
| Roslindale | Kilmer | 0.02 | (0.01,0.03) | 0.06 | (0.04,0.08) | 0.08 | (0.05,0.10) | 0.08 |
| Roslindale | Lyndon | 0.07 | (0.05,0.09) | 0.10 | (0.07,0.14) | 0.09 | (0.06,0.12) | 0.10 |
| Roslindale | Manning | 0.00 | (0.00,0.01) | 0.02 | (0.01,0.04) | 0.02 | (0.00,0.04) | 0.01 |
| Roslindale | Mattahunt | 0.01 | (0.00,0.01) | 0.01 | (0.00,0.02) | 0.01 | (0.00,0.02) | |
| Roslindale | Mendell | 0.02 | (0.01,0.03) | 0.02 | (0.00,0.03) | 0.02 | (0.00,0.03) | 0.02 |
| Roslindale | Mission Hill | | | 0.02 | (0.01,0.04) | 0.02 | (0.00,0.04) | 0.04 |
| Roslindale | Mozart | 0.05 | (0.03,0.06) | 0.08 | (0.05,0.11) | 0.08 | (0.05,0.10) | 0.04 |
| Roslindale | Philbrick | 0.06 | (0.03,0.09) | 0.02 | (0.01,0.05) | 0.02 | (0.01,0.04) | 0.04 |
| Roslindale | Roosevelt | | | 0.01 | (0.00,0.02) | 0.01 | (0.00,0.02) | 0.01 |
| Roslindale | Sumner | 0.31 | (0.26,0.36) | 0.11 | (0.08,0.14) | 0.12 | (0.09,0.16) | 0.11 |
| Roslindale | Taylor | 0.03 | (0.01,0.05) | 0.01 | (0.00,0.02) | 0.01 | (0.00,0.02) | 0.01 |
| Roslindale | Trotter | 0.03 | (0.02,0.04) | 0.01 | (0.00,0.02) | 0.01 | (0.00,0.02) | |
| Roslindale | West Zone ELC | 0.02 | (0.01,0.02) | 0.02 | (0.00,0.03) | 0.02 | (0.01,0.04) | 0.03 |
| Roslindale | Young Achievers | | | 0.01 | (0.00,0.02) | 0.01 | (0.00,0.02) | |
| Roxbury | BTU | | | 0.03 | (0.02,0.04) | 0.02 | (0.01,0.04) | 0.01 |
| Roxbury | Baldwin | | | 0.01 | (0.00,0.01) | 0.01 | (0.00,0.01) | |
| Roxbury | Bates | | | 0.01 | (0.00,0.01) | 0.00 | (0.00,0.01) | |
| Roxbury | Beethoven | 0.03 | (0.02,0.04) | 0.02 | (0.01,0.03) | 0.02 | (0.01,0.03) | 0.02 |
| Roxbury | Blackstone | 0.01 | (0.01,0.02) | 0.02 | (0.01,0.03) | 0.02 | (0.01,0.03) | 0.01 |
| Roxbury | Clap | | | 0.01 | (0.00,0.01) | 0.01 | (0.00,0.01) | |
| Roxbury | Conley | | | 0.00 | (0.00,0.01) | | | |
| Roxbury | Curley | 0.04 | (0.03,0.05) | 0.05 | (0.03,0.07) | 0.05 | (0.04,0.07) | 0.04 |
| Roxbury | Dever | 0.01 | (0.01,0.02) | 0.01 | (0.00,0.02) | 0.01 | (0.00,0.02) | |
| Roxbury | Edison | 0.01 | (0.01,0.01) | 0.01 | (0.00,0.01) | | | |
| Roxbury | Eliot | | | 0.01 | (0.00,0.02) | 0.01 | (0.00,0.01) | |
| Roxbury | Ellis | 0.05 | (0.04,0.06) | 0.05 | (0.03,0.06) | 0.05 | (0.04,0.06) | 0.06 |
| Roxbury | Everett | | | 0.01 | (0.00,0.02) | 0.01 | (0.00,0.02) | |
| Roxbury | Gardner | | | 0.01 | (0.00,0.01) | 0.01 | (0.00,0.01) | |
| Roxbury | Hale | 0.17 | (0.14,0.20) | 0.03 | (0.02,0.05) | 0.04 | (0.02,0.05) | 0.04 |
| Roxbury | Haley | 0.01 | (0.00,0.01) | 0.01 | (0.01,0.02) | 0.01 | (0.00,0.02) | |
| Roxbury | Harvard/Kent | 0.00 | (0.00,0.01) | | | | | |
| Roxbury | Haynes | 0.01 | (0.01,0.01) | 0.04 | (0.02,0.05) | 0.04 | (0.03,0.06) | 0.06 |
| Roxbury | Henderson | 0.04 | (0.03,0.06) | | | 0.00 | (0.00,0.01) | |
| Roxbury | Hennigan | 0.02 | (0.01,0.03) | 0.03 | (0.01,0.05) | 0.03 | (0.01,0.04) | 0.03 |
| Roxbury | Hernandez | 0.02 | (0.01,0.03) | 0.05 | (0.04,0.07) | 0.06 | (0.04,0.08) | 0.06 |
| Roxbury | Higginson/Lewis | 0.02 | (0.01,0.03) | 0.02 | (0.01,0.03) | 0.02 | (0.01,0.03) | 0.03 |
| Roxbury | Holland | 0.02 | (0.01,0.02) | 0.03 | (0.02,0.04) | 0.03 | (0.02,0.04) | 0.03 |
| Roxbury | Holmes | | | 0.01 | (0.00,0.01) | 0.01 | (0.00,0.01) | |
| Roxbury | Hurley | 0.05 | (0.03,0.07) | 0.02 | (0.01,0.03) | 0.02 | (0.01,0.03) | |
| Roxbury | J.F. Kennedy | 0.03 | (0.02,0.04) | 0.03 | (0.02,0.05) | 0.03 | (0.02,0.04) | 0.02 |

Continued on next page

**Table 1 – continued from previous page**

| Neighborhood | School | Naive mean | Naive (95% C.I.) | Logit mean | Logit (95% C.I.) | Mixed Logit mean | Mixed Logit (95% C.I.) | Actual |
|---|---|---|---|---|---|---|---|---|
| Roxbury | Jackson/Mann | 0.01 | (0.00,0.01) | 0.01 | (0.00,0.01) | | | |
| Roxbury | Kilmer | 0.01 | (0.00,0.01) | 0.01 | (0.00,0.01) | 0.01 | (0.00,0.02) | |
| Roxbury | King | 0.03 | (0.02,0.03) | 0.02 | (0.01,0.03) | 0.02 | (0.01,0.03) | 0.05 |
| Roxbury | Lyndon | 0.01 | (0.00,0.01) | 0.02 | (0.01,0.03) | 0.01 | (0.01,0.02) | 0.01 |
| Roxbury | Manning | | | 0.01 | (0.00,0.01) | 0.01 | (0.00,0.01) | |
| Roxbury | Mason | 0.07 | (0.06,0.09) | 0.03 | (0.02,0.04) | 0.03 | (0.02,0.04) | 0.03 |
| Roxbury | Mather | 0.01 | (0.01,0.01) | 0.01 | (0.01,0.02) | 0.01 | (0.01,0.02) | 0.01 |
| Roxbury | Mattahunt | 0.00 | (0.00,0.01) | | | | | |
| Roxbury | Mendell | 0.01 | (0.01,0.02) | 0.02 | (0.01,0.04) | 0.02 | (0.01,0.03) | 0.03 |
| Roxbury | Mission Hill | | | 0.02 | (0.01,0.03) | 0.02 | (0.01,0.03) | 0.01 |
| Roxbury | Mozart | | | 0.01 | (0.00,0.01) | 0.00 | (0.00,0.01) | |
| Roxbury | Murphy | | | 0.01 | (0.00,0.01) | 0.01 | (0.00,0.01) | |
| Roxbury | Orchard Gardens | 0.06 | (0.05,0.07) | 0.06 | (0.04,0.08) | 0.06 | (0.04,0.07) | 0.06 |
| Roxbury | Otis | 0.01 | (0.00,0.02) | | | | | |
| Roxbury | Philbrick | | | 0.00 | (0.00,0.01) | | | |
| Roxbury | Quincy | | | 0.01 | (0.00,0.01) | 0.01 | (0.00,0.01) | 0.01 |
| Roxbury | Roosevelt | | | | | 0.00 | (0.00,0.01) | |
| Roxbury | Russell | 0.01 | (0.00,0.01) | 0.02 | (0.01,0.03) | 0.02 | (0.01,0.03) | 0.01 |
| Roxbury | S. Greenwood | 0.01 | (0.01,0.02) | 0.02 | (0.01,0.04) | 0.03 | (0.01,0.04) | 0.03 |
| Roxbury | Sumner | 0.05 | (0.03,0.06) | 0.02 | (0.01,0.03) | 0.02 | (0.01,0.02) | 0.01 |
| Roxbury | Taylor | 0.01 | (0.00,0.01) | 0.00 | (0.00,0.01) | | | |
| Roxbury | Tobin | 0.01 | (0.00,0.01) | 0.02 | (0.01,0.03) | 0.01 | (0.01,0.02) | 0.02 |
| Roxbury | Trotter | 0.06 | (0.04,0.07) | 0.05 | (0.03,0.07) | 0.05 | (0.04,0.06) | 0.06 |
| Roxbury | West Zone ELC | 0.01 | (0.01,0.02) | 0.03 | (0.02,0.04) | 0.03 | (0.02,0.05) | 0.02 |
| Roxbury | Winship | | | 0.01 | (0.00,0.01) | | | |
| Roxbury | Winthrop | 0.04 | (0.03,0.05) | 0.04 | (0.03,0.06) | 0.04 | (0.03,0.06) | 0.06 |
| Roxbury | Young Achievers | | | 0.01 | (0.01,0.02) | 0.01 | (0.01,0.02) | 0.01 |
| South Boston | Blackstone | 0.01 | (0.00,0.02) | 0.02 | (0.01,0.05) | 0.02 | (0.01,0.05) | |
| South Boston | Channing | | | 0.00 | (0.00,0.01) | 0.00 | (0.00,0.02) | |
| South Boston | Chittick | | | 0.00 | (0.00,0.01) | 0.00 | (0.00,0.01) | |
| South Boston | Clap | | | 0.03 | (0.01,0.07) | 0.04 | (0.01,0.07) | 0.03 |
| South Boston | Condon | 0.22 | (0.17,0.28) | 0.23 | (0.17,0.30) | 0.23 | (0.17,0.29) | 0.34 |
| South Boston | Dever | 0.02 | (0.01,0.03) | 0.08 | (0.04,0.13) | 0.08 | (0.05,0.12) | 0.05 |
| South Boston | E Greenwood | | | 0.00 | (0.00,0.02) | 0.01 | (0.00,0.02) | |
| South Boston | Ellison/Parks | | | 0.01 | (0.00,0.03) | 0.01 | (0.00,0.03) | |
| South Boston | Everett | | | 0.02 | (0.00,0.05) | 0.02 | (0.00,0.04) | |
| South Boston | Grew | | | | | 0.00 | (0.00,0.02) | |
| South Boston | Harvard/Kent | | | 0.01 | (0.00,0.02) | 0.01 | (0.00,0.02) | |
| South Boston | Henderson | 0.04 | (0.01,0.07) | 0.01 | (0.00,0.03) | 0.01 | (0.00,0.03) | 0.03 |
| South Boston | Hernandez | | | 0.02 | (0.01,0.05) | 0.02 | (0.01,0.05) | |
| South Boston | Holland | 0.02 | (0.01,0.03) | 0.02 | (0.01,0.05) | 0.02 | (0.00,0.04) | 0.02 |
| South Boston | Holmes | | | 0.00 | (0.00,0.02) | 0.00 | (0.00,0.01) | |
| South Boston | Kenny | 0.01 | (0.00,0.03) | 0.01 | (0.00,0.02) | 0.01 | (0.00,0.02) | |
| South Boston | Mason | 0.07 | (0.03,0.11) | 0.02 | (0.00,0.04) | 0.02 | (0.00,0.04) | |
| South Boston | Mather | | | 0.01 | (0.00,0.04) | 0.01 | (0.00,0.03) | |
| South Boston | Murphy | 0.16 | (0.10,0.22) | 0.05 | (0.01,0.08) | 0.05 | (0.01,0.09) | 0.04 |
| South Boston | Orchard Gardens | 0.01 | (0.00,0.03) | 0.01 | (0.00,0.02) | 0.01 | (0.00,0.02) | |
| South Boston | Perkins | 0.03 | (0.01,0.07) | 0.04 | (0.01,0.07) | 0.04 | (0.01,0.08) | 0.08 |
| South Boston | Perry | 0.09 | (0.06,0.12) | 0.20 | (0.15,0.27) | 0.21 | (0.16,0.27) | 0.20 |
| South Boston | Quincy | 0.10 | (0.05,0.15) | 0.04 | (0.01,0.08) | 0.05 | (0.01,0.08) | 0.05 |
| South Boston | Roosevelt | | | 0.00 | (0.00,0.02) | 0.01 | (0.00,0.03) | |
| South Boston | Russell | | | 0.04 | (0.01,0.08) | 0.04 | (0.01,0.07) | |
| South Boston | S. Greenwood | 0.13 | (0.07,0.18) | 0.02 | (0.00,0.04) | 0.02 | (0.00,0.04) | 0.01 |
| South Boston | Taylor | | | 0.00 | (0.00,0.01) | 0.00 | (0.00,0.01) | |
| South Boston | Tynan | 0.02 | (0.00,0.05) | 0.05 | (0.02,0.09) | 0.05 | (0.01,0.09) | 0.06 |

Continued on next page

**Table 1 – continued from previous page**

| Neighborhood | School | Naive mean | Naive (95% C.I.) | Logit mean | Logit (95% C.I.) | Mixed Logit mean | Mixed Logit (95% C.I.) | Actual |
|---|---|---|---|---|---|---|---|---|
| South Boston | Young Achievers | 0.01 | (0.00,0.03) | 0.02 | (0.00,0.05) | 0.02 | (0.00,0.05) | 0.01 |
| South Dorchester | Channing | 0.01 | (0.00,0.02) | 0.01 | (0.00,0.02) | 0.01 | (0.00,0.02) | 0.01 |
| South Dorchester | Chittick | 0.01 | (0.01,0.02) | 0.01 | (0.00,0.02) | 0.01 | (0.00,0.02) | |
| South Dorchester | Clap | 0.01 | (0.00,0.02) | 0.02 | (0.01,0.03) | 0.02 | (0.01,0.03) | 0.01 |
| South Dorchester | Condon | 0.03 | (0.02,0.04) | 0.03 | (0.01,0.04) | 0.02 | (0.01,0.03) | 0.03 |
| South Dorchester | Dever | 0.03 | (0.01,0.04) | 0.04 | (0.02,0.05) | 0.04 | (0.02,0.06) | 0.02 |
| South Dorchester | E Greenwood | | | 0.01 | (0.00,0.03) | 0.01 | (0.00,0.02) | |
| South Dorchester | Ellison/Parks | 0.01 | (0.00,0.01) | 0.03 | (0.01,0.04) | 0.03 | (0.01,0.04) | 0.05 |
| South Dorchester | Everett | 0.01 | (0.00,0.02) | 0.03 | (0.01,0.05) | 0.03 | (0.01,0.04) | 0.02 |
| South Dorchester | Grew | | | 0.01 | (0.00,0.01) | 0.01 | (0.00,0.01) | |
| South Dorchester | Haynes | | | 0.01 | (0.00,0.02) | 0.01 | (0.00,0.02) | 0.01 |
| South Dorchester | Henderson | 0.26 | (0.21,0.30) | 0.05 | (0.03,0.07) | 0.06 | (0.04,0.08) | 0.08 |
| South Dorchester | Hernandez | | | 0.03 | (0.01,0.04) | 0.03 | (0.01,0.04) | 0.02 |
| South Dorchester | Holland | 0.07 | (0.05,0.08) | 0.08 | (0.06,0.10) | 0.08 | (0.06,0.10) | 0.07 |
| South Dorchester | Holmes | 0.03 | (0.02,0.04) | 0.03 | (0.02,0.05) | 0.04 | (0.02,0.05) | 0.04 |
| South Dorchester | Kenny | 0.05 | (0.04,0.07) | 0.06 | (0.04,0.09) | 0.07 | (0.05,0.09) | 0.04 |
| South Dorchester | King | 0.01 | (0.01,0.02) | 0.01 | (0.01,0.02) | 0.01 | (0.01,0.02) | 0.02 |
| South Dorchester | Mather | 0.11 | (0.09,0.13) | 0.10 | (0.08,0.12) | 0.09 | (0.07,0.12) | 0.11 |
| South Dorchester | Mattahunt | 0.01 | (0.00,0.02) | 0.01 | (0.00,0.02) | 0.01 | (0.00,0.01) | 0.01 |
| South Dorchester | Murphy | 0.15 | (0.12,0.18) | 0.18 | (0.15,0.22) | 0.21 | (0.18,0.25) | 0.24 |
| South Dorchester | Orchard Gardens | 0.02 | (0.01,0.04) | 0.01 | (0.00,0.01) | 0.00 | (0.00,0.01) | |
| South Dorchester | Perkins | | | 0.01 | (0.00,0.02) | 0.01 | (0.00,0.01) | |
| South Dorchester | Perry | 0.01 | (0.01,0.02) | 0.03 | (0.01,0.04) | 0.02 | (0.01,0.04) | 0.01 |
| South Dorchester | Roosevelt | 0.01 | (0.01,0.01) | 0.02 | (0.01,0.03) | 0.02 | (0.01,0.04) | 0.01 |
| South Dorchester | Russell | 0.02 | (0.01,0.03) | 0.03 | (0.02,0.05) | 0.03 | (0.02,0.05) | 0.02 |
| South Dorchester | S. Greenwood | 0.08 | (0.06,0.10) | 0.06 | (0.04,0.08) | 0.06 | (0.04,0.08) | 0.05 |
| South Dorchester | Taylor | 0.02 | (0.01,0.03) | 0.02 | (0.01,0.03) | 0.02 | (0.01,0.03) | 0.01 |
| South Dorchester | Tynan | 0.01 | (0.00,0.02) | 0.01 | (0.00,0.02) | 0.01 | (0.00,0.01) | |
| South Dorchester | Winthrop | 0.01 | (0.00,0.01) | 0.01 | (0.00,0.02) | 0.01 | (0.00,0.02) | |
| South Dorchester | Young Achievers | 0.01 | (0.01,0.02) | 0.06 | (0.04,0.08) | 0.06 | (0.04,0.08) | 0.05 |
| South End | Adams | | | | | 0.00 | (0.00,0.01) | |
| South End | Baldwin | 0.01 | (0.00,0.01) | 0.02 | (0.01,0.05) | 0.02 | (0.01,0.05) | 0.02 |
| South End | Blackstone | 0.10 | (0.07,0.13) | 0.12 | (0.09,0.17) | 0.12 | (0.09,0.17) | 0.14 |
| South End | Bradley | | | 0.00 | (0.00,0.01) | 0.00 | (0.00,0.01) | |
| South End | Condon | | | 0.02 | (0.01,0.04) | 0.02 | (0.01,0.04) | |
| South End | Curley | 0.01 | (0.00,0.02) | 0.00 | (0.00,0.01) | 0.00 | (0.00,0.01) | |
| South End | East Boston EEC | | | 0.01 | (0.00,0.02) | 0.01 | (0.00,0.04) | |
| South End | Edison | 0.03 | (0.01,0.05) | 0.02 | (0.01,0.04) | 0.02 | (0.01,0.03) | 0.02 |
| South End | Eliot | 0.02 | (0.01,0.02) | 0.08 | (0.04,0.11) | 0.07 | (0.04,0.10) | 0.07 |
| South End | Gardner | 0.01 | (0.01,0.03) | 0.03 | (0.01,0.06) | 0.03 | (0.01,0.05) | 0.01 |
| South End | Guild | | | 0.00 | (0.00,0.01) | 0.00 | (0.00,0.01) | |
| South End | Hale | | | 0.01 | (0.00,0.03) | 0.01 | (0.00,0.03) | |
| South End | Harvard/Kent | 0.05 | (0.03,0.07) | 0.05 | (0.03,0.07) | 0.04 | (0.02,0.07) | |
| South End | Hernandez | 0.03 | (0.02,0.03) | 0.04 | (0.02,0.07) | 0.04 | (0.02,0.07) | 0.04 |
| South End | Higginson/Lewis | | | 0.01 | (0.00,0.01) | 0.01 | (0.00,0.02) | |
| South End | Hurley | 0.38 | (0.32,0.43) | 0.15 | (0.11,0.19) | 0.16 | (0.12,0.21) | 0.22 |
| South End | J.F. Kennedy | 0.01 | (0.00,0.02) | 0.00 | (0.00,0.01) | 0.00 | (0.00,0.01) | |
| South End | Jackson/Mann | 0.02 | (0.01,0.04) | 0.02 | (0.00,0.04) | 0.01 | (0.00,0.03) | |
| South End | Kennedy Patrick | | | 0.00 | (0.00,0.02) | 0.00 | (0.00,0.01) | |
| South End | Lyon K-8 | | | 0.01 | (0.00,0.03) | 0.01 | (0.00,0.03) | 0.02 |
| South End | Mario Umana | | | 0.00 | (0.00,0.02) | 0.01 | (0.00,0.02) | |
| South End | Mason | | | 0.04 | (0.01,0.07) | 0.03 | (0.01,0.06) | |
| South End | Mather | 0.01 | (0.00,0.02) | | | 0.00 | (0.00,0.01) | |
| South End | McKay | | | 0.00 | (0.00,0.01) | 0.01 | (0.00,0.02) | |
| South End | Mendell | 0.01 | (0.00,0.02) | | | | | |

Continued on next page

**Table 1 – continued from previous page**

| Neighborhood | School | Naive mean | Naive (95% C.I.) | Logit mean | Logit (95% C.I.) | Mixed Logit mean | Mixed Logit (95% C.I.) | Actual |
|---|---|---|---|---|---|---|---|---|
| South End | Mission Hill | 0.01 | (0.00,0.03) | 0.00 | (0.00,0.01) | 0.00 | (0.00,0.01) | 0.01 |
| South End | O'Donnell | | | 0.00 | (0.00,0.02) | 0.00 | (0.00,0.01) | |
| South End | Orchard Gardens | 0.07 | (0.05,0.09) | 0.10 | (0.06,0.14) | 0.09 | (0.06,0.13) | 0.09 |
| South End | Otis | 0.03 | (0.01,0.06) | 0.00 | (0.00,0.01) | 0.00 | (0.00,0.01) | |
| South End | Quincy | 0.18 | (0.13,0.23) | 0.15 | (0.11,0.20) | 0.18 | (0.13,0.23) | 0.29 |
| South End | S. Greenwood | 0.01 | (0.00,0.02) | | | | | |
| South End | Tobin | 0.01 | (0.00,0.02) | 0.03 | (0.01,0.05) | 0.03 | (0.01,0.05) | 0.02 |
| South End | Warren/Prescott | | | 0.02 | (0.01,0.05) | 0.02 | (0.01,0.04) | |
| South End | Winship | | | 0.02 | (0.00,0.04) | 0.01 | (0.00,0.03) | |
| South End | Winthrop | | | 0.01 | (0.00,0.03) | 0.01 | (0.00,0.02) | |
| West Roxbury | BTU | 0.01 | (0.00,0.01) | 0.03 | (0.01,0.06) | 0.03 | (0.01,0.05) | 0.04 |
| West Roxbury | Bates | | | 0.02 | (0.01,0.04) | 0.02 | (0.01,0.04) | 0.02 |
| West Roxbury | Beethoven | 0.10 | (0.08,0.13) | 0.23 | (0.18,0.28) | 0.23 | (0.18,0.28) | 0.25 |
| West Roxbury | Channing | | | 0.01 | (0.00,0.03) | 0.02 | (0.00,0.03) | |
| West Roxbury | Conley | | | 0.01 | (0.00,0.03) | 0.01 | (0.00,0.03) | |
| West Roxbury | Curley | 0.01 | (0.00,0.01) | 0.01 | (0.00,0.03) | 0.01 | (0.00,0.03) | 0.01 |
| West Roxbury | Ellis | 0.01 | (0.00,0.01) | 0.00 | (0.00,0.01) | 0.00 | (0.00,0.01) | |
| West Roxbury | Grew | | | 0.01 | (0.00,0.02) | 0.01 | (0.00,0.02) | |
| West Roxbury | Hale | 0.01 | (0.00,0.02) | | | 0.00 | (0.00,0.01) | 0.01 |
| West Roxbury | Haley | | | 0.01 | (0.00,0.02) | 0.01 | (0.00,0.02) | |
| West Roxbury | Haynes | | | | | 0.00 | (0.00,0.01) | |
| West Roxbury | Hennigan | | | 0.00 | (0.00,0.01) | 0.01 | (0.00,0.02) | |
| West Roxbury | Hernandez | | | 0.01 | (0.00,0.02) | 0.01 | (0.00,0.02) | |
| West Roxbury | Higginson/Lewis | 0.01 | (0.01,0.02) | 0.00 | (0.00,0.01) | 0.00 | (0.00,0.01) | |
| West Roxbury | J.F. Kennedy | | | 0.00 | (0.00,0.01) | 0.00 | (0.00,0.01) | |
| West Roxbury | Kilmer | 0.32 | (0.28,0.37) | 0.25 | (0.20,0.30) | 0.28 | (0.23,0.33) | 0.24 |
| West Roxbury | King | 0.01 | (0.00,0.01) | | | | | |
| West Roxbury | Lyndon | 0.30 | (0.25,0.35) | 0.22 | (0.17,0.26) | 0.20 | (0.16,0.25) | 0.20 |
| West Roxbury | Manning | 0.01 | (0.00,0.03) | 0.02 | (0.00,0.04) | 0.01 | (0.00,0.03) | 0.01 |
| West Roxbury | Mattahunt | 0.01 | (0.00,0.02) | | | | | |
| West Roxbury | Mendell | | | 0.00 | (0.00,0.01) | 0.00 | (0.00,0.01) | |
| West Roxbury | Mission Hill | | | 0.01 | (0.00,0.03) | 0.01 | (0.00,0.02) | 0.02 |
| West Roxbury | Mozart | 0.05 | (0.03,0.06) | 0.07 | (0.05,0.10) | 0.06 | (0.04,0.09) | 0.05 |
| West Roxbury | Philbrick | | | 0.01 | (0.00,0.02) | 0.01 | (0.00,0.02) | |
| West Roxbury | Quincy | 0.01 | (0.00,0.02) | | | | | |
| West Roxbury | Sumner | 0.07 | (0.04,0.10) | 0.02 | (0.01,0.04) | 0.02 | (0.01,0.04) | 0.02 |
| West Roxbury | Taylor | 0.01 | (0.00,0.02) | | | | | |
| West Roxbury | Trotter | 0.02 | (0.01,0.03) | 0.00 | (0.00,0.01) | 0.00 | (0.00,0.01) | 0.02 |
| West Roxbury | West Zone ELC | 0.02 | (0.01,0.02) | 0.01 | (0.00,0.03) | 0.02 | (0.00,0.03) | 0.02 |

Table 2: Top 2 Choices Market Share Predictions for 2013 K2

| Neighborhood | School | Naive mean | Naive (95% C.I.) | Logit mean | Logit (95% C.I.) | Mixed Logit mean | Mixed Logit (95% C.I.) | Actual |
|---|---|---|---|---|---|---|---|---|
| Allston-Brighton | Baldwin | 0.08 | (0.06,0.10) | 0.16 | (0.13,0.19) | 0.16 | (0.12,0.19) | 0.17 |
| Allston-Brighton | Blackstone | 0.01 | (0.00,0.02) | 0.01 | (0.00,0.02) | 0.01 | (0.00,0.02) | 0.01 |
| Allston-Brighton | Bradley | 0.00 | (0.00,0.01) | | | 0.00 | (0.00,0.01) | |
| Allston-Brighton | East Boston EEC | | | | | 0.01 | (0.00,0.02) | |
| Allston-Brighton | Edison | 0.04 | (0.03,0.06) | 0.09 | (0.07,0.12) | 0.08 | (0.06,0.11) | 0.13 |
| Allston-Brighton | Eliot | 0.01 | (0.00,0.01) | 0.02 | (0.01,0.04) | 0.02 | (0.01,0.03) | 0.02 |
| Allston-Brighton | Gardner | 0.06 | (0.04,0.08) | 0.15 | (0.12,0.18) | 0.15 | (0.12,0.19) | 0.19 |
| Allston-Brighton | Harvard/Kent | 0.02 | (0.01,0.04) | 0.01 | (0.00,0.02) | 0.01 | (0.00,0.02) | 0.01 |

Continued on next page

**Table 2 – continued from previous page**

| Neighborhood | School | Naive mean | Naive (95% C.I.) | Logit mean | Logit (95% C.I.) | Mixed Logit mean | Mixed Logit (95% C.I.) | Actual |
|---|---|---|---|---|---|---|---|---|
| Allston-Brighton | Hernandez | | | 0.01 | (0.00,0.02) | 0.01 | (0.00,0.02) | |
| Allston-Brighton | Hurley | 0.14 | (0.10,0.18) | 0.01 | (0.00,0.02) | 0.01 | (0.00,0.02) | |
| Allston-Brighton | Jackson/Mann | 0.14 | (0.11,0.17) | 0.15 | (0.11,0.18) | 0.13 | (0.10,0.16) | 0.14 |
| Allston-Brighton | Kennedy Patrick | | | | | 0.00 | (0.00,0.01) | |
| Allston-Brighton | Kenny | 0.00 | (0.00,0.01) | | | | | |
| Allston-Brighton | Kilmer | 0.00 | (0.00,0.01) | | | | | |
| Allston-Brighton | Lyon K-8 | 0.23 | (0.21,0.26) | 0.14 | (0.10,0.18) | 0.17 | (0.13,0.20) | 0.11 |
| Allston-Brighton | Mario Umana | | | | | 0.00 | (0.00,0.01) | |
| Allston-Brighton | Mason | 0.01 | (0.00,0.01) | 0.01 | (0.00,0.01) | 0.00 | (0.00,0.01) | |
| Allston-Brighton | McKay | | | | | 0.00 | (0.00,0.01) | |
| Allston-Brighton | O'Donnell | | | | | 0.00 | (0.00,0.01) | |
| Allston-Brighton | Orchard Gardens | 0.04 | (0.02,0.06) | 0.01 | (0.00,0.02) | 0.01 | (0.00,0.02) | |
| Allston-Brighton | Otis | 0.05 | (0.04,0.07) | | | | | |
| Allston-Brighton | Perkins | 0.00 | (0.00,0.01) | | | | | |
| Allston-Brighton | Quincy | 0.05 | (0.03,0.07) | 0.02 | (0.01,0.04) | 0.02 | (0.01,0.04) | 0.05 |
| Allston-Brighton | Tobin | | | 0.01 | (0.00,0.02) | 0.01 | (0.00,0.02) | |
| Allston-Brighton | Warren/Prescott | | | 0.01 | (0.00,0.03) | 0.01 | (0.00,0.03) | |
| Allston-Brighton | Winship | 0.08 | (0.06,0.10) | 0.17 | (0.13,0.20) | 0.15 | (0.12,0.18) | 0.14 |
| Allston-Brighton | Winthrop | 0.01 | (0.00,0.01) | 0.00 | (0.00,0.01) | | | |
| Charlestown | Adams | | | 0.00 | (0.00,0.01) | 0.00 | (0.00,0.01) | |
| Charlestown | Baldwin | 0.01 | (0.00,0.01) | 0.01 | (0.00,0.03) | 0.02 | (0.00,0.04) | |
| Charlestown | Blackstone | | | 0.02 | (0.00,0.03) | 0.02 | (0.00,0.04) | |
| Charlestown | Bradley | | | 0.01 | (0.00,0.02) | 0.01 | (0.00,0.02) | |
| Charlestown | East Boston EEC | | | 0.02 | (0.00,0.04) | 0.02 | (0.01,0.04) | |
| Charlestown | Edison | | | 0.01 | (0.00,0.02) | 0.01 | (0.00,0.02) | |
| Charlestown | Eliot | 0.01 | (0.00,0.02) | 0.23 | (0.18,0.29) | 0.23 | (0.18,0.28) | 0.22 |
| Charlestown | Gardner | | | 0.02 | (0.01,0.04) | 0.02 | (0.00,0.03) | |
| Charlestown | Guild | | | 0.01 | (0.00,0.02) | 0.00 | (0.00,0.01) | |
| Charlestown | Harvard/Kent | 0.41 | (0.38,0.44) | 0.18 | (0.14,0.22) | 0.19 | (0.14,0.23) | 0.29 |
| Charlestown | Hernandez | | | 0.01 | (0.00,0.02) | 0.01 | (0.00,0.02) | |
| Charlestown | Holland | 0.00 | (0.00,0.01) | | | | | |
| Charlestown | Hurley | 0.06 | (0.04,0.09) | 0.03 | (0.01,0.04) | 0.03 | (0.01,0.04) | 0.03 |
| Charlestown | Jackson/Mann | 0.02 | (0.00,0.03) | 0.01 | (0.00,0.03) | 0.01 | (0.00,0.02) | |
| Charlestown | Kennedy Patrick | | | 0.02 | (0.00,0.03) | 0.01 | (0.00,0.03) | |
| Charlestown | Lyon K-8 | | | 0.01 | (0.00,0.02) | 0.01 | (0.00,0.02) | |
| Charlestown | Mario Umana | | | 0.01 | (0.00,0.03) | 0.01 | (0.00,0.03) | |
| Charlestown | Mason | 0.02 | (0.00,0.04) | 0.01 | (0.00,0.02) | 0.01 | (0.00,0.02) | |
| Charlestown | Mather | 0.00 | (0.00,0.01) | | | | | |
| Charlestown | McKay | | | 0.01 | (0.00,0.03) | 0.01 | (0.00,0.03) | |
| Charlestown | O'Donnell | | | 0.02 | (0.01,0.04) | 0.02 | (0.00,0.03) | |
| Charlestown | Orchard Gardens | 0.03 | (0.01,0.05) | 0.01 | (0.00,0.03) | 0.01 | (0.00,0.03) | |
| Charlestown | Otis | 0.02 | (0.00,0.04) | 0.01 | (0.00,0.03) | 0.01 | (0.00,0.02) | |
| Charlestown | Quincy | 0.02 | (0.00,0.04) | 0.05 | (0.03,0.08) | 0.05 | (0.03,0.08) | 0.03 |
| Charlestown | Tobin | | | 0.01 | (0.00,0.02) | 0.01 | (0.00,0.02) | |
| Charlestown | Warren/Prescott | 0.37 | (0.34,0.41) | 0.26 | (0.22,0.30) | 0.29 | (0.25,0.33) | 0.37 |
| Charlestown | Winship | 0.01 | (0.00,0.01) | 0.01 | (0.00,0.02) | 0.01 | (0.00,0.02) | |
| Downtown | Baldwin | | | 0.03 | (0.01,0.05) | 0.03 | (0.01,0.05) | |
| Downtown | Blackstone | 0.01 | (0.00,0.03) | 0.03 | (0.02,0.06) | 0.04 | (0.02,0.06) | 0.01 |
| Downtown | Bradley | | | 0.00 | (0.00,0.01) | 0.00 | (0.00,0.01) | |
| Downtown | Condon | | | 0.02 | (0.00,0.03) | 0.02 | (0.00,0.04) | |
| Downtown | East Boston EEC | | | 0.01 | (0.00,0.02) | 0.01 | (0.00,0.03) | |
| Downtown | Edison | | | 0.01 | (0.00,0.03) | 0.01 | (0.00,0.02) | 0.02 |
| Downtown | Eliot | 0.29 | (0.23,0.35) | 0.24 | (0.19,0.30) | 0.24 | (0.19,0.30) | 0.37 |
| Downtown | Gardner | 0.01 | (0.00,0.02) | 0.02 | (0.01,0.04) | 0.02 | (0.00,0.04) | |
| Downtown | Hale | 0.01 | (0.00,0.02) | | | | | |

Continued on next page

Table 2 – continued from previous page

| Neighborhood | School | Naive mean | Naive (95% C.I.) | Logit mean | Logit (95% C.I.) | Mixed Logit mean | Mixed Logit (95% C.I.) | Actual |
|---|---|---|---|---|---|---|---|---|
| Downtown | Harvard/Kent | 0.11 | (0.08,0.14) | 0.07 | (0.05,0.10) | 0.07 | (0.05,0.10) | 0.13 |
| Downtown | Hennigan | | | 0.00 | (0.00,0.01) | 0.00 | (0.00,0.01) | |
| Downtown | Hernandez | | | 0.02 | (0.00,0.03) | 0.01 | (0.00,0.03) | |
| Downtown | Hurley | 0.13 | (0.10,0.17) | 0.05 | (0.02,0.07) | 0.05 | (0.03,0.08) | 0.06 |
| Downtown | Jackson/Mann | 0.03 | (0.01,0.05) | 0.02 | (0.01,0.04) | 0.02 | (0.00,0.03) | 0.03 |
| Downtown | Kennedy Patrick | 0.00 | (0.00,0.01) | 0.00 | (0.00,0.02) | 0.00 | (0.00,0.01) | |
| Downtown | Lyon K-8 | | | 0.02 | (0.00,0.04) | 0.02 | (0.00,0.03) | |
| Downtown | Mario Umana | | | 0.00 | (0.00,0.01) | 0.00 | (0.00,0.01) | |
| Downtown | Mason | 0.01 | (0.00,0.02) | 0.02 | (0.01,0.04) | 0.02 | (0.00,0.04) | 0.01 |
| Downtown | McKay | | | 0.00 | (0.00,0.01) | 0.00 | (0.00,0.01) | |
| Downtown | Mission Hill | | | | | 0.01 | | |
| Downtown | O'Donnell | | | 0.00 | (0.00,0.01) | 0.00 | (0.00,0.01) | |
| Downtown | Orchard Gardens | 0.04 | (0.02,0.07) | 0.03 | (0.01,0.06) | 0.03 | (0.01,0.05) | 0.01 |
| Downtown | Otis | 0.02 | (0.00,0.03) | 0.00 | (0.00,0.01) | 0.00 | (0.00,0.01) | |
| Downtown | Quincy | 0.28 | (0.22,0.33) | 0.26 | (0.21,0.31) | 0.26 | (0.20,0.31) | 0.26 |
| Downtown | Russell | 0.00 | (0.00,0.01) | | | | | |
| Downtown | Tobin | | | 0.02 | (0.01,0.04) | 0.02 | (0.01,0.04) | |
| Downtown | Warren/Prescott | 0.00 | (0.00,0.01) | 0.06 | (0.03,0.10) | 0.07 | (0.04,0.10) | 0.04 |
| Downtown | West Zone ELC | | | 0.00 | (0.00,0.01) | 0.00 | (0.00,0.01) | |
| Downtown | Winship | 0.01 | (0.00,0.01) | 0.02 | (0.01,0.04) | 0.02 | (0.01,0.03) | |
| Downtown | Winthrop | 0.02 | (0.00,0.03) | 0.01 | (0.00,0.02) | 0.01 | (0.00,0.02) | |
| East Boston | Adams | 0.06 | (0.05,0.08) | 0.07 | (0.05,0.09) | 0.07 | (0.06,0.08) | 0.08 |
| East Boston | Baldwin | | | | | 0.01 | (0.00,0.01) | |
| East Boston | Blackstone | 0.03 | (0.02,0.04) | 0.01 | (0.01,0.02) | 0.01 | (0.01,0.02) | 0.01 |
| East Boston | Bradley | 0.09 | (0.08,0.10) | 0.05 | (0.04,0.07) | 0.06 | (0.05,0.07) | 0.07 |
| East Boston | East Boston EEC | 0.05 | (0.04,0.07) | 0.13 | (0.11,0.16) | 0.13 | (0.11,0.16) | 0.12 |
| East Boston | Edison | | | | | 0.01 | (0.00,0.01) | |
| East Boston | Eliot | 0.01 | (0.01,0.01) | 0.02 | (0.01,0.03) | 0.02 | (0.01,0.02) | 0.02 |
| East Boston | Gardner | | | 0.01 | (0.01,0.02) | 0.02 | (0.01,0.03) | |
| East Boston | Guild | 0.02 | (0.01,0.04) | 0.06 | (0.04,0.08) | 0.05 | (0.04,0.07) | 0.06 |
| East Boston | Harvard/Kent | 0.02 | (0.01,0.03) | 0.01 | (0.01,0.02) | 0.01 | (0.01,0.02) | 0.02 |
| East Boston | Hernandez | | | | | 0.01 | (0.00,0.02) | |
| East Boston | Hurley | 0.18 | (0.16,0.20) | 0.01 | (0.00,0.01) | 0.01 | (0.01,0.02) | |
| East Boston | Jackson/Mann | 0.03 | (0.02,0.04) | | | | | |
| East Boston | Kennedy Patrick | 0.20 | (0.18,0.22) | 0.16 | (0.14,0.20) | 0.15 | (0.13,0.17) | 0.14 |
| East Boston | Lyon K-8 | | | | | 0.01 | (0.00,0.01) | |
| East Boston | Mario Umana | 0.02 | (0.01,0.03) | 0.04 | (0.03,0.06) | 0.06 | (0.04,0.07) | 0.03 |
| East Boston | McKay | 0.04 | (0.03,0.06) | 0.15 | (0.13,0.17) | 0.14 | (0.12,0.16) | 0.13 |
| East Boston | O'Donnell | 0.04 | (0.03,0.05) | 0.14 | (0.12,0.17) | 0.11 | (0.10,0.13) | 0.12 |
| East Boston | Orchard Gardens | 0.01 | (0.01,0.02) | 0.01 | (0.00,0.01) | 0.01 | (0.00,0.01) | |
| East Boston | Otis | 0.16 | (0.14,0.17) | 0.08 | (0.06,0.10) | 0.08 | (0.06,0.10) | 0.14 |
| East Boston | Quincy | 0.01 | (0.00,0.01) | | | 0.00 | (0.00,0.01) | 0.01 |
| East Boston | Tobin | | | | | 0.01 | (0.00,0.01) | |
| East Boston | Warren/Prescott | | | 0.01 | (0.00,0.02) | 0.01 | (0.01,0.02) | |
| East Boston | Winship | | | | | 0.01 | (0.00,0.01) | |
| East Boston | Winthrop | 0.01 | (0.00,0.01) | | | | | |
| Hyde Park | BTU | | | 0.01 | (0.00,0.01) | 0.01 | (0.00,0.02) | |
| Hyde Park | Bates | | | 0.01 | (0.00,0.02) | 0.01 | (0.00,0.02) | 0.02 |
| Hyde Park | Beethoven | 0.02 | (0.01,0.02) | 0.06 | (0.04,0.08) | 0.05 | (0.04,0.07) | 0.04 |
| Hyde Park | Channing | 0.03 | (0.02,0.04) | 0.09 | (0.07,0.12) | 0.09 | (0.07,0.12) | 0.06 |
| Hyde Park | Chittick | 0.04 | (0.03,0.05) | 0.05 | (0.03,0.07) | 0.05 | (0.03,0.06) | 0.07 |
| Hyde Park | Clap | | | 0.01 | (0.00,0.01) | 0.00 | (0.00,0.01) | |
| Hyde Park | Condon | 0.01 | (0.00,0.02) | 0.01 | (0.00,0.01) | 0.01 | (0.00,0.01) | |
| Hyde Park | Conley | 0.12 | (0.09,0.14) | 0.03 | (0.01,0.04) | 0.03 | (0.02,0.05) | 0.02 |
| Hyde Park | Dever | 0.01 | (0.00,0.01) | 0.01 | (0.00,0.02) | 0.01 | (0.00,0.02) | |

Continued on next page

**Table 2 – continued from previous page**

| Neighborhood | School | Naive mean | Naive (95% C.I.) | Logit mean | Logit (95% C.I.) | Mixed Logit mean | Mixed Logit (95% C.I.) | Actual |
|---|---|---|---|---|---|---|---|---|
| Hyde Park | E Greenwood | 0.02 | (0.01,0.04) | 0.09 | (0.06,0.13) | 0.09 | (0.06,0.11) | 0.09 |
| Hyde Park | Ellis | 0.01 | (0.00,0.01) | | | | | |
| Hyde Park | Ellison/Parks | 0.01 | (0.00,0.01) | 0.05 | (0.04,0.08) | 0.05 | (0.03,0.07) | 0.05 |
| Hyde Park | Everett | | | 0.01 | (0.00,0.01) | 0.01 | (0.00,0.01) | |
| Hyde Park | Grew | 0.01 | (0.00,0.01) | 0.07 | (0.04,0.09) | 0.07 | (0.05,0.10) | 0.08 |
| Hyde Park | Haley | 0.00 | (0.00,0.01) | 0.01 | (0.00,0.02) | 0.01 | (0.00,0.02) | |
| Hyde Park | Henderson | 0.15 | (0.13,0.18) | 0.01 | (0.00,0.02) | 0.01 | (0.00,0.03) | |
| Hyde Park | Hernandez | 0.01 | (0.00,0.01) | 0.02 | (0.01,0.04) | 0.02 | (0.01,0.03) | 0.02 |
| Hyde Park | Holland | | | 0.01 | (0.00,0.02) | 0.01 | (0.00,0.02) | |
| Hyde Park | Holmes | | | 0.01 | (0.00,0.01) | 0.01 | (0.00,0.01) | |
| Hyde Park | Kenny | 0.02 | (0.01,0.03) | 0.01 | (0.00,0.02) | 0.01 | (0.00,0.02) | |
| Hyde Park | Kilmer | 0.01 | (0.00,0.02) | 0.01 | (0.00,0.02) | 0.01 | (0.00,0.02) | 0.02 |
| Hyde Park | Lyndon | 0.01 | (0.00,0.02) | 0.01 | (0.00,0.02) | 0.01 | (0.00,0.02) | |
| Hyde Park | Mather | 0.01 | (0.00,0.01) | 0.01 | (0.00,0.02) | 0.01 | (0.00,0.02) | |
| Hyde Park | Mattahunt | 0.03 | (0.01,0.04) | 0.03 | (0.02,0.04) | 0.03 | (0.02,0.04) | 0.04 |
| Hyde Park | Mozart | | | 0.01 | (0.00,0.02) | 0.01 | (0.00,0.01) | |
| Hyde Park | Murphy | 0.02 | (0.01,0.04) | 0.03 | (0.01,0.04) | 0.03 | (0.01,0.05) | 0.03 |
| Hyde Park | Perry | | | 0.01 | (0.00,0.02) | 0.01 | (0.00,0.02) | 0.01 |
| Hyde Park | Philbrick | 0.03 | (0.02,0.05) | 0.01 | (0.00,0.02) | 0.01 | (0.00,0.01) | |
| Hyde Park | Roosevelt | 0.27 | (0.24,0.29) | 0.20 | (0.17,0.23) | 0.20 | (0.17,0.24) | 0.23 |
| Hyde Park | Russell | 0.02 | (0.01,0.04) | 0.01 | (0.00,0.02) | 0.01 | (0.00,0.02) | |
| Hyde Park | S. Greenwood | 0.05 | (0.03,0.06) | 0.02 | (0.01,0.03) | 0.02 | (0.01,0.03) | 0.02 |
| Hyde Park | Sumner | 0.03 | (0.01,0.04) | 0.01 | (0.00,0.02) | 0.01 | (0.00,0.02) | 0.01 |
| Hyde Park | Taylor | 0.04 | (0.03,0.06) | 0.02 | (0.01,0.03) | 0.02 | (0.01,0.03) | 0.02 |
| Hyde Park | Young Achievers | 0.01 | (0.00,0.01) | 0.06 | (0.04,0.08) | 0.06 | (0.04,0.08) | 0.06 |
| Jamaica Plain | BTU | 0.02 | (0.01,0.02) | 0.07 | (0.05,0.09) | 0.06 | (0.04,0.08) | 0.08 |
| Jamaica Plain | Baldwin | | | 0.01 | (0.01,0.02) | 0.01 | (0.01,0.02) | 0.02 |
| Jamaica Plain | Bates | | | 0.01 | (0.00,0.02) | 0.01 | (0.00,0.01) | |
| Jamaica Plain | Beethoven | 0.02 | (0.01,0.03) | 0.03 | (0.01,0.04) | 0.03 | (0.01,0.04) | 0.01 |
| Jamaica Plain | Blackstone | | | 0.01 | (0.01,0.02) | 0.01 | (0.00,0.02) | |
| Jamaica Plain | Conley | | | 0.01 | (0.00,0.01) | 0.00 | (0.00,0.01) | |
| Jamaica Plain | Curley | 0.05 | (0.04,0.06) | 0.11 | (0.09,0.14) | 0.12 | (0.10,0.14) | 0.16 |
| Jamaica Plain | East Boston EEC | | | | | 0.00 | (0.00,0.01) | |
| Jamaica Plain | Edison | | | 0.01 | (0.00,0.02) | 0.01 | (0.00,0.01) | |
| Jamaica Plain | Eliot | | | 0.01 | (0.00,0.02) | 0.01 | (0.00,0.02) | |
| Jamaica Plain | Ellis | 0.01 | (0.01,0.01) | 0.01 | (0.01,0.03) | 0.01 | (0.01,0.02) | |
| Jamaica Plain | Gardner | | | 0.01 | (0.00,0.02) | 0.01 | (0.00,0.02) | |
| Jamaica Plain | Hale | 0.23 | (0.21,0.26) | 0.02 | (0.01,0.04) | 0.02 | (0.01,0.03) | 0.01 |
| Jamaica Plain | Haley | 0.01 | (0.01,0.01) | 0.02 | (0.01,0.04) | 0.02 | (0.01,0.03) | 0.02 |
| Jamaica Plain | Harvard/Kent | 0.02 | (0.01,0.03) | 0.01 | (0.00,0.02) | 0.01 | (0.00,0.02) | 0.02 |
| Jamaica Plain | Haynes | | | 0.01 | (0.00,0.02) | 0.01 | (0.00,0.02) | 0.02 |
| Jamaica Plain | Hennigan | 0.03 | (0.01,0.05) | 0.06 | (0.04,0.09) | 0.06 | (0.04,0.09) | 0.07 |
| Jamaica Plain | Hernandez | 0.02 | (0.02,0.03) | 0.05 | (0.03,0.07) | 0.06 | (0.04,0.08) | 0.05 |
| Jamaica Plain | Higginson/Lewis | 0.01 | (0.01,0.01) | 0.01 | (0.00,0.02) | 0.01 | (0.00,0.02) | 0.01 |
| Jamaica Plain | Hurley | 0.04 | (0.03,0.05) | 0.01 | (0.01,0.03) | 0.02 | (0.01,0.03) | |
| Jamaica Plain | J.F. Kennedy | 0.04 | (0.03,0.06) | 0.06 | (0.04,0.08) | 0.05 | (0.04,0.07) | 0.07 |
| Jamaica Plain | Jackson/Mann | 0.01 | (0.00,0.03) | 0.01 | (0.00,0.02) | 0.01 | (0.00,0.02) | |
| Jamaica Plain | Kilmer | 0.01 | (0.00,0.01) | 0.02 | (0.01,0.04) | 0.03 | (0.02,0.05) | 0.02 |
| Jamaica Plain | Lyndon | 0.02 | (0.01,0.04) | 0.03 | (0.01,0.04) | 0.02 | (0.01,0.04) | |
| Jamaica Plain | Lyon K-8 | | | 0.01 | (0.00,0.02) | 0.01 | (0.00,0.02) | |
| Jamaica Plain | Manning | 0.17 | (0.15,0.20) | 0.04 | (0.02,0.06) | 0.04 | (0.03,0.06) | 0.05 |
| Jamaica Plain | Mason | 0.01 | (0.00,0.02) | 0.01 | (0.00,0.02) | 0.01 | (0.00,0.02) | |
| Jamaica Plain | Mendell | 0.03 | (0.03,0.04) | 0.05 | (0.04,0.07) | 0.05 | (0.03,0.07) | 0.04 |
| Jamaica Plain | Mission Hill | 0.01 | (0.01,0.02) | 0.05 | (0.03,0.08) | 0.05 | (0.03,0.07) | 0.11 |
| Jamaica Plain | Mozart | | | 0.01 | (0.01,0.02) | 0.01 | (0.00,0.02) | |

Continued on next page

**Table 2 – continued from previous page**

| Neighborhood | School | Naive mean | Naive (95% C.I.) | Logit mean | Logit (95% C.I.) | Mixed Logit mean | Mixed Logit (95% C.I.) | Actual |
|---|---|---|---|---|---|---|---|---|
| Jamaica Plain | Orchard Gardens | 0.03 | (0.02,0.03) | 0.02 | (0.01,0.04) | 0.02 | (0.01,0.03) | 0.01 |
| Jamaica Plain | Philbrick | 0.03 | (0.02,0.05) | 0.01 | (0.00,0.02) | 0.01 | (0.00,0.02) | 0.02 |
| Jamaica Plain | Quincy | 0.02 | (0.01,0.03) | 0.02 | (0.01,0.03) | 0.02 | (0.01,0.03) | 0.03 |
| Jamaica Plain | Sumner | 0.05 | (0.03,0.07) | 0.01 | (0.01,0.03) | 0.01 | (0.00,0.02) | 0.01 |
| Jamaica Plain | Tobin | 0.00 | (0.00,0.01) | 0.03 | (0.02,0.05) | 0.03 | (0.02,0.05) | 0.02 |
| Jamaica Plain | Trotter | | | 0.01 | (0.00,0.02) | 0.01 | (0.00,0.02) | 0.01 |
| Jamaica Plain | Warren/Prescott | | | 0.00 | (0.00,0.01) | 0.00 | (0.00,0.01) | |
| Jamaica Plain | West Zone ELC | 0.02 | (0.02,0.02) | 0.06 | (0.04,0.09) | 0.07 | (0.05,0.10) | 0.05 |
| Jamaica Plain | Winship | | | 0.01 | (0.00,0.02) | 0.01 | (0.00,0.01) | |
| Jamaica Plain | Winthrop | 0.01 | (0.00,0.01) | 0.01 | (0.00,0.01) | 0.01 | (0.00,0.01) | |
| Mattapan | BTU | | | 0.01 | (0.00,0.01) | 0.01 | (0.00,0.01) | |
| Mattapan | Beethoven | | | 0.00 | (0.00,0.01) | | | |
| Mattapan | Channing | 0.01 | (0.00,0.01) | 0.02 | (0.01,0.04) | 0.02 | (0.01,0.03) | 0.03 |
| Mattapan | Chittick | 0.02 | (0.01,0.03) | 0.03 | (0.02,0.05) | 0.03 | (0.02,0.05) | 0.04 |
| Mattapan | Clap | 0.01 | (0.00,0.02) | 0.02 | (0.01,0.03) | 0.01 | (0.01,0.02) | 0.03 |
| Mattapan | Condon | 0.01 | (0.00,0.02) | 0.01 | (0.00,0.02) | 0.01 | (0.00,0.02) | 0.02 |
| Mattapan | Curley | | | 0.01 | (0.00,0.01) | | | |
| Mattapan | Dever | 0.01 | (0.00,0.02) | 0.02 | (0.01,0.04) | 0.02 | (0.01,0.04) | 0.03 |
| Mattapan | E Greenwood | | | 0.04 | (0.02,0.06) | 0.03 | (0.02,0.04) | 0.04 |
| Mattapan | Ellison/Parks | 0.02 | (0.01,0.03) | 0.09 | (0.07,0.12) | 0.10 | (0.08,0.12) | 0.12 |
| Mattapan | Everett | | | 0.02 | (0.01,0.03) | 0.01 | (0.01,0.03) | 0.01 |
| Mattapan | Grew | | | 0.02 | (0.01,0.03) | 0.01 | (0.01,0.03) | |
| Mattapan | Haley | | | 0.03 | (0.02,0.05) | 0.03 | (0.02,0.05) | 0.02 |
| Mattapan | Henderson | 0.30 | (0.28,0.33) | 0.02 | (0.01,0.03) | 0.03 | (0.01,0.04) | 0.02 |
| Mattapan | Hernandez | 0.02 | (0.02,0.03) | 0.05 | (0.03,0.06) | 0.04 | (0.03,0.06) | 0.05 |
| Mattapan | Holland | 0.02 | (0.01,0.03) | 0.03 | (0.02,0.04) | 0.03 | (0.02,0.04) | 0.05 |
| Mattapan | Holmes | 0.01 | (0.00,0.01) | 0.02 | (0.01,0.03) | 0.02 | (0.01,0.03) | 0.02 |
| Mattapan | J.F. Kennedy | 0.01 | (0.00,0.02) | 0.00 | (0.00,0.01) | | | |
| Mattapan | Kenny | 0.02 | (0.01,0.03) | 0.03 | (0.01,0.04) | 0.03 | (0.01,0.04) | 0.01 |
| Mattapan | Lyndon | 0.01 | (0.00,0.02) | 0.01 | (0.00,0.01) | 0.01 | (0.00,0.01) | |
| Mattapan | Mather | 0.02 | (0.01,0.02) | 0.02 | (0.01,0.04) | 0.02 | (0.01,0.03) | 0.02 |
| Mattapan | Mattahunt | 0.02 | (0.01,0.04) | 0.04 | (0.02,0.05) | 0.03 | (0.02,0.05) | 0.06 |
| Mattapan | Murphy | 0.15 | (0.12,0.18) | 0.05 | (0.03,0.07) | 0.06 | (0.04,0.08) | 0.06 |
| Mattapan | Orchard Gardens | 0.01 | (0.00,0.01) | | | | | |
| Mattapan | Perkins | | | 0.01 | (0.00,0.01) | 0.01 | (0.00,0.01) | |
| Mattapan | Perry | | | 0.01 | (0.00,0.02) | 0.01 | (0.00,0.03) | |
| Mattapan | Philbrick | 0.05 | (0.04,0.07) | 0.00 | (0.00,0.01) | 0.00 | (0.00,0.01) | |
| Mattapan | Quincy | 0.00 | (0.00,0.01) | | | | | |
| Mattapan | Roosevelt | 0.02 | (0.01,0.04) | 0.05 | (0.03,0.07) | 0.05 | (0.03,0.06) | 0.04 |
| Mattapan | Russell | 0.04 | (0.02,0.05) | 0.02 | (0.01,0.04) | 0.02 | (0.01,0.04) | 0.02 |
| Mattapan | S. Greenwood | 0.05 | (0.04,0.07) | 0.06 | (0.04,0.08) | 0.06 | (0.04,0.08) | 0.06 |
| Mattapan | Sumner | 0.02 | (0.01,0.03) | 0.01 | (0.00,0.01) | 0.01 | (0.00,0.01) | |
| Mattapan | Taylor | 0.06 | (0.04,0.07) | 0.05 | (0.03,0.07) | 0.05 | (0.03,0.06) | 0.07 |
| Mattapan | Trotter | | | 0.01 | (0.00,0.01) | 0.01 | (0.00,0.01) | |
| Mattapan | Tynan | | | 0.01 | (0.00,0.01) | 0.00 | (0.00,0.01) | |
| Mattapan | West Zone ELC | | | 0.00 | (0.00,0.01) | 0.00 | (0.00,0.01) | |
| Mattapan | Winthrop | 0.01 | (0.00,0.01) | | | | | |
| Mattapan | Young Achievers | 0.03 | (0.02,0.04) | 0.16 | (0.12,0.19) | 0.18 | (0.15,0.21) | 0.12 |
| North Dorchester | Baldwin | | | 0.00 | (0.00,0.01) | | | |
| North Dorchester | Bates | 0.00 | (0.00,0.01) | | | | | |
| North Dorchester | Blackstone | 0.01 | (0.00,0.01) | 0.01 | (0.00,0.02) | 0.01 | (0.00,0.02) | |
| North Dorchester | Channing | | | 0.01 | (0.00,0.01) | 0.01 | (0.00,0.02) | |
| North Dorchester | Chittick | | | 0.00 | (0.00,0.01) | | | |
| North Dorchester | Clap | 0.02 | (0.01,0.02) | 0.06 | (0.04,0.08) | 0.06 | (0.04,0.08) | 0.07 |
| North Dorchester | Condon | 0.04 | (0.02,0.06) | 0.04 | (0.03,0.06) | 0.04 | (0.02,0.06) | 0.03 |

Continued on next page

**Table 2 – continued from previous page**

| | | Naive | | Logit | | Mixed Logit | | |
|---|---|---|---|---|---|---|---|---|
| Neighborhood | School | mean | (95% C.I.) | mean | (95% C.I.) | mean | (95% C.I.) | Actual |
| North Dorchester | Dever | 0.04 | (0.02,0.06) | 0.07 | (0.05,0.10) | 0.08 | (0.05,0.10) | 0.03 |
| North Dorchester | E Greenwood | | | 0.01 | (0.00,0.02) | 0.01 | (0.00,0.02) | |
| North Dorchester | East Boston EEC | | | | | 0.00 | (0.00,0.01) | |
| North Dorchester | Eliot | 0.01 | (0.00,0.02) | 0.01 | (0.00,0.02) | 0.01 | (0.00,0.01) | |
| North Dorchester | Ellison/Parks | | | 0.01 | (0.00,0.03) | 0.01 | (0.00,0.03) | |
| North Dorchester | Everett | 0.01 | (0.00,0.02) | 0.07 | (0.04,0.09) | 0.07 | (0.04,0.10) | 0.11 |
| North Dorchester | Gardner | | | 0.00 | (0.00,0.01) | | | |
| North Dorchester | Grew | | | 0.00 | (0.00,0.01) | 0.01 | (0.00,0.01) | |
| North Dorchester | Harvard/Kent | 0.01 | (0.00,0.01) | | | | | |
| North Dorchester | Haynes | 0.01 | (0.00,0.01) | 0.04 | (0.02,0.06) | 0.04 | (0.02,0.06) | 0.03 |
| North Dorchester | Henderson | 0.09 | (0.07,0.12) | 0.02 | (0.01,0.04) | 0.02 | (0.01,0.04) | 0.02 |
| North Dorchester | Hernandez | | | 0.03 | (0.01,0.04) | 0.02 | (0.01,0.04) | |
| North Dorchester | Holland | 0.04 | (0.02,0.06) | 0.05 | (0.03,0.07) | 0.04 | (0.03,0.07) | 0.05 |
| North Dorchester | Holmes | | | 0.01 | (0.00,0.02) | 0.01 | (0.00,0.02) | |
| North Dorchester | Hurley | 0.00 | (0.00,0.01) | 0.01 | (0.00,0.02) | 0.01 | (0.00,0.02) | |
| North Dorchester | Jackson/Mann | 0.01 | (0.00,0.02) | 0.01 | (0.00,0.01) | 0.00 | (0.00,0.01) | |
| North Dorchester | Kenny | | | 0.01 | (0.00,0.02) | 0.01 | (0.00,0.02) | |
| North Dorchester | King | | | 0.01 | (0.00,0.02) | 0.01 | (0.00,0.02) | 0.01 |
| North Dorchester | Lyon K-8 | | | | | 0.01 | | |
| North Dorchester | Mason | 0.31 | (0.24,0.38) | 0.05 | (0.03,0.07) | 0.05 | (0.03,0.07) | 0.04 |
| North Dorchester | Mather | 0.06 | (0.04,0.08) | 0.08 | (0.05,0.10) | 0.08 | (0.06,0.11) | 0.12 |
| North Dorchester | Mattahunt | 0.01 | (0.00,0.02) | 0.00 | (0.00,0.01) | 0.00 | (0.00,0.01) | |
| North Dorchester | Murphy | 0.13 | (0.10,0.16) | 0.08 | (0.05,0.11) | 0.10 | (0.07,0.13) | 0.15 |
| North Dorchester | Orchard Gardens | 0.06 | (0.04,0.08) | 0.03 | (0.01,0.05) | 0.03 | (0.01,0.05) | 0.02 |
| North Dorchester | Otis | 0.01 | (0.00,0.03) | | | | | |
| North Dorchester | Perkins | | | 0.02 | (0.00,0.03) | 0.01 | (0.00,0.03) | |
| North Dorchester | Perry | | | 0.03 | (0.02,0.06) | 0.03 | (0.02,0.05) | 0.03 |
| North Dorchester | Quincy | 0.02 | (0.00,0.03) | 0.01 | (0.00,0.03) | 0.01 | (0.00,0.03) | |
| North Dorchester | Roosevelt | 0.01 | (0.00,0.02) | 0.01 | (0.00,0.02) | 0.02 | (0.01,0.03) | 0.01 |
| North Dorchester | Russell | 0.05 | (0.03,0.07) | 0.09 | (0.06,0.11) | 0.09 | (0.07,0.12) | 0.09 |
| North Dorchester | S. Greenwood | 0.01 | (0.00,0.03) | 0.01 | (0.00,0.03) | 0.01 | (0.00,0.03) | 0.01 |
| North Dorchester | Taylor | | | 0.01 | (0.00,0.01) | 0.00 | (0.00,0.01) | |
| North Dorchester | Tobin | | | 0.00 | (0.00,0.01) | | | |
| North Dorchester | Trotter | | | 0.00 | (0.00,0.01) | 0.00 | (0.00,0.01) | 0.01 |
| North Dorchester | Tynan | 0.00 | (0.00,0.01) | 0.01 | (0.00,0.03) | 0.01 | (0.00,0.03) | 0.01 |
| North Dorchester | Winthrop | 0.02 | (0.01,0.03) | 0.03 | (0.02,0.05) | 0.03 | (0.01,0.05) | 0.02 |
| North Dorchester | Young Achievers | 0.01 | (0.00,0.02) | 0.02 | (0.01,0.04) | 0.02 | (0.01,0.04) | 0.02 |
| Roslindale | BTU | 0.02 | (0.01,0.02) | 0.09 | (0.07,0.12) | 0.10 | (0.07,0.12) | 0.07 |
| Roslindale | Bates | 0.01 | (0.00,0.01) | 0.05 | (0.04,0.07) | 0.06 | (0.04,0.07) | 0.06 |
| Roslindale | Beethoven | 0.05 | (0.04,0.06) | 0.11 | (0.09,0.14) | 0.11 | (0.08,0.14) | 0.09 |
| Roslindale | Conley | 0.14 | (0.12,0.16) | 0.04 | (0.02,0.06) | 0.03 | (0.02,0.05) | 0.06 |
| Roslindale | Curley | 0.02 | (0.01,0.03) | 0.04 | (0.02,0.05) | 0.03 | (0.02,0.05) | 0.03 |
| Roslindale | E Greenwood | 0.00 | (0.00,0.01) | 0.02 | (0.01,0.03) | 0.01 | (0.01,0.03) | |
| Roslindale | Ellis | 0.02 | (0.01,0.03) | 0.01 | (0.00,0.02) | 0.01 | (0.00,0.02) | |
| Roslindale | Grew | | | 0.01 | (0.00,0.01) | 0.01 | (0.00,0.01) | |
| Roslindale | Hale | 0.01 | (0.00,0.01) | 0.01 | (0.00,0.01) | 0.00 | (0.00,0.01) | |
| Roslindale | Haley | 0.02 | (0.01,0.03) | 0.05 | (0.04,0.07) | 0.05 | (0.04,0.07) | 0.09 |
| Roslindale | Haynes | | | 0.01 | (0.00,0.01) | 0.01 | (0.00,0.02) | 0.01 |
| Roslindale | Hennigan | 0.01 | (0.00,0.02) | 0.02 | (0.01,0.03) | 0.01 | (0.01,0.03) | 0.02 |
| Roslindale | Hernandez | 0.02 | (0.01,0.03) | 0.03 | (0.02,0.05) | 0.03 | (0.02,0.05) | 0.04 |
| Roslindale | Higginson/Lewis | 0.01 | (0.00,0.01) | | | | | |
| Roslindale | J.F. Kennedy | 0.01 | (0.01,0.02) | 0.01 | (0.01,0.03) | 0.01 | (0.00,0.02) | |
| Roslindale | Kenny | 0.01 | (0.00,0.02) | | | | | |
| Roslindale | Kilmer | 0.01 | (0.01,0.02) | 0.07 | (0.05,0.09) | 0.08 | (0.06,0.10) | 0.08 |
| Roslindale | Lyndon | 0.07 | (0.06,0.09) | 0.10 | (0.08,0.13) | 0.09 | (0.07,0.11) | 0.09 |

Continued on next page

**Table 2 – continued from previous page**

| Neighborhood | School | Naive mean | Naive (95% C.I.) | Logit mean | Logit (95% C.I.) | Mixed Logit mean | Mixed Logit (95% C.I.) | Actual |
|---|---|---|---|---|---|---|---|---|
| Roslindale | Manning | 0.01 | (0.00,0.02) | 0.03 | (0.01,0.04) | 0.03 | (0.01,0.04) | 0.03 |
| Roslindale | Mattahunt | | | 0.01 | (0.00,0.01) | 0.01 | (0.00,0.01) | |
| Roslindale | Mendell | 0.01 | (0.01,0.01) | 0.02 | (0.01,0.03) | 0.01 | (0.01,0.02) | 0.01 |
| Roslindale | Mission Hill | | | 0.03 | (0.01,0.04) | 0.02 | (0.01,0.04) | 0.04 |
| Roslindale | Mozart | 0.02 | (0.02,0.03) | 0.07 | (0.06,0.09) | 0.07 | (0.06,0.10) | 0.05 |
| Roslindale | Philbrick | 0.13 | (0.11,0.16) | 0.03 | (0.01,0.05) | 0.03 | (0.01,0.04) | 0.04 |
| Roslindale | Roosevelt | 0.01 | (0.00,0.01) | 0.01 | (0.00,0.01) | 0.01 | (0.00,0.01) | 0.01 |
| Roslindale | Sumner | 0.32 | (0.29,0.34) | 0.09 | (0.07,0.11) | 0.10 | (0.08,0.12) | 0.09 |
| Roslindale | Taylor | 0.02 | (0.01,0.03) | 0.01 | (0.00,0.01) | 0.01 | (0.00,0.01) | |
| Roslindale | Trotter | 0.01 | (0.01,0.02) | 0.01 | (0.00,0.01) | 0.01 | (0.00,0.01) | |
| Roslindale | West Zone ELC | 0.01 | (0.01,0.01) | 0.02 | (0.01,0.03) | 0.02 | (0.01,0.03) | 0.02 |
| Roslindale | Young Achievers | | | 0.01 | (0.00,0.01) | 0.01 | (0.00,0.01) | |
| Roxbury | BTU | | | 0.03 | (0.02,0.04) | 0.03 | (0.02,0.04) | 0.02 |
| Roxbury | Baldwin | | | 0.01 | (0.00,0.01) | 0.01 | (0.00,0.01) | |
| Roxbury | Bates | | | 0.01 | (0.00,0.01) | 0.01 | (0.00,0.01) | |
| Roxbury | Beethoven | 0.03 | (0.02,0.04) | 0.02 | (0.01,0.03) | 0.02 | (0.01,0.03) | 0.02 |
| Roxbury | Blackstone | 0.01 | (0.01,0.01) | 0.02 | (0.01,0.02) | 0.02 | (0.01,0.02) | 0.02 |
| Roxbury | Clap | | | 0.01 | (0.00,0.01) | 0.01 | (0.00,0.01) | |
| Roxbury | Conley | | | 0.01 | (0.00,0.01) | | | |
| Roxbury | Curley | 0.03 | (0.02,0.03) | 0.05 | (0.04,0.06) | 0.05 | (0.04,0.06) | 0.04 |
| Roxbury | Dever | 0.01 | (0.00,0.01) | 0.01 | (0.00,0.01) | 0.01 | (0.00,0.01) | |
| Roxbury | Eliot | | | 0.01 | (0.00,0.02) | 0.01 | (0.00,0.01) | |
| Roxbury | Ellis | 0.04 | (0.03,0.05) | 0.04 | (0.03,0.05) | 0.04 | (0.03,0.05) | 0.05 |
| Roxbury | Everett | | | 0.01 | (0.01,0.02) | 0.01 | (0.01,0.02) | |
| Roxbury | Gardner | | | 0.01 | (0.00,0.01) | 0.01 | (0.00,0.01) | |
| Roxbury | Hale | 0.18 | (0.17,0.19) | 0.03 | (0.02,0.04) | 0.03 | (0.02,0.04) | 0.03 |
| Roxbury | Haley | | | 0.01 | (0.01,0.02) | 0.01 | (0.01,0.02) | |
| Roxbury | Haynes | 0.01 | (0.01,0.01) | 0.04 | (0.03,0.06) | 0.05 | (0.04,0.06) | 0.06 |
| Roxbury | Henderson | 0.04 | (0.03,0.05) | | | | | |
| Roxbury | Hennigan | 0.02 | (0.01,0.03) | 0.03 | (0.02,0.05) | 0.03 | (0.02,0.04) | 0.04 |
| Roxbury | Hernandez | 0.01 | (0.01,0.02) | 0.06 | (0.04,0.07) | 0.07 | (0.05,0.08) | 0.06 |
| Roxbury | Higginson/Lewis | 0.01 | (0.01,0.01) | 0.02 | (0.01,0.03) | 0.02 | (0.01,0.03) | 0.03 |
| Roxbury | Holland | 0.01 | (0.01,0.01) | 0.03 | (0.02,0.04) | 0.03 | (0.02,0.04) | 0.03 |
| Roxbury | Holmes | | | 0.01 | (0.00,0.01) | 0.01 | (0.00,0.01) | |
| Roxbury | Hurley | 0.04 | (0.03,0.05) | 0.02 | (0.01,0.03) | 0.02 | (0.01,0.03) | 0.01 |
| Roxbury | J.F. Kennedy | 0.02 | (0.01,0.03) | 0.03 | (0.02,0.05) | 0.03 | (0.02,0.04) | 0.02 |
| Roxbury | Jackson/Mann | 0.01 | (0.01,0.02) | 0.01 | (0.00,0.01) | | | |
| Roxbury | Kilmer | | | 0.01 | (0.00,0.01) | 0.01 | (0.01,0.02) | |
| Roxbury | King | 0.02 | (0.01,0.02) | 0.02 | (0.01,0.03) | 0.02 | (0.01,0.03) | 0.05 |
| Roxbury | Lyndon | 0.02 | (0.01,0.03) | 0.02 | (0.01,0.03) | 0.02 | (0.01,0.02) | 0.02 |
| Roxbury | Manning | 0.03 | (0.02,0.04) | 0.01 | (0.00,0.01) | 0.01 | (0.00,0.01) | |
| Roxbury | Mason | 0.14 | (0.12,0.16) | 0.03 | (0.02,0.04) | 0.03 | (0.02,0.04) | 0.03 |
| Roxbury | Mather | | | 0.01 | (0.01,0.02) | 0.01 | (0.01,0.02) | 0.01 |
| Roxbury | Mendell | 0.01 | (0.01,0.01) | 0.02 | (0.01,0.03) | 0.02 | (0.01,0.03) | 0.02 |
| Roxbury | Mission Hill | | | 0.02 | (0.01,0.03) | 0.02 | (0.01,0.03) | 0.03 |
| Roxbury | Mozart | | | 0.01 | (0.00,0.01) | 0.01 | (0.00,0.01) | |
| Roxbury | Murphy | 0.02 | (0.02,0.03) | 0.01 | (0.00,0.01) | 0.01 | (0.00,0.01) | |
| Roxbury | Orchard Gardens | 0.05 | (0.04,0.06) | 0.05 | (0.04,0.07) | 0.05 | (0.04,0.06) | 0.06 |
| Roxbury | Otis | 0.01 | (0.01,0.02) | | | | | |
| Roxbury | Philbrick | 0.03 | (0.02,0.04) | 0.01 | (0.00,0.01) | | | |
| Roxbury | Quincy | | | 0.01 | (0.00,0.01) | 0.01 | (0.00,0.01) | 0.01 |
| Roxbury | Russell | 0.01 | (0.00,0.01) | 0.02 | (0.01,0.03) | 0.02 | (0.01,0.03) | 0.01 |
| Roxbury | S. Greenwood | 0.01 | (0.01,0.02) | 0.02 | (0.02,0.03) | 0.03 | (0.02,0.04) | 0.03 |
| Roxbury | Sumner | 0.04 | (0.03,0.05) | 0.01 | (0.01,0.02) | 0.01 | (0.01,0.02) | 0.01 |
| Roxbury | Tobin | | | 0.02 | (0.01,0.03) | 0.02 | (0.01,0.02) | 0.02 |

Continued on next page

Table 2 – continued from previous page

| Neighborhood | School | Naive mean | Naive (95% C.I.) | Logit mean | Logit (95% C.I.) | Mixed Logit mean | Mixed Logit (95% C.I.) | Actual |
|---|---|---|---|---|---|---|---|---|
| Roxbury | Trotter | 0.03 | (0.02,0.04) | 0.04 | (0.03,0.06) | 0.04 | (0.03,0.05) | 0.05 |
| Roxbury | West Zone ELC | | | 0.03 | (0.02,0.04) | 0.04 | (0.03,0.05) | 0.02 |
| Roxbury | Winthrop | 0.02 | (0.02,0.03) | 0.04 | (0.03,0.04) | 0.03 | (0.03,0.04) | 0.05 |
| Roxbury | Young Achievers | | | 0.01 | (0.01,0.02) | 0.01 | (0.01,0.02) | 0.01 |
| South Boston | Blackstone | 0.01 | (0.00,0.02) | 0.02 | (0.01,0.04) | 0.02 | (0.01,0.04) | 0.01 |
| South Boston | Channing | | | 0.00 | (0.00,0.01) | 0.01 | (0.00,0.01) | |
| South Boston | Chittick | | | 0.00 | (0.00,0.01) | 0.00 | (0.00,0.01) | |
| South Boston | Clap | | | 0.04 | (0.02,0.06) | 0.04 | (0.02,0.07) | 0.04 |
| South Boston | Condon | 0.17 | (0.13,0.20) | 0.19 | (0.15,0.23) | 0.18 | (0.14,0.22) | 0.29 |
| South Boston | Dever | 0.02 | (0.01,0.03) | 0.08 | (0.05,0.12) | 0.09 | (0.05,0.12) | 0.05 |
| South Boston | E Greenwood | | | 0.01 | (0.00,0.02) | 0.01 | (0.00,0.02) | |
| South Boston | Eliot | | | | | 0.01 | | |
| South Boston | Ellison/Parks | | | 0.01 | (0.00,0.02) | 0.01 | (0.00,0.02) | |
| South Boston | Everett | | | 0.03 | (0.01,0.05) | 0.02 | (0.01,0.04) | |
| South Boston | Grew | | | | | 0.00 | (0.00,0.01) | |
| South Boston | Harvard/Kent | 0.02 | (0.01,0.03) | 0.01 | (0.00,0.01) | 0.01 | (0.00,0.01) | 0.02 |
| South Boston | Henderson | 0.11 | (0.07,0.14) | 0.02 | (0.00,0.03) | 0.01 | (0.00,0.03) | 0.03 |
| South Boston | Hernandez | | | 0.03 | (0.01,0.05) | 0.02 | (0.01,0.04) | 0.01 |
| South Boston | Holland | 0.01 | (0.00,0.02) | 0.02 | (0.01,0.04) | 0.02 | (0.01,0.04) | 0.01 |
| South Boston | Holmes | | | 0.00 | (0.00,0.01) | 0.00 | (0.00,0.01) | |
| South Boston | Kenny | 0.00 | (0.00,0.01) | 0.01 | (0.00,0.02) | 0.01 | (0.00,0.02) | |
| South Boston | Mason | 0.12 | (0.08,0.17) | 0.02 | (0.01,0.04) | 0.02 | (0.01,0.04) | |
| South Boston | Mather | | | 0.02 | (0.00,0.03) | 0.02 | (0.00,0.03) | |
| South Boston | Mattahunt | | | 0.00 | (0.00,0.01) | | | |
| South Boston | Murphy | 0.18 | (0.15,0.22) | 0.06 | (0.03,0.09) | 0.06 | (0.03,0.09) | 0.07 |
| South Boston | Orchard Gardens | 0.01 | (0.00,0.02) | 0.01 | (0.00,0.01) | 0.01 | (0.00,0.01) | |
| South Boston | Perkins | 0.02 | (0.00,0.03) | 0.04 | (0.02,0.07) | 0.05 | (0.02,0.07) | 0.07 |
| South Boston | Perry | 0.05 | (0.03,0.06) | 0.16 | (0.13,0.20) | 0.17 | (0.13,0.21) | 0.18 |
| South Boston | Quincy | 0.09 | (0.06,0.12) | 0.05 | (0.02,0.07) | 0.05 | (0.02,0.07) | 0.03 |
| South Boston | Roosevelt | | | 0.01 | (0.00,0.01) | 0.01 | (0.00,0.03) | |
| South Boston | Russell | 0.06 | (0.03,0.09) | 0.05 | (0.03,0.07) | 0.04 | (0.02,0.07) | 0.02 |
| South Boston | S. Greenwood | 0.08 | (0.05,0.11) | 0.02 | (0.01,0.04) | 0.02 | (0.01,0.04) | |
| South Boston | Taylor | 0.00 | (0.00,0.01) | 0.00 | (0.00,0.01) | 0.00 | (0.00,0.01) | |
| South Boston | Tynan | 0.01 | (0.00,0.03) | 0.07 | (0.04,0.10) | 0.07 | (0.04,0.10) | 0.07 |
| South Boston | Young Achievers | 0.00 | (0.00,0.01) | 0.03 | (0.01,0.05) | 0.03 | (0.01,0.05) | 0.01 |
| South Dorchester | Channing | | | 0.01 | (0.01,0.02) | 0.01 | (0.01,0.02) | 0.01 |
| South Dorchester | Chittick | 0.01 | (0.00,0.01) | 0.01 | (0.00,0.02) | 0.01 | (0.00,0.01) | |
| South Dorchester | Clap | | | 0.02 | (0.01,0.03) | 0.02 | (0.01,0.03) | 0.01 |
| South Dorchester | Condon | 0.03 | (0.02,0.04) | 0.03 | (0.02,0.04) | 0.02 | (0.01,0.03) | 0.03 |
| South Dorchester | Dever | 0.02 | (0.01,0.03) | 0.04 | (0.03,0.05) | 0.04 | (0.03,0.05) | 0.02 |
| South Dorchester | E Greenwood | 0.01 | (0.00,0.01) | 0.02 | (0.01,0.03) | 0.01 | (0.01,0.02) | |
| South Dorchester | Ellison/Parks | 0.01 | (0.00,0.01) | 0.03 | (0.02,0.04) | 0.03 | (0.02,0.04) | 0.05 |
| South Dorchester | Everett | | | 0.04 | (0.03,0.05) | 0.03 | (0.02,0.04) | 0.04 |
| South Dorchester | Grew | | | 0.01 | (0.00,0.01) | 0.01 | (0.00,0.01) | |
| South Dorchester | Haynes | | | 0.01 | (0.01,0.02) | 0.01 | (0.01,0.02) | |
| South Dorchester | Henderson | 0.30 | (0.28,0.32) | 0.06 | (0.05,0.08) | 0.07 | (0.06,0.09) | 0.10 |
| South Dorchester | Hernandez | | | 0.03 | (0.02,0.04) | 0.03 | (0.02,0.04) | 0.03 |
| South Dorchester | Holland | 0.07 | (0.06,0.08) | 0.07 | (0.05,0.09) | 0.07 | (0.06,0.08) | 0.07 |
| South Dorchester | Holmes | 0.02 | (0.01,0.02) | 0.03 | (0.02,0.04) | 0.03 | (0.02,0.04) | 0.04 |
| South Dorchester | Kenny | 0.03 | (0.03,0.04) | 0.06 | (0.04,0.07) | 0.06 | (0.05,0.08) | 0.04 |
| South Dorchester | King | 0.01 | (0.01,0.01) | 0.01 | (0.01,0.02) | 0.01 | (0.01,0.02) | 0.01 |
| South Dorchester | Mather | 0.08 | (0.07,0.09) | 0.08 | (0.06,0.10) | 0.08 | (0.06,0.09) | 0.09 |
| South Dorchester | Mattahunt | | | 0.01 | (0.00,0.02) | 0.01 | (0.00,0.01) | 0.01 |
| South Dorchester | Murphy | 0.24 | (0.21,0.26) | 0.18 | (0.15,0.20) | 0.20 | (0.18,0.22) | 0.21 |
| South Dorchester | Orchard Gardens | 0.02 | (0.01,0.03) | 0.01 | (0.00,0.01) | 0.01 | (0.00,0.01) | |

Continued on next page

**Table 2 – continued from previous page**

| Neighborhood | School | Naive mean | Naive (95% C.I.) | Logit mean | Logit (95% C.I.) | Mixed Logit mean | Mixed Logit (95% C.I.) | Actual |
|---|---|---|---|---|---|---|---|---|
| South Dorchester | Perkins | | | 0.01 | (0.00,0.02) | 0.01 | (0.00,0.01) | 0.01 |
| South Dorchester | Perry | 0.01 | (0.00,0.01) | 0.03 | (0.02,0.04) | 0.03 | (0.02,0.04) | 0.01 |
| South Dorchester | Roosevelt | | | 0.02 | (0.01,0.03) | 0.02 | (0.01,0.03) | 0.01 |
| South Dorchester | Russell | 0.04 | (0.03,0.05) | 0.03 | (0.02,0.04) | 0.03 | (0.02,0.04) | 0.03 |
| South Dorchester | S. Greenwood | 0.05 | (0.04,0.06) | 0.05 | (0.04,0.07) | 0.05 | (0.04,0.07) | 0.05 |
| South Dorchester | Taylor | 0.01 | (0.01,0.02) | 0.02 | (0.01,0.03) | 0.02 | (0.01,0.03) | 0.01 |
| South Dorchester | Tynan | 0.01 | (0.00,0.01) | 0.01 | (0.00,0.02) | 0.01 | (0.00,0.01) | |
| South Dorchester | Winthrop | | | 0.01 | (0.00,0.01) | 0.01 | (0.00,0.01) | |
| South Dorchester | Young Achievers | 0.01 | (0.01,0.01) | 0.06 | (0.04,0.07) | 0.06 | (0.05,0.08) | 0.06 |
| South End | Baldwin | | | 0.03 | (0.01,0.04) | 0.03 | (0.01,0.04) | 0.01 |
| South End | Blackstone | 0.06 | (0.04,0.08) | 0.10 | (0.08,0.13) | 0.11 | (0.08,0.14) | 0.16 |
| South End | Bradley | | | | | 0.00 | (0.00,0.01) | |
| South End | Condon | | | 0.02 | (0.01,0.03) | 0.02 | (0.01,0.04) | |
| South End | Curley | 0.01 | (0.00,0.02) | | | | | |
| South End | East Boston EEC | | | 0.01 | (0.00,0.02) | 0.02 | (0.01,0.03) | 0.01 |
| South End | Edison | 0.02 | (0.01,0.03) | 0.02 | (0.01,0.03) | 0.01 | (0.01,0.03) | 0.01 |
| South End | Eliot | 0.02 | (0.01,0.02) | 0.09 | (0.06,0.12) | 0.08 | (0.06,0.11) | 0.08 |
| South End | Gardner | 0.01 | (0.00,0.02) | 0.03 | (0.02,0.05) | 0.03 | (0.01,0.04) | 0.01 |
| South End | Guild | | | | | 0.00 | (0.00,0.01) | |
| South End | Hale | 0.03 | (0.02,0.05) | 0.01 | (0.00,0.02) | 0.01 | (0.00,0.02) | |
| South End | Harvard/Kent | 0.06 | (0.04,0.08) | 0.04 | (0.03,0.06) | 0.04 | (0.02,0.05) | 0.05 |
| South End | Hernandez | 0.02 | (0.01,0.03) | 0.04 | (0.03,0.06) | 0.04 | (0.02,0.06) | 0.03 |
| South End | Higginson/Lewis | | | 0.01 | (0.00,0.01) | 0.01 | (0.00,0.01) | |
| South End | Hurley | 0.35 | (0.32,0.38) | 0.13 | (0.10,0.17) | 0.14 | (0.11,0.18) | 0.19 |
| South End | J.F. Kennedy | 0.01 | (0.00,0.02) | | | | | |
| South End | Jackson/Mann | 0.04 | (0.02,0.06) | 0.02 | (0.01,0.04) | 0.02 | (0.01,0.03) | |
| South End | Kennedy Patrick | | | 0.01 | (0.00,0.01) | 0.01 | (0.00,0.01) | |
| South End | Lyon K-8 | | | 0.02 | (0.00,0.03) | 0.01 | (0.00,0.03) | 0.01 |
| South End | Mario Umana | | | 0.01 | (0.00,0.01) | 0.01 | (0.00,0.01) | |
| South End | Mason | 0.03 | (0.02,0.05) | 0.04 | (0.02,0.07) | 0.04 | (0.03,0.07) | 0.01 |
| South End | Mather | 0.01 | (0.00,0.01) | | | | | |
| South End | McKay | | | 0.01 | (0.00,0.01) | 0.01 | (0.00,0.02) | |
| South End | Mission Hill | 0.01 | (0.00,0.01) | | | 0.02 | | |
| South End | O'Donnell | | | 0.01 | (0.00,0.01) | 0.01 | (0.00,0.01) | |
| South End | Orchard Gardens | 0.07 | (0.05,0.08) | 0.09 | (0.06,0.12) | 0.08 | (0.06,0.11) | 0.10 |
| South End | Otis | 0.03 | (0.02,0.04) | 0.00 | (0.00,0.01) | 0.00 | (0.00,0.01) | |
| South End | Quincy | 0.19 | (0.16,0.23) | 0.15 | (0.12,0.18) | 0.16 | (0.13,0.20) | 0.22 |
| South End | S. Greenwood | 0.00 | (0.00,0.01) | | | | | |
| South End | Tobin | 0.01 | (0.00,0.01) | 0.03 | (0.02,0.06) | 0.03 | (0.02,0.05) | 0.02 |
| South End | Warren/Prescott | | | 0.03 | (0.01,0.05) | 0.03 | (0.01,0.05) | |
| South End | Winship | 0.01 | (0.00,0.01) | 0.02 | (0.01,0.03) | 0.01 | (0.00,0.03) | |
| South End | Winthrop | | | 0.01 | (0.00,0.02) | 0.01 | (0.00,0.02) | |
| West Roxbury | BTU | | | 0.04 | (0.02,0.06) | 0.03 | (0.02,0.05) | 0.03 |
| West Roxbury | Bates | | | 0.03 | (0.02,0.05) | 0.03 | (0.02,0.04) | 0.03 |
| West Roxbury | Beethoven | 0.08 | (0.06,0.09) | 0.22 | (0.18,0.25) | 0.22 | (0.18,0.25) | 0.21 |
| West Roxbury | Channing | | | 0.02 | (0.01,0.03) | 0.02 | (0.01,0.03) | 0.01 |
| West Roxbury | Conley | 0.02 | (0.01,0.03) | 0.02 | (0.01,0.03) | 0.02 | (0.01,0.03) | 0.01 |
| West Roxbury | Curley | 0.01 | (0.00,0.02) | 0.02 | (0.01,0.03) | 0.01 | (0.00,0.03) | 0.02 |
| West Roxbury | Grew | | | 0.01 | (0.00,0.02) | 0.01 | (0.00,0.02) | |
| West Roxbury | Hale | 0.00 | (0.00,0.01) | | | | | |
| West Roxbury | Haley | | | 0.01 | (0.01,0.03) | 0.01 | (0.00,0.02) | 0.01 |
| West Roxbury | Haynes | | | | | 0.01 | (0.00,0.01) | 0.01 |
| West Roxbury | Hennigan | 0.01 | (0.00,0.02) | 0.01 | (0.00,0.01) | 0.01 | (0.00,0.02) | |
| West Roxbury | Hernandez | | | 0.01 | (0.00,0.02) | 0.01 | (0.00,0.02) | |
| West Roxbury | J.F. Kennedy | | | 0.01 | (0.00,0.01) | 0.00 | (0.00,0.01) | |

Continued on next page

**Table 2 – continued from previous page**

| Neighborhood | School | Naive mean | Naive (95% C.I.) | Logit mean | Logit (95% C.I.) | Mixed Logit mean | Mixed Logit (95% C.I.) | Actual |
|---|---|---|---|---|---|---|---|---|
| West Roxbury | Kenny | 0.01 | (0.00,0.01) | | | | | |
| West Roxbury | Kilmer | 0.31 | (0.29,0.34) | 0.23 | (0.20,0.26) | 0.25 | (0.22,0.28) | 0.26 |
| West Roxbury | King | 0.01 | (0.00,0.01) | | | | | |
| West Roxbury | Lyndon | 0.35 | (0.33,0.38) | 0.20 | (0.17,0.23) | 0.20 | (0.17,0.23) | 0.21 |
| West Roxbury | Manning | 0.02 | (0.01,0.03) | 0.02 | (0.01,0.04) | 0.02 | (0.01,0.04) | 0.02 |
| West Roxbury | Mendell | | | 0.01 | (0.00,0.01) | | | |
| West Roxbury | Mission Hill | | | 0.01 | (0.00,0.03) | 0.01 | (0.00,0.02) | 0.01 |
| West Roxbury | Mozart | 0.02 | (0.02,0.03) | 0.07 | (0.05,0.09) | 0.06 | (0.04,0.08) | 0.04 |
| West Roxbury | Philbrick | | | 0.01 | (0.00,0.02) | 0.01 | (0.00,0.02) | 0.02 |
| West Roxbury | Quincy | 0.01 | (0.01,0.02) | | | | | |
| West Roxbury | Sumner | 0.07 | (0.05,0.09) | 0.02 | (0.01,0.04) | 0.02 | (0.01,0.04) | 0.01 |
| West Roxbury | Taylor | 0.01 | (0.00,0.01) | | | | | |
| West Roxbury | Trotter | 0.01 | (0.01,0.02) | 0.00 | (0.00,0.01) | 0.00 | (0.00,0.01) | 0.01 |
| West Roxbury | West Zone ELC | 0.01 | (0.00,0.01) | 0.01 | (0.00,0.02) | 0.02 | (0.01,0.03) | 0.02 |

Table 3: Top 3 Choices Market Share Predictions for 2013 K2

| Neighborhood | School | Naive mean | Naive (95% C.I.) | Logit mean | Logit (95% C.I.) | Mixed Logit mean | Mixed Logit (95% C.I.) | Actual |
|---|---|---|---|---|---|---|---|---|
| Allston-Brighton | Baldwin | 0.05 | (0.04,0.06) | 0.14 | (0.12,0.16) | 0.14 | (0.11,0.16) | 0.16 |
| Allston-Brighton | Blackstone | 0.01 | (0.00,0.02) | 0.01 | (0.00,0.02) | 0.01 | (0.00,0.02) | 0.01 |
| Allston-Brighton | East Boston EEC | | | | | 0.01 | (0.00,0.02) | |
| Allston-Brighton | Edison | 0.05 | (0.04,0.06) | 0.10 | (0.08,0.12) | 0.09 | (0.07,0.12) | 0.13 |
| Allston-Brighton | Eliot | 0.01 | (0.00,0.01) | 0.03 | (0.01,0.04) | 0.02 | (0.01,0.04) | 0.02 |
| Allston-Brighton | Gardner | 0.04 | (0.03,0.05) | 0.14 | (0.12,0.17) | 0.14 | (0.12,0.17) | 0.18 |
| Allston-Brighton | Harvard/Kent | 0.03 | (0.02,0.04) | 0.01 | (0.00,0.02) | 0.01 | (0.00,0.02) | 0.01 |
| Allston-Brighton | Hernandez | | | 0.01 | (0.00,0.02) | 0.01 | (0.00,0.02) | |
| Allston-Brighton | Hurley | 0.19 | (0.17,0.21) | 0.01 | (0.01,0.03) | 0.01 | (0.00,0.02) | |
| Allston-Brighton | Jackson/Mann | 0.14 | (0.11,0.17) | 0.15 | (0.12,0.18) | 0.14 | (0.12,0.17) | 0.15 |
| Allston-Brighton | Kennedy Patrick | 0.02 | (0.01,0.03) | | | | | |
| Allston-Brighton | Lyon K-8 | 0.18 | (0.16,0.20) | 0.14 | (0.11,0.17) | 0.15 | (0.13,0.18) | 0.11 |
| Allston-Brighton | Mason | 0.04 | (0.02,0.06) | 0.01 | (0.00,0.01) | 0.01 | (0.00,0.01) | |
| Allston-Brighton | McKay | | | | | 0.00 | (0.00,0.01) | |
| Allston-Brighton | Orchard Gardens | 0.03 | (0.02,0.04) | 0.01 | (0.00,0.02) | 0.01 | (0.00,0.02) | |
| Allston-Brighton | Otis | 0.05 | (0.04,0.07) | | | | | |
| Allston-Brighton | Quincy | 0.08 | (0.06,0.10) | 0.03 | (0.01,0.04) | 0.03 | (0.01,0.04) | 0.04 |
| Allston-Brighton | Tobin | | | 0.01 | (0.00,0.02) | 0.01 | (0.00,0.02) | |
| Allston-Brighton | Warren/Prescott | 0.01 | (0.00,0.01) | 0.02 | (0.01,0.03) | 0.02 | (0.01,0.03) | |
| Allston-Brighton | Winship | 0.05 | (0.04,0.07) | 0.16 | (0.13,0.19) | 0.15 | (0.13,0.18) | 0.16 |
| Charlestown | Adams | | | 0.01 | (0.00,0.01) | 0.00 | (0.00,0.01) | |
| Charlestown | Baldwin | | | 0.02 | (0.01,0.03) | 0.02 | (0.01,0.03) | |
| Charlestown | Blackstone | | | 0.02 | (0.01,0.03) | 0.02 | (0.01,0.03) | 0.02 |
| Charlestown | Bradley | | | 0.01 | (0.00,0.02) | 0.01 | (0.00,0.01) | |
| Charlestown | East Boston EEC | | | 0.02 | (0.01,0.04) | 0.02 | (0.01,0.04) | |
| Charlestown | Edison | 0.01 | (0.00,0.02) | 0.01 | (0.00,0.02) | 0.01 | (0.00,0.01) | |
| Charlestown | Eliot | 0.24 | (0.22,0.27) | 0.25 | (0.21,0.30) | 0.27 | (0.23,0.31) | 0.28 |
| Charlestown | Gardner | | | 0.02 | (0.01,0.04) | 0.02 | (0.01,0.03) | |
| Charlestown | Guild | | | 0.01 | (0.00,0.02) | 0.01 | (0.00,0.01) | |
| Charlestown | Harvard/Kent | 0.28 | (0.27,0.30) | 0.17 | (0.14,0.20) | 0.17 | (0.15,0.20) | 0.26 |
| Charlestown | Hernandez | | | 0.01 | (0.00,0.02) | 0.01 | (0.00,0.02) | |
| Charlestown | Hurley | 0.05 | (0.03,0.07) | 0.03 | (0.01,0.04) | 0.02 | (0.01,0.04) | 0.03 |
| Charlestown | Jackson/Mann | 0.01 | (0.00,0.03) | 0.01 | (0.00,0.02) | 0.01 | (0.00,0.02) | |

Continued on next page

**Table 3 – continued from previous page**

| Neighborhood | School | Naive mean | Naive (95% C.I.) | Logit mean | Logit (95% C.I.) | Mixed Logit mean | Mixed Logit (95% C.I.) | Actual |
|---|---|---|---|---|---|---|---|---|
| Charlestown | Kennedy Patrick | 0.02 | (0.01,0.03) | 0.02 | (0.01,0.03) | 0.01 | (0.00,0.02) | |
| Charlestown | Lyon K-8 | | | 0.01 | (0.00,0.02) | 0.01 | (0.00,0.02) | |
| Charlestown | Mario Umana | | | 0.02 | (0.00,0.03) | 0.01 | (0.00,0.02) | |
| Charlestown | Mason | 0.02 | (0.00,0.04) | 0.01 | (0.00,0.02) | 0.01 | (0.00,0.02) | |
| Charlestown | McKay | | | 0.02 | (0.01,0.03) | 0.01 | (0.00,0.03) | |
| Charlestown | O'Donnell | | | 0.02 | (0.01,0.04) | 0.02 | (0.01,0.03) | |
| Charlestown | Orchard Gardens | 0.04 | (0.02,0.06) | 0.01 | (0.00,0.03) | 0.01 | (0.00,0.02) | |
| Charlestown | Otis | 0.02 | (0.01,0.04) | 0.01 | (0.00,0.03) | 0.01 | (0.00,0.02) | |
| Charlestown | Quincy | 0.02 | (0.01,0.03) | 0.06 | (0.04,0.09) | 0.06 | (0.04,0.09) | 0.03 |
| Charlestown | Tobin | | | 0.01 | (0.00,0.02) | 0.01 | (0.00,0.02) | |
| Charlestown | Warren/Prescott | 0.26 | (0.24,0.28) | 0.21 | (0.19,0.24) | 0.23 | (0.20,0.25) | 0.29 |
| Charlestown | Winship | | | 0.01 | (0.00,0.02) | 0.01 | (0.00,0.02) | |
| Downtown | Baldwin | | | 0.03 | (0.01,0.05) | 0.03 | (0.01,0.04) | 0.01 |
| Downtown | Blackstone | 0.01 | (0.00,0.02) | 0.04 | (0.02,0.05) | 0.04 | (0.02,0.06) | 0.01 |
| Downtown | Bradley | | | 0.00 | (0.00,0.01) | 0.00 | (0.00,0.01) | |
| Downtown | Condon | | | 0.02 | (0.01,0.04) | 0.03 | (0.01,0.04) | 0.01 |
| Downtown | East Boston EEC | | | 0.01 | (0.00,0.02) | 0.01 | (0.00,0.03) | |
| Downtown | Edison | 0.01 | (0.00,0.01) | 0.01 | (0.00,0.03) | 0.01 | (0.00,0.02) | 0.03 |
| Downtown | Eliot | 0.23 | (0.19,0.28) | 0.22 | (0.18,0.27) | 0.23 | (0.19,0.27) | 0.31 |
| Downtown | Gardner | 0.00 | (0.00,0.02) | 0.03 | (0.01,0.04) | 0.02 | (0.01,0.04) | |
| Downtown | Hale | 0.01 | (0.01,0.02) | | | | | |
| Downtown | Harvard/Kent | 0.14 | (0.12,0.17) | 0.08 | (0.06,0.10) | 0.08 | (0.05,0.10) | 0.11 |
| Downtown | Hennigan | | | 0.00 | (0.00,0.01) | 0.00 | (0.00,0.01) | |
| Downtown | Hernandez | | | 0.02 | (0.01,0.03) | 0.02 | (0.01,0.03) | |
| Downtown | Hurley | 0.11 | (0.09,0.13) | 0.05 | (0.03,0.07) | 0.05 | (0.04,0.07) | 0.07 |
| Downtown | Jackson/Mann | 0.03 | (0.01,0.05) | 0.02 | (0.01,0.04) | 0.02 | (0.01,0.03) | 0.07 |
| Downtown | Kennedy Patrick | 0.01 | (0.00,0.03) | 0.01 | (0.00,0.01) | 0.00 | (0.00,0.01) | |
| Downtown | Lyon K-8 | | | 0.02 | (0.01,0.04) | 0.02 | (0.01,0.04) | 0.01 |
| Downtown | Mario Umana | | | 0.01 | (0.00,0.01) | 0.01 | (0.00,0.01) | |
| Downtown | Mason | 0.05 | (0.03,0.07) | 0.02 | (0.01,0.04) | 0.02 | (0.01,0.03) | |
| Downtown | McKay | | | 0.00 | (0.00,0.01) | 0.00 | (0.00,0.01) | |
| Downtown | O'Donnell | | | 0.00 | (0.00,0.01) | 0.00 | (0.00,0.01) | |
| Downtown | Orchard Gardens | 0.03 | (0.02,0.05) | 0.03 | (0.01,0.05) | 0.03 | (0.01,0.05) | 0.01 |
| Downtown | Otis | 0.05 | (0.03,0.07) | 0.00 | (0.00,0.01) | 0.00 | (0.00,0.01) | |
| Downtown | Quincy | 0.25 | (0.23,0.29) | 0.22 | (0.19,0.27) | 0.23 | (0.18,0.26) | 0.25 |
| Downtown | Tobin | | | 0.02 | (0.01,0.04) | 0.02 | (0.01,0.04) | |
| Downtown | Warren/Prescott | 0.01 | (0.01,0.02) | 0.08 | (0.05,0.10) | 0.08 | (0.06,0.10) | 0.05 |
| Downtown | West Zone ELC | | | 0.00 | (0.00,0.01) | 0.00 | (0.00,0.01) | |
| Downtown | Winship | | | 0.02 | (0.01,0.04) | 0.02 | (0.01,0.03) | 0.01 |
| Downtown | Winthrop | 0.01 | (0.00,0.02) | 0.01 | (0.00,0.02) | 0.01 | (0.00,0.02) | |
| East Boston | Adams | 0.04 | (0.04,0.05) | 0.07 | (0.05,0.09) | 0.06 | (0.05,0.07) | 0.08 |
| East Boston | Baldwin | | | | | 0.01 | (0.00,0.01) | |
| East Boston | Blackstone | 0.02 | (0.02,0.03) | 0.01 | (0.01,0.01) | 0.01 | (0.01,0.02) | 0.01 |
| East Boston | Bradley | 0.09 | (0.08,0.10) | 0.05 | (0.04,0.06) | 0.05 | (0.04,0.07) | 0.07 |
| East Boston | East Boston EEC | 0.05 | (0.04,0.05) | 0.14 | (0.12,0.15) | 0.14 | (0.12,0.16) | 0.11 |
| East Boston | Edison | 0.02 | (0.01,0.03) | | | 0.01 | (0.00,0.01) | |
| East Boston | Eliot | 0.01 | (0.00,0.01) | 0.02 | (0.01,0.03) | 0.02 | (0.01,0.03) | 0.02 |
| East Boston | Gardner | | | 0.01 | (0.01,0.02) | 0.02 | (0.01,0.02) | |
| East Boston | Guild | 0.12 | (0.10,0.13) | 0.06 | (0.05,0.08) | 0.05 | (0.04,0.07) | 0.05 |
| East Boston | Harvard/Kent | 0.01 | (0.01,0.02) | 0.01 | (0.01,0.02) | 0.01 | (0.01,0.02) | 0.01 |
| East Boston | Hernandez | | | | | 0.01 | (0.01,0.01) | |
| East Boston | Hurley | 0.18 | (0.17,0.19) | 0.01 | (0.01,0.01) | 0.01 | (0.01,0.02) | |
| East Boston | Jackson/Mann | 0.03 | (0.02,0.03) | | | | | |
| East Boston | Kennedy Patrick | 0.15 | (0.14,0.17) | 0.16 | (0.14,0.19) | 0.14 | (0.12,0.16) | 0.14 |
| East Boston | Mario Umana | 0.02 | (0.01,0.02) | 0.05 | (0.03,0.06) | 0.06 | (0.05,0.07) | 0.04 |

Continued on next page

**Table 3 – continued from previous page**

| Neighborhood | School | Naive mean | Naive (95% C.I.) | Logit mean | Logit (95% C.I.) | Mixed Logit mean | Mixed Logit (95% C.I.) | Actual |
|---|---|---|---|---|---|---|---|---|
| East Boston | McKay | 0.04 | (0.02,0.05) | 0.15 | (0.13,0.17) | 0.14 | (0.12,0.16) | 0.12 |
| East Boston | O'Donnell | 0.03 | (0.02,0.04) | 0.14 | (0.12,0.16) | 0.12 | (0.10,0.13) | 0.12 |
| East Boston | Orchard Gardens | 0.01 | (0.01,0.01) | 0.01 | (0.00,0.01) | 0.01 | (0.01,0.01) | |
| East Boston | Otis | 0.13 | (0.12,0.14) | 0.08 | (0.07,0.10) | 0.08 | (0.07,0.10) | 0.16 |
| East Boston | Quincy | 0.01 | (0.01,0.01) | | | | | |
| East Boston | Tobin | | | | | 0.01 | (0.00,0.01) | |
| East Boston | Warren/Prescott | 0.05 | (0.04,0.06) | 0.01 | (0.01,0.02) | 0.01 | (0.01,0.02) | |
| East Boston | Winship | | | | | 0.01 | (0.00,0.01) | |
| Hyde Park | BTU | | | 0.01 | (0.00,0.01) | 0.01 | (0.00,0.02) | |
| Hyde Park | Bates | | | 0.01 | (0.01,0.02) | 0.01 | (0.00,0.02) | 0.01 |
| Hyde Park | Beethoven | 0.01 | (0.01,0.02) | 0.05 | (0.04,0.07) | 0.05 | (0.03,0.06) | 0.04 |
| Hyde Park | Channing | 0.02 | (0.01,0.03) | 0.09 | (0.07,0.12) | 0.09 | (0.07,0.12) | 0.08 |
| Hyde Park | Chittick | 0.03 | (0.02,0.03) | 0.05 | (0.03,0.06) | 0.04 | (0.03,0.06) | 0.06 |
| Hyde Park | Clap | | | 0.01 | (0.00,0.01) | 0.01 | (0.00,0.01) | |
| Hyde Park | Condon | 0.01 | (0.01,0.02) | 0.01 | (0.00,0.01) | 0.01 | (0.00,0.01) | |
| Hyde Park | Conley | 0.09 | (0.07,0.11) | 0.03 | (0.02,0.04) | 0.03 | (0.02,0.04) | 0.03 |
| Hyde Park | Dever | 0.02 | (0.01,0.03) | 0.01 | (0.00,0.02) | 0.01 | (0.01,0.02) | |
| Hyde Park | E Greenwood | 0.02 | (0.01,0.03) | 0.09 | (0.07,0.13) | 0.09 | (0.07,0.12) | 0.09 |
| Hyde Park | Ellison/Parks | | | 0.06 | (0.04,0.07) | 0.06 | (0.04,0.07) | 0.04 |
| Hyde Park | Everett | | | 0.01 | (0.00,0.02) | 0.01 | (0.00,0.01) | |
| Hyde Park | Grew | 0.00 | (0.00,0.01) | 0.07 | (0.05,0.10) | 0.08 | (0.06,0.10) | 0.09 |
| Hyde Park | Haley | | | 0.01 | (0.00,0.02) | 0.01 | (0.01,0.02) | |
| Hyde Park | Henderson | 0.18 | (0.16,0.20) | 0.01 | (0.01,0.02) | 0.02 | (0.01,0.03) | 0.01 |
| Hyde Park | Hernandez | | | 0.02 | (0.01,0.04) | 0.02 | (0.01,0.03) | 0.03 |
| Hyde Park | Holland | | | 0.01 | (0.00,0.02) | 0.01 | (0.00,0.01) | |
| Hyde Park | Holmes | | | 0.01 | (0.00,0.01) | 0.01 | (0.00,0.01) | |
| Hyde Park | Kenny | 0.02 | (0.01,0.03) | 0.01 | (0.01,0.03) | 0.01 | (0.01,0.02) | |
| Hyde Park | Kilmer | 0.01 | (0.00,0.01) | 0.01 | (0.00,0.01) | 0.01 | (0.00,0.02) | 0.01 |
| Hyde Park | Lyndon | 0.01 | (0.01,0.02) | 0.01 | (0.01,0.02) | 0.01 | (0.00,0.02) | |
| Hyde Park | Mather | | | 0.01 | (0.01,0.02) | 0.01 | (0.00,0.02) | |
| Hyde Park | Mattahunt | 0.03 | (0.02,0.04) | 0.03 | (0.02,0.04) | 0.03 | (0.02,0.04) | 0.03 |
| Hyde Park | Mozart | | | 0.01 | (0.00,0.01) | 0.01 | (0.00,0.01) | |
| Hyde Park | Murphy | 0.12 | (0.10,0.14) | 0.03 | (0.02,0.04) | 0.04 | (0.02,0.05) | 0.03 |
| Hyde Park | Perry | | | 0.01 | (0.00,0.02) | 0.01 | (0.00,0.02) | |
| Hyde Park | Philbrick | 0.04 | (0.02,0.05) | 0.01 | (0.00,0.01) | 0.01 | (0.00,0.01) | |
| Hyde Park | Roosevelt | 0.21 | (0.19,0.22) | 0.16 | (0.14,0.18) | 0.16 | (0.14,0.19) | 0.19 |
| Hyde Park | Russell | 0.02 | (0.01,0.03) | 0.01 | (0.00,0.02) | 0.01 | (0.00,0.01) | |
| Hyde Park | S. Greenwood | 0.03 | (0.02,0.05) | 0.02 | (0.01,0.03) | 0.02 | (0.01,0.03) | 0.02 |
| Hyde Park | Sumner | 0.04 | (0.02,0.05) | 0.01 | (0.00,0.01) | 0.01 | (0.00,0.01) | 0.01 |
| Hyde Park | Taylor | 0.03 | (0.02,0.04) | 0.02 | (0.01,0.03) | 0.01 | (0.01,0.02) | 0.02 |
| Hyde Park | Young Achievers | | | 0.06 | (0.04,0.08) | 0.06 | (0.05,0.08) | 0.07 |
| Jamaica Plain | BTU | 0.01 | (0.01,0.01) | 0.06 | (0.05,0.08) | 0.06 | (0.05,0.07) | 0.08 |
| Jamaica Plain | Baldwin | | | 0.01 | (0.01,0.02) | 0.01 | (0.01,0.02) | 0.01 |
| Jamaica Plain | Bates | | | 0.01 | (0.00,0.02) | 0.01 | (0.00,0.01) | |
| Jamaica Plain | Beethoven | 0.01 | (0.01,0.02) | 0.03 | (0.02,0.04) | 0.03 | (0.02,0.04) | 0.01 |
| Jamaica Plain | Blackstone | | | 0.01 | (0.01,0.02) | 0.01 | (0.00,0.02) | 0.01 |
| Jamaica Plain | Conley | | | 0.01 | (0.00,0.01) | 0.01 | (0.00,0.01) | |
| Jamaica Plain | Curley | 0.04 | (0.04,0.05) | 0.10 | (0.08,0.13) | 0.11 | (0.09,0.13) | 0.15 |
| Jamaica Plain | East Boston EEC | | | | | 0.00 | (0.00,0.01) | |
| Jamaica Plain | Edison | 0.01 | (0.00,0.01) | 0.01 | (0.00,0.01) | 0.01 | (0.00,0.01) | |
| Jamaica Plain | Eliot | | | 0.01 | (0.00,0.02) | 0.01 | (0.00,0.02) | |
| Jamaica Plain | Ellis | | | 0.01 | (0.01,0.02) | 0.01 | (0.01,0.02) | |
| Jamaica Plain | Gardner | | | 0.01 | (0.00,0.02) | 0.01 | (0.00,0.02) | |
| Jamaica Plain | Hale | 0.18 | (0.17,0.20) | 0.02 | (0.01,0.03) | 0.02 | (0.01,0.03) | |
| Jamaica Plain | Haley | | | 0.02 | (0.01,0.03) | 0.02 | (0.01,0.03) | 0.02 |

Continued on next page

**Table 3 – continued from previous page**

| Neighborhood | School | Naive mean | Naive (95% C.I.) | Logit mean | Logit (95% C.I.) | Mixed Logit mean | Mixed Logit (95% C.I.) | Actual |
|---|---|---|---|---|---|---|---|---|
| Jamaica Plain | Harvard/Kent | 0.02 | (0.01,0.03) | 0.01 | (0.00,0.02) | 0.01 | (0.00,0.01) | 0.01 |
| Jamaica Plain | Haynes | | | 0.01 | (0.00,0.02) | 0.01 | (0.01,0.02) | 0.02 |
| Jamaica Plain | Hennigan | 0.03 | (0.01,0.04) | 0.07 | (0.05,0.09) | 0.06 | (0.05,0.09) | 0.07 |
| Jamaica Plain | Hernandez | 0.02 | (0.01,0.02) | 0.05 | (0.04,0.07) | 0.06 | (0.04,0.07) | 0.05 |
| Jamaica Plain | Higginson/Lewis | | | 0.01 | (0.01,0.02) | 0.01 | (0.01,0.02) | |
| Jamaica Plain | Hurley | 0.06 | (0.05,0.08) | 0.02 | (0.01,0.02) | 0.02 | (0.01,0.03) | |
| Jamaica Plain | J.F. Kennedy | 0.04 | (0.03,0.05) | 0.06 | (0.04,0.08) | 0.05 | (0.04,0.07) | 0.07 |
| Jamaica Plain | Jackson/Mann | 0.01 | (0.00,0.02) | 0.01 | (0.01,0.02) | 0.01 | (0.00,0.02) | |
| Jamaica Plain | Kilmer | | | 0.02 | (0.01,0.04) | 0.03 | (0.02,0.05) | 0.02 |
| Jamaica Plain | Lyndon | 0.02 | (0.01,0.03) | 0.03 | (0.02,0.04) | 0.02 | (0.01,0.04) | 0.01 |
| Jamaica Plain | Lyon K-8 | | | 0.01 | (0.00,0.01) | 0.01 | (0.00,0.02) | |
| Jamaica Plain | Manning | 0.17 | (0.16,0.19) | 0.04 | (0.03,0.06) | 0.04 | (0.03,0.06) | 0.05 |
| Jamaica Plain | Mason | 0.03 | (0.02,0.05) | 0.01 | (0.00,0.01) | 0.01 | (0.00,0.02) | |
| Jamaica Plain | Mendell | 0.02 | (0.02,0.03) | 0.05 | (0.03,0.06) | 0.04 | (0.03,0.06) | 0.04 |
| Jamaica Plain | Mission Hill | 0.01 | (0.00,0.02) | 0.05 | (0.04,0.07) | 0.06 | (0.04,0.07) | 0.11 |
| Jamaica Plain | Mozart | | | 0.01 | (0.01,0.02) | 0.01 | (0.01,0.02) | 0.01 |
| Jamaica Plain | Orchard Gardens | 0.02 | (0.01,0.03) | 0.02 | (0.01,0.03) | 0.02 | (0.01,0.03) | 0.02 |
| Jamaica Plain | Otis | 0.01 | (0.00,0.01) | | | | | |
| Jamaica Plain | Philbrick | 0.10 | (0.09,0.12) | 0.01 | (0.00,0.02) | 0.01 | (0.00,0.02) | 0.02 |
| Jamaica Plain | Quincy | 0.02 | (0.01,0.03) | 0.02 | (0.01,0.03) | 0.02 | (0.01,0.03) | 0.02 |
| Jamaica Plain | Sumner | 0.08 | (0.06,0.09) | 0.02 | (0.01,0.02) | 0.01 | (0.01,0.02) | 0.01 |
| Jamaica Plain | Tobin | | | 0.03 | (0.02,0.05) | 0.04 | (0.02,0.05) | 0.02 |
| Jamaica Plain | Trotter | | | 0.01 | (0.01,0.02) | 0.01 | (0.01,0.02) | 0.01 |
| Jamaica Plain | Warren/Prescott | | | | | 0.00 | (0.00,0.01) | |
| Jamaica Plain | West Zone ELC | 0.01 | (0.01,0.02) | 0.06 | (0.04,0.08) | 0.07 | (0.06,0.09) | 0.05 |
| Jamaica Plain | Winship | | | 0.01 | (0.00,0.02) | 0.01 | (0.00,0.01) | |
| Jamaica Plain | Winthrop | | | 0.01 | (0.00,0.01) | | | |
| Mattapan | BTU | | | 0.01 | (0.00,0.01) | 0.01 | (0.00,0.01) | |
| Mattapan | Beethoven | | | 0.00 | (0.00,0.01) | | | |
| Mattapan | Channing | | | 0.02 | (0.01,0.04) | 0.02 | (0.01,0.03) | 0.03 |
| Mattapan | Chittick | 0.01 | (0.01,0.02) | 0.03 | (0.02,0.04) | 0.03 | (0.02,0.04) | 0.05 |
| Mattapan | Clap | 0.01 | (0.00,0.01) | 0.02 | (0.01,0.02) | 0.01 | (0.01,0.02) | 0.02 |
| Mattapan | Condon | 0.01 | (0.01,0.02) | 0.01 | (0.01,0.02) | 0.01 | (0.00,0.02) | 0.02 |
| Mattapan | Conley | 0.01 | (0.00,0.01) | | | | | |
| Mattapan | Curley | | | 0.01 | (0.00,0.01) | 0.01 | (0.00,0.01) | |
| Mattapan | Dever | 0.02 | (0.01,0.03) | 0.02 | (0.01,0.04) | 0.02 | (0.01,0.04) | 0.02 |
| Mattapan | E Greenwood | | | 0.04 | (0.02,0.06) | 0.03 | (0.02,0.05) | 0.05 |
| Mattapan | Ellison/Parks | 0.01 | (0.01,0.02) | 0.09 | (0.07,0.11) | 0.10 | (0.08,0.12) | 0.11 |
| Mattapan | Everett | | | 0.02 | (0.01,0.03) | 0.02 | (0.01,0.02) | 0.02 |
| Mattapan | Grew | | | 0.02 | (0.01,0.03) | 0.02 | (0.01,0.03) | 0.01 |
| Mattapan | Haley | | | 0.03 | (0.02,0.05) | 0.03 | (0.02,0.04) | 0.02 |
| Mattapan | Henderson | 0.22 | (0.21,0.23) | 0.02 | (0.01,0.03) | 0.03 | (0.02,0.04) | 0.02 |
| Mattapan | Hernandez | 0.02 | (0.01,0.02) | 0.05 | (0.03,0.06) | 0.04 | (0.03,0.06) | 0.05 |
| Mattapan | Holland | 0.01 | (0.01,0.02) | 0.03 | (0.02,0.04) | 0.03 | (0.02,0.04) | 0.04 |
| Mattapan | Holmes | | | 0.02 | (0.01,0.03) | 0.02 | (0.01,0.03) | 0.02 |
| Mattapan | J.F. Kennedy | 0.01 | (0.00,0.01) | 0.00 | (0.00,0.01) | | | |
| Mattapan | Kenny | 0.03 | (0.02,0.04) | 0.03 | (0.01,0.04) | 0.03 | (0.02,0.04) | 0.02 |
| Mattapan | Lyndon | 0.01 | (0.00,0.02) | 0.01 | (0.00,0.01) | 0.01 | (0.00,0.01) | |
| Mattapan | Mather | 0.01 | (0.01,0.02) | 0.02 | (0.01,0.03) | 0.02 | (0.01,0.03) | 0.02 |
| Mattapan | Mattahunt | 0.03 | (0.02,0.04) | 0.04 | (0.02,0.05) | 0.03 | (0.02,0.04) | 0.07 |
| Mattapan | Murphy | 0.21 | (0.19,0.22) | 0.05 | (0.04,0.07) | 0.06 | (0.05,0.08) | 0.05 |
| Mattapan | Perkins | | | 0.01 | (0.00,0.01) | 0.01 | (0.00,0.01) | |
| Mattapan | Perry | | | 0.01 | (0.01,0.02) | 0.02 | (0.01,0.02) | |
| Mattapan | Philbrick | 0.03 | (0.03,0.04) | | | | | |
| Mattapan | Roosevelt | 0.11 | (0.10,0.13) | 0.05 | (0.03,0.06) | 0.04 | (0.03,0.06) | 0.03 |

Continued on next page

**Table 3 – continued from previous page**

| Neighborhood | School | Naive mean | Naive (95% C.I.) | Logit mean | Logit (95% C.I.) | Mixed Logit mean | Mixed Logit (95% C.I.) | Actual |
|---|---|---|---|---|---|---|---|---|
| Mattapan | Russell | 0.03 | (0.02,0.04) | 0.02 | (0.01,0.03) | 0.02 | (0.01,0.03) | 0.02 |
| Mattapan | S. Greenwood | 0.05 | (0.04,0.07) | 0.05 | (0.04,0.07) | 0.06 | (0.04,0.07) | 0.06 |
| Mattapan | Sumner | 0.03 | (0.02,0.04) | 0.01 | (0.00,0.01) | 0.01 | (0.00,0.01) | |
| Mattapan | Taylor | 0.04 | (0.03,0.06) | 0.05 | (0.03,0.06) | 0.05 | (0.03,0.06) | 0.07 |
| Mattapan | Tynan | | | 0.01 | (0.00,0.01) | 0.01 | (0.00,0.01) | |
| Mattapan | Young Achievers | 0.02 | (0.01,0.03) | 0.15 | (0.12,0.18) | 0.17 | (0.14,0.18) | 0.12 |
| North Dorchester | Blackstone | | | 0.01 | (0.00,0.02) | 0.01 | (0.00,0.01) | |
| North Dorchester | Channing | | | 0.01 | (0.00,0.01) | 0.01 | (0.00,0.01) | |
| North Dorchester | Clap | 0.01 | (0.01,0.02) | 0.06 | (0.04,0.07) | 0.06 | (0.04,0.07) | 0.08 |
| North Dorchester | Condon | 0.04 | (0.03,0.06) | 0.04 | (0.03,0.06) | 0.04 | (0.02,0.05) | 0.05 |
| North Dorchester | Dever | 0.03 | (0.02,0.04) | 0.07 | (0.05,0.09) | 0.07 | (0.05,0.09) | 0.03 |
| North Dorchester | E Greenwood | | | 0.01 | (0.00,0.02) | 0.01 | (0.00,0.02) | |
| North Dorchester | Edison | 0.00 | (0.00,0.01) | | | | | |
| North Dorchester | Eliot | 0.00 | (0.00,0.01) | 0.01 | (0.00,0.01) | 0.01 | (0.00,0.01) | |
| North Dorchester | Ellison/Parks | | | 0.02 | (0.01,0.03) | 0.01 | (0.01,0.03) | |
| North Dorchester | Everett | 0.01 | (0.00,0.01) | 0.07 | (0.05,0.09) | 0.07 | (0.05,0.09) | 0.10 |
| North Dorchester | Gardner | | | 0.00 | (0.00,0.01) | | | |
| North Dorchester | Grew | | | 0.00 | (0.00,0.01) | 0.01 | (0.00,0.01) | |
| North Dorchester | Harvard/Kent | 0.01 | (0.00,0.01) | | | | | |
| North Dorchester | Haynes | 0.01 | (0.00,0.01) | 0.04 | (0.03,0.06) | 0.04 | (0.03,0.06) | 0.03 |
| North Dorchester | Henderson | 0.13 | (0.10,0.16) | 0.02 | (0.01,0.04) | 0.02 | (0.01,0.04) | 0.03 |
| North Dorchester | Hernandez | | | 0.03 | (0.02,0.04) | 0.03 | (0.01,0.04) | |
| North Dorchester | Holland | 0.04 | (0.02,0.05) | 0.05 | (0.03,0.07) | 0.04 | (0.03,0.06) | 0.04 |
| North Dorchester | Holmes | | | 0.01 | (0.00,0.02) | 0.01 | (0.00,0.02) | |
| North Dorchester | Hurley | 0.03 | (0.02,0.04) | 0.01 | (0.00,0.01) | 0.01 | (0.00,0.01) | |
| North Dorchester | Jackson/Mann | 0.01 | (0.00,0.02) | 0.00 | (0.00,0.01) | | | |
| North Dorchester | Kenny | | | 0.01 | (0.00,0.02) | 0.01 | (0.00,0.02) | |
| North Dorchester | King | | | 0.01 | (0.00,0.02) | 0.01 | (0.00,0.02) | |
| North Dorchester | Mason | 0.26 | (0.22,0.30) | 0.05 | (0.03,0.07) | 0.05 | (0.03,0.07) | 0.05 |
| North Dorchester | Mather | 0.05 | (0.03,0.06) | 0.07 | (0.05,0.09) | 0.08 | (0.06,0.10) | 0.10 |
| North Dorchester | Mattahunt | 0.01 | (0.00,0.01) | 0.00 | (0.00,0.01) | | | |
| North Dorchester | Murphy | 0.13 | (0.11,0.15) | 0.08 | (0.06,0.10) | 0.09 | (0.07,0.12) | 0.13 |
| North Dorchester | Orchard Gardens | 0.05 | (0.03,0.07) | 0.03 | (0.01,0.04) | 0.03 | (0.02,0.04) | 0.02 |
| North Dorchester | Otis | 0.01 | (0.01,0.02) | | | | | |
| North Dorchester | Perkins | | | 0.02 | (0.01,0.03) | 0.02 | (0.01,0.03) | |
| North Dorchester | Perry | | | 0.04 | (0.02,0.05) | 0.04 | (0.02,0.05) | 0.04 |
| North Dorchester | Quincy | 0.01 | (0.00,0.02) | 0.01 | (0.00,0.02) | 0.01 | (0.00,0.02) | |
| North Dorchester | Roosevelt | 0.05 | (0.03,0.06) | 0.01 | (0.01,0.02) | 0.02 | (0.01,0.03) | |
| North Dorchester | Russell | 0.04 | (0.03,0.06) | 0.08 | (0.06,0.10) | 0.08 | (0.06,0.10) | 0.08 |
| North Dorchester | S. Greenwood | 0.03 | (0.01,0.04) | 0.02 | (0.01,0.03) | 0.01 | (0.01,0.03) | 0.01 |
| North Dorchester | Taylor | | | 0.01 | (0.00,0.01) | 0.00 | (0.00,0.01) | |
| North Dorchester | Trotter | | | 0.00 | (0.00,0.01) | | | |
| North Dorchester | Tynan | | | 0.02 | (0.01,0.03) | 0.01 | (0.00,0.03) | 0.02 |
| North Dorchester | Winthrop | 0.02 | (0.01,0.03) | 0.03 | (0.02,0.05) | 0.03 | (0.02,0.04) | 0.02 |
| North Dorchester | Young Achievers | 0.00 | (0.00,0.01) | 0.02 | (0.01,0.04) | 0.02 | (0.01,0.04) | 0.02 |
| Roslindale | BTU | 0.01 | (0.01,0.02) | 0.09 | (0.07,0.11) | 0.09 | (0.08,0.11) | 0.07 |
| Roslindale | Bates | 0.01 | (0.00,0.01) | 0.06 | (0.04,0.07) | 0.06 | (0.04,0.07) | 0.06 |
| Roslindale | Beethoven | 0.04 | (0.03,0.05) | 0.11 | (0.09,0.13) | 0.11 | (0.09,0.13) | 0.09 |
| Roslindale | Conley | 0.18 | (0.16,0.19) | 0.04 | (0.03,0.06) | 0.04 | (0.03,0.05) | 0.06 |
| Roslindale | Curley | 0.03 | (0.02,0.04) | 0.04 | (0.02,0.05) | 0.04 | (0.02,0.05) | 0.04 |
| Roslindale | E Greenwood | | | 0.02 | (0.01,0.03) | 0.02 | (0.01,0.02) | |
| Roslindale | Ellis | 0.01 | (0.01,0.02) | 0.01 | (0.00,0.01) | 0.01 | (0.00,0.02) | |
| Roslindale | Grew | | | 0.01 | (0.00,0.01) | 0.01 | (0.00,0.01) | |
| Roslindale | Hale | | | 0.01 | (0.00,0.01) | | | |
| Roslindale | Haley | 0.01 | (0.01,0.02) | 0.05 | (0.04,0.06) | 0.05 | (0.04,0.07) | 0.07 |

Continued on next page

**Table 3 – continued from previous page**

| Neighborhood | School | Naive mean | Naive (95% C.I.) | Logit mean | Logit (95% C.I.) | Mixed Logit mean | Mixed Logit (95% C.I.) | Actual |
|---|---|---|---|---|---|---|---|---|
| Roslindale | Haynes | | | 0.01 | (0.00,0.01) | 0.01 | (0.00,0.02) | 0.02 |
| Roslindale | Hennigan | 0.02 | (0.01,0.03) | 0.02 | (0.01,0.03) | 0.02 | (0.01,0.03) | 0.02 |
| Roslindale | Hernandez | 0.01 | (0.01,0.02) | 0.03 | (0.02,0.04) | 0.03 | (0.02,0.04) | 0.04 |
| Roslindale | J.F. Kennedy | 0.01 | (0.01,0.02) | 0.02 | (0.01,0.03) | 0.01 | (0.01,0.02) | 0.02 |
| Roslindale | Kenny | 0.01 | (0.01,0.02) | | | | | |
| Roslindale | Kilmer | 0.01 | (0.01,0.01) | 0.07 | (0.05,0.08) | 0.08 | (0.06,0.09) | 0.08 |
| Roslindale | Lyndon | 0.08 | (0.07,0.10) | 0.10 | (0.09,0.12) | 0.09 | (0.07,0.11) | 0.09 |
| Roslindale | Manning | 0.02 | (0.01,0.03) | 0.03 | (0.02,0.04) | 0.03 | (0.02,0.04) | 0.03 |
| Roslindale | Mattahunt | 0.01 | (0.00,0.01) | 0.01 | (0.00,0.01) | 0.01 | (0.00,0.01) | |
| Roslindale | Mendell | | | 0.01 | (0.01,0.02) | 0.01 | (0.01,0.02) | 0.01 |
| Roslindale | Mission Hill | | | 0.03 | (0.02,0.04) | 0.03 | (0.02,0.04) | 0.03 |
| Roslindale | Mozart | 0.02 | (0.01,0.02) | 0.07 | (0.06,0.09) | 0.07 | (0.06,0.09) | 0.06 |
| Roslindale | Philbrick | 0.15 | (0.13,0.16) | 0.03 | (0.02,0.05) | 0.03 | (0.02,0.04) | 0.06 |
| Roslindale | Roosevelt | 0.01 | (0.00,0.01) | 0.01 | (0.00,0.01) | 0.01 | (0.00,0.01) | |
| Roslindale | Sumner | 0.29 | (0.28,0.31) | 0.08 | (0.06,0.10) | 0.09 | (0.07,0.10) | 0.09 |
| Roslindale | Taylor | 0.02 | (0.01,0.02) | | | | | |
| Roslindale | Trotter | 0.01 | (0.01,0.01) | 0.01 | (0.00,0.01) | 0.01 | (0.00,0.01) | |
| Roslindale | West Zone ELC | | | 0.02 | (0.01,0.03) | 0.02 | (0.01,0.03) | 0.02 |
| Roslindale | Young Achievers | | | 0.01 | (0.00,0.01) | 0.01 | (0.00,0.01) | |
| Roxbury | BTU | | | 0.03 | (0.03,0.04) | 0.03 | (0.02,0.04) | 0.02 |
| Roxbury | Bates | | | 0.01 | (0.00,0.01) | 0.01 | (0.00,0.01) | |
| Roxbury | Beethoven | 0.02 | (0.02,0.03) | 0.02 | (0.02,0.03) | 0.02 | (0.02,0.03) | 0.02 |
| Roxbury | Blackstone | | | 0.02 | (0.01,0.02) | 0.02 | (0.01,0.02) | 0.02 |
| Roxbury | Clap | | | 0.01 | (0.01,0.01) | 0.01 | (0.00,0.01) | |
| Roxbury | Conley | | | 0.01 | (0.00,0.01) | | | |
| Roxbury | Curley | 0.02 | (0.01,0.02) | 0.05 | (0.04,0.06) | 0.05 | (0.04,0.06) | 0.04 |
| Roxbury | Dever | 0.01 | (0.00,0.01) | 0.01 | (0.00,0.01) | 0.01 | (0.00,0.01) | |
| Roxbury | Eliot | | | 0.01 | (0.01,0.01) | 0.01 | (0.01,0.01) | |
| Roxbury | Ellis | 0.03 | (0.02,0.03) | 0.03 | (0.03,0.04) | 0.04 | (0.03,0.04) | 0.05 |
| Roxbury | Everett | | | 0.01 | (0.01,0.02) | 0.01 | (0.01,0.02) | |
| Roxbury | Gardner | | | 0.01 | (0.00,0.01) | 0.01 | (0.00,0.01) | |
| Roxbury | Hale | 0.15 | (0.14,0.16) | 0.03 | (0.02,0.04) | 0.03 | (0.02,0.04) | 0.03 |
| Roxbury | Haley | | | 0.01 | (0.01,0.02) | 0.01 | (0.01,0.02) | 0.01 |
| Roxbury | Haynes | 0.01 | (0.01,0.01) | 0.04 | (0.03,0.06) | 0.05 | (0.04,0.06) | 0.06 |
| Roxbury | Henderson | 0.03 | (0.02,0.03) | | | | | |
| Roxbury | Hennigan | 0.02 | (0.01,0.02) | 0.04 | (0.03,0.05) | 0.03 | (0.02,0.04) | 0.04 |
| Roxbury | Hernandez | 0.01 | (0.01,0.01) | 0.06 | (0.04,0.07) | 0.07 | (0.06,0.08) | 0.06 |
| Roxbury | Higginson/Lewis | 0.01 | (0.01,0.01) | 0.02 | (0.01,0.03) | 0.02 | (0.01,0.03) | 0.03 |
| Roxbury | Holland | 0.01 | (0.01,0.01) | 0.03 | (0.02,0.04) | 0.03 | (0.02,0.04) | 0.03 |
| Roxbury | Holmes | | | 0.01 | (0.00,0.01) | 0.01 | (0.01,0.01) | |
| Roxbury | Hurley | 0.04 | (0.03,0.05) | 0.02 | (0.01,0.03) | 0.02 | (0.01,0.03) | 0.01 |
| Roxbury | J.F. Kennedy | 0.02 | (0.01,0.03) | 0.03 | (0.02,0.05) | 0.03 | (0.02,0.04) | 0.03 |
| Roxbury | Jackson/Mann | 0.01 | (0.01,0.02) | 0.01 | (0.00,0.01) | | | |
| Roxbury | Kennedy Patrick | 0.01 | (0.00,0.01) | | | | | |
| Roxbury | Kilmer | | | 0.01 | (0.00,0.01) | 0.01 | (0.01,0.02) | |
| Roxbury | King | 0.01 | (0.01,0.01) | 0.02 | (0.01,0.03) | 0.02 | (0.01,0.03) | 0.04 |
| Roxbury | Lyndon | 0.03 | (0.02,0.03) | 0.02 | (0.01,0.03) | 0.02 | (0.01,0.02) | 0.02 |
| Roxbury | Manning | 0.07 | (0.06,0.08) | 0.01 | (0.01,0.01) | 0.01 | (0.01,0.01) | |
| Roxbury | Mason | 0.16 | (0.14,0.17) | 0.03 | (0.02,0.04) | 0.04 | (0.03,0.04) | 0.03 |
| Roxbury | Mather | | | 0.01 | (0.01,0.02) | 0.01 | (0.01,0.02) | 0.01 |
| Roxbury | Mendell | | | 0.02 | (0.01,0.03) | 0.02 | (0.02,0.03) | 0.02 |
| Roxbury | Mission Hill | | | 0.02 | (0.02,0.03) | 0.02 | (0.01,0.03) | 0.03 |
| Roxbury | Mozart | | | 0.01 | (0.00,0.01) | 0.01 | (0.00,0.01) | |
| Roxbury | Murphy | 0.03 | (0.02,0.03) | 0.01 | (0.00,0.01) | 0.01 | (0.00,0.01) | |
| Roxbury | Orchard Gardens | 0.04 | (0.03,0.05) | 0.05 | (0.04,0.07) | 0.04 | (0.04,0.05) | 0.06 |

Continued on next page

**Table 3 – continued from previous page**

| Neighborhood | School | Naive mean | Naive (95% C.I.) | Logit mean | Logit (95% C.I.) | Mixed Logit mean | Mixed Logit (95% C.I.) | Actual |
|---|---|---|---|---|---|---|---|---|
| Roxbury | Otis | 0.01 | (0.01,0.01) | | | | | |
| Roxbury | Philbrick | 0.05 | (0.04,0.06) | 0.01 | (0.00,0.01) | | | |
| Roxbury | Quincy | | | 0.01 | (0.00,0.01) | 0.01 | (0.00,0.01) | |
| Roxbury | Roosevelt | 0.02 | (0.01,0.02) | | | | | |
| Roxbury | Russell | 0.01 | (0.01,0.01) | 0.02 | (0.01,0.03) | 0.02 | (0.01,0.03) | 0.01 |
| Roxbury | S. Greenwood | 0.02 | (0.01,0.02) | 0.02 | (0.02,0.03) | 0.02 | (0.02,0.03) | 0.03 |
| Roxbury | Sumner | 0.05 | (0.04,0.06) | 0.01 | (0.01,0.02) | 0.01 | (0.01,0.02) | 0.01 |
| Roxbury | Tobin | | | 0.02 | (0.01,0.03) | 0.02 | (0.01,0.03) | 0.02 |
| Roxbury | Trotter | 0.02 | (0.02,0.02) | 0.04 | (0.03,0.05) | 0.03 | (0.03,0.04) | 0.05 |
| Roxbury | West Zone ELC | | | 0.03 | (0.02,0.04) | 0.04 | (0.03,0.04) | 0.02 |
| Roxbury | Winthrop | 0.02 | (0.01,0.02) | 0.03 | (0.03,0.04) | 0.03 | (0.02,0.04) | 0.04 |
| Roxbury | Young Achievers | | | 0.01 | (0.01,0.02) | 0.01 | (0.01,0.02) | 0.01 |
| South Boston | Blackstone | 0.01 | (0.00,0.01) | 0.02 | (0.01,0.04) | 0.02 | (0.01,0.04) | 0.02 |
| South Boston | Channing | | | | | 0.01 | (0.00,0.01) | |
| South Boston | Chittick | | | | | 0.00 | (0.00,0.01) | |
| South Boston | Clap | | | 0.04 | (0.02,0.06) | 0.05 | (0.03,0.07) | 0.05 |
| South Boston | Condon | 0.12 | (0.09,0.14) | 0.16 | (0.13,0.19) | 0.16 | (0.13,0.19) | 0.26 |
| South Boston | Dever | 0.05 | (0.03,0.07) | 0.09 | (0.06,0.11) | 0.09 | (0.06,0.11) | 0.04 |
| South Boston | E Greenwood | | | 0.01 | (0.00,0.01) | 0.01 | (0.00,0.02) | |
| South Boston | Eliot | | | | | 0.01 | | |
| South Boston | Ellison/Parks | 0.01 | (0.00,0.02) | 0.01 | (0.00,0.02) | 0.01 | (0.00,0.02) | 0.01 |
| South Boston | Everett | | | 0.03 | (0.02,0.05) | 0.03 | (0.01,0.05) | 0.01 |
| South Boston | Grew | | | | | 0.00 | (0.00,0.01) | |
| South Boston | Harvard/Kent | 0.02 | (0.01,0.03) | 0.01 | (0.00,0.01) | 0.01 | (0.00,0.01) | 0.01 |
| South Boston | Henderson | 0.15 | (0.12,0.17) | 0.02 | (0.01,0.03) | 0.02 | (0.01,0.03) | 0.04 |
| South Boston | Hernandez | | | 0.03 | (0.01,0.04) | 0.03 | (0.01,0.04) | 0.01 |
| South Boston | Holland | 0.01 | (0.00,0.01) | 0.02 | (0.01,0.04) | 0.02 | (0.01,0.03) | 0.01 |
| South Boston | Holmes | | | 0.01 | (0.00,0.01) | 0.00 | (0.00,0.01) | |
| South Boston | Kenny | 0.01 | (0.00,0.01) | 0.01 | (0.00,0.02) | 0.01 | (0.00,0.02) | |
| South Boston | Mason | 0.13 | (0.10,0.17) | 0.02 | (0.01,0.04) | 0.02 | (0.01,0.04) | 0.01 |
| South Boston | Mather | | | 0.02 | (0.01,0.03) | 0.02 | (0.01,0.03) | |
| South Boston | Murphy | 0.16 | (0.14,0.19) | 0.07 | (0.05,0.09) | 0.07 | (0.04,0.09) | 0.06 |
| South Boston | Orchard Gardens | 0.01 | (0.00,0.01) | 0.00 | (0.00,0.01) | 0.00 | (0.00,0.01) | |
| South Boston | Perkins | 0.01 | (0.00,0.02) | 0.05 | (0.03,0.07) | 0.05 | (0.03,0.07) | 0.06 |
| South Boston | Perry | 0.03 | (0.02,0.04) | 0.14 | (0.11,0.17) | 0.14 | (0.12,0.17) | 0.18 |
| South Boston | Quincy | 0.07 | (0.05,0.09) | 0.04 | (0.03,0.06) | 0.04 | (0.02,0.06) | 0.03 |
| South Boston | Roosevelt | 0.06 | (0.04,0.08) | 0.01 | (0.00,0.01) | 0.01 | (0.00,0.03) | |
| South Boston | Russell | 0.05 | (0.03,0.07) | 0.05 | (0.03,0.07) | 0.05 | (0.03,0.07) | 0.03 |
| South Boston | S. Greenwood | 0.08 | (0.06,0.10) | 0.02 | (0.01,0.03) | 0.02 | (0.01,0.03) | 0.01 |
| South Boston | Taylor | | | 0.00 | (0.00,0.01) | | | |
| South Boston | Tynan | 0.01 | (0.00,0.02) | 0.07 | (0.05,0.10) | 0.07 | (0.05,0.10) | 0.10 |
| South Boston | Young Achievers | | | 0.03 | (0.01,0.04) | 0.03 | (0.01,0.04) | 0.01 |
| South Dorchester | Channing | | | 0.01 | (0.01,0.02) | 0.01 | (0.01,0.02) | 0.01 |
| South Dorchester | Chittick | | | 0.01 | (0.01,0.01) | 0.01 | (0.00,0.01) | |
| South Dorchester | Clap | | | 0.02 | (0.01,0.03) | 0.02 | (0.01,0.03) | 0.02 |
| South Dorchester | Condon | 0.03 | (0.02,0.04) | 0.03 | (0.02,0.04) | 0.02 | (0.02,0.03) | 0.03 |
| South Dorchester | Dever | 0.03 | (0.02,0.04) | 0.04 | (0.03,0.05) | 0.04 | (0.03,0.05) | 0.02 |
| South Dorchester | E Greenwood | 0.01 | (0.00,0.01) | 0.02 | (0.01,0.03) | 0.02 | (0.01,0.02) | 0.01 |
| South Dorchester | Ellison/Parks | 0.01 | (0.00,0.01) | 0.03 | (0.03,0.04) | 0.04 | (0.03,0.05) | 0.04 |
| South Dorchester | Everett | | | 0.04 | (0.03,0.05) | 0.04 | (0.03,0.05) | 0.04 |
| South Dorchester | Grew | | | 0.01 | (0.00,0.01) | 0.01 | (0.00,0.01) | |
| South Dorchester | Haynes | | | 0.01 | (0.01,0.02) | 0.01 | (0.01,0.02) | |
| South Dorchester | Henderson | 0.22 | (0.20,0.23) | 0.07 | (0.06,0.08) | 0.08 | (0.06,0.09) | 0.09 |
| South Dorchester | Hernandez | | | 0.03 | (0.03,0.04) | 0.03 | (0.02,0.04) | 0.03 |
| South Dorchester | Holland | 0.06 | (0.05,0.07) | 0.07 | (0.05,0.08) | 0.07 | (0.06,0.08) | 0.07 |

Continued on next page

**Table 3 – continued from previous page**

| Neighborhood | School | Naive mean | Naive (95% C.I.) | Logit mean | Logit (95% C.I.) | Mixed Logit mean | Mixed Logit (95% C.I.) | Actual |
|---|---|---|---|---|---|---|---|---|
| South Dorchester | Holmes | 0.01 | (0.01,0.01) | 0.03 | (0.02,0.04) | 0.03 | (0.02,0.04) | 0.03 |
| South Dorchester | Kenny | 0.02 | (0.02,0.03) | 0.06 | (0.04,0.07) | 0.06 | (0.05,0.07) | 0.04 |
| South Dorchester | King | | | 0.01 | (0.01,0.01) | 0.01 | (0.01,0.01) | |
| South Dorchester | Mather | 0.06 | (0.05,0.07) | 0.07 | (0.06,0.09) | 0.08 | (0.06,0.09) | 0.08 |
| South Dorchester | Mattahunt | 0.01 | (0.00,0.01) | 0.01 | (0.01,0.01) | 0.01 | (0.00,0.01) | 0.02 |
| South Dorchester | Murphy | 0.25 | (0.24,0.26) | 0.17 | (0.15,0.18) | 0.18 | (0.16,0.20) | 0.18 |
| South Dorchester | Orchard Gardens | 0.02 | (0.01,0.02) | 0.01 | (0.00,0.01) | | | |
| South Dorchester | Perkins | | | 0.01 | (0.01,0.02) | 0.01 | (0.00,0.01) | |
| South Dorchester | Perry | | | 0.03 | (0.02,0.04) | 0.03 | (0.02,0.04) | 0.02 |
| South Dorchester | Roosevelt | 0.13 | (0.11,0.14) | 0.02 | (0.01,0.03) | 0.02 | (0.02,0.03) | 0.01 |
| South Dorchester | Russell | 0.03 | (0.03,0.04) | 0.03 | (0.02,0.04) | 0.03 | (0.02,0.04) | 0.03 |
| South Dorchester | S. Greenwood | 0.05 | (0.04,0.06) | 0.05 | (0.04,0.06) | 0.05 | (0.04,0.06) | 0.05 |
| South Dorchester | Taylor | 0.01 | (0.01,0.02) | 0.02 | (0.01,0.03) | 0.02 | (0.01,0.03) | 0.01 |
| South Dorchester | Tynan | | | 0.01 | (0.01,0.02) | 0.01 | (0.00,0.01) | |
| South Dorchester | Winthrop | | | 0.01 | (0.00,0.01) | 0.01 | (0.00,0.01) | |
| South Dorchester | Young Achievers | | | 0.06 | (0.04,0.07) | 0.06 | (0.05,0.07) | 0.06 |
| South End | Baldwin | | | 0.03 | (0.02,0.04) | 0.03 | (0.02,0.04) | 0.01 |
| South End | Blackstone | 0.04 | (0.03,0.06) | 0.10 | (0.08,0.12) | 0.10 | (0.08,0.12) | 0.16 |
| South End | Bradley | | | | | 0.01 | (0.00,0.01) | |
| South End | Condon | | | 0.02 | (0.01,0.04) | 0.03 | (0.01,0.04) | |
| South End | Curley | 0.00 | (0.00,0.01) | | | | | |
| South End | East Boston EEC | | | 0.01 | (0.00,0.02) | 0.02 | (0.01,0.03) | |
| South End | Edison | 0.02 | (0.01,0.04) | 0.02 | (0.01,0.03) | 0.01 | (0.01,0.02) | 0.01 |
| South End | Eliot | 0.02 | (0.01,0.02) | 0.10 | (0.07,0.12) | 0.09 | (0.07,0.12) | 0.08 |
| South End | Gardner | 0.01 | (0.01,0.02) | 0.04 | (0.02,0.05) | 0.03 | (0.02,0.04) | 0.01 |
| South End | Hale | 0.04 | (0.03,0.05) | 0.01 | (0.01,0.02) | 0.01 | (0.01,0.02) | |
| South End | Harvard/Kent | 0.05 | (0.03,0.06) | 0.04 | (0.03,0.06) | 0.04 | (0.02,0.05) | 0.04 |
| South End | Hernandez | 0.01 | (0.01,0.02) | 0.04 | (0.03,0.05) | 0.04 | (0.02,0.05) | 0.03 |
| South End | Higginson/Lewis | | | 0.01 | (0.00,0.01) | 0.00 | (0.00,0.01) | |
| South End | Hurley | 0.27 | (0.26,0.29) | 0.13 | (0.10,0.15) | 0.14 | (0.11,0.16) | 0.17 |
| South End | J.F. Kennedy | 0.00 | (0.00,0.01) | | | | | |
| South End | Jackson/Mann | 0.04 | (0.02,0.05) | 0.03 | (0.01,0.04) | 0.02 | (0.01,0.03) | 0.02 |
| South End | Kennedy Patrick | 0.02 | (0.01,0.03) | 0.01 | (0.00,0.01) | 0.01 | (0.00,0.01) | |
| South End | Lyon K-8 | | | 0.02 | (0.01,0.03) | 0.02 | (0.01,0.03) | |
| South End | Mario Umana | | | 0.01 | (0.00,0.01) | 0.01 | (0.00,0.01) | |
| South End | Mason | 0.16 | (0.14,0.19) | 0.05 | (0.03,0.07) | 0.05 | (0.03,0.07) | 0.02 |
| South End | McKay | | | 0.01 | (0.00,0.01) | 0.01 | (0.00,0.02) | |
| South End | Mission Hill | | | | | 0.02 | | |
| South End | O'Donnell | | | 0.01 | (0.00,0.01) | 0.01 | (0.00,0.01) | |
| South End | Orchard Gardens | 0.06 | (0.04,0.07) | 0.09 | (0.06,0.12) | 0.08 | (0.06,0.10) | 0.10 |
| South End | Otis | 0.04 | (0.03,0.06) | 0.01 | (0.00,0.01) | 0.00 | (0.00,0.01) | |
| South End | Quincy | 0.17 | (0.15,0.19) | 0.13 | (0.11,0.16) | 0.14 | (0.12,0.16) | 0.20 |
| South End | Tobin | | | 0.04 | (0.02,0.05) | 0.04 | (0.02,0.05) | 0.02 |
| South End | Warren/Prescott | | | 0.04 | (0.02,0.05) | 0.04 | (0.02,0.05) | 0.01 |
| South End | Winship | | | 0.02 | (0.01,0.03) | 0.01 | (0.01,0.03) | |
| South End | Winthrop | | | 0.01 | (0.00,0.02) | 0.01 | (0.01,0.02) | |
| West Roxbury | BTU | | | 0.04 | (0.03,0.06) | 0.04 | (0.03,0.06) | 0.04 |
| West Roxbury | Bates | | | 0.04 | (0.03,0.06) | 0.04 | (0.03,0.05) | 0.03 |
| West Roxbury | Beethoven | 0.06 | (0.04,0.07) | 0.21 | (0.19,0.23) | 0.21 | (0.19,0.23) | 0.22 |
| West Roxbury | Channing | | | 0.02 | (0.01,0.03) | 0.02 | (0.01,0.03) | 0.01 |
| West Roxbury | Conley | 0.10 | (0.08,0.12) | 0.02 | (0.01,0.04) | 0.02 | (0.01,0.03) | 0.02 |
| West Roxbury | Curley | 0.01 | (0.01,0.02) | 0.02 | (0.01,0.03) | 0.02 | (0.01,0.03) | 0.01 |
| West Roxbury | Grew | | | 0.01 | (0.01,0.02) | 0.01 | (0.01,0.02) | 0.01 |
| West Roxbury | Haley | | | 0.02 | (0.01,0.03) | 0.02 | (0.01,0.03) | 0.02 |
| West Roxbury | Harvard/Kent | 0.01 | (0.00,0.01) | | | | | |

Continued on next page

**Table 3 – continued from previous page**

| Neighborhood | School | Naive | | Logit | | Mixed Logit | | Actual |
|---|---|---|---|---|---|---|---|---|
| | | mean | (95% C.I.) | mean | (95% C.I.) | mean | (95% C.I.) | |
| West Roxbury | Haynes | 0.01 | (0.00,0.01) | | | 0.01 | (0.00,0.01) | 0.02 |
| West Roxbury | Hennigan | 0.02 | (0.01,0.03) | 0.01 | (0.00,0.01) | 0.01 | (0.00,0.01) | |
| West Roxbury | Hernandez | | | 0.01 | (0.00,0.02) | 0.01 | (0.01,0.02) | 0.01 |
| West Roxbury | J.F. Kennedy | | | 0.01 | (0.00,0.01) | 0.01 | (0.00,0.01) | |
| West Roxbury | Kilmer | 0.25 | (0.23,0.26) | 0.21 | (0.18,0.23) | 0.21 | (0.19,0.23) | 0.23 |
| West Roxbury | Lyndon | 0.29 | (0.28,0.30) | 0.19 | (0.17,0.21) | 0.19 | (0.17,0.21) | 0.20 |
| West Roxbury | Manning | 0.02 | (0.01,0.03) | 0.03 | (0.02,0.05) | 0.03 | (0.02,0.04) | 0.03 |
| West Roxbury | Mattahunt | 0.01 | (0.00,0.01) | | | | | |
| West Roxbury | Mendell | | | 0.01 | (0.00,0.01) | 0.00 | (0.00,0.01) | |
| West Roxbury | Mission Hill | | | 0.02 | (0.01,0.03) | 0.01 | (0.01,0.02) | 0.01 |
| West Roxbury | Mozart | 0.02 | (0.01,0.03) | 0.07 | (0.06,0.09) | 0.07 | (0.05,0.09) | 0.05 |
| West Roxbury | Philbrick | | | 0.01 | (0.01,0.03) | 0.01 | (0.00,0.02) | 0.02 |
| West Roxbury | Quincy | 0.01 | (0.00,0.01) | | | | | |
| West Roxbury | Sumner | 0.14 | (0.12,0.16) | 0.02 | (0.01,0.04) | 0.03 | (0.01,0.04) | 0.02 |
| West Roxbury | Trotter | 0.01 | (0.00,0.01) | | | 0.01 | | |
| West Roxbury | West Zone ELC | | | 0.01 | (0.01,0.02) | 0.02 | (0.01,0.02) | 0.02 |

### D.1.2 K1

Table 4: Top Choice Market Share Predictions for 2013 K1

| Neighborhood | School | Naive | | Logit | | Mixed Logit | | Actual |
|---|---|---|---|---|---|---|---|---|
| | | mean | (95% C.I.) | mean | (95% C.I.) | mean | (95% C.I.) | |
| Allston-Brighton | Adams | | | | | 0.00 | (0.00,0.02) | |
| Allston-Brighton | Baldwin | 0.20 | (0.17,0.24) | 0.32 | (0.25,0.38) | 0.32 | (0.25,0.39) | 0.50 |
| Allston-Brighton | Blackstone | | | 0.02 | (0.00,0.05) | 0.02 | (0.00,0.04) | |
| Allston-Brighton | Bradley | | | 0.00 | (0.00,0.01) | 0.01 | (0.00,0.02) | |
| Allston-Brighton | East Boston EEC | | | 0.01 | (0.00,0.02) | 0.02 | (0.00,0.04) | |
| Allston-Brighton | Edison | 0.03 | (0.01,0.06) | 0.17 | (0.11,0.24) | 0.18 | (0.12,0.25) | 0.04 |
| Allston-Brighton | Eliot | | | 0.02 | (0.00,0.05) | 0.02 | (0.00,0.05) | |
| Allston-Brighton | Ellison/Parks | 0.01 | (0.00,0.03) | | | | | |
| Allston-Brighton | Gardner | 0.04 | (0.01,0.07) | 0.13 | (0.08,0.19) | 0.14 | (0.08,0.21) | 0.14 |
| Allston-Brighton | Harvard/Kent | 0.07 | (0.03,0.12) | 0.02 | (0.00,0.04) | 0.02 | (0.00,0.04) | |
| Allston-Brighton | Hernandez | | | 0.02 | (0.00,0.05) | 0.02 | (0.00,0.05) | |
| Allston-Brighton | Hurley | 0.38 | (0.30,0.45) | 0.03 | (0.01,0.06) | 0.03 | (0.00,0.06) | |
| Allston-Brighton | Jackson/Mann | 0.05 | (0.01,0.09) | 0.10 | (0.05,0.15) | 0.08 | (0.04,0.13) | 0.12 |
| Allston-Brighton | Kennedy Patrick | | | 0.00 | (0.00,0.01) | 0.00 | (0.00,0.01) | |
| Allston-Brighton | Mason | | | 0.01 | (0.00,0.02) | 0.01 | (0.00,0.02) | |
| Allston-Brighton | O'Donnell | | | 0.00 | (0.00,0.01) | 0.00 | (0.00,0.01) | |
| Allston-Brighton | Orchard Gardens | 0.01 | (0.00,0.03) | 0.01 | (0.00,0.02) | 0.01 | (0.00,0.02) | |
| Allston-Brighton | Otis | 0.18 | (0.12,0.24) | 0.00 | (0.00,0.02) | 0.01 | (0.00,0.02) | |
| Allston-Brighton | Quincy | 0.01 | (0.00,0.02) | 0.03 | (0.01,0.06) | 0.03 | (0.01,0.07) | 0.03 |
| Allston-Brighton | Tobin | | | 0.01 | (0.00,0.03) | 0.01 | (0.00,0.02) | |
| Allston-Brighton | Winship | 0.02 | (0.00,0.05) | 0.10 | (0.05,0.16) | 0.08 | (0.04,0.13) | 0.12 |
| Charlestown | Adams | | | 0.01 | (0.00,0.04) | 0.00 | (0.00,0.03) | |
| Charlestown | Baldwin | 0.06 | (0.02,0.10) | 0.04 | (0.00,0.10) | 0.04 | (0.00,0.10) | 0.03 |
| Charlestown | Blackstone | | | 0.03 | (0.00,0.09) | 0.03 | (0.00,0.10) | 0.02 |
| Charlestown | Bradley | | | 0.02 | (0.00,0.06) | 0.01 | (0.00,0.06) | 0.02 |
| Charlestown | Dever | 0.02 | (0.00,0.06) | | | | | |
| Charlestown | East Boston EEC | | | 0.02 | (0.00,0.09) | 0.02 | (0.00,0.07) | 0.02 |
| Charlestown | Edison | | | 0.01 | (0.00,0.03) | 0.01 | (0.00,0.04) | |
| Charlestown | Eliot | 0.02 | (0.00,0.07) | 0.37 | (0.24,0.51) | 0.38 | (0.25,0.54) | 0.47 |

Continued on next page

**Table 4 – continued from previous page**

| | | Naive | | Logit | | Mixed Logit | | |
|---|---|---|---|---|---|---|---|---|
| Neighborhood | School | mean | (95% C.I.) | mean | (95% C.I.) | mean | (95% C.I.) | Actual |
| Charlestown | Gardner | | | 0.01 | (0.00,0.06) | 0.01 | (0.00,0.05) | 0.02 |
| Charlestown | Harvard/Kent | 0.69 | (0.55,0.81) | 0.21 | (0.10,0.34) | 0.24 | (0.12,0.37) | 0.39 |
| Charlestown | Hernandez | | | 0.01 | (0.00,0.04) | 0.01 | (0.00,0.05) | |
| Charlestown | Hurley | 0.12 | (0.03,0.23) | 0.04 | (0.00,0.11) | 0.04 | (0.00,0.10) | 0.02 |
| Charlestown | Jackson/Mann | | | 0.01 | (0.00,0.05) | 0.00 | (0.00,0.03) | |
| Charlestown | Kennedy Patrick | | | 0.01 | (0.00,0.05) | 0.01 | (0.00,0.04) | |
| Charlestown | Mason | 0.02 | (0.00,0.06) | 0.00 | (0.00,0.03) | 0.00 | (0.00,0.03) | |
| Charlestown | O'Donnell | | | 0.01 | (0.00,0.06) | 0.01 | (0.00,0.04) | |
| Charlestown | Orchard Gardens | | | 0.01 | (0.00,0.04) | 0.01 | (0.00,0.04) | |
| Charlestown | Otis | 0.02 | (0.00,0.06) | 0.02 | (0.00,0.07) | 0.01 | (0.00,0.06) | |
| Charlestown | Quincy | 0.02 | (0.00,0.06) | 0.14 | (0.05,0.26) | 0.14 | (0.05,0.24) | 0.03 |
| Charlestown | Roosevelt | | | | | 0.00 | (0.00,0.02) | |
| Charlestown | Taylor | 0.03 | (0.00,0.10) | | | 0.00 | (0.00,0.02) | |
| Charlestown | Tobin | 0.02 | (0.00,0.06) | 0.01 | (0.00,0.04) | 0.01 | (0.00,0.04) | |
| Charlestown | Winship | | | 0.01 | (0.00,0.04) | 0.01 | (0.00,0.04) | |
| Charlestown | Winthrop | | | 0.00 | (0.00,0.02) | | | |
| Charlestown | Young Achievers | | | | | 0.00 | (0.00,0.02) | |
| Downtown | Adams | | | | | 0.00 | (0.00,0.01) | |
| Downtown | Baldwin | | | 0.03 | (0.00,0.06) | 0.03 | (0.00,0.06) | 0.05 |
| Downtown | Blackstone | 0.01 | (0.00,0.03) | 0.05 | (0.02,0.10) | 0.05 | (0.02,0.09) | 0.01 |
| Downtown | Bradley | | | 0.01 | (0.00,0.02) | 0.01 | (0.00,0.03) | |
| Downtown | Condon | | | 0.01 | (0.00,0.03) | 0.01 | (0.00,0.02) | |
| Downtown | East Boston EEC | | | 0.01 | (0.00,0.03) | 0.02 | (0.00,0.05) | |
| Downtown | Edison | 0.01 | (0.00,0.03) | 0.01 | (0.00,0.04) | 0.02 | (0.00,0.04) | |
| Downtown | Eliot | 0.34 | (0.26,0.41) | 0.32 | (0.23,0.40) | 0.31 | (0.23,0.38) | 0.46 |
| Downtown | Gardner | 0.01 | (0.00,0.03) | 0.02 | (0.00,0.05) | 0.02 | (0.00,0.04) | |
| Downtown | Hale | 0.03 | (0.00,0.06) | 0.00 | (0.00,0.02) | 0.00 | (0.00,0.02) | |
| Downtown | Harvard/Kent | 0.06 | (0.02,0.10) | 0.06 | (0.02,0.10) | 0.06 | (0.02,0.11) | |
| Downtown | Hernandez | | | 0.02 | (0.00,0.04) | 0.01 | (0.00,0.04) | 0.02 |
| Downtown | Hurley | 0.14 | (0.09,0.20) | 0.05 | (0.02,0.09) | 0.05 | (0.02,0.10) | 0.02 |
| Downtown | J.F. Kennedy | | | 0.00 | (0.00,0.02) | 0.00 | (0.00,0.02) | |
| Downtown | Jackson/Mann | | | 0.01 | (0.00,0.03) | 0.01 | (0.00,0.03) | |
| Downtown | Kennedy Patrick | | | 0.00 | (0.00,0.02) | 0.00 | (0.00,0.02) | |
| Downtown | Mason | | | 0.01 | (0.00,0.03) | 0.01 | (0.00,0.02) | |
| Downtown | Mission Hill | 0.01 | (0.00,0.03) | 0.00 | (0.00,0.01) | 0.00 | (0.00,0.02) | 0.01 |
| Downtown | O'Donnell | | | 0.00 | (0.00,0.02) | 0.00 | (0.00,0.01) | |
| Downtown | Orchard Gardens | 0.01 | (0.00,0.03) | 0.02 | (0.00,0.04) | 0.02 | (0.00,0.04) | 0.04 |
| Downtown | Otis | 0.13 | (0.08,0.20) | 0.01 | (0.00,0.03) | 0.01 | (0.00,0.02) | |
| Downtown | Quincy | 0.23 | (0.16,0.32) | 0.32 | (0.24,0.40) | 0.32 | (0.24,0.40) | 0.36 |
| Downtown | Tobin | | | 0.02 | (0.00,0.04) | 0.02 | (0.00,0.04) | 0.02 |
| Downtown | West Zone ELC | | | 0.01 | (0.00,0.03) | 0.01 | (0.00,0.03) | |
| Downtown | Winship | 0.01 | (0.00,0.03) | 0.01 | (0.00,0.03) | 0.01 | (0.00,0.02) | |
| Downtown | Winthrop | | | 0.00 | (0.00,0.02) | | | |
| East Boston | Adams | 0.03 | (0.01,0.05) | 0.11 | (0.06,0.16) | 0.10 | (0.07,0.14) | 0.09 |
| East Boston | Baldwin | | | 0.00 | (0.00,0.01) | 0.01 | (0.00,0.02) | |
| East Boston | Blackstone | 0.02 | (0.01,0.03) | 0.01 | (0.00,0.03) | 0.02 | (0.01,0.04) | 0.03 |
| East Boston | Bradley | 0.06 | (0.03,0.08) | 0.13 | (0.09,0.16) | 0.14 | (0.10,0.17) | 0.13 |
| East Boston | East Boston EEC | 0.07 | (0.05,0.09) | 0.28 | (0.23,0.33) | 0.28 | (0.24,0.34) | 0.38 |
| East Boston | Edison | 0.01 | (0.00,0.02) | 0.01 | (0.00,0.01) | 0.01 | (0.00,0.02) | |
| East Boston | Eliot | | | 0.02 | (0.01,0.04) | 0.02 | (0.01,0.04) | 0.02 |
| East Boston | Gardner | 0.00 | (0.00,0.01) | 0.01 | (0.00,0.01) | 0.01 | (0.00,0.01) | |
| East Boston | Harvard/Kent | 0.03 | (0.01,0.06) | 0.02 | (0.01,0.03) | 0.01 | (0.00,0.03) | |
| East Boston | Hernandez | | | 0.01 | (0.00,0.02) | 0.02 | (0.01,0.03) | 0.01 |
| East Boston | Hurley | 0.42 | (0.36,0.47) | 0.01 | (0.00,0.03) | 0.02 | (0.01,0.04) | 0.01 |
| East Boston | Jackson/Mann | 0.01 | (0.00,0.02) | | | 0.00 | (0.00,0.01) | |

Continued on next page

**Table 4 – continued from previous page**

| Neighborhood | School | Naive mean | Naive (95% C.I.) | Logit mean | Logit (95% C.I.) | Mixed Logit mean | Mixed Logit (95% C.I.) | Actual |
|---|---|---|---|---|---|---|---|---|
| East Boston | Kennedy Patrick | 0.04 | (0.02,0.06) | 0.09 | (0.05,0.14) | 0.07 | (0.04,0.10) | 0.09 |
| East Boston | Mather | 0.01 | (0.00,0.02) | | | | | |
| East Boston | O'Donnell | 0.03 | (0.01,0.04) | 0.07 | (0.04,0.11) | 0.05 | (0.03,0.08) | 0.07 |
| East Boston | Orchard Gardens | 0.01 | (0.00,0.03) | | | | | |
| East Boston | Otis | 0.26 | (0.22,0.31) | 0.22 | (0.17,0.27) | 0.21 | (0.17,0.26) | 0.14 |
| East Boston | Quincy | 0.00 | (0.00,0.01) | 0.01 | (0.00,0.02) | 0.01 | (0.00,0.03) | 0.02 |
| East Boston | Winship | | | | | 0.00 | (0.00,0.01) | |
| Hyde Park | BTU | | | 0.01 | (0.00,0.03) | 0.01 | (0.00,0.03) | |
| Hyde Park | Bates | | | 0.02 | (0.00,0.03) | 0.01 | (0.00,0.03) | 0.02 |
| Hyde Park | Beethoven | 0.02 | (0.01,0.05) | 0.06 | (0.03,0.09) | 0.05 | (0.02,0.08) | 0.08 |
| Hyde Park | Channing | 0.05 | (0.02,0.08) | 0.10 | (0.06,0.14) | 0.09 | (0.05,0.14) | 0.03 |
| Hyde Park | Chittick | | | 0.05 | (0.02,0.09) | 0.05 | (0.02,0.08) | 0.07 |
| Hyde Park | Clap | | | 0.01 | (0.00,0.03) | 0.01 | (0.00,0.02) | |
| Hyde Park | Condon | 0.01 | (0.00,0.02) | 0.01 | (0.00,0.02) | 0.01 | (0.00,0.02) | |
| Hyde Park | Conley | 0.14 | (0.10,0.19) | 0.03 | (0.01,0.07) | 0.04 | (0.01,0.07) | 0.04 |
| Hyde Park | Curley | 0.01 | (0.00,0.03) | 0.01 | (0.00,0.03) | 0.01 | (0.00,0.02) | |
| Hyde Park | Dever | 0.01 | (0.00,0.03) | 0.01 | (0.00,0.02) | 0.01 | (0.00,0.03) | |
| Hyde Park | Ellison/Parks | 0.14 | (0.10,0.19) | 0.09 | (0.05,0.13) | 0.10 | (0.06,0.14) | 0.12 |
| Hyde Park | Everett | | | 0.01 | (0.00,0.02) | 0.01 | (0.00,0.02) | |
| Hyde Park | Haley | | | 0.01 | (0.00,0.03) | 0.01 | (0.00,0.03) | |
| Hyde Park | Harvard/Kent | 0.01 | (0.00,0.02) | | | | | |
| Hyde Park | Haynes | 0.02 | (0.01,0.05) | 0.00 | (0.00,0.01) | 0.00 | (0.00,0.01) | |
| Hyde Park | Henderson | 0.02 | (0.00,0.04) | 0.01 | (0.00,0.03) | 0.01 | (0.00,0.03) | |
| Hyde Park | Hernandez | | | 0.02 | (0.00,0.04) | 0.02 | (0.00,0.04) | 0.08 |
| Hyde Park | Holland | 0.01 | (0.00,0.02) | 0.01 | (0.00,0.02) | 0.01 | (0.00,0.02) | |
| Hyde Park | Holmes | | | 0.00 | (0.00,0.02) | 0.00 | (0.00,0.01) | |
| Hyde Park | Kenny | | | 0.01 | (0.00,0.03) | 0.01 | (0.00,0.02) | |
| Hyde Park | Kilmer | 0.01 | (0.00,0.02) | 0.01 | (0.00,0.03) | 0.01 | (0.00,0.03) | 0.01 |
| Hyde Park | King | 0.01 | (0.00,0.02) | | | | | |
| Hyde Park | Lee | 0.02 | (0.01,0.04) | 0.04 | (0.02,0.07) | 0.04 | (0.01,0.06) | 0.04 |
| Hyde Park | Lyndon | 0.01 | (0.00,0.02) | 0.01 | (0.00,0.03) | 0.01 | (0.00,0.03) | |
| Hyde Park | Manning | 0.01 | (0.00,0.02) | 0.00 | (0.00,0.01) | 0.00 | (0.00,0.01) | |
| Hyde Park | Mason | 0.01 | (0.00,0.02) | | | | | |
| Hyde Park | Mather | 0.02 | (0.01,0.05) | 0.01 | (0.00,0.02) | 0.01 | (0.00,0.02) | |
| Hyde Park | Mattahunt | 0.01 | (0.00,0.03) | 0.04 | (0.01,0.07) | 0.03 | (0.01,0.06) | 0.03 |
| Hyde Park | Mission Hill | | | 0.01 | (0.00,0.02) | 0.00 | (0.00,0.01) | 0.01 |
| Hyde Park | Mozart | | | 0.01 | (0.00,0.02) | 0.01 | (0.00,0.02) | |
| Hyde Park | Murphy | 0.01 | (0.00,0.03) | 0.04 | (0.02,0.07) | 0.04 | (0.01,0.08) | 0.03 |
| Hyde Park | Perry | | | 0.01 | (0.00,0.02) | 0.01 | (0.00,0.02) | |
| Hyde Park | Philbrick | 0.03 | (0.01,0.06) | 0.01 | (0.00,0.02) | 0.01 | (0.00,0.02) | 0.01 |
| Hyde Park | Roosevelt | 0.30 | (0.24,0.37) | 0.24 | (0.17,0.31) | 0.26 | (0.19,0.33) | 0.29 |
| Hyde Park | Russell | 0.01 | (0.00,0.02) | 0.01 | (0.00,0.02) | 0.01 | (0.00,0.02) | |
| Hyde Park | S. Greenwood | 0.05 | (0.02,0.08) | 0.01 | (0.00,0.03) | 0.01 | (0.00,0.03) | 0.01 |
| Hyde Park | Sumner | 0.01 | (0.00,0.02) | 0.01 | (0.00,0.03) | 0.01 | (0.00,0.03) | 0.01 |
| Hyde Park | Taylor | 0.04 | (0.01,0.06) | 0.02 | (0.00,0.04) | 0.01 | (0.00,0.03) | |
| Hyde Park | Tynan | | | 0.00 | (0.00,0.01) | 0.00 | (0.00,0.01) | |
| Hyde Park | West Zone ELC | 0.01 | (0.00,0.02) | 0.00 | (0.00,0.01) | 0.00 | (0.00,0.01) | |
| Hyde Park | Young Achievers | 0.01 | (0.00,0.03) | 0.06 | (0.03,0.10) | 0.07 | (0.03,0.10) | 0.07 |
| Jamaica Plain | BTU | 0.02 | (0.01,0.05) | 0.08 | (0.04,0.12) | 0.07 | (0.04,0.11) | 0.06 |
| Jamaica Plain | Baldwin | | | 0.02 | (0.00,0.04) | 0.02 | (0.00,0.04) | 0.02 |
| Jamaica Plain | Bates | | | 0.01 | (0.00,0.03) | 0.01 | (0.00,0.02) | |
| Jamaica Plain | Beethoven | 0.01 | (0.00,0.02) | 0.02 | (0.01,0.05) | 0.02 | (0.00,0.04) | 0.02 |
| Jamaica Plain | Blackstone | 0.01 | (0.01,0.02) | 0.02 | (0.01,0.04) | 0.02 | (0.01,0.04) | |
| Jamaica Plain | Bradley | | | | | 0.00 | (0.00,0.01) | |
| Jamaica Plain | Conley | 0.01 | (0.00,0.02) | 0.01 | (0.00,0.03) | 0.01 | (0.00,0.02) | |

Continued on next page

| | | Naive | | Logit | | Mixed Logit | | |
|---|---|---|---|---|---|---|---|---|
| Neighborhood | School | mean | (95% C.I.) | mean | (95% C.I.) | mean | (95% C.I.) | Actual |
| Jamaica Plain | Curley | 0.06 | (0.03,0.09) | 0.20 | (0.14,0.27) | 0.21 | (0.16,0.27) | 0.16 |
| Jamaica Plain | Dever | 0.01 | (0.00,0.02) | 0.00 | (0.00,0.01) | 0.00 | (0.00,0.01) | |
| Jamaica Plain | East Boston EEC | | | 0.00 | (0.00,0.01) | 0.01 | (0.00,0.02) | |
| Jamaica Plain | Edison | 0.01 | (0.00,0.02) | 0.01 | (0.00,0.03) | 0.01 | (0.00,0.03) | |
| Jamaica Plain | Eliot | | | 0.01 | (0.00,0.03) | 0.01 | (0.00,0.03) | |
| Jamaica Plain | Ellis | | | 0.02 | (0.00,0.04) | 0.02 | (0.00,0.04) | 0.01 |
| Jamaica Plain | Gardner | | | 0.01 | (0.00,0.02) | 0.01 | (0.00,0.02) | |
| Jamaica Plain | Hale | 0.29 | (0.23,0.34) | 0.02 | (0.00,0.04) | 0.02 | (0.00,0.03) | |
| Jamaica Plain | Haley | | | 0.02 | (0.00,0.04) | 0.02 | (0.00,0.04) | |
| Jamaica Plain | Harvard/Kent | 0.04 | (0.02,0.07) | 0.01 | (0.00,0.03) | 0.01 | (0.00,0.03) | |
| Jamaica Plain | Haynes | 0.08 | (0.04,0.12) | 0.01 | (0.00,0.03) | 0.02 | (0.00,0.04) | 0.01 |
| Jamaica Plain | Hernandez | 0.02 | (0.00,0.04) | 0.05 | (0.02,0.09) | 0.06 | (0.03,0.09) | 0.10 |
| Jamaica Plain | Higginson/Lewis | | | 0.01 | (0.00,0.02) | 0.01 | (0.00,0.02) | |
| Jamaica Plain | Hurley | 0.01 | (0.00,0.03) | 0.01 | (0.00,0.03) | 0.01 | (0.00,0.03) | |
| Jamaica Plain | J.F. Kennedy | 0.02 | (0.00,0.04) | 0.03 | (0.01,0.07) | 0.03 | (0.01,0.06) | 0.04 |
| Jamaica Plain | Jackson/Mann | 0.01 | (0.00,0.03) | 0.01 | (0.00,0.03) | 0.01 | (0.00,0.02) | |
| Jamaica Plain | Kilmer | | | 0.03 | (0.01,0.06) | 0.05 | (0.02,0.09) | 0.01 |
| Jamaica Plain | King | | | 0.00 | (0.00,0.01) | 0.00 | (0.00,0.01) | |
| Jamaica Plain | Lyndon | | | 0.03 | (0.01,0.05) | 0.02 | (0.01,0.05) | |
| Jamaica Plain | Manning | 0.27 | (0.21,0.34) | 0.07 | (0.03,0.11) | 0.07 | (0.03,0.11) | 0.07 |
| Jamaica Plain | Mason | | | 0.00 | (0.00,0.01) | 0.00 | (0.00,0.01) | |
| Jamaica Plain | Mather | 0.01 | (0.00,0.03) | | | | | |
| Jamaica Plain | Mendell | 0.01 | (0.00,0.03) | 0.03 | (0.01,0.06) | 0.03 | (0.01,0.05) | 0.03 |
| Jamaica Plain | Mission Hill | 0.01 | (0.01,0.01) | 0.07 | (0.04,0.12) | 0.07 | (0.04,0.11) | 0.26 |
| Jamaica Plain | Mozart | | | 0.02 | (0.00,0.04) | 0.01 | (0.00,0.03) | |
| Jamaica Plain | Orchard Gardens | 0.01 | (0.00,0.02) | 0.01 | (0.00,0.03) | 0.01 | (0.00,0.03) | |
| Jamaica Plain | Otis | 0.03 | (0.01,0.06) | 0.00 | (0.00,0.01) | 0.00 | (0.00,0.01) | |
| Jamaica Plain | Philbrick | 0.01 | (0.00,0.03) | 0.01 | (0.00,0.04) | 0.01 | (0.00,0.03) | |
| Jamaica Plain | Quincy | 0.01 | (0.00,0.03) | 0.02 | (0.01,0.04) | 0.02 | (0.01,0.05) | |
| Jamaica Plain | Sumner | 0.05 | (0.02,0.08) | 0.01 | (0.00,0.03) | 0.01 | (0.00,0.03) | |
| Jamaica Plain | Tobin | | | 0.02 | (0.00,0.04) | 0.02 | (0.01,0.04) | 0.04 |
| Jamaica Plain | Trotter | | | 0.01 | (0.00,0.02) | 0.01 | (0.00,0.02) | |
| Jamaica Plain | West Zone ELC | | | 0.05 | (0.02,0.09) | 0.07 | (0.03,0.10) | 0.06 |
| Jamaica Plain | Winship | 0.00 | (0.00,0.02) | 0.01 | (0.00,0.02) | 0.00 | (0.00,0.01) | |
| Mattapan | BTU | | | 0.01 | (0.00,0.02) | 0.01 | (0.00,0.02) | 0.01 |
| Mattapan | Bates | | | 0.00 | (0.00,0.01) | | | |
| Mattapan | Beethoven | 0.02 | (0.00,0.04) | 0.01 | (0.00,0.02) | 0.01 | (0.00,0.02) | |
| Mattapan | Blackstone | 0.01 | (0.00,0.02) | | | | | |
| Mattapan | Channing | 0.00 | (0.00,0.02) | 0.02 | (0.01,0.04) | 0.02 | (0.00,0.04) | 0.02 |
| Mattapan | Chittick | 0.02 | (0.00,0.03) | 0.04 | (0.02,0.07) | 0.04 | (0.01,0.07) | 0.02 |
| Mattapan | Clap | | | 0.02 | (0.00,0.04) | 0.01 | (0.00,0.03) | |
| Mattapan | Condon | | | 0.01 | (0.00,0.03) | 0.01 | (0.00,0.02) | 0.01 |
| Mattapan | Conley | | | 0.00 | (0.00,0.01) | | | |
| Mattapan | Curley | | | 0.01 | (0.00,0.03) | 0.01 | (0.00,0.03) | |
| Mattapan | Dever | 0.01 | (0.00,0.02) | 0.02 | (0.00,0.04) | 0.02 | (0.01,0.04) | 0.05 |
| Mattapan | Ellis | | | 0.00 | (0.00,0.01) | 0.00 | (0.00,0.01) | |
| Mattapan | Ellison/Parks | 0.13 | (0.09,0.18) | 0.13 | (0.08,0.18) | 0.15 | (0.10,0.20) | 0.26 |
| Mattapan | Everett | 0.01 | (0.00,0.03) | 0.02 | (0.00,0.04) | 0.01 | (0.00,0.03) | |
| Mattapan | Haley | 0.01 | (0.00,0.02) | 0.03 | (0.01,0.07) | 0.03 | (0.01,0.05) | 0.03 |
| Mattapan | Haynes | 0.03 | (0.01,0.04) | 0.01 | (0.00,0.02) | 0.01 | (0.00,0.03) | 0.02 |
| Mattapan | Henderson | 0.35 | (0.28,0.41) | 0.02 | (0.01,0.04) | 0.03 | (0.01,0.05) | |
| Mattapan | Hernandez | 0.02 | (0.01,0.04) | 0.04 | (0.01,0.07) | 0.04 | (0.01,0.07) | 0.07 |
| Mattapan | Higginson/Lewis | 0.01 | (0.00,0.02) | | | | | |
| Mattapan | Holland | 0.01 | (0.00,0.02) | 0.01 | (0.00,0.03) | 0.01 | (0.00,0.03) | 0.01 |
| Mattapan | Holmes | 0.01 | (0.00,0.02) | 0.01 | (0.00,0.04) | 0.01 | (0.00,0.03) | 0.01 |

Continued on next page

**Table 4 – continued from previous page**

| Neighborhood | School | Naive mean | Naive (95% C.I.) | Logit mean | Logit (95% C.I.) | Mixed Logit mean | Mixed Logit (95% C.I.) | Actual |
|---|---|---|---|---|---|---|---|---|
| Mattapan | J.F. Kennedy | 0.01 | (0.00,0.02) | 0.00 | (0.00,0.01) | | | |
| Mattapan | Kenny | | | 0.02 | (0.00,0.04) | 0.02 | (0.00,0.03) | 0.01 |
| Mattapan | Kilmer | | | | | 0.00 | (0.00,0.01) | |
| Mattapan | Lee | 0.02 | (0.01,0.04) | 0.09 | (0.05,0.14) | 0.09 | (0.05,0.13) | 0.08 |
| Mattapan | Lyndon | 0.01 | (0.00,0.03) | 0.00 | (0.00,0.01) | 0.00 | (0.00,0.01) | |
| Mattapan | Mather | 0.02 | (0.00,0.04) | 0.01 | (0.00,0.03) | 0.01 | (0.00,0.03) | 0.02 |
| Mattapan | Mattahunt | 0.04 | (0.01,0.07) | 0.04 | (0.01,0.07) | 0.03 | (0.01,0.06) | 0.03 |
| Mattapan | Mission Hill | | | 0.00 | (0.00,0.01) | 0.00 | (0.00,0.01) | |
| Mattapan | Mozart | | | 0.00 | (0.00,0.01) | | | |
| Mattapan | Murphy | 0.02 | (0.00,0.04) | 0.07 | (0.03,0.10) | 0.08 | (0.04,0.12) | 0.07 |
| Mattapan | Perry | 0.01 | (0.00,0.02) | 0.01 | (0.00,0.03) | 0.01 | (0.00,0.03) | 0.01 |
| Mattapan | Philbrick | 0.06 | (0.03,0.10) | 0.00 | (0.00,0.02) | 0.00 | (0.00,0.01) | |
| Mattapan | Roosevelt | 0.01 | (0.00,0.02) | 0.04 | (0.01,0.06) | 0.03 | (0.01,0.06) | 0.02 |
| Mattapan | Russell | 0.01 | (0.00,0.03) | 0.01 | (0.00,0.04) | 0.01 | (0.00,0.03) | 0.01 |
| Mattapan | S. Greenwood | 0.07 | (0.04,0.10) | 0.04 | (0.02,0.07) | 0.04 | (0.01,0.07) | 0.03 |
| Mattapan | Sumner | 0.05 | (0.02,0.08) | 0.01 | (0.00,0.02) | 0.01 | (0.00,0.02) | 0.02 |
| Mattapan | Taylor | 0.07 | (0.04,0.10) | 0.04 | (0.01,0.07) | 0.03 | (0.01,0.06) | 0.04 |
| Mattapan | Tynan | | | 0.00 | (0.00,0.02) | 0.00 | (0.00,0.01) | |
| Mattapan | West Zone ELC | | | 0.00 | (0.00,0.01) | 0.00 | (0.00,0.01) | |
| Mattapan | Winship | 0.01 | (0.00,0.02) | | | | | |
| Mattapan | Young Achievers | 0.02 | (0.01,0.04) | 0.17 | (0.12,0.23) | 0.19 | (0.14,0.25) | 0.11 |
| North Dorchester | Baldwin | | | 0.00 | (0.00,0.02) | 0.00 | (0.00,0.01) | |
| North Dorchester | Blackstone | | | 0.01 | (0.00,0.03) | 0.01 | (0.00,0.03) | |
| North Dorchester | Bradley | | | | | 0.00 | (0.00,0.01) | |
| North Dorchester | Channing | | | 0.00 | (0.00,0.01) | 0.00 | (0.00,0.02) | |
| North Dorchester | Chittick | | | 0.00 | (0.00,0.02) | 0.00 | (0.00,0.02) | |
| North Dorchester | Clap | 0.02 | (0.01,0.05) | 0.11 | (0.05,0.16) | 0.10 | (0.05,0.15) | 0.06 |
| North Dorchester | Condon | | | 0.03 | (0.01,0.07) | 0.02 | (0.00,0.05) | 0.04 |
| North Dorchester | Dever | 0.04 | (0.01,0.08) | 0.07 | (0.03,0.11) | 0.07 | (0.03,0.11) | 0.10 |
| North Dorchester | East Boston EEC | | | | | 0.00 | (0.00,0.02) | |
| North Dorchester | Edison | | | 0.00 | (0.00,0.01) | 0.00 | (0.00,0.01) | |
| North Dorchester | Eliot | | | 0.01 | (0.00,0.02) | 0.00 | (0.00,0.01) | |
| North Dorchester | Ellison/Parks | 0.09 | (0.04,0.13) | 0.02 | (0.00,0.05) | 0.03 | (0.01,0.06) | 0.03 |
| North Dorchester | Everett | 0.06 | (0.03,0.10) | 0.09 | (0.04,0.13) | 0.09 | (0.04,0.14) | 0.12 |
| North Dorchester | Gardner | 0.01 | (0.00,0.03) | 0.00 | (0.00,0.02) | 0.00 | (0.00,0.01) | |
| North Dorchester | Harvard/Kent | | | 0.00 | (0.00,0.01) | | | |
| North Dorchester | Haynes | 0.15 | (0.10,0.22) | 0.06 | (0.02,0.10) | 0.07 | (0.04,0.12) | 0.05 |
| North Dorchester | Henderson | 0.08 | (0.04,0.12) | 0.03 | (0.01,0.06) | 0.03 | (0.01,0.06) | 0.01 |
| North Dorchester | Hernandez | | | 0.02 | (0.00,0.05) | 0.02 | (0.00,0.04) | 0.03 |
| North Dorchester | Higginson/Lewis | | | 0.00 | (0.00,0.01) | | | |
| North Dorchester | Holland | | | 0.03 | (0.01,0.06) | 0.03 | (0.01,0.05) | 0.01 |
| North Dorchester | Holmes | | | 0.01 | (0.00,0.02) | 0.01 | (0.00,0.02) | |
| North Dorchester | Hurley | | | 0.01 | (0.00,0.02) | 0.01 | (0.00,0.02) | |
| North Dorchester | Jackson/Mann | | | 0.00 | (0.00,0.01) | | | |
| North Dorchester | Kenny | | | 0.01 | (0.00,0.03) | 0.01 | (0.00,0.03) | |
| North Dorchester | King | | | 0.01 | (0.00,0.03) | 0.01 | (0.00,0.03) | |
| North Dorchester | Lee | 0.02 | (0.00,0.03) | 0.03 | (0.01,0.06) | 0.03 | (0.01,0.06) | 0.03 |
| North Dorchester | Mason | 0.16 | (0.10,0.23) | 0.02 | (0.00,0.05) | 0.02 | (0.00,0.05) | 0.04 |
| North Dorchester | Mather | 0.11 | (0.06,0.16) | 0.08 | (0.04,0.13) | 0.09 | (0.05,0.14) | 0.10 |
| North Dorchester | Mattahunt | 0.01 | (0.00,0.03) | 0.00 | (0.00,0.02) | 0.00 | (0.00,0.02) | |
| North Dorchester | Murphy | 0.06 | (0.03,0.10) | 0.11 | (0.07,0.17) | 0.13 | (0.07,0.18) | 0.14 |
| North Dorchester | Orchard Gardens | 0.02 | (0.00,0.04) | 0.01 | (0.00,0.03) | 0.01 | (0.00,0.03) | 0.03 |
| North Dorchester | Otis | 0.04 | (0.01,0.08) | | | 0.00 | (0.00,0.01) | |
| North Dorchester | Perry | | | 0.04 | (0.01,0.07) | 0.03 | (0.01,0.07) | 0.02 |
| North Dorchester | Quincy | 0.01 | (0.00,0.03) | 0.01 | (0.00,0.03) | 0.01 | (0.00,0.03) | |

Continued on next page

**Table 4 – continued from previous page**

| | | Naive | | Logit | | Mixed Logit | | |
|---|---|---|---|---|---|---|---|---|
| Neighborhood | School | mean | (95% C.I.) | mean | (95% C.I.) | mean | (95% C.I.) | Actual |
| North Dorchester | Roosevelt | 0.01 | (0.00,0.03) | 0.01 | (0.00,0.02) | 0.01 | (0.00,0.04) | 0.01 |
| North Dorchester | Russell | 0.06 | (0.02,0.10) | 0.07 | (0.04,0.12) | 0.08 | (0.04,0.13) | 0.06 |
| North Dorchester | S. Greenwood | 0.03 | (0.00,0.06) | 0.01 | (0.00,0.03) | 0.01 | (0.00,0.03) | 0.02 |
| North Dorchester | Taylor | | | 0.00 | (0.00,0.02) | 0.00 | (0.00,0.01) | |
| North Dorchester | Tobin | | | 0.00 | (0.00,0.01) | | | |
| North Dorchester | Tynan | 0.01 | (0.00,0.03) | 0.01 | (0.00,0.04) | 0.01 | (0.00,0.03) | 0.01 |
| North Dorchester | Winship | | | 0.00 | (0.00,0.01) | | | |
| North Dorchester | Winthrop | 0.01 | (0.00,0.03) | 0.01 | (0.00,0.04) | 0.01 | (0.00,0.03) | |
| North Dorchester | Young Achievers | | | 0.02 | (0.00,0.04) | 0.02 | (0.00,0.04) | 0.02 |
| Roslindale | BTU | 0.02 | (0.01,0.04) | 0.11 | (0.07,0.15) | 0.11 | (0.08,0.15) | 0.13 |
| Roslindale | Bates | 0.03 | (0.01,0.05) | 0.07 | (0.04,0.10) | 0.07 | (0.04,0.10) | 0.08 |
| Roslindale | Beethoven | 0.03 | (0.01,0.06) | 0.09 | (0.06,0.12) | 0.09 | (0.05,0.12) | 0.07 |
| Roslindale | Channing | | | 0.00 | (0.00,0.01) | 0.00 | (0.00,0.01) | |
| Roslindale | Chittick | | | 0.01 | (0.00,0.01) | 0.00 | (0.00,0.01) | |
| Roslindale | Conley | 0.16 | (0.12,0.20) | 0.05 | (0.03,0.09) | 0.05 | (0.03,0.08) | 0.02 |
| Roslindale | Curley | 0.02 | (0.00,0.03) | 0.05 | (0.03,0.09) | 0.05 | (0.03,0.08) | 0.02 |
| Roslindale | Ellis | 0.01 | (0.00,0.02) | 0.01 | (0.00,0.02) | 0.01 | (0.00,0.02) | |
| Roslindale | Ellison/Parks | 0.01 | (0.00,0.02) | | | | | |
| Roslindale | Hale | 0.00 | (0.00,0.01) | 0.00 | (0.00,0.01) | 0.00 | (0.00,0.01) | |
| Roslindale | Haley | 0.05 | (0.02,0.08) | 0.06 | (0.03,0.09) | 0.06 | (0.03,0.09) | 0.08 |
| Roslindale | Harvard/Kent | 0.00 | (0.00,0.01) | | | | | |
| Roslindale | Haynes | 0.10 | (0.07,0.14) | 0.01 | (0.00,0.03) | 0.02 | (0.01,0.04) | 0.03 |
| Roslindale | Hernandez | 0.02 | (0.00,0.04) | 0.03 | (0.01,0.05) | 0.03 | (0.01,0.05) | 0.07 |
| Roslindale | J.F. Kennedy | 0.01 | (0.00,0.02) | 0.01 | (0.00,0.02) | 0.01 | (0.00,0.02) | |
| Roslindale | Kenny | 0.00 | (0.00,0.01) | | | | | |
| Roslindale | Kilmer | 0.01 | (0.00,0.03) | 0.09 | (0.06,0.13) | 0.12 | (0.08,0.17) | 0.05 |
| Roslindale | Lyndon | 0.04 | (0.02,0.07) | 0.09 | (0.06,0.13) | 0.07 | (0.05,0.11) | 0.10 |
| Roslindale | Manning | 0.01 | (0.00,0.02) | 0.04 | (0.02,0.07) | 0.04 | (0.02,0.06) | |
| Roslindale | Mattahunt | | | 0.01 | (0.00,0.02) | 0.01 | (0.00,0.02) | |
| Roslindale | Mendell | 0.01 | (0.00,0.03) | 0.01 | (0.00,0.02) | 0.01 | (0.00,0.02) | |
| Roslindale | Mission Hill | | | 0.04 | (0.02,0.06) | 0.03 | (0.01,0.05) | 0.06 |
| Roslindale | Mozart | 0.01 | (0.00,0.03) | 0.07 | (0.04,0.10) | 0.07 | (0.04,0.10) | 0.06 |
| Roslindale | Philbrick | 0.14 | (0.10,0.18) | 0.05 | (0.02,0.09) | 0.04 | (0.02,0.07) | 0.05 |
| Roslindale | Roosevelt | | | 0.01 | (0.00,0.02) | 0.01 | (0.00,0.02) | |
| Roslindale | Sumner | 0.29 | (0.23,0.34) | 0.06 | (0.03,0.09) | 0.07 | (0.04,0.11) | 0.09 |
| Roslindale | Taylor | 0.01 | (0.00,0.02) | | | | | |
| Roslindale | Trotter | | | 0.00 | (0.00,0.01) | 0.00 | (0.00,0.01) | |
| Roslindale | West Zone ELC | | | 0.01 | (0.00,0.03) | 0.01 | (0.00,0.03) | 0.02 |
| Roslindale | Young Achievers | | | 0.00 | (0.00,0.01) | 0.01 | (0.00,0.01) | |
| Roxbury | BTU | 0.01 | (0.00,0.02) | 0.04 | (0.02,0.06) | 0.03 | (0.01,0.06) | 0.03 |
| Roxbury | Baldwin | 0.01 | (0.01,0.01) | 0.01 | (0.00,0.02) | 0.01 | (0.00,0.02) | 0.02 |
| Roxbury | Bates | | | 0.01 | (0.00,0.02) | 0.01 | (0.00,0.02) | |
| Roxbury | Beethoven | 0.01 | (0.00,0.02) | 0.02 | (0.01,0.03) | 0.02 | (0.01,0.04) | |
| Roxbury | Blackstone | 0.02 | (0.01,0.03) | 0.03 | (0.01,0.04) | 0.02 | (0.01,0.04) | |
| Roxbury | Channing | 0.01 | (0.00,0.02) | 0.00 | (0.00,0.01) | | | |
| Roxbury | Clap | | | 0.02 | (0.00,0.03) | 0.01 | (0.00,0.03) | |
| Roxbury | Condon | | | 0.00 | (0.00,0.01) | | | |
| Roxbury | Conley | 0.01 | (0.00,0.01) | 0.01 | (0.00,0.02) | 0.01 | (0.00,0.01) | |
| Roxbury | Curley | 0.02 | (0.01,0.04) | 0.09 | (0.06,0.12) | 0.09 | (0.06,0.12) | 0.03 |
| Roxbury | Dever | 0.01 | (0.00,0.01) | 0.01 | (0.00,0.02) | 0.01 | (0.00,0.01) | |
| Roxbury | East Boston EEC | | | | | 0.01 | (0.00,0.02) | |
| Roxbury | Edison | | | 0.00 | (0.00,0.01) | 0.00 | (0.00,0.01) | |
| Roxbury | Eliot | 0.01 | (0.00,0.01) | 0.01 | (0.00,0.02) | 0.01 | (0.00,0.02) | |
| Roxbury | Ellis | 0.02 | (0.01,0.04) | 0.04 | (0.02,0.07) | 0.04 | (0.02,0.07) | 0.02 |
| Roxbury | Ellison/Parks | 0.01 | (0.00,0.02) | 0.01 | (0.00,0.01) | 0.01 | (0.00,0.02) | 0.03 |

Continued on next page

**Table 4 – continued from previous page**

| Neighborhood | School | Naive mean | Naive (95% C.I.) | Logit mean | Logit (95% C.I.) | Mixed Logit mean | Mixed Logit (95% C.I.) | Actual |
|---|---|---|---|---|---|---|---|---|
| Roxbury | Everett | | | 0.02 | (0.01,0.03) | 0.02 | (0.00,0.03) | |
| Roxbury | Gardner | 0.01 | (0.00,0.01) | 0.00 | (0.00,0.01) | | | |
| Roxbury | Hale | 0.23 | (0.18,0.27) | 0.02 | (0.01,0.04) | 0.02 | (0.01,0.04) | 0.02 |
| Roxbury | Haley | 0.00 | (0.00,0.01) | 0.01 | (0.00,0.03) | 0.01 | (0.00,0.02) | 0.03 |
| Roxbury | Haynes | 0.12 | (0.08,0.15) | 0.08 | (0.05,0.11) | 0.11 | (0.08,0.14) | 0.16 |
| Roxbury | Henderson | 0.06 | (0.03,0.08) | 0.00 | (0.00,0.01) | 0.00 | (0.00,0.01) | |
| Roxbury | Hernandez | 0.02 | (0.01,0.04) | 0.07 | (0.04,0.10) | 0.08 | (0.05,0.11) | 0.08 |
| Roxbury | Higginson/Lewis | 0.01 | (0.00,0.02) | 0.02 | (0.01,0.03) | 0.01 | (0.00,0.03) | 0.02 |
| Roxbury | Holland | 0.01 | (0.00,0.01) | 0.02 | (0.01,0.03) | 0.02 | (0.01,0.03) | 0.02 |
| Roxbury | Holmes | 0.01 | (0.00,0.01) | 0.01 | (0.00,0.02) | 0.01 | (0.00,0.02) | |
| Roxbury | Hurley | 0.02 | (0.01,0.04) | 0.02 | (0.01,0.03) | 0.02 | (0.00,0.03) | |
| Roxbury | J.F. Kennedy | 0.02 | (0.01,0.04) | 0.02 | (0.01,0.04) | 0.02 | (0.01,0.04) | 0.03 |
| Roxbury | Jackson/Mann | 0.01 | (0.00,0.02) | 0.00 | (0.00,0.01) | | | |
| Roxbury | Kenny | | | 0.00 | (0.00,0.01) | | | |
| Roxbury | Kilmer | | | 0.01 | (0.00,0.02) | 0.02 | (0.01,0.03) | 0.01 |
| Roxbury | King | 0.01 | (0.00,0.02) | 0.02 | (0.01,0.03) | 0.01 | (0.00,0.03) | |
| Roxbury | Lee | 0.01 | (0.01,0.02) | 0.03 | (0.01,0.04) | 0.03 | (0.01,0.05) | 0.02 |
| Roxbury | Lyndon | 0.01 | (0.00,0.02) | 0.02 | (0.00,0.03) | 0.01 | (0.00,0.03) | 0.02 |
| Roxbury | Manning | | | 0.01 | (0.00,0.03) | 0.01 | (0.00,0.03) | |
| Roxbury | Mason | 0.06 | (0.04,0.09) | 0.02 | (0.01,0.03) | 0.02 | (0.01,0.04) | 0.04 |
| Roxbury | Mather | 0.01 | (0.00,0.02) | 0.01 | (0.00,0.03) | 0.01 | (0.00,0.03) | |
| Roxbury | Mattahunt | 0.01 | (0.00,0.02) | 0.00 | (0.00,0.01) | | | |
| Roxbury | Mendell | 0.01 | (0.00,0.03) | 0.03 | (0.01,0.04) | 0.02 | (0.01,0.04) | |
| Roxbury | Mission Hill | | | 0.03 | (0.01,0.05) | 0.03 | (0.01,0.04) | 0.05 |
| Roxbury | Mozart | | | 0.01 | (0.00,0.02) | 0.01 | (0.00,0.02) | |
| Roxbury | Murphy | 0.01 | (0.00,0.01) | 0.01 | (0.00,0.02) | 0.01 | (0.00,0.03) | |
| Roxbury | Orchard Gardens | 0.01 | (0.00,0.03) | 0.02 | (0.01,0.05) | 0.02 | (0.01,0.04) | 0.06 |
| Roxbury | Otis | 0.04 | (0.02,0.06) | | | | | |
| Roxbury | Philbrick | 0.01 | (0.00,0.02) | 0.01 | (0.00,0.02) | 0.01 | (0.00,0.02) | |
| Roxbury | Quincy | 0.01 | (0.00,0.02) | 0.01 | (0.00,0.02) | 0.01 | (0.00,0.03) | 0.03 |
| Roxbury | Roosevelt | | | 0.00 | (0.00,0.01) | 0.00 | (0.00,0.01) | |
| Roxbury | Russell | | | 0.02 | (0.01,0.03) | 0.02 | (0.01,0.04) | |
| Roxbury | S. Greenwood | 0.01 | (0.00,0.03) | 0.02 | (0.01,0.04) | 0.02 | (0.01,0.04) | 0.02 |
| Roxbury | Sumner | 0.07 | (0.04,0.10) | 0.01 | (0.00,0.02) | 0.01 | (0.00,0.02) | |
| Roxbury | Taylor | 0.01 | (0.00,0.02) | 0.00 | (0.00,0.01) | 0.00 | (0.00,0.01) | |
| Roxbury | Tobin | 0.01 | (0.00,0.01) | 0.01 | (0.00,0.03) | 0.01 | (0.00,0.03) | 0.01 |
| Roxbury | Trotter | 0.03 | (0.01,0.04) | 0.02 | (0.00,0.04) | 0.02 | (0.01,0.04) | 0.05 |
| Roxbury | West Zone ELC | | | 0.03 | (0.01,0.05) | 0.04 | (0.02,0.06) | 0.04 |
| Roxbury | Winthrop | 0.02 | (0.01,0.04) | 0.02 | (0.00,0.03) | 0.01 | (0.00,0.03) | 0.02 |
| Roxbury | Young Achievers | 0.01 | (0.00,0.02) | 0.02 | (0.00,0.03) | 0.02 | (0.00,0.03) | 0.02 |
| South Boston | Adams | | | | | 0.00 | (0.00,0.01) | |
| South Boston | Baldwin | | | | | 0.00 | (0.00,0.01) | |
| South Boston | Blackstone | | | 0.03 | (0.00,0.08) | 0.03 | (0.00,0.07) | |
| South Boston | Bradley | | | | | 0.00 | (0.00,0.01) | |
| South Boston | Channing | | | 0.00 | (0.00,0.01) | 0.00 | (0.00,0.03) | |
| South Boston | Chittick | | | 0.00 | (0.00,0.02) | 0.00 | (0.00,0.02) | 0.01 |
| South Boston | Clap | | | 0.07 | (0.02,0.14) | 0.07 | (0.02,0.12) | 0.06 |
| South Boston | Condon | 0.05 | (0.01,0.10) | 0.14 | (0.07,0.22) | 0.13 | (0.05,0.20) | 0.11 |
| South Boston | Dever | 0.04 | (0.00,0.08) | 0.08 | (0.03,0.15) | 0.09 | (0.03,0.16) | 0.01 |
| South Boston | East Boston EEC | | | 0.00 | (0.00,0.01) | 0.00 | (0.00,0.01) | |
| South Boston | Edison | | | 0.00 | (0.00,0.01) | 0.00 | (0.00,0.01) | |
| South Boston | Eliot | | | 0.01 | (0.00,0.03) | 0.01 | (0.00,0.03) | 0.01 |
| South Boston | Ellison/Parks | 0.07 | (0.02,0.13) | 0.01 | (0.00,0.04) | 0.02 | (0.00,0.05) | 0.04 |
| South Boston | Everett | | | 0.03 | (0.00,0.06) | 0.02 | (0.00,0.06) | 0.01 |
| South Boston | Gardner | | | 0.00 | (0.00,0.01) | 0.00 | (0.00,0.01) | |

Continued on next page

Table 4 – continued from previous page

| Neighborhood | School | Naive mean | Naive (95% C.I.) | Logit mean | Logit (95% C.I.) | Mixed Logit mean | Mixed Logit (95% C.I.) | Actual |
|---|---|---|---|---|---|---|---|---|
| South Boston | Harvard/Kent | 0.02 | (0.00,0.07) | 0.00 | (0.00,0.03) | 0.01 | (0.00,0.03) | 0.03 |
| South Boston | Henderson | 0.05 | (0.01,0.10) | 0.02 | (0.00,0.05) | 0.01 | (0.00,0.04) | 0.03 |
| South Boston | Hernandez | | | 0.02 | (0.00,0.06) | 0.02 | (0.00,0.05) | |
| South Boston | Holland | 0.01 | (0.00,0.04) | 0.01 | (0.00,0.03) | 0.01 | (0.00,0.03) | 0.01 |
| South Boston | Holmes | | | 0.00 | (0.00,0.02) | 0.00 | (0.00,0.02) | |
| South Boston | Hurley | 0.01 | (0.00,0.04) | 0.00 | (0.00,0.02) | 0.00 | (0.00,0.02) | |
| South Boston | Jackson/Mann | | | 0.00 | (0.00,0.01) | | | |
| South Boston | Kenny | | | 0.01 | (0.00,0.03) | 0.01 | (0.00,0.03) | |
| South Boston | Lee | 0.03 | (0.00,0.06) | 0.02 | (0.00,0.05) | 0.02 | (0.00,0.05) | 0.03 |
| South Boston | Mason | 0.05 | (0.01,0.10) | 0.01 | (0.00,0.04) | 0.01 | (0.00,0.04) | |
| South Boston | Mather | 0.02 | (0.00,0.06) | 0.02 | (0.00,0.05) | 0.02 | (0.00,0.04) | |
| South Boston | Mattahunt | 0.01 | (0.00,0.04) | 0.00 | (0.00,0.02) | 0.00 | (0.00,0.01) | |
| South Boston | Murphy | 0.31 | (0.21,0.40) | 0.07 | (0.02,0.14) | 0.07 | (0.01,0.13) | 0.03 |
| South Boston | Orchard Gardens | | | 0.00 | (0.00,0.01) | 0.00 | (0.00,0.01) | |
| South Boston | Otis | 0.01 | (0.00,0.04) | | | 0.00 | (0.00,0.01) | |
| South Boston | Perry | 0.07 | (0.01,0.12) | 0.20 | (0.12,0.30) | 0.23 | (0.14,0.34) | 0.37 |
| South Boston | Quincy | 0.09 | (0.04,0.16) | 0.06 | (0.01,0.12) | 0.06 | (0.01,0.12) | 0.09 |
| South Boston | Roosevelt | | | 0.00 | (0.00,0.02) | 0.01 | (0.00,0.04) | 0.03 |
| South Boston | Russell | 0.01 | (0.00,0.04) | 0.05 | (0.01,0.10) | 0.04 | (0.00,0.10) | 0.03 |
| South Boston | S. Greenwood | 0.08 | (0.04,0.15) | 0.01 | (0.00,0.04) | 0.01 | (0.00,0.04) | 0.03 |
| South Boston | Taylor | | | 0.00 | (0.00,0.01) | 0.00 | (0.00,0.01) | |
| South Boston | Tobin | | | 0.00 | (0.00,0.01) | | | |
| South Boston | Tynan | 0.06 | (0.01,0.11) | 0.07 | (0.02,0.14) | 0.07 | (0.01,0.12) | 0.03 |
| South Boston | Young Achievers | | | 0.02 | (0.00,0.05) | 0.02 | (0.00,0.05) | 0.03 |
| South Dorchester | Channing | 0.01 | (0.00,0.01) | 0.01 | (0.00,0.02) | 0.01 | (0.00,0.02) | |
| South Dorchester | Chittick | | | 0.01 | (0.00,0.02) | 0.01 | (0.00,0.02) | |
| South Dorchester | Clap | | | 0.03 | (0.02,0.05) | 0.03 | (0.01,0.04) | 0.02 |
| South Dorchester | Condon | 0.01 | (0.00,0.02) | 0.02 | (0.01,0.04) | 0.01 | (0.00,0.03) | 0.03 |
| South Dorchester | Dever | 0.01 | (0.00,0.03) | 0.03 | (0.01,0.04) | 0.03 | (0.01,0.05) | 0.01 |
| South Dorchester | Ellison/Parks | 0.10 | (0.07,0.12) | 0.04 | (0.02,0.06) | 0.06 | (0.04,0.08) | 0.07 |
| South Dorchester | Everett | 0.01 | (0.00,0.03) | 0.04 | (0.02,0.06) | 0.03 | (0.01,0.05) | 0.03 |
| South Dorchester | Haynes | 0.05 | (0.03,0.07) | 0.02 | (0.01,0.03) | 0.02 | (0.01,0.04) | 0.02 |
| South Dorchester | Henderson | 0.33 | (0.29,0.38) | 0.07 | (0.05,0.10) | 0.07 | (0.05,0.10) | 0.09 |
| South Dorchester | Hernandez | | | 0.03 | (0.01,0.04) | 0.02 | (0.01,0.04) | 0.02 |
| South Dorchester | Holland | 0.04 | (0.02,0.06) | 0.05 | (0.03,0.07) | 0.05 | (0.03,0.07) | 0.05 |
| South Dorchester | Holmes | 0.01 | (0.00,0.02) | 0.02 | (0.01,0.03) | 0.02 | (0.01,0.04) | 0.02 |
| South Dorchester | Kenny | 0.03 | (0.01,0.05) | 0.03 | (0.01,0.05) | 0.04 | (0.02,0.06) | 0.04 |
| South Dorchester | King | | | 0.01 | (0.00,0.01) | 0.01 | (0.00,0.02) | |
| South Dorchester | Lee | 0.04 | (0.03,0.06) | 0.09 | (0.07,0.13) | 0.09 | (0.06,0.12) | 0.10 |
| South Dorchester | Mason | 0.01 | (0.00,0.02) | | | | | |
| South Dorchester | Mather | 0.10 | (0.07,0.13) | 0.07 | (0.04,0.09) | 0.07 | (0.04,0.10) | 0.07 |
| South Dorchester | Mattahunt | 0.01 | (0.00,0.02) | 0.01 | (0.00,0.02) | 0.01 | (0.00,0.02) | |
| South Dorchester | Murphy | 0.15 | (0.11,0.18) | 0.25 | (0.21,0.30) | 0.27 | (0.22,0.32) | 0.27 |
| South Dorchester | Perry | | | 0.02 | (0.01,0.04) | 0.02 | (0.01,0.04) | |
| South Dorchester | Roosevelt | 0.01 | (0.00,0.01) | 0.01 | (0.00,0.03) | 0.02 | (0.01,0.04) | 0.01 |
| South Dorchester | Russell | 0.01 | (0.00,0.01) | 0.02 | (0.01,0.04) | 0.02 | (0.01,0.04) | 0.02 |
| South Dorchester | S. Greenwood | 0.04 | (0.02,0.06) | 0.03 | (0.01,0.05) | 0.03 | (0.02,0.05) | 0.02 |
| South Dorchester | Taylor | 0.01 | (0.00,0.02) | 0.01 | (0.00,0.03) | 0.01 | (0.00,0.03) | |
| South Dorchester | Tynan | 0.01 | (0.00,0.03) | 0.01 | (0.00,0.02) | 0.01 | (0.00,0.01) | 0.02 |
| South Dorchester | Winthrop | | | 0.00 | (0.00,0.01) | | | |
| South Dorchester | Young Achievers | | | 0.04 | (0.02,0.07) | 0.04 | (0.03,0.07) | 0.05 |
| South End | Adams | | | 0.00 | (0.00,0.01) | 0.00 | (0.00,0.02) | |
| South End | Baldwin | 0.03 | (0.00,0.06) | 0.04 | (0.00,0.07) | 0.04 | (0.01,0.08) | 0.05 |
| South End | Blackstone | 0.03 | (0.01,0.07) | 0.14 | (0.08,0.21) | 0.13 | (0.07,0.20) | 0.11 |
| South End | Bradley | | | 0.00 | (0.00,0.02) | 0.01 | (0.00,0.03) | |

Continued on next page

**Table 4 – continued from previous page**

| Neighborhood | School | Naive mean | Naive (95% C.I.) | Logit mean | Logit (95% C.I.) | Mixed Logit mean | Mixed Logit (95% C.I.) | Actual |
|---|---|---|---|---|---|---|---|---|
| South End | Channing | 0.01 | (0.00,0.03) | | | | | |
| South End | Condon | | | 0.02 | (0.00,0.04) | 0.01 | (0.00,0.04) | |
| South End | East Boston EEC | | | 0.01 | (0.00,0.04) | 0.02 | (0.00,0.05) | |
| South End | Edison | 0.03 | (0.00,0.06) | 0.02 | (0.00,0.04) | 0.02 | (0.00,0.05) | |
| South End | Eliot | 0.03 | (0.01,0.06) | 0.09 | (0.04,0.14) | 0.08 | (0.04,0.13) | 0.11 |
| South End | Gardner | 0.02 | (0.00,0.05) | 0.02 | (0.00,0.05) | 0.02 | (0.00,0.04) | 0.04 |
| South End | Hale | | | 0.01 | (0.00,0.03) | 0.01 | (0.00,0.04) | 0.02 |
| South End | Harvard/Kent | 0.05 | (0.01,0.09) | 0.03 | (0.00,0.06) | 0.02 | (0.00,0.05) | |
| South End | Hernandez | 0.01 | (0.00,0.03) | 0.03 | (0.00,0.07) | 0.03 | (0.01,0.07) | |
| South End | Higginson/Lewis | | | 0.00 | (0.00,0.02) | 0.00 | (0.00,0.02) | |
| South End | Hurley | 0.43 | (0.33,0.52) | 0.13 | (0.06,0.20) | 0.14 | (0.08,0.20) | 0.25 |
| South End | Jackson/Mann | | | 0.01 | (0.00,0.04) | 0.01 | (0.00,0.03) | |
| South End | Kennedy Patrick | | | 0.00 | (0.00,0.02) | 0.00 | (0.00,0.02) | |
| South End | Mason | 0.01 | (0.00,0.02) | 0.03 | (0.00,0.06) | 0.03 | (0.00,0.06) | 0.03 |
| South End | Mission Hill | 0.02 | (0.00,0.04) | 0.01 | (0.00,0.02) | 0.01 | (0.00,0.02) | 0.03 |
| South End | O'Donnell | | | 0.00 | (0.00,0.02) | 0.00 | (0.00,0.01) | |
| South End | Orchard Gardens | 0.04 | (0.01,0.08) | 0.06 | (0.02,0.11) | 0.05 | (0.02,0.09) | 0.03 |
| South End | Otis | 0.10 | (0.05,0.16) | 0.01 | (0.00,0.02) | 0.01 | (0.00,0.03) | |
| South End | Quincy | 0.16 | (0.10,0.23) | 0.29 | (0.22,0.37) | 0.30 | (0.21,0.39) | 0.31 |
| South End | S. Greenwood | 0.01 | (0.00,0.03) | | | | | |
| South End | Tobin | 0.02 | (0.00,0.05) | 0.03 | (0.01,0.07) | 0.03 | (0.00,0.07) | |
| South End | Tynan | | | | | 0.00 | (0.00,0.01) | |
| South End | Winship | | | 0.01 | (0.00,0.03) | 0.01 | (0.00,0.03) | |
| South End | Winthrop | | | 0.01 | (0.00,0.02) | 0.00 | (0.00,0.02) | |
| West Roxbury | BTU | 0.00 | (0.00,0.01) | 0.03 | (0.01,0.05) | 0.03 | (0.01,0.05) | 0.03 |
| West Roxbury | Bates | 0.02 | (0.00,0.04) | 0.04 | (0.01,0.06) | 0.03 | (0.01,0.06) | 0.03 |
| West Roxbury | Beethoven | 0.07 | (0.04,0.10) | 0.18 | (0.13,0.23) | 0.17 | (0.13,0.22) | 0.20 |
| West Roxbury | Channing | | | 0.02 | (0.00,0.03) | 0.02 | (0.01,0.04) | 0.01 |
| West Roxbury | Conley | 0.01 | (0.00,0.03) | 0.02 | (0.00,0.04) | 0.01 | (0.00,0.03) | 0.01 |
| West Roxbury | Curley | 0.02 | (0.00,0.04) | 0.02 | (0.01,0.04) | 0.02 | (0.01,0.04) | |
| West Roxbury | Ellis | | | 0.00 | (0.00,0.01) | 0.00 | (0.00,0.01) | |
| West Roxbury | Haley | 0.00 | (0.00,0.01) | 0.01 | (0.00,0.03) | 0.01 | (0.00,0.02) | 0.01 |
| West Roxbury | Harvard/Kent | 0.02 | (0.01,0.04) | | | | | |
| West Roxbury | Haynes | 0.12 | (0.08,0.16) | 0.01 | (0.00,0.02) | 0.02 | (0.00,0.03) | 0.03 |
| West Roxbury | Hernandez | 0.00 | (0.00,0.02) | 0.01 | (0.00,0.03) | 0.01 | (0.00,0.03) | 0.03 |
| West Roxbury | Higginson/Lewis | 0.00 | (0.00,0.02) | | | | | |
| West Roxbury | J.F. Kennedy | 0.00 | (0.00,0.02) | 0.00 | (0.00,0.01) | | | |
| West Roxbury | Kilmer | 0.20 | (0.15,0.25) | 0.31 | (0.25,0.37) | 0.36 | (0.30,0.43) | 0.33 |
| West Roxbury | Lyndon | 0.38 | (0.33,0.44) | 0.21 | (0.15,0.26) | 0.19 | (0.14,0.23) | 0.21 |
| West Roxbury | Manning | 0.03 | (0.01,0.05) | 0.03 | (0.01,0.05) | 0.02 | (0.01,0.04) | 0.01 |
| West Roxbury | Mather | 0.01 | (0.00,0.03) | | | | | |
| West Roxbury | Mendell | 0.00 | (0.00,0.01) | 0.00 | (0.00,0.01) | 0.00 | (0.00,0.01) | |
| West Roxbury | Mission Hill | | | 0.01 | (0.00,0.03) | 0.01 | (0.00,0.03) | 0.02 |
| West Roxbury | Mozart | 0.01 | (0.00,0.03) | 0.05 | (0.03,0.09) | 0.04 | (0.02,0.07) | 0.04 |
| West Roxbury | Philbrick | 0.01 | (0.00,0.02) | 0.01 | (0.00,0.03) | 0.01 | (0.00,0.02) | 0.01 |
| West Roxbury | Sumner | 0.06 | (0.03,0.09) | 0.02 | (0.00,0.03) | 0.02 | (0.00,0.04) | 0.01 |
| West Roxbury | West Zone ELC | | | 0.01 | (0.00,0.02) | 0.01 | (0.00,0.02) | 0.01 |
| West Roxbury | Young Achievers | 0.00 | (0.00,0.01) | | | | | |

Table 5: Top 2 Choices Market Share Predictions for 2013 K1

| | | Naive | | Logit | | Mixed Logit | | |
|---|---|---|---|---|---|---|---|---|
| Neighborhood | School | mean | (95% C.I.) | mean | (95% C.I.) | mean | (95% C.I.) | Actual |
| Allston-Brighton | Adams | 0.07 | (0.04,0.09) | 0.00 | (0.00,0.01) | 0.00 | (0.00,0.01) | |
| Allston-Brighton | Baldwin | 0.10 | (0.08,0.12) | 0.23 | (0.19,0.27) | 0.22 | (0.19,0.26) | 0.39 |
| Allston-Brighton | Blackstone | | | 0.03 | (0.01,0.05) | 0.02 | (0.01,0.04) | 0.01 |
| Allston-Brighton | Bradley | | | 0.00 | (0.00,0.01) | 0.01 | (0.00,0.02) | |
| Allston-Brighton | East Boston EEC | | | 0.01 | (0.00,0.02) | 0.02 | (0.00,0.04) | |
| Allston-Brighton | Edison | 0.12 | (0.09,0.16) | 0.19 | (0.14,0.24) | 0.19 | (0.14,0.23) | 0.07 |
| Allston-Brighton | Eliot | | | 0.03 | (0.01,0.05) | 0.03 | (0.01,0.05) | 0.02 |
| Allston-Brighton | Ellison/Parks | 0.00 | (0.00,0.01) | | | | | |
| Allston-Brighton | Gardner | 0.03 | (0.01,0.05) | 0.13 | (0.10,0.18) | 0.14 | (0.10,0.19) | 0.13 |
| Allston-Brighton | Harvard/Kent | 0.06 | (0.04,0.09) | 0.02 | (0.00,0.04) | 0.02 | (0.00,0.04) | |
| Allston-Brighton | Hernandez | | | 0.02 | (0.01,0.04) | 0.02 | (0.01,0.04) | 0.01 |
| Allston-Brighton | Hurley | 0.27 | (0.23,0.30) | 0.03 | (0.01,0.05) | 0.03 | (0.01,0.05) | |
| Allston-Brighton | Jackson/Mann | 0.05 | (0.01,0.09) | 0.11 | (0.07,0.16) | 0.10 | (0.06,0.14) | 0.15 |
| Allston-Brighton | Kennedy Patrick | | | 0.00 | (0.00,0.01) | | | |
| Allston-Brighton | Mason | 0.04 | (0.02,0.06) | 0.01 | (0.00,0.02) | 0.01 | (0.00,0.01) | |
| Allston-Brighton | Mission Hill | | | | | 0.01 | | |
| Allston-Brighton | O'Donnell | | | 0.00 | (0.00,0.01) | 0.00 | (0.00,0.01) | |
| Allston-Brighton | Orchard Gardens | 0.00 | (0.00,0.01) | 0.01 | (0.00,0.02) | 0.01 | (0.00,0.02) | |
| Allston-Brighton | Otis | 0.15 | (0.12,0.19) | 0.01 | (0.00,0.02) | 0.01 | (0.00,0.02) | |
| Allston-Brighton | Quincy | 0.09 | (0.06,0.13) | 0.04 | (0.02,0.07) | 0.05 | (0.02,0.07) | 0.03 |
| Allston-Brighton | Tobin | | | 0.01 | (0.00,0.02) | 0.01 | (0.00,0.02) | |
| Allston-Brighton | Winship | 0.02 | (0.00,0.03) | 0.12 | (0.08,0.15) | 0.11 | (0.07,0.15) | 0.18 |
| Charlestown | Adams | 0.04 | (0.01,0.09) | 0.01 | (0.00,0.03) | 0.00 | (0.00,0.02) | |
| Charlestown | Baldwin | 0.03 | (0.01,0.05) | 0.04 | (0.01,0.07) | 0.03 | (0.00,0.07) | 0.03 |
| Charlestown | Blackstone | | | 0.03 | (0.00,0.07) | 0.03 | (0.00,0.07) | 0.04 |
| Charlestown | Bradley | | | 0.02 | (0.00,0.05) | 0.01 | (0.00,0.04) | |
| Charlestown | Dever | 0.01 | (0.00,0.03) | | | | | |
| Charlestown | East Boston EEC | | | 0.03 | (0.00,0.06) | 0.03 | (0.00,0.06) | 0.03 |
| Charlestown | Edison | 0.01 | (0.00,0.03) | 0.01 | (0.00,0.03) | 0.01 | (0.00,0.03) | |
| Charlestown | Eliot | 0.33 | (0.25,0.39) | 0.36 | (0.26,0.47) | 0.39 | (0.28,0.49) | 0.53 |
| Charlestown | Gardner | | | 0.02 | (0.00,0.05) | 0.01 | (0.00,0.04) | |
| Charlestown | Harvard/Kent | 0.38 | (0.31,0.44) | 0.20 | (0.14,0.27) | 0.22 | (0.14,0.29) | 0.25 |
| Charlestown | Hernandez | | | 0.01 | (0.00,0.04) | 0.01 | (0.00,0.04) | |
| Charlestown | Hurley | 0.09 | (0.03,0.17) | 0.04 | (0.00,0.08) | 0.03 | (0.00,0.07) | |
| Charlestown | Jackson/Mann | | | 0.01 | (0.00,0.03) | 0.01 | (0.00,0.02) | |
| Charlestown | Kennedy Patrick | | | 0.01 | (0.00,0.04) | 0.01 | (0.00,0.03) | |
| Charlestown | Mason | 0.01 | (0.00,0.03) | 0.01 | (0.00,0.02) | 0.00 | (0.00,0.02) | |
| Charlestown | O'Donnell | | | 0.02 | (0.00,0.04) | 0.01 | (0.00,0.03) | |
| Charlestown | Orchard Gardens | 0.01 | (0.00,0.02) | 0.01 | (0.00,0.03) | 0.01 | (0.00,0.03) | |
| Charlestown | Otis | 0.03 | (0.00,0.07) | 0.02 | (0.00,0.06) | 0.02 | (0.00,0.05) | |
| Charlestown | Quincy | 0.03 | (0.00,0.07) | 0.15 | (0.08,0.23) | 0.15 | (0.08,0.23) | 0.07 |
| Charlestown | Roosevelt | | | | | 0.00 | (0.00,0.01) | |
| Charlestown | Taylor | 0.02 | (0.00,0.05) | | | 0.00 | (0.00,0.01) | |
| Charlestown | Tobin | 0.02 | (0.00,0.05) | 0.01 | (0.00,0.03) | 0.01 | (0.00,0.03) | |
| Charlestown | Winship | 0.01 | (0.00,0.03) | 0.01 | (0.00,0.04) | 0.01 | (0.00,0.03) | |
| Charlestown | Winthrop | | | 0.00 | (0.00,0.02) | 0.00 | (0.00,0.01) | |
| Charlestown | Young Achievers | | | 0.00 | (0.00,0.01) | 0.00 | (0.00,0.01) | |
| Downtown | Adams | 0.02 | (0.00,0.04) | | | | | |
| Downtown | Baldwin | | | 0.03 | (0.01,0.04) | 0.03 | (0.01,0.05) | 0.04 |
| Downtown | Blackstone | 0.01 | (0.00,0.03) | 0.05 | (0.03,0.09) | 0.06 | (0.03,0.09) | 0.01 |
| Downtown | Bradley | | | 0.01 | (0.00,0.02) | 0.01 | (0.00,0.02) | |
| Downtown | Chittick | 0.00 | (0.00,0.01) | | | | | |
| Downtown | Condon | | | 0.01 | (0.00,0.02) | 0.01 | (0.00,0.02) | |
| Downtown | East Boston EEC | | | 0.01 | (0.00,0.03) | 0.02 | (0.00,0.04) | 0.02 |

Continued on next page

**Table 5 – continued from previous page**

| | | Naive | | Logit | | Mixed Logit | | |
|---|---|---|---|---|---|---|---|---|
| Neighborhood | School | mean | (95% C.I.) | mean | (95% C.I.) | mean | (95% C.I.) | Actual |
| Downtown | Edison | 0.07 | (0.04,0.11) | 0.02 | (0.00,0.03) | 0.02 | (0.00,0.03) | |
| Downtown | Eliot | 0.34 | (0.26,0.41) | 0.31 | (0.24,0.38) | 0.31 | (0.25,0.38) | 0.47 |
| Downtown | Gardner | 0.00 | (0.00,0.01) | 0.02 | (0.00,0.04) | 0.02 | (0.00,0.03) | |
| Downtown | Hale | 0.02 | (0.01,0.04) | 0.00 | (0.00,0.01) | 0.00 | (0.00,0.01) | |
| Downtown | Harvard/Kent | 0.03 | (0.01,0.05) | 0.06 | (0.04,0.10) | 0.06 | (0.03,0.09) | 0.01 |
| Downtown | Hernandez | | | 0.02 | (0.00,0.03) | 0.02 | (0.00,0.03) | 0.02 |
| Downtown | Hurley | 0.10 | (0.07,0.14) | 0.05 | (0.02,0.08) | 0.05 | (0.03,0.08) | 0.04 |
| Downtown | J.F. Kennedy | | | 0.00 | (0.00,0.01) | 0.00 | (0.00,0.01) | |
| Downtown | Jackson/Mann | | | 0.01 | (0.00,0.03) | 0.01 | (0.00,0.02) | |
| Downtown | Kennedy Patrick | | | 0.00 | (0.00,0.01) | 0.00 | (0.00,0.01) | |
| Downtown | Mason | 0.00 | (0.00,0.01) | 0.01 | (0.00,0.02) | 0.01 | (0.00,0.02) | |
| Downtown | Mission Hill | 0.00 | (0.00,0.01) | | | 0.02 | | |
| Downtown | O'Donnell | | | 0.00 | (0.00,0.01) | 0.00 | (0.00,0.01) | |
| Downtown | Orchard Gardens | 0.00 | (0.00,0.02) | 0.02 | (0.00,0.04) | 0.02 | (0.00,0.03) | 0.02 |
| Downtown | Otis | 0.10 | (0.07,0.14) | 0.01 | (0.00,0.02) | 0.01 | (0.00,0.02) | |
| Downtown | Quincy | 0.28 | (0.20,0.36) | 0.31 | (0.25,0.37) | 0.32 | (0.25,0.38) | 0.31 |
| Downtown | Tobin | | | 0.02 | (0.00,0.03) | 0.02 | (0.00,0.04) | 0.01 |
| Downtown | West Zone ELC | | | 0.01 | (0.00,0.02) | 0.01 | (0.00,0.02) | |
| Downtown | Winship | 0.00 | (0.00,0.01) | 0.01 | (0.00,0.03) | 0.01 | (0.00,0.02) | |
| Downtown | Winthrop | | | 0.00 | (0.00,0.01) | | | |
| East Boston | Adams | 0.23 | (0.20,0.26) | 0.11 | (0.07,0.15) | 0.11 | (0.08,0.13) | 0.06 |
| East Boston | Baldwin | | | | | 0.01 | (0.00,0.02) | 0.01 |
| East Boston | Blackstone | 0.01 | (0.01,0.03) | 0.02 | (0.01,0.03) | 0.02 | (0.01,0.03) | 0.03 |
| East Boston | Bradley | 0.06 | (0.03,0.08) | 0.13 | (0.10,0.16) | 0.14 | (0.11,0.17) | 0.12 |
| East Boston | East Boston EEC | 0.07 | (0.05,0.09) | 0.27 | (0.23,0.30) | 0.27 | (0.23,0.30) | 0.37 |
| East Boston | Edison | 0.08 | (0.06,0.10) | 0.01 | (0.00,0.01) | 0.01 | (0.01,0.02) | |
| East Boston | Eliot | | | 0.02 | (0.01,0.04) | 0.02 | (0.01,0.03) | 0.03 |
| East Boston | Gardner | | | 0.01 | (0.00,0.01) | 0.01 | (0.00,0.01) | |
| East Boston | Harvard/Kent | 0.02 | (0.01,0.03) | 0.02 | (0.01,0.03) | 0.01 | (0.01,0.02) | |
| East Boston | Hernandez | | | 0.01 | (0.00,0.01) | 0.02 | (0.01,0.03) | |
| East Boston | Hurley | 0.24 | (0.21,0.27) | 0.02 | (0.01,0.03) | 0.02 | (0.01,0.03) | |
| East Boston | Jackson/Mann | 0.01 | (0.00,0.02) | | | | | |
| East Boston | Kennedy Patrick | 0.02 | (0.01,0.03) | 0.09 | (0.06,0.13) | 0.07 | (0.05,0.09) | 0.09 |
| East Boston | O'Donnell | 0.01 | (0.01,0.02) | 0.07 | (0.05,0.10) | 0.05 | (0.04,0.07) | 0.08 |
| East Boston | Orchard Gardens | 0.01 | (0.00,0.02) | | | | | |
| East Boston | Otis | 0.23 | (0.19,0.27) | 0.22 | (0.18,0.26) | 0.21 | (0.18,0.25) | 0.16 |
| East Boston | Quincy | 0.00 | (0.00,0.01) | 0.01 | (0.00,0.02) | 0.01 | (0.00,0.02) | 0.02 |
| Hyde Park | BTU | | | 0.01 | (0.00,0.02) | 0.01 | (0.00,0.02) | |
| Hyde Park | Bates | | | 0.02 | (0.01,0.03) | 0.02 | (0.01,0.03) | 0.01 |
| Hyde Park | Beethoven | 0.01 | (0.00,0.02) | 0.05 | (0.03,0.07) | 0.05 | (0.03,0.07) | 0.07 |
| Hyde Park | Channing | 0.02 | (0.01,0.04) | 0.10 | (0.07,0.13) | 0.11 | (0.08,0.14) | 0.10 |
| Hyde Park | Chittick | | | 0.06 | (0.04,0.09) | 0.06 | (0.04,0.08) | 0.06 |
| Hyde Park | Clap | | | 0.01 | (0.00,0.02) | 0.01 | (0.00,0.02) | |
| Hyde Park | Condon | 0.01 | (0.00,0.02) | 0.01 | (0.00,0.02) | 0.01 | (0.00,0.02) | |
| Hyde Park | Conley | 0.14 | (0.11,0.17) | 0.03 | (0.02,0.06) | 0.04 | (0.02,0.06) | 0.04 |
| Hyde Park | Curley | 0.02 | (0.00,0.03) | 0.01 | (0.00,0.02) | 0.01 | (0.00,0.02) | |
| Hyde Park | Dever | 0.01 | (0.00,0.01) | 0.01 | (0.00,0.02) | 0.01 | (0.00,0.02) | |
| Hyde Park | Ellison/Parks | 0.10 | (0.07,0.12) | 0.09 | (0.06,0.11) | 0.09 | (0.07,0.12) | 0.09 |
| Hyde Park | Everett | | | 0.01 | (0.00,0.02) | 0.01 | (0.00,0.02) | |
| Hyde Park | Haley | | | 0.01 | (0.00,0.02) | 0.01 | (0.00,0.02) | |
| Hyde Park | Harvard/Kent | 0.00 | (0.00,0.01) | | | | | |
| Hyde Park | Haynes | 0.02 | (0.01,0.03) | | | 0.00 | (0.00,0.01) | |
| Hyde Park | Henderson | 0.16 | (0.13,0.19) | 0.02 | (0.01,0.03) | 0.02 | (0.01,0.03) | |
| Hyde Park | Hernandez | | | 0.02 | (0.01,0.04) | 0.02 | (0.01,0.03) | 0.06 |
| Hyde Park | Holland | 0.01 | (0.00,0.02) | 0.01 | (0.00,0.02) | 0.01 | (0.00,0.01) | |

Continued on next page

**Table 5 – continued from previous page**

| Neighborhood | School | Naive mean | Naive (95% C.I.) | Logit mean | Logit (95% C.I.) | Mixed Logit mean | Mixed Logit (95% C.I.) | Actual |
|---|---|---|---|---|---|---|---|---|
| Hyde Park | Holmes | | | 0.01 | (0.00,0.01) | 0.00 | (0.00,0.01) | |
| Hyde Park | Kenny | | | 0.01 | (0.00,0.02) | 0.01 | (0.00,0.02) | |
| Hyde Park | Kilmer | | | 0.01 | (0.00,0.02) | 0.01 | (0.00,0.03) | 0.03 |
| Hyde Park | King | 0.00 | (0.00,0.01) | | | | | |
| Hyde Park | Lee | 0.02 | (0.01,0.04) | 0.04 | (0.02,0.06) | 0.03 | (0.02,0.05) | 0.04 |
| Hyde Park | Lyndon | 0.01 | (0.00,0.01) | 0.01 | (0.00,0.02) | 0.01 | (0.00,0.02) | 0.01 |
| Hyde Park | Manning | 0.00 | (0.00,0.01) | 0.00 | (0.00,0.01) | 0.00 | (0.00,0.01) | |
| Hyde Park | Mather | 0.01 | (0.00,0.03) | 0.01 | (0.00,0.02) | 0.01 | (0.00,0.02) | |
| Hyde Park | Mattahunt | 0.01 | (0.00,0.03) | 0.04 | (0.02,0.07) | 0.04 | (0.02,0.06) | 0.04 |
| Hyde Park | Mission Hill | | | 0.00 | (0.00,0.01) | | | |
| Hyde Park | Mozart | | | 0.01 | (0.00,0.02) | 0.01 | (0.00,0.02) | |
| Hyde Park | Murphy | 0.01 | (0.00,0.03) | 0.05 | (0.03,0.08) | 0.06 | (0.03,0.08) | 0.06 |
| Hyde Park | Perry | | | 0.01 | (0.00,0.02) | 0.01 | (0.00,0.02) | |
| Hyde Park | Philbrick | 0.04 | (0.02,0.05) | 0.01 | (0.00,0.02) | 0.01 | (0.00,0.02) | 0.01 |
| Hyde Park | Roosevelt | 0.27 | (0.24,0.31) | 0.19 | (0.16,0.24) | 0.20 | (0.16,0.24) | 0.22 |
| Hyde Park | Russell | 0.02 | (0.01,0.04) | 0.01 | (0.00,0.02) | 0.01 | (0.00,0.02) | |
| Hyde Park | S. Greenwood | 0.03 | (0.01,0.05) | 0.02 | (0.01,0.03) | 0.01 | (0.00,0.02) | 0.01 |
| Hyde Park | Sumner | 0.02 | (0.01,0.04) | 0.01 | (0.00,0.02) | 0.01 | (0.00,0.02) | |
| Hyde Park | Taylor | 0.02 | (0.01,0.04) | 0.02 | (0.01,0.03) | 0.02 | (0.01,0.03) | |
| Hyde Park | Tynan | | | | | 0.00 | (0.00,0.01) | |
| Hyde Park | Young Achievers | 0.01 | (0.00,0.01) | 0.06 | (0.04,0.09) | 0.07 | (0.04,0.10) | 0.07 |
| Jamaica Plain | BTU | 0.01 | (0.00,0.02) | 0.08 | (0.05,0.11) | 0.07 | (0.04,0.10) | 0.10 |
| Jamaica Plain | Baldwin | | | 0.02 | (0.01,0.03) | 0.02 | (0.01,0.03) | 0.02 |
| Jamaica Plain | Bates | | | 0.01 | (0.00,0.03) | 0.01 | (0.00,0.02) | |
| Jamaica Plain | Beethoven | 0.00 | (0.00,0.01) | 0.02 | (0.01,0.04) | 0.02 | (0.01,0.04) | 0.01 |
| Jamaica Plain | Blackstone | 0.01 | (0.01,0.02) | 0.02 | (0.01,0.03) | 0.02 | (0.01,0.03) | 0.01 |
| Jamaica Plain | Bradley | | | | | 0.00 | (0.00,0.01) | |
| Jamaica Plain | Conley | | | 0.01 | (0.00,0.02) | 0.01 | (0.00,0.02) | |
| Jamaica Plain | Curley | 0.08 | (0.05,0.12) | 0.20 | (0.15,0.24) | 0.21 | (0.17,0.26) | 0.23 |
| Jamaica Plain | Dever | 0.01 | (0.00,0.02) | | | | | |
| Jamaica Plain | East Boston EEC | | | | | 0.01 | (0.00,0.01) | |
| Jamaica Plain | Edison | 0.03 | (0.01,0.04) | 0.01 | (0.00,0.02) | 0.01 | (0.00,0.02) | |
| Jamaica Plain | Eliot | | | 0.01 | (0.00,0.03) | 0.01 | (0.00,0.02) | |
| Jamaica Plain | Ellis | | | 0.02 | (0.01,0.03) | 0.02 | (0.01,0.03) | 0.02 |
| Jamaica Plain | Gardner | | | 0.01 | (0.00,0.02) | 0.01 | (0.00,0.01) | |
| Jamaica Plain | Hale | 0.22 | (0.18,0.25) | 0.02 | (0.01,0.03) | 0.02 | (0.01,0.03) | |
| Jamaica Plain | Haley | | | 0.02 | (0.01,0.04) | 0.02 | (0.01,0.03) | |
| Jamaica Plain | Harvard/Kent | 0.03 | (0.01,0.04) | 0.01 | (0.00,0.02) | 0.01 | (0.00,0.02) | |
| Jamaica Plain | Haynes | 0.05 | (0.03,0.07) | 0.01 | (0.00,0.03) | 0.02 | (0.01,0.03) | 0.02 |
| Jamaica Plain | Hernandez | 0.02 | (0.00,0.04) | 0.05 | (0.03,0.08) | 0.06 | (0.04,0.08) | 0.08 |
| Jamaica Plain | Higginson/Lewis | | | 0.01 | (0.00,0.02) | 0.01 | (0.00,0.02) | |
| Jamaica Plain | Holland | 0.01 | (0.00,0.01) | | | | | |
| Jamaica Plain | Hurley | 0.05 | (0.03,0.07) | 0.02 | (0.00,0.03) | 0.02 | (0.00,0.03) | |
| Jamaica Plain | J.F. Kennedy | 0.01 | (0.00,0.02) | 0.03 | (0.01,0.06) | 0.03 | (0.01,0.05) | 0.05 |
| Jamaica Plain | Jackson/Mann | 0.01 | (0.00,0.03) | 0.01 | (0.00,0.02) | 0.01 | (0.00,0.01) | 0.01 |
| Jamaica Plain | Kilmer | | | 0.03 | (0.02,0.05) | 0.05 | (0.03,0.07) | 0.02 |
| Jamaica Plain | King | | | 0.00 | (0.00,0.01) | | | |
| Jamaica Plain | Lyndon | | | 0.03 | (0.01,0.05) | 0.02 | (0.01,0.04) | 0.02 |
| Jamaica Plain | Manning | 0.26 | (0.22,0.29) | 0.06 | (0.04,0.09) | 0.07 | (0.04,0.09) | 0.05 |
| Jamaica Plain | Mason | | | 0.00 | (0.00,0.01) | 0.00 | (0.00,0.01) | |
| Jamaica Plain | Mather | 0.01 | (0.00,0.01) | | | | | |
| Jamaica Plain | Mendell | 0.01 | (0.00,0.01) | 0.03 | (0.02,0.06) | 0.03 | (0.01,0.05) | 0.05 |
| Jamaica Plain | Mission Hill | | | 0.07 | (0.05,0.10) | 0.07 | (0.05,0.09) | 0.16 |
| Jamaica Plain | Mozart | | | 0.02 | (0.01,0.03) | 0.01 | (0.00,0.02) | |
| Jamaica Plain | Orchard Gardens | 0.01 | (0.00,0.01) | 0.01 | (0.00,0.02) | 0.01 | (0.00,0.02) | |

Continued on next page

**Table 5 – continued from previous page**

| Neighborhood | School | Naive mean | Naive (95% C.I.) | Logit mean | Logit (95% C.I.) | Mixed Logit mean | Mixed Logit (95% C.I.) | Actual |
|---|---|---|---|---|---|---|---|---|
| Jamaica Plain | Otis | 0.03 | (0.01,0.05) | | | | | |
| Jamaica Plain | Philbrick | 0.09 | (0.07,0.12) | 0.01 | (0.00,0.03) | 0.01 | (0.00,0.03) | |
| Jamaica Plain | Quincy | 0.01 | (0.00,0.03) | 0.02 | (0.01,0.04) | 0.02 | (0.01,0.04) | |
| Jamaica Plain | Sumner | 0.05 | (0.03,0.07) | 0.01 | (0.00,0.02) | 0.01 | (0.00,0.02) | |
| Jamaica Plain | Tobin | | | 0.02 | (0.01,0.03) | 0.02 | (0.01,0.04) | 0.03 |
| Jamaica Plain | Trotter | | | 0.01 | (0.00,0.02) | 0.01 | (0.00,0.01) | |
| Jamaica Plain | West Zone ELC | | | 0.05 | (0.03,0.08) | 0.06 | (0.04,0.09) | 0.06 |
| Jamaica Plain | Winship | | | 0.01 | (0.00,0.02) | 0.00 | (0.00,0.01) | |
| Mattapan | BTU | | | 0.01 | (0.00,0.01) | 0.01 | (0.00,0.01) | |
| Mattapan | Beethoven | 0.01 | (0.00,0.02) | 0.01 | (0.00,0.02) | 0.01 | (0.00,0.01) | |
| Mattapan | Blackstone | 0.01 | (0.00,0.02) | | | | | |
| Mattapan | Channing | | | 0.02 | (0.01,0.04) | 0.02 | (0.01,0.03) | 0.02 |
| Mattapan | Chittick | 0.02 | (0.00,0.04) | 0.05 | (0.03,0.07) | 0.05 | (0.03,0.07) | 0.04 |
| Mattapan | Clap | | | 0.02 | (0.01,0.03) | 0.01 | (0.01,0.03) | 0.01 |
| Mattapan | Condon | | | 0.02 | (0.00,0.03) | 0.01 | (0.00,0.02) | 0.01 |
| Mattapan | Curley | | | 0.01 | (0.00,0.02) | 0.01 | (0.00,0.02) | |
| Mattapan | Dever | 0.01 | (0.00,0.01) | 0.02 | (0.01,0.04) | 0.02 | (0.01,0.04) | 0.03 |
| Mattapan | Ellis | 0.01 | (0.00,0.01) | | | | | |
| Mattapan | Ellison/Parks | 0.09 | (0.07,0.12) | 0.12 | (0.09,0.15) | 0.13 | (0.10,0.16) | 0.19 |
| Mattapan | Everett | 0.01 | (0.00,0.01) | 0.02 | (0.01,0.03) | 0.01 | (0.00,0.03) | |
| Mattapan | Hale | 0.01 | (0.00,0.01) | | | | | |
| Mattapan | Haley | | | 0.03 | (0.01,0.06) | 0.03 | (0.01,0.05) | 0.03 |
| Mattapan | Haynes | 0.02 | (0.01,0.03) | 0.01 | (0.00,0.02) | 0.01 | (0.00,0.02) | 0.01 |
| Mattapan | Henderson | 0.29 | (0.26,0.32) | 0.02 | (0.01,0.04) | 0.03 | (0.01,0.04) | 0.01 |
| Mattapan | Hernandez | 0.02 | (0.00,0.04) | 0.04 | (0.02,0.06) | 0.04 | (0.02,0.06) | 0.06 |
| Mattapan | Holland | 0.01 | (0.00,0.01) | 0.01 | (0.00,0.03) | 0.01 | (0.00,0.02) | 0.02 |
| Mattapan | Holmes | | | 0.01 | (0.00,0.03) | 0.01 | (0.00,0.03) | |
| Mattapan | J.F. Kennedy | 0.01 | (0.00,0.01) | | | | | |
| Mattapan | Kenny | | | 0.02 | (0.01,0.03) | 0.02 | (0.01,0.03) | |
| Mattapan | Lee | 0.02 | (0.01,0.04) | 0.09 | (0.06,0.13) | 0.09 | (0.06,0.12) | 0.10 |
| Mattapan | Lyndon | 0.01 | (0.00,0.01) | | | | | |
| Mattapan | Mather | 0.01 | (0.00,0.02) | 0.01 | (0.00,0.03) | 0.01 | (0.00,0.03) | 0.01 |
| Mattapan | Mattahunt | 0.04 | (0.02,0.07) | 0.04 | (0.02,0.07) | 0.04 | (0.02,0.06) | 0.04 |
| Mattapan | Murphy | 0.16 | (0.13,0.20) | 0.07 | (0.04,0.10) | 0.08 | (0.05,0.11) | 0.07 |
| Mattapan | Perry | | | 0.01 | (0.00,0.02) | 0.01 | (0.00,0.03) | |
| Mattapan | Philbrick | 0.05 | (0.03,0.07) | 0.00 | (0.00,0.01) | 0.00 | (0.00,0.01) | |
| Mattapan | Roosevelt | 0.03 | (0.01,0.05) | 0.04 | (0.02,0.06) | 0.04 | (0.02,0.05) | 0.04 |
| Mattapan | Russell | 0.04 | (0.02,0.06) | 0.02 | (0.01,0.03) | 0.01 | (0.01,0.03) | 0.01 |
| Mattapan | S. Greenwood | 0.05 | (0.03,0.07) | 0.04 | (0.03,0.07) | 0.04 | (0.02,0.07) | 0.04 |
| Mattapan | Sumner | 0.04 | (0.02,0.06) | 0.01 | (0.00,0.02) | 0.01 | (0.00,0.02) | |
| Mattapan | Taylor | 0.04 | (0.02,0.06) | 0.04 | (0.02,0.06) | 0.04 | (0.02,0.06) | 0.04 |
| Mattapan | Tynan | | | 0.01 | (0.00,0.01) | 0.00 | (0.00,0.01) | |
| Mattapan | Young Achievers | 0.01 | (0.00,0.02) | 0.16 | (0.12,0.20) | 0.18 | (0.14,0.21) | 0.12 |
| North Dorchester | Baldwin | | | 0.00 | (0.00,0.01) | 0.00 | (0.00,0.01) | |
| North Dorchester | Blackstone | | | 0.01 | (0.00,0.03) | 0.01 | (0.00,0.02) | 0.01 |
| North Dorchester | Channing | | | 0.00 | (0.00,0.01) | 0.01 | (0.00,0.02) | |
| North Dorchester | Chittick | | | 0.01 | (0.00,0.01) | 0.00 | (0.00,0.01) | |
| North Dorchester | Clap | 0.02 | (0.01,0.05) | 0.11 | (0.07,0.15) | 0.10 | (0.07,0.13) | 0.09 |
| North Dorchester | Condon | | | 0.04 | (0.01,0.06) | 0.03 | (0.01,0.04) | 0.05 |
| North Dorchester | Dever | 0.03 | (0.01,0.05) | 0.07 | (0.04,0.10) | 0.07 | (0.04,0.10) | 0.07 |
| North Dorchester | East Boston EEC | | | | | 0.00 | (0.00,0.01) | 0.01 |
| North Dorchester | Edison | 0.02 | (0.01,0.04) | 0.00 | (0.00,0.01) | 0.00 | (0.00,0.01) | |
| North Dorchester | Eliot | | | 0.01 | (0.00,0.02) | 0.00 | (0.00,0.01) | |
| North Dorchester | Ellison/Parks | 0.13 | (0.09,0.17) | 0.02 | (0.01,0.04) | 0.03 | (0.01,0.06) | 0.02 |
| North Dorchester | Everett | 0.03 | (0.01,0.05) | 0.08 | (0.06,0.12) | 0.09 | (0.06,0.12) | 0.12 |

Continued on next page

**Table 5 – continued from previous page**

| Neighborhood | School | Naive mean | Naive (95% C.I.) | Logit mean | Logit (95% C.I.) | Mixed Logit mean | Mixed Logit (95% C.I.) | Actual |
|---|---|---|---|---|---|---|---|---|
| North Dorchester | Gardner | 0.00 | (0.00,0.01) | 0.00 | (0.00,0.01) | | | |
| North Dorchester | Haynes | 0.10 | (0.07,0.14) | 0.06 | (0.03,0.09) | 0.07 | (0.04,0.10) | 0.04 |
| North Dorchester | Henderson | 0.12 | (0.09,0.15) | 0.03 | (0.01,0.04) | 0.03 | (0.01,0.04) | 0.01 |
| North Dorchester | Hernandez | | | 0.02 | (0.01,0.04) | 0.02 | (0.01,0.04) | 0.02 |
| North Dorchester | Holland | 0.04 | (0.02,0.07) | 0.03 | (0.01,0.06) | 0.03 | (0.01,0.05) | 0.02 |
| North Dorchester | Holmes | | | 0.01 | (0.00,0.02) | 0.01 | (0.00,0.02) | |
| North Dorchester | Hurley | 0.03 | (0.01,0.04) | 0.01 | (0.00,0.02) | 0.01 | (0.00,0.02) | |
| North Dorchester | Kenny | | | 0.01 | (0.00,0.02) | 0.01 | (0.00,0.02) | |
| North Dorchester | King | | | 0.01 | (0.00,0.02) | 0.01 | (0.00,0.02) | |
| North Dorchester | Lee | 0.02 | (0.00,0.03) | 0.03 | (0.01,0.05) | 0.03 | (0.01,0.05) | 0.04 |
| North Dorchester | Mason | 0.12 | (0.09,0.15) | 0.02 | (0.01,0.04) | 0.02 | (0.01,0.04) | 0.03 |
| North Dorchester | Mather | 0.07 | (0.04,0.10) | 0.08 | (0.04,0.11) | 0.08 | (0.05,0.12) | 0.10 |
| North Dorchester | Mattahunt | 0.01 | (0.00,0.03) | 0.01 | (0.00,0.01) | 0.00 | (0.00,0.01) | |
| North Dorchester | Mission Hill | | | | | 0.01 | | |
| North Dorchester | Murphy | 0.12 | (0.07,0.16) | 0.12 | (0.08,0.15) | 0.13 | (0.09,0.17) | 0.17 |
| North Dorchester | Orchard Gardens | 0.01 | (0.00,0.02) | 0.01 | (0.00,0.03) | 0.01 | (0.00,0.02) | 0.01 |
| North Dorchester | Otis | 0.03 | (0.02,0.06) | | | | | |
| North Dorchester | Perry | | | 0.04 | (0.02,0.06) | 0.04 | (0.02,0.06) | 0.02 |
| North Dorchester | Quincy | 0.01 | (0.00,0.03) | 0.01 | (0.00,0.02) | 0.01 | (0.00,0.03) | |
| North Dorchester | Roosevelt | 0.01 | (0.00,0.02) | 0.01 | (0.00,0.02) | 0.01 | (0.00,0.03) | 0.01 |
| North Dorchester | Russell | 0.05 | (0.02,0.09) | 0.07 | (0.04,0.10) | 0.07 | (0.04,0.10) | 0.06 |
| North Dorchester | S. Greenwood | 0.01 | (0.00,0.03) | 0.01 | (0.00,0.03) | 0.01 | (0.00,0.03) | 0.01 |
| North Dorchester | Taylor | | | 0.01 | (0.00,0.01) | 0.00 | (0.00,0.01) | |
| North Dorchester | Tynan | 0.00 | (0.00,0.01) | 0.02 | (0.00,0.03) | 0.01 | (0.00,0.03) | |
| North Dorchester | Winthrop | 0.00 | (0.00,0.01) | 0.01 | (0.00,0.03) | 0.01 | (0.00,0.02) | |
| North Dorchester | Young Achievers | | | 0.02 | (0.01,0.04) | 0.02 | (0.01,0.03) | 0.02 |
| Roslindale | BTU | 0.01 | (0.00,0.02) | 0.11 | (0.08,0.13) | 0.11 | (0.09,0.14) | 0.13 |
| Roslindale | Bates | 0.02 | (0.01,0.03) | 0.07 | (0.05,0.09) | 0.07 | (0.05,0.09) | 0.07 |
| Roslindale | Beethoven | 0.02 | (0.01,0.03) | 0.09 | (0.07,0.11) | 0.08 | (0.06,0.11) | 0.08 |
| Roslindale | Chittick | | | 0.01 | (0.00,0.01) | 0.00 | (0.00,0.01) | |
| Roslindale | Conley | 0.17 | (0.14,0.20) | 0.05 | (0.04,0.08) | 0.05 | (0.03,0.07) | 0.04 |
| Roslindale | Curley | 0.05 | (0.03,0.07) | 0.06 | (0.04,0.08) | 0.05 | (0.04,0.07) | 0.03 |
| Roslindale | Ellis | 0.01 | (0.00,0.02) | 0.01 | (0.00,0.02) | 0.01 | (0.00,0.02) | |
| Roslindale | Ellison/Parks | 0.00 | (0.00,0.01) | | | | | |
| Roslindale | Hale | 0.01 | (0.00,0.02) | 0.00 | (0.00,0.01) | | | |
| Roslindale | Haley | 0.03 | (0.01,0.04) | 0.06 | (0.04,0.08) | 0.06 | (0.04,0.08) | 0.09 |
| Roslindale | Harvard/Kent | 0.00 | (0.00,0.01) | | | | | |
| Roslindale | Haynes | 0.10 | (0.07,0.12) | 0.01 | (0.00,0.03) | 0.02 | (0.01,0.03) | 0.03 |
| Roslindale | Hernandez | 0.01 | (0.00,0.03) | 0.03 | (0.01,0.04) | 0.03 | (0.01,0.04) | 0.05 |
| Roslindale | J.F. Kennedy | 0.01 | (0.00,0.01) | 0.01 | (0.00,0.02) | 0.01 | (0.00,0.01) | 0.02 |
| Roslindale | Kilmer | 0.01 | (0.00,0.02) | 0.09 | (0.07,0.11) | 0.11 | (0.09,0.14) | 0.09 |
| Roslindale | Lyndon | 0.04 | (0.02,0.05) | 0.09 | (0.07,0.12) | 0.07 | (0.05,0.10) | 0.09 |
| Roslindale | Manning | 0.02 | (0.01,0.03) | 0.04 | (0.02,0.06) | 0.04 | (0.02,0.06) | |
| Roslindale | Mattahunt | | | 0.01 | (0.00,0.01) | 0.01 | (0.00,0.01) | |
| Roslindale | Mendell | 0.01 | (0.00,0.01) | 0.01 | (0.00,0.02) | 0.01 | (0.00,0.02) | 0.01 |
| Roslindale | Mission Hill | | | 0.04 | (0.02,0.05) | 0.03 | (0.02,0.04) | 0.05 |
| Roslindale | Mozart | 0.01 | (0.00,0.01) | 0.07 | (0.06,0.10) | 0.07 | (0.05,0.09) | 0.06 |
| Roslindale | Philbrick | 0.15 | (0.12,0.17) | 0.05 | (0.03,0.08) | 0.04 | (0.03,0.06) | 0.05 |
| Roslindale | Roosevelt | 0.01 | (0.00,0.02) | 0.01 | (0.00,0.01) | 0.01 | (0.00,0.01) | |
| Roslindale | Sumner | 0.32 | (0.29,0.34) | 0.06 | (0.04,0.08) | 0.07 | (0.05,0.09) | 0.07 |
| Roslindale | Trotter | | | 0.00 | (0.00,0.01) | | | |
| Roslindale | West Zone ELC | | | 0.01 | (0.00,0.02) | 0.01 | (0.01,0.03) | 0.01 |
| Roslindale | Young Achievers | | | 0.01 | (0.00,0.01) | 0.01 | (0.00,0.01) | |
| Roxbury | BTU | | | 0.04 | (0.03,0.06) | 0.03 | (0.02,0.05) | 0.03 |
| Roxbury | Baldwin | | | 0.01 | (0.00,0.01) | 0.01 | (0.00,0.01) | |

Continued on next page

**Table 5 – continued from previous page**

| Neighborhood | School | Naive | | Logit | | Mixed Logit | | |
|---|---|---|---|---|---|---|---|---|
| | | mean | (95% C.I.) | mean | (95% C.I.) | mean | (95% C.I.) | Actual |
| Roxbury | Bates | | | 0.01 | (0.00,0.02) | 0.01 | (0.00,0.01) | |
| Roxbury | Beethoven | 0.01 | (0.00,0.01) | 0.02 | (0.01,0.03) | 0.02 | (0.01,0.03) | 0.02 |
| Roxbury | Blackstone | 0.02 | (0.01,0.03) | 0.03 | (0.01,0.04) | 0.02 | (0.01,0.04) | 0.01 |
| Roxbury | Clap | | | 0.02 | (0.01,0.03) | 0.01 | (0.01,0.03) | |
| Roxbury | Conley | | | 0.01 | (0.00,0.01) | 0.01 | (0.00,0.01) | |
| Roxbury | Curley | 0.05 | (0.03,0.07) | 0.09 | (0.07,0.11) | 0.09 | (0.07,0.11) | 0.05 |
| Roxbury | Dever | | | 0.01 | (0.00,0.01) | 0.01 | (0.00,0.01) | |
| Roxbury | East Boston EEC | | | | | 0.01 | (0.00,0.01) | |
| Roxbury | Edison | 0.02 | (0.01,0.03) | 0.00 | (0.00,0.01) | 0.00 | (0.00,0.01) | |
| Roxbury | Eliot | 0.01 | (0.00,0.01) | 0.01 | (0.00,0.02) | 0.01 | (0.00,0.01) | |
| Roxbury | Ellis | 0.02 | (0.01,0.04) | 0.04 | (0.03,0.06) | 0.04 | (0.03,0.06) | 0.03 |
| Roxbury | Ellison/Parks | 0.01 | (0.00,0.01) | 0.01 | (0.00,0.01) | 0.01 | (0.00,0.01) | 0.01 |
| Roxbury | Everett | | | 0.02 | (0.01,0.03) | 0.02 | (0.01,0.03) | 0.01 |
| Roxbury | Hale | 0.22 | (0.19,0.24) | 0.02 | (0.01,0.04) | 0.02 | (0.01,0.04) | 0.02 |
| Roxbury | Haley | | | 0.01 | (0.01,0.03) | 0.01 | (0.01,0.02) | 0.01 |
| Roxbury | Haynes | 0.08 | (0.06,0.10) | 0.07 | (0.05,0.10) | 0.09 | (0.07,0.11) | 0.12 |
| Roxbury | Henderson | 0.05 | (0.03,0.06) | | | | | |
| Roxbury | Hernandez | 0.01 | (0.00,0.03) | 0.07 | (0.05,0.09) | 0.08 | (0.06,0.10) | 0.08 |
| Roxbury | Higginson/Lewis | 0.01 | (0.00,0.01) | 0.02 | (0.01,0.03) | 0.02 | (0.01,0.03) | 0.02 |
| Roxbury | Holland | | | 0.02 | (0.01,0.03) | 0.02 | (0.01,0.03) | 0.02 |
| Roxbury | Holmes | 0.01 | (0.00,0.01) | 0.01 | (0.00,0.02) | 0.01 | (0.00,0.02) | |
| Roxbury | Hurley | 0.03 | (0.02,0.04) | 0.02 | (0.01,0.03) | 0.02 | (0.01,0.03) | |
| Roxbury | J.F. Kennedy | 0.01 | (0.00,0.02) | 0.02 | (0.01,0.04) | 0.02 | (0.01,0.03) | 0.03 |
| Roxbury | Jackson/Mann | 0.01 | (0.00,0.02) | 0.00 | (0.00,0.01) | | | |
| Roxbury | Kilmer | | | 0.01 | (0.00,0.01) | 0.01 | (0.01,0.02) | 0.01 |
| Roxbury | King | 0.01 | (0.00,0.01) | 0.02 | (0.01,0.03) | 0.02 | (0.01,0.03) | |
| Roxbury | Lee | 0.01 | (0.01,0.02) | 0.03 | (0.01,0.04) | 0.03 | (0.02,0.04) | 0.03 |
| Roxbury | Lyndon | 0.01 | (0.00,0.01) | 0.02 | (0.01,0.03) | 0.01 | (0.01,0.02) | 0.02 |
| Roxbury | Manning | 0.06 | (0.04,0.08) | 0.01 | (0.01,0.02) | 0.01 | (0.01,0.02) | |
| Roxbury | Mason | 0.09 | (0.07,0.11) | 0.02 | (0.01,0.03) | 0.02 | (0.01,0.03) | 0.03 |
| Roxbury | Mather | | | 0.01 | (0.01,0.02) | 0.01 | (0.01,0.02) | |
| Roxbury | Mattahunt | 0.01 | (0.00,0.02) | | | | | |
| Roxbury | Mendell | 0.01 | (0.00,0.01) | 0.03 | (0.01,0.04) | 0.02 | (0.01,0.04) | |
| Roxbury | Mission Hill | | | 0.03 | (0.02,0.05) | 0.03 | (0.01,0.04) | 0.05 |
| Roxbury | Mozart | | | 0.01 | (0.00,0.02) | 0.01 | (0.00,0.01) | |
| Roxbury | Murphy | 0.03 | (0.02,0.05) | 0.01 | (0.00,0.02) | 0.01 | (0.01,0.02) | |
| Roxbury | Orchard Gardens | 0.01 | (0.00,0.01) | 0.02 | (0.01,0.04) | 0.02 | (0.01,0.03) | 0.05 |
| Roxbury | Otis | 0.03 | (0.02,0.04) | | | | | |
| Roxbury | Philbrick | 0.03 | (0.02,0.04) | 0.01 | (0.00,0.02) | 0.01 | (0.00,0.01) | |
| Roxbury | Quincy | 0.01 | (0.00,0.02) | 0.01 | (0.00,0.02) | 0.01 | (0.01,0.02) | 0.02 |
| Roxbury | Russell | 0.01 | (0.00,0.02) | 0.02 | (0.01,0.03) | 0.02 | (0.01,0.03) | |
| Roxbury | S. Greenwood | 0.02 | (0.01,0.03) | 0.02 | (0.01,0.03) | 0.02 | (0.01,0.04) | 0.02 |
| Roxbury | Sumner | 0.04 | (0.03,0.06) | 0.01 | (0.01,0.02) | 0.01 | (0.00,0.02) | |
| Roxbury | Taylor | 0.01 | (0.00,0.02) | | | | | |
| Roxbury | Tobin | | | 0.01 | (0.01,0.02) | 0.01 | (0.01,0.02) | 0.02 |
| Roxbury | Trotter | 0.02 | (0.01,0.02) | 0.02 | (0.01,0.03) | 0.02 | (0.01,0.03) | 0.04 |
| Roxbury | West Zone ELC | | | 0.03 | (0.02,0.05) | 0.04 | (0.02,0.05) | 0.04 |
| Roxbury | Winthrop | 0.01 | (0.00,0.02) | 0.02 | (0.01,0.03) | 0.01 | (0.01,0.02) | 0.02 |
| Roxbury | Young Achievers | 0.01 | (0.00,0.01) | 0.02 | (0.01,0.03) | 0.02 | (0.01,0.03) | 0.02 |
| South Boston | Blackstone | | | 0.03 | (0.01,0.06) | 0.03 | (0.01,0.06) | |
| South Boston | Channing | | | 0.00 | (0.00,0.01) | 0.01 | (0.00,0.02) | |
| South Boston | Chittick | | | 0.00 | (0.00,0.01) | 0.00 | (0.00,0.02) | |
| South Boston | Clap | | | 0.08 | (0.03,0.12) | 0.08 | (0.04,0.12) | 0.06 |
| South Boston | Condon | 0.07 | (0.02,0.12) | 0.14 | (0.09,0.21) | 0.14 | (0.09,0.19) | 0.21 |
| South Boston | Dever | 0.02 | (0.00,0.06) | 0.08 | (0.04,0.12) | 0.09 | (0.05,0.13) | 0.01 |

Continued on next page

**Table 5 – continued from previous page**

| Neighborhood | School | Naive mean | Naive (95% C.I.) | Logit mean | Logit (95% C.I.) | Mixed Logit mean | Mixed Logit (95% C.I.) | Actual |
|---|---|---|---|---|---|---|---|---|
| South Boston | Edison | 0.01 | (0.00,0.02) | | | | | |
| South Boston | Eliot | | | 0.01 | (0.00,0.02) | 0.01 | (0.00,0.02) | 0.01 |
| South Boston | Ellison/Parks | 0.08 | (0.04,0.11) | 0.01 | (0.00,0.03) | 0.02 | (0.00,0.04) | 0.02 |
| South Boston | Everett | | | 0.03 | (0.01,0.06) | 0.02 | (0.01,0.05) | |
| South Boston | Harvard/Kent | 0.01 | (0.00,0.03) | 0.00 | (0.00,0.02) | 0.01 | (0.00,0.02) | 0.03 |
| South Boston | Henderson | 0.03 | (0.01,0.06) | 0.02 | (0.00,0.04) | 0.01 | (0.00,0.03) | 0.01 |
| South Boston | Hernandez | | | 0.02 | (0.01,0.05) | 0.02 | (0.01,0.04) | 0.02 |
| South Boston | Holland | 0.01 | (0.00,0.03) | 0.01 | (0.00,0.03) | 0.01 | (0.00,0.03) | |
| South Boston | Holmes | | | 0.00 | (0.00,0.02) | 0.00 | (0.00,0.01) | |
| South Boston | Hurley | 0.01 | (0.00,0.03) | 0.00 | (0.00,0.01) | 0.00 | (0.00,0.01) | |
| South Boston | Kenny | | | 0.01 | (0.00,0.02) | 0.01 | (0.00,0.02) | |
| South Boston | Lee | 0.03 | (0.00,0.06) | 0.02 | (0.00,0.04) | 0.02 | (0.00,0.04) | 0.03 |
| South Boston | Mason | 0.05 | (0.02,0.09) | 0.01 | (0.00,0.03) | 0.01 | (0.00,0.03) | 0.01 |
| South Boston | Mather | 0.01 | (0.00,0.03) | 0.02 | (0.00,0.04) | 0.02 | (0.00,0.04) | |
| South Boston | Mattahunt | 0.01 | (0.00,0.04) | 0.00 | (0.00,0.01) | 0.00 | (0.00,0.01) | |
| South Boston | Murphy | 0.36 | (0.27,0.45) | 0.08 | (0.04,0.12) | 0.08 | (0.04,0.13) | 0.07 |
| South Boston | Orchard Gardens | | | 0.00 | (0.00,0.01) | 0.00 | (0.00,0.01) | |
| South Boston | Otis | 0.01 | (0.00,0.02) | | | | | |
| South Boston | Perry | 0.03 | (0.01,0.06) | 0.17 | (0.12,0.22) | 0.18 | (0.12,0.24) | 0.24 |
| South Boston | Quincy | 0.12 | (0.06,0.19) | 0.06 | (0.02,0.10) | 0.06 | (0.02,0.11) | 0.07 |
| South Boston | Roosevelt | | | 0.00 | (0.00,0.02) | 0.01 | (0.00,0.03) | 0.02 |
| South Boston | Russell | 0.06 | (0.03,0.10) | 0.05 | (0.02,0.09) | 0.04 | (0.02,0.07) | 0.01 |
| South Boston | S. Greenwood | 0.04 | (0.02,0.07) | 0.01 | (0.00,0.03) | 0.01 | (0.00,0.03) | 0.01 |
| South Boston | Taylor | | | 0.00 | (0.00,0.01) | 0.00 | (0.00,0.01) | |
| South Boston | Tynan | 0.03 | (0.01,0.06) | 0.08 | (0.04,0.11) | 0.08 | (0.04,0.12) | 0.05 |
| South Boston | Young Achievers | | | 0.02 | (0.00,0.04) | 0.02 | (0.00,0.05) | 0.03 |
| South Dorchester | Channing | | | 0.01 | (0.00,0.01) | 0.01 | (0.00,0.02) | |
| South Dorchester | Chittick | | | 0.01 | (0.01,0.02) | 0.01 | (0.00,0.02) | |
| South Dorchester | Clap | | | 0.04 | (0.02,0.05) | 0.03 | (0.02,0.04) | 0.03 |
| South Dorchester | Condon | 0.01 | (0.00,0.02) | 0.03 | (0.01,0.04) | 0.02 | (0.01,0.03) | 0.03 |
| South Dorchester | Dever | 0.01 | (0.00,0.02) | 0.03 | (0.02,0.04) | 0.03 | (0.02,0.05) | 0.02 |
| South Dorchester | Ellison/Parks | 0.09 | (0.07,0.11) | 0.04 | (0.03,0.06) | 0.05 | (0.04,0.07) | 0.06 |
| South Dorchester | Everett | 0.01 | (0.00,0.01) | 0.04 | (0.02,0.05) | 0.03 | (0.02,0.05) | 0.03 |
| South Dorchester | Haynes | 0.03 | (0.02,0.04) | 0.02 | (0.01,0.03) | 0.02 | (0.01,0.03) | 0.02 |
| South Dorchester | Henderson | 0.24 | (0.22,0.27) | 0.07 | (0.05,0.09) | 0.07 | (0.05,0.09) | 0.08 |
| South Dorchester | Hernandez | | | 0.03 | (0.01,0.04) | 0.02 | (0.01,0.03) | 0.02 |
| South Dorchester | Holland | 0.07 | (0.05,0.09) | 0.05 | (0.03,0.06) | 0.05 | (0.04,0.07) | 0.05 |
| South Dorchester | Holmes | 0.01 | (0.00,0.01) | 0.02 | (0.01,0.03) | 0.02 | (0.01,0.03) | 0.02 |
| South Dorchester | Kenny | 0.01 | (0.01,0.02) | 0.04 | (0.02,0.05) | 0.04 | (0.03,0.05) | 0.03 |
| South Dorchester | King | | | 0.01 | (0.00,0.01) | 0.01 | (0.00,0.01) | |
| South Dorchester | Lee | 0.04 | (0.03,0.06) | 0.09 | (0.07,0.11) | 0.08 | (0.06,0.10) | 0.10 |
| South Dorchester | Mather | 0.06 | (0.04,0.08) | 0.06 | (0.05,0.08) | 0.07 | (0.05,0.09) | 0.06 |
| South Dorchester | Mattahunt | 0.01 | (0.00,0.02) | 0.01 | (0.00,0.02) | 0.01 | (0.00,0.02) | 0.01 |
| South Dorchester | Murphy | 0.33 | (0.29,0.36) | 0.25 | (0.21,0.28) | 0.27 | (0.23,0.31) | 0.29 |
| South Dorchester | Perry | | | 0.02 | (0.01,0.03) | 0.02 | (0.01,0.03) | 0.01 |
| South Dorchester | Roosevelt | | | 0.02 | (0.01,0.03) | 0.02 | (0.01,0.03) | 0.01 |
| South Dorchester | Russell | 0.02 | (0.01,0.03) | 0.03 | (0.01,0.04) | 0.02 | (0.01,0.04) | 0.02 |
| South Dorchester | S. Greenwood | 0.03 | (0.01,0.04) | 0.03 | (0.02,0.05) | 0.03 | (0.02,0.04) | 0.02 |
| South Dorchester | Taylor | 0.01 | (0.00,0.01) | 0.01 | (0.01,0.03) | 0.01 | (0.01,0.02) | |
| South Dorchester | Tynan | 0.01 | (0.00,0.01) | 0.01 | (0.00,0.02) | 0.01 | (0.00,0.01) | 0.01 |
| South Dorchester | Young Achievers | | | 0.04 | (0.03,0.06) | 0.05 | (0.03,0.06) | 0.05 |
| South End | Adams | 0.04 | (0.02,0.07) | | | 0.00 | (0.00,0.01) | |
| South End | Baldwin | 0.02 | (0.00,0.03) | 0.03 | (0.01,0.06) | 0.03 | (0.01,0.06) | 0.04 |
| South End | Blackstone | 0.03 | (0.01,0.06) | 0.14 | (0.10,0.19) | 0.14 | (0.10,0.19) | 0.12 |
| South End | Bradley | | | 0.00 | (0.00,0.01) | 0.01 | (0.00,0.03) | |

Continued on next page

**Table 5 – continued from previous page**

| | | Naive | | Logit | | Mixed Logit | | |
|---|---|---|---|---|---|---|---|---|
| Neighborhood | School | mean | (95% C.I.) | mean | (95% C.I.) | mean | (95% C.I.) | Actual |
| South End | Channing | 0.01 | (0.00,0.02) | | | | | |
| South End | Condon | | | 0.02 | (0.00,0.04) | 0.01 | (0.00,0.03) | |
| South End | East Boston EEC | | | 0.01 | (0.00,0.03) | 0.02 | (0.01,0.04) | 0.01 |
| South End | Edison | 0.07 | (0.04,0.10) | 0.02 | (0.00,0.04) | 0.02 | (0.00,0.04) | |
| South End | Eliot | 0.04 | (0.01,0.07) | 0.10 | (0.06,0.14) | 0.09 | (0.05,0.12) | 0.13 |
| South End | Gardner | 0.01 | (0.00,0.03) | 0.02 | (0.01,0.04) | 0.02 | (0.00,0.04) | 0.02 |
| South End | Hale | 0.03 | (0.01,0.05) | 0.01 | (0.00,0.03) | 0.01 | (0.00,0.03) | |
| South End | Harvard/Kent | 0.02 | (0.01,0.05) | 0.03 | (0.01,0.05) | 0.02 | (0.01,0.04) | |
| South End | Hernandez | 0.01 | (0.00,0.03) | 0.04 | (0.01,0.07) | 0.04 | (0.02,0.06) | 0.01 |
| South End | Higginson/Lewis | | | 0.00 | (0.00,0.01) | 0.00 | (0.00,0.01) | |
| South End | Hurley | 0.27 | (0.22,0.32) | 0.13 | (0.08,0.17) | 0.13 | (0.09,0.17) | 0.18 |
| South End | Jackson/Mann | | | 0.02 | (0.00,0.03) | 0.01 | (0.00,0.02) | |
| South End | Kennedy Patrick | | | 0.00 | (0.00,0.01) | 0.00 | (0.00,0.01) | |
| South End | Mason | 0.03 | (0.01,0.04) | 0.03 | (0.01,0.05) | 0.03 | (0.01,0.05) | 0.02 |
| South End | Mission Hill | 0.01 | (0.00,0.02) | 0.01 | (0.00,0.01) | 0.01 | (0.00,0.01) | 0.02 |
| South End | O'Donnell | | | 0.00 | (0.00,0.01) | 0.00 | (0.00,0.01) | |
| South End | Orchard Gardens | 0.02 | (0.00,0.04) | 0.06 | (0.03,0.09) | 0.05 | (0.03,0.07) | 0.06 |
| South End | Otis | 0.09 | (0.06,0.13) | 0.01 | (0.00,0.02) | 0.01 | (0.00,0.03) | |
| South End | Quincy | 0.29 | (0.21,0.35) | 0.28 | (0.22,0.34) | 0.30 | (0.22,0.36) | 0.33 |
| South End | S. Greenwood | 0.00 | (0.00,0.01) | | | | | |
| South End | Tobin | 0.02 | (0.00,0.04) | 0.03 | (0.01,0.06) | 0.03 | (0.01,0.06) | |
| South End | Winship | | | 0.01 | (0.00,0.03) | 0.01 | (0.00,0.02) | |
| South End | Winthrop | | | 0.01 | (0.00,0.02) | 0.00 | (0.00,0.01) | |
| West Roxbury | BTU | | | 0.03 | (0.02,0.05) | 0.03 | (0.02,0.05) | 0.02 |
| West Roxbury | Bates | 0.01 | (0.01,0.03) | 0.04 | (0.02,0.06) | 0.04 | (0.02,0.06) | 0.05 |
| West Roxbury | Beethoven | 0.03 | (0.02,0.05) | 0.18 | (0.14,0.21) | 0.17 | (0.14,0.20) | 0.19 |
| West Roxbury | Channing | | | 0.02 | (0.01,0.03) | 0.02 | (0.01,0.04) | 0.02 |
| West Roxbury | Conley | 0.02 | (0.01,0.04) | 0.02 | (0.01,0.03) | 0.02 | (0.01,0.03) | 0.02 |
| West Roxbury | Curley | 0.04 | (0.02,0.06) | 0.03 | (0.01,0.05) | 0.03 | (0.01,0.04) | 0.01 |
| West Roxbury | Ellis | | | 0.00 | (0.00,0.01) | 0.00 | (0.00,0.01) | |
| West Roxbury | Haley | | | 0.02 | (0.01,0.03) | 0.01 | (0.00,0.02) | 0.02 |
| West Roxbury | Harvard/Kent | 0.02 | (0.01,0.03) | | | | | |
| West Roxbury | Haynes | 0.08 | (0.06,0.10) | 0.01 | (0.00,0.01) | 0.01 | (0.01,0.03) | 0.02 |
| West Roxbury | Hernandez | 0.00 | (0.00,0.02) | 0.01 | (0.00,0.02) | 0.01 | (0.00,0.02) | 0.01 |
| West Roxbury | Holland | 0.00 | (0.00,0.01) | | | | | |
| West Roxbury | J.F. Kennedy | | | 0.00 | (0.00,0.01) | 0.01 | | |
| West Roxbury | Kilmer | 0.32 | (0.28,0.35) | 0.27 | (0.24,0.31) | 0.29 | (0.26,0.33) | 0.29 |
| West Roxbury | Lyndon | 0.34 | (0.31,0.37) | 0.21 | (0.17,0.24) | 0.21 | (0.18,0.24) | 0.25 |
| West Roxbury | Manning | 0.02 | (0.01,0.03) | 0.03 | (0.02,0.05) | 0.03 | (0.02,0.04) | |
| West Roxbury | Mather | 0.01 | (0.00,0.02) | | | | | |
| West Roxbury | Mendell | | | 0.00 | (0.00,0.01) | 0.00 | (0.00,0.01) | |
| West Roxbury | Mission Hill | | | 0.01 | (0.00,0.03) | 0.01 | (0.00,0.02) | 0.02 |
| West Roxbury | Mozart | 0.01 | (0.00,0.02) | 0.06 | (0.04,0.09) | 0.05 | (0.04,0.07) | 0.03 |
| West Roxbury | Philbrick | 0.00 | (0.00,0.01) | 0.01 | (0.00,0.03) | 0.01 | (0.00,0.02) | |
| West Roxbury | Sumner | 0.07 | (0.04,0.09) | 0.02 | (0.01,0.03) | 0.02 | (0.01,0.03) | 0.02 |
| West Roxbury | West Zone ELC | | | 0.01 | (0.00,0.01) | 0.01 | (0.00,0.02) | 0.01 |

Table 6: Top 3 Choices Market Share Predictions for 2013 K1

| | | Naive | | Logit | | Mixed Logit | | |
|---|---|---|---|---|---|---|---|---|
| Neighborhood | School | mean | (95% C.I.) | mean | (95% C.I.) | mean | (95% C.I.) | Actual |
| Allston-Brighton | Adams | 0.06 | (0.04,0.07) | | | 0.00 | (0.00,0.01) | |

Continued on next page

**Table 6 – continued from previous page**

| Neighborhood | School | Naive mean | Naive (95% C.I.) | Logit mean | Logit (95% C.I.) | Mixed Logit mean | Mixed Logit (95% C.I.) | Actual |
|---|---|---|---|---|---|---|---|---|
| Allston-Brighton | Baldwin | 0.07 | (0.06,0.08) | 0.19 | (0.16,0.22) | 0.18 | (0.16,0.21) | 0.31 |
| Allston-Brighton | Blackstone | 0.04 | (0.02,0.06) | 0.03 | (0.01,0.05) | 0.03 | (0.01,0.04) | |
| Allston-Brighton | Bradley | | | 0.00 | (0.00,0.01) | 0.01 | (0.00,0.02) | |
| Allston-Brighton | East Boston EEC | 0.06 | (0.04,0.08) | 0.01 | (0.00,0.02) | 0.02 | (0.01,0.04) | |
| Allston-Brighton | Edison | 0.13 | (0.10,0.16) | 0.19 | (0.15,0.23) | 0.18 | (0.15,0.21) | 0.12 |
| Allston-Brighton | Eliot | | | 0.04 | (0.02,0.05) | 0.03 | (0.02,0.05) | 0.01 |
| Allston-Brighton | Ellison/Parks | 0.01 | (0.00,0.02) | | | | | |
| Allston-Brighton | Gardner | 0.02 | (0.01,0.03) | 0.13 | (0.10,0.16) | 0.14 | (0.11,0.17) | 0.13 |
| Allston-Brighton | Harvard/Kent | 0.04 | (0.03,0.07) | 0.02 | (0.01,0.04) | 0.02 | (0.01,0.03) | |
| Allston-Brighton | Hernandez | 0.01 | (0.00,0.01) | 0.03 | (0.01,0.04) | 0.03 | (0.01,0.04) | |
| Allston-Brighton | Hurley | 0.19 | (0.16,0.22) | 0.03 | (0.02,0.05) | 0.03 | (0.02,0.05) | |
| Allston-Brighton | Jackson/Mann | 0.03 | (0.01,0.06) | 0.12 | (0.09,0.16) | 0.12 | (0.09,0.16) | 0.16 |
| Allston-Brighton | Mason | 0.04 | (0.03,0.06) | 0.01 | (0.00,0.01) | 0.01 | (0.00,0.01) | 0.01 |
| Allston-Brighton | Mission Hill | | | | | 0.01 | | |
| Allston-Brighton | Orchard Gardens | | | 0.01 | (0.00,0.02) | 0.01 | (0.00,0.02) | |
| Allston-Brighton | Otis | 0.13 | (0.10,0.15) | 0.01 | (0.00,0.01) | 0.01 | (0.00,0.02) | |
| Allston-Brighton | Quincy | 0.17 | (0.13,0.21) | 0.05 | (0.03,0.07) | 0.05 | (0.03,0.07) | 0.04 |
| Allston-Brighton | Tobin | | | 0.01 | (0.00,0.02) | 0.01 | (0.00,0.02) | |
| Allston-Brighton | Winship | 0.01 | (0.00,0.02) | 0.12 | (0.09,0.15) | 0.12 | (0.09,0.15) | 0.17 |
| Charlestown | Adams | 0.04 | (0.01,0.08) | 0.01 | (0.00,0.02) | 0.01 | (0.00,0.02) | |
| Charlestown | Baldwin | 0.02 | (0.01,0.03) | 0.03 | (0.01,0.06) | 0.03 | (0.01,0.06) | 0.03 |
| Charlestown | Beethoven | 0.01 | (0.00,0.01) | | | | | |
| Charlestown | Blackstone | 0.03 | (0.01,0.06) | 0.03 | (0.01,0.07) | 0.03 | (0.01,0.07) | 0.03 |
| Charlestown | Bradley | | | 0.02 | (0.00,0.04) | 0.01 | (0.00,0.04) | 0.01 |
| Charlestown | Dever | 0.01 | (0.00,0.02) | | | | | |
| Charlestown | East Boston EEC | 0.01 | (0.00,0.02) | 0.03 | (0.00,0.06) | 0.03 | (0.00,0.07) | 0.04 |
| Charlestown | Edison | 0.02 | (0.00,0.05) | 0.01 | (0.00,0.03) | 0.01 | (0.00,0.03) | |
| Charlestown | Eliot | 0.44 | (0.34,0.52) | 0.35 | (0.28,0.43) | 0.38 | (0.30,0.45) | 0.45 |
| Charlestown | Gardner | | | 0.02 | (0.00,0.04) | 0.01 | (0.00,0.04) | |
| Charlestown | Harvard/Kent | 0.27 | (0.23,0.31) | 0.19 | (0.14,0.24) | 0.20 | (0.15,0.26) | 0.27 |
| Charlestown | Hernandez | | | 0.01 | (0.00,0.03) | 0.01 | (0.00,0.03) | |
| Charlestown | Hurley | 0.06 | (0.02,0.11) | 0.04 | (0.01,0.07) | 0.03 | (0.01,0.07) | 0.02 |
| Charlestown | Jackson/Mann | | | 0.01 | (0.00,0.03) | 0.01 | (0.00,0.02) | |
| Charlestown | Kennedy Patrick | | | 0.01 | (0.00,0.03) | 0.01 | (0.00,0.03) | |
| Charlestown | Mason | 0.01 | (0.00,0.02) | 0.01 | (0.00,0.02) | 0.00 | (0.00,0.02) | |
| Charlestown | O'Donnell | | | 0.02 | (0.00,0.04) | 0.01 | (0.00,0.03) | |
| Charlestown | Orchard Gardens | 0.01 | (0.00,0.01) | 0.01 | (0.00,0.03) | 0.01 | (0.00,0.02) | |
| Charlestown | Otis | 0.03 | (0.01,0.06) | 0.03 | (0.00,0.05) | 0.02 | (0.00,0.04) | |
| Charlestown | Quincy | 0.03 | (0.00,0.07) | 0.16 | (0.10,0.22) | 0.17 | (0.10,0.23) | 0.11 |
| Charlestown | Roosevelt | 0.01 | (0.00,0.01) | | | | | |
| Charlestown | Taylor | 0.01 | (0.00,0.03) | | | | | |
| Charlestown | Tobin | 0.01 | (0.00,0.03) | 0.01 | (0.00,0.03) | 0.01 | (0.00,0.03) | |
| Charlestown | Winship | 0.01 | (0.00,0.02) | 0.01 | (0.00,0.03) | 0.01 | (0.00,0.02) | |
| Charlestown | Winthrop | | | 0.00 | (0.00,0.01) | | | |
| Downtown | Adams | 0.02 | (0.01,0.03) | | | | | |
| Downtown | Baldwin | | | 0.03 | (0.02,0.05) | 0.03 | (0.01,0.04) | 0.03 |
| Downtown | Blackstone | 0.02 | (0.00,0.03) | 0.06 | (0.04,0.09) | 0.06 | (0.04,0.09) | 0.03 |
| Downtown | Bradley | | | 0.01 | (0.00,0.02) | 0.01 | (0.00,0.02) | |
| Downtown | Chittick | 0.01 | (0.00,0.02) | | | | | |
| Downtown | Condon | | | 0.01 | (0.00,0.02) | 0.01 | (0.00,0.02) | |
| Downtown | East Boston EEC | 0.04 | (0.03,0.07) | 0.01 | (0.00,0.02) | 0.02 | (0.01,0.04) | 0.02 |
| Downtown | Edison | 0.07 | (0.05,0.10) | 0.02 | (0.01,0.03) | 0.02 | (0.01,0.03) | |
| Downtown | Eliot | 0.26 | (0.21,0.31) | 0.29 | (0.24,0.34) | 0.29 | (0.24,0.34) | 0.36 |
| Downtown | Gardner | | | 0.02 | (0.01,0.04) | 0.02 | (0.01,0.03) | |
| Downtown | Hale | 0.02 | (0.01,0.03) | 0.00 | (0.00,0.01) | 0.00 | (0.00,0.01) | |

Continued on next page

**Table 6 – continued from previous page**

| Neighborhood | School | Naive mean | Naive (95% C.I.) | Logit mean | Logit (95% C.I.) | Mixed Logit mean | Mixed Logit (95% C.I.) | Actual |
|---|---|---|---|---|---|---|---|---|
| Downtown | Harvard/Kent | 0.10 | (0.07,0.13) | 0.07 | (0.05,0.10) | 0.07 | (0.05,0.10) | 0.05 |
| Downtown | Hernandez | | | 0.02 | (0.01,0.03) | 0.02 | (0.01,0.03) | 0.02 |
| Downtown | Hurley | 0.08 | (0.06,0.10) | 0.05 | (0.03,0.08) | 0.05 | (0.03,0.07) | 0.07 |
| Downtown | Jackson/Mann | | | 0.02 | (0.01,0.03) | 0.01 | (0.00,0.02) | 0.02 |
| Downtown | Kennedy Patrick | | | 0.00 | (0.00,0.01) | 0.00 | (0.00,0.01) | |
| Downtown | Mason | 0.02 | (0.01,0.03) | 0.01 | (0.00,0.02) | 0.01 | (0.00,0.02) | |
| Downtown | Mission Hill | | | | | 0.02 | | |
| Downtown | O'Donnell | | | 0.00 | (0.00,0.01) | 0.00 | (0.00,0.01) | |
| Downtown | Orchard Gardens | 0.00 | (0.00,0.01) | 0.02 | (0.01,0.04) | 0.02 | (0.01,0.03) | 0.03 |
| Downtown | Otis | 0.07 | (0.05,0.10) | 0.01 | (0.00,0.02) | 0.01 | (0.00,0.02) | |
| Downtown | Quincy | 0.28 | (0.23,0.34) | 0.30 | (0.25,0.34) | 0.30 | (0.25,0.35) | 0.31 |
| Downtown | Tobin | | | 0.02 | (0.01,0.03) | 0.02 | (0.01,0.04) | 0.01 |
| Downtown | West Zone ELC | | | 0.01 | (0.00,0.02) | 0.01 | (0.00,0.02) | |
| Downtown | Winship | | | 0.01 | (0.00,0.02) | 0.01 | (0.00,0.02) | |
| Downtown | Winthrop | | | 0.00 | (0.00,0.01) | | | |
| East Boston | Adams | 0.17 | (0.16,0.19) | 0.11 | (0.07,0.14) | 0.11 | (0.09,0.13) | 0.07 |
| East Boston | Baldwin | | | | | 0.01 | (0.00,0.01) | |
| East Boston | Blackstone | 0.15 | (0.13,0.17) | 0.02 | (0.01,0.03) | 0.02 | (0.01,0.03) | 0.02 |
| East Boston | Bradley | 0.07 | (0.05,0.09) | 0.13 | (0.10,0.15) | 0.13 | (0.11,0.16) | 0.11 |
| East Boston | East Boston EEC | 0.10 | (0.08,0.12) | 0.26 | (0.23,0.29) | 0.25 | (0.23,0.28) | 0.34 |
| East Boston | Edison | 0.07 | (0.05,0.08) | 0.01 | (0.00,0.01) | 0.01 | (0.01,0.02) | |
| East Boston | Eliot | | | 0.03 | (0.02,0.04) | 0.02 | (0.01,0.04) | 0.04 |
| East Boston | Gardner | | | 0.01 | (0.00,0.01) | 0.01 | (0.00,0.01) | |
| East Boston | Harvard/Kent | 0.01 | (0.01,0.02) | 0.02 | (0.01,0.03) | 0.01 | (0.01,0.02) | |
| East Boston | Hernandez | | | 0.01 | (0.00,0.01) | 0.02 | (0.01,0.03) | |
| East Boston | Hurley | 0.17 | (0.15,0.18) | 0.02 | (0.01,0.02) | 0.02 | (0.01,0.03) | |
| East Boston | Jackson/Mann | 0.00 | (0.00,0.01) | | | | | |
| East Boston | Kennedy Patrick | 0.01 | (0.01,0.02) | 0.09 | (0.07,0.12) | 0.07 | (0.06,0.09) | 0.11 |
| East Boston | O'Donnell | 0.01 | (0.01,0.02) | 0.07 | (0.05,0.10) | 0.06 | (0.04,0.07) | 0.08 |
| East Boston | Orchard Gardens | 0.01 | (0.00,0.01) | | | | | |
| East Boston | Otis | 0.20 | (0.18,0.23) | 0.22 | (0.20,0.25) | 0.21 | (0.19,0.24) | 0.17 |
| East Boston | Quincy | | | 0.01 | (0.01,0.02) | 0.01 | (0.01,0.02) | 0.02 |
| Hyde Park | BTU | | | 0.01 | (0.00,0.02) | 0.01 | (0.00,0.02) | |
| Hyde Park | Bates | | | 0.02 | (0.01,0.03) | 0.02 | (0.01,0.03) | 0.02 |
| Hyde Park | Beethoven | 0.01 | (0.00,0.02) | 0.05 | (0.03,0.06) | 0.05 | (0.03,0.06) | 0.06 |
| Hyde Park | Channing | 0.02 | (0.01,0.03) | 0.10 | (0.08,0.12) | 0.10 | (0.08,0.13) | 0.13 |
| Hyde Park | Chittick | | | 0.07 | (0.05,0.09) | 0.07 | (0.04,0.09) | 0.07 |
| Hyde Park | Clap | | | 0.01 | (0.01,0.02) | 0.01 | (0.00,0.02) | |
| Hyde Park | Condon | 0.01 | (0.00,0.02) | 0.01 | (0.00,0.02) | 0.01 | (0.00,0.02) | |
| Hyde Park | Conley | 0.11 | (0.09,0.14) | 0.03 | (0.02,0.05) | 0.04 | (0.02,0.05) | 0.04 |
| Hyde Park | Curley | 0.02 | (0.01,0.03) | 0.01 | (0.00,0.02) | 0.01 | (0.00,0.02) | |
| Hyde Park | Dever | 0.02 | (0.01,0.03) | 0.01 | (0.00,0.02) | 0.01 | (0.00,0.02) | 0.01 |
| Hyde Park | Ellison/Parks | 0.07 | (0.06,0.09) | 0.08 | (0.06,0.11) | 0.09 | (0.07,0.11) | 0.08 |
| Hyde Park | Everett | | | 0.01 | (0.00,0.02) | 0.01 | (0.00,0.02) | |
| Hyde Park | Haley | | | 0.01 | (0.00,0.02) | 0.01 | (0.00,0.02) | |
| Hyde Park | Haynes | 0.01 | (0.01,0.02) | | | | | |
| Hyde Park | Henderson | 0.19 | (0.17,0.21) | 0.02 | (0.01,0.03) | 0.02 | (0.01,0.03) | |
| Hyde Park | Hernandez | | | 0.03 | (0.01,0.04) | 0.02 | (0.01,0.03) | 0.05 |
| Hyde Park | Holland | 0.01 | (0.00,0.01) | 0.01 | (0.00,0.02) | 0.01 | (0.00,0.01) | |
| Hyde Park | Holmes | | | 0.01 | (0.00,0.01) | 0.00 | (0.00,0.01) | |
| Hyde Park | Kenny | | | 0.01 | (0.00,0.02) | 0.01 | (0.00,0.02) | |
| Hyde Park | Kilmer | | | 0.01 | (0.00,0.02) | 0.01 | (0.01,0.02) | 0.02 |
| Hyde Park | Lee | 0.02 | (0.00,0.02) | 0.04 | (0.03,0.06) | 0.03 | (0.02,0.05) | 0.03 |
| Hyde Park | Lyndon | | | 0.01 | (0.00,0.02) | 0.01 | (0.00,0.02) | |
| Hyde Park | Mather | 0.01 | (0.00,0.02) | 0.01 | (0.00,0.02) | 0.01 | (0.00,0.02) | |

Continued on next page

**Table 6 – continued from previous page**

| Neighborhood | School | Naive mean | Naive (95% C.I.) | Logit mean | Logit (95% C.I.) | Mixed Logit mean | Mixed Logit (95% C.I.) | Actual |
|---|---|---|---|---|---|---|---|---|
| Hyde Park | Mattahunt | 0.01 | (0.00,0.02) | 0.04 | (0.03,0.06) | 0.04 | (0.03,0.06) | 0.04 |
| Hyde Park | Mission Hill | | | 0.00 | (0.00,0.01) | | | |
| Hyde Park | Mozart | | | 0.01 | (0.00,0.02) | 0.01 | (0.00,0.02) | |
| Hyde Park | Murphy | 0.11 | (0.09,0.13) | 0.06 | (0.04,0.08) | 0.06 | (0.04,0.09) | 0.06 |
| Hyde Park | Perry | | | 0.01 | (0.00,0.02) | 0.01 | (0.00,0.02) | |
| Hyde Park | Philbrick | 0.04 | (0.02,0.05) | 0.01 | (0.00,0.02) | 0.01 | (0.00,0.01) | 0.02 |
| Hyde Park | Roosevelt | 0.23 | (0.21,0.25) | 0.16 | (0.14,0.19) | 0.17 | (0.14,0.19) | 0.17 |
| Hyde Park | Russell | 0.02 | (0.01,0.03) | 0.01 | (0.00,0.02) | 0.01 | (0.00,0.02) | |
| Hyde Park | S. Greenwood | 0.02 | (0.01,0.04) | 0.02 | (0.01,0.03) | 0.01 | (0.00,0.03) | 0.02 |
| Hyde Park | Sumner | 0.03 | (0.02,0.05) | 0.01 | (0.00,0.02) | 0.01 | (0.00,0.02) | |
| Hyde Park | Taylor | 0.02 | (0.01,0.03) | 0.02 | (0.01,0.03) | 0.02 | (0.01,0.03) | |
| Hyde Park | Young Achievers | 0.01 | (0.00,0.01) | 0.07 | (0.05,0.09) | 0.07 | (0.06,0.09) | 0.07 |
| Jamaica Plain | Adams | 0.01 | (0.00,0.01) | | | | | |
| Jamaica Plain | BTU | 0.01 | (0.00,0.01) | 0.07 | (0.06,0.10) | 0.07 | (0.05,0.09) | 0.10 |
| Jamaica Plain | Baldwin | | | 0.01 | (0.01,0.03) | 0.01 | (0.01,0.02) | 0.01 |
| Jamaica Plain | Bates | | | 0.01 | (0.00,0.02) | 0.01 | (0.00,0.02) | |
| Jamaica Plain | Beethoven | | | 0.02 | (0.01,0.04) | 0.02 | (0.01,0.04) | 0.03 |
| Jamaica Plain | Blackstone | 0.01 | (0.00,0.02) | 0.02 | (0.01,0.03) | 0.02 | (0.01,0.03) | 0.02 |
| Jamaica Plain | Conley | | | 0.01 | (0.00,0.02) | 0.01 | (0.00,0.01) | |
| Jamaica Plain | Curley | 0.06 | (0.04,0.08) | 0.19 | (0.15,0.23) | 0.20 | (0.17,0.24) | 0.23 |
| Jamaica Plain | Dever | 0.00 | (0.00,0.01) | | | | | |
| Jamaica Plain | East Boston EEC | 0.01 | (0.00,0.02) | | | 0.01 | (0.00,0.01) | |
| Jamaica Plain | Edison | 0.03 | (0.01,0.04) | 0.01 | (0.00,0.02) | 0.01 | (0.00,0.02) | |
| Jamaica Plain | Eliot | | | 0.01 | (0.00,0.02) | 0.01 | (0.00,0.02) | |
| Jamaica Plain | Ellis | | | 0.02 | (0.01,0.04) | 0.02 | (0.01,0.03) | 0.01 |
| Jamaica Plain | Gardner | | | 0.01 | (0.00,0.02) | 0.01 | (0.00,0.01) | |
| Jamaica Plain | Hale | 0.19 | (0.17,0.21) | 0.02 | (0.01,0.03) | 0.02 | (0.01,0.03) | |
| Jamaica Plain | Haley | | | 0.02 | (0.01,0.04) | 0.02 | (0.01,0.03) | |
| Jamaica Plain | Harvard/Kent | 0.02 | (0.01,0.03) | 0.01 | (0.00,0.02) | 0.01 | (0.00,0.02) | |
| Jamaica Plain | Haynes | 0.03 | (0.02,0.05) | 0.01 | (0.01,0.02) | 0.02 | (0.01,0.03) | 0.02 |
| Jamaica Plain | Hernandez | 0.03 | (0.01,0.04) | 0.05 | (0.03,0.07) | 0.06 | (0.04,0.08) | 0.07 |
| Jamaica Plain | Higginson/Lewis | | | 0.01 | (0.00,0.02) | 0.01 | (0.00,0.02) | |
| Jamaica Plain | Hurley | 0.04 | (0.03,0.06) | 0.02 | (0.01,0.03) | 0.02 | (0.01,0.03) | |
| Jamaica Plain | J.F. Kennedy | 0.01 | (0.00,0.01) | 0.03 | (0.02,0.06) | 0.03 | (0.01,0.04) | 0.06 |
| Jamaica Plain | Jackson/Mann | 0.01 | (0.00,0.02) | 0.01 | (0.00,0.02) | 0.01 | (0.00,0.01) | |
| Jamaica Plain | Kilmer | | | 0.03 | (0.02,0.05) | 0.05 | (0.03,0.07) | 0.03 |
| Jamaica Plain | Lyndon | | | 0.03 | (0.02,0.04) | 0.03 | (0.01,0.04) | 0.02 |
| Jamaica Plain | Manning | 0.21 | (0.18,0.23) | 0.06 | (0.04,0.08) | 0.07 | (0.05,0.09) | 0.05 |
| Jamaica Plain | Mason | 0.03 | (0.01,0.04) | 0.00 | (0.00,0.01) | | | |
| Jamaica Plain | Mendell | | | 0.04 | (0.02,0.05) | 0.03 | (0.02,0.04) | 0.05 |
| Jamaica Plain | Mission Hill | | | 0.07 | (0.05,0.09) | 0.07 | (0.05,0.09) | 0.14 |
| Jamaica Plain | Mozart | | | 0.02 | (0.01,0.03) | 0.01 | (0.00,0.02) | 0.01 |
| Jamaica Plain | Orchard Gardens | | | 0.01 | (0.00,0.02) | 0.01 | (0.00,0.02) | |
| Jamaica Plain | Otis | 0.03 | (0.01,0.04) | | | | | |
| Jamaica Plain | Philbrick | 0.17 | (0.15,0.19) | 0.01 | (0.01,0.03) | 0.01 | (0.00,0.02) | |
| Jamaica Plain | Quincy | 0.01 | (0.00,0.02) | 0.02 | (0.01,0.03) | 0.02 | (0.01,0.04) | |
| Jamaica Plain | Sumner | 0.09 | (0.07,0.11) | 0.01 | (0.00,0.02) | 0.01 | (0.00,0.02) | |
| Jamaica Plain | Tobin | | | 0.02 | (0.01,0.03) | 0.02 | (0.01,0.03) | 0.03 |
| Jamaica Plain | Trotter | | | 0.01 | (0.00,0.01) | 0.01 | (0.00,0.01) | |
| Jamaica Plain | West Zone ELC | | | 0.06 | (0.03,0.08) | 0.06 | (0.05,0.08) | 0.05 |
| Jamaica Plain | Winship | | | 0.01 | (0.00,0.01) | 0.00 | (0.00,0.01) | |
| Mattapan | BTU | | | 0.01 | (0.00,0.01) | 0.01 | (0.00,0.01) | |
| Mattapan | Beethoven | 0.01 | (0.00,0.01) | 0.01 | (0.00,0.01) | 0.01 | (0.00,0.01) | |
| Mattapan | Blackstone | 0.01 | (0.00,0.02) | | | | | |
| Mattapan | Channing | | | 0.02 | (0.01,0.04) | 0.02 | (0.01,0.03) | 0.02 |

Continued on next page

**Table 6 – continued from previous page**

| Neighborhood | School | Naive | | Logit | | Mixed Logit | | |
|---|---|---|---|---|---|---|---|---|
| | | mean | (95% C.I.) | mean | (95% C.I.) | mean | (95% C.I.) | Actual |
| Mattapan | Chittick | 0.01 | (0.00,0.03) | 0.05 | (0.03,0.07) | 0.05 | (0.03,0.07) | 0.04 |
| Mattapan | Clap | | | 0.02 | (0.01,0.03) | 0.02 | (0.01,0.03) | 0.02 |
| Mattapan | Condon | | | 0.02 | (0.01,0.03) | 0.01 | (0.00,0.02) | 0.01 |
| Mattapan | Conley | 0.01 | (0.00,0.01) | | | | | |
| Mattapan | Curley | 0.01 | (0.01,0.02) | 0.01 | (0.00,0.02) | 0.01 | (0.00,0.02) | |
| Mattapan | Dever | 0.02 | (0.01,0.04) | 0.02 | (0.01,0.04) | 0.02 | (0.01,0.04) | 0.03 |
| Mattapan | Ellis | 0.01 | (0.00,0.02) | | | | | |
| Mattapan | Ellison/Parks | 0.07 | (0.06,0.09) | 0.11 | (0.09,0.14) | 0.12 | (0.10,0.14) | 0.16 |
| Mattapan | Everett | | | 0.02 | (0.01,0.03) | 0.01 | (0.01,0.03) | |
| Mattapan | Hale | 0.01 | (0.00,0.01) | | | | | |
| Mattapan | Haley | | | 0.03 | (0.02,0.05) | 0.03 | (0.02,0.04) | 0.04 |
| Mattapan | Haynes | 0.01 | (0.00,0.02) | 0.01 | (0.00,0.01) | 0.01 | (0.00,0.02) | 0.01 |
| Mattapan | Henderson | 0.23 | (0.21,0.25) | 0.02 | (0.01,0.03) | 0.03 | (0.01,0.04) | 0.01 |
| Mattapan | Hernandez | 0.01 | (0.00,0.02) | 0.04 | (0.03,0.06) | 0.04 | (0.02,0.06) | 0.06 |
| Mattapan | Holland | | | 0.01 | (0.01,0.03) | 0.01 | (0.01,0.02) | 0.02 |
| Mattapan | Holmes | | | 0.02 | (0.01,0.03) | 0.01 | (0.01,0.03) | |
| Mattapan | Kenny | | | 0.02 | (0.01,0.03) | 0.02 | (0.01,0.03) | 0.01 |
| Mattapan | Lee | 0.02 | (0.01,0.04) | 0.09 | (0.06,0.12) | 0.09 | (0.07,0.12) | 0.09 |
| Mattapan | Mather | 0.01 | (0.00,0.01) | 0.02 | (0.01,0.03) | 0.01 | (0.01,0.02) | 0.02 |
| Mattapan | Mattahunt | 0.03 | (0.01,0.05) | 0.04 | (0.03,0.07) | 0.04 | (0.02,0.06) | 0.04 |
| Mattapan | Murphy | 0.30 | (0.26,0.34) | 0.07 | (0.05,0.09) | 0.08 | (0.06,0.10) | 0.07 |
| Mattapan | Perry | | | 0.01 | (0.00,0.02) | 0.01 | (0.01,0.02) | 0.01 |
| Mattapan | Philbrick | 0.04 | (0.02,0.05) | 0.00 | (0.00,0.01) | | | |
| Mattapan | Roosevelt | 0.02 | (0.01,0.04) | 0.04 | (0.02,0.05) | 0.04 | (0.02,0.05) | 0.05 |
| Mattapan | Russell | 0.03 | (0.01,0.04) | 0.02 | (0.01,0.03) | 0.02 | (0.01,0.03) | 0.01 |
| Mattapan | S. Greenwood | 0.05 | (0.04,0.07) | 0.05 | (0.03,0.06) | 0.05 | (0.03,0.06) | 0.03 |
| Mattapan | Sumner | 0.04 | (0.03,0.06) | 0.01 | (0.00,0.01) | 0.01 | (0.00,0.01) | |
| Mattapan | Taylor | 0.03 | (0.01,0.04) | 0.04 | (0.02,0.06) | 0.04 | (0.02,0.05) | 0.04 |
| Mattapan | Tynan | | | 0.01 | (0.00,0.01) | 0.00 | (0.00,0.01) | |
| Mattapan | Young Achievers | 0.01 | (0.00,0.02) | 0.15 | (0.12,0.18) | 0.16 | (0.14,0.19) | 0.12 |
| North Dorchester | Blackstone | | | 0.01 | (0.00,0.02) | 0.01 | (0.00,0.02) | |
| North Dorchester | Channing | | | | | 0.01 | (0.00,0.01) | |
| North Dorchester | Chittick | | | 0.01 | (0.00,0.01) | 0.01 | (0.00,0.01) | |
| North Dorchester | Clap | 0.02 | (0.00,0.03) | 0.11 | (0.08,0.14) | 0.11 | (0.08,0.14) | 0.10 |
| North Dorchester | Condon | | | 0.04 | (0.02,0.06) | 0.03 | (0.01,0.04) | 0.05 |
| North Dorchester | Dever | 0.03 | (0.01,0.04) | 0.06 | (0.04,0.09) | 0.06 | (0.04,0.09) | 0.06 |
| North Dorchester | East Boston EEC | | | | | 0.00 | (0.00,0.01) | |
| North Dorchester | Edison | 0.02 | (0.01,0.04) | | | 0.00 | (0.00,0.01) | |
| North Dorchester | Eliot | | | 0.01 | (0.00,0.01) | 0.01 | (0.00,0.01) | |
| North Dorchester | Ellison/Parks | 0.12 | (0.09,0.15) | 0.02 | (0.01,0.04) | 0.03 | (0.02,0.05) | 0.03 |
| North Dorchester | Everett | 0.02 | (0.01,0.03) | 0.08 | (0.06,0.10) | 0.08 | (0.06,0.11) | 0.13 |
| North Dorchester | Gardner | | | 0.00 | (0.00,0.01) | | | |
| North Dorchester | Haynes | 0.10 | (0.07,0.12) | 0.06 | (0.03,0.08) | 0.06 | (0.04,0.08) | 0.03 |
| North Dorchester | Henderson | 0.13 | (0.10,0.15) | 0.03 | (0.02,0.04) | 0.03 | (0.01,0.04) | 0.01 |
| North Dorchester | Hernandez | | | 0.03 | (0.01,0.04) | 0.02 | (0.01,0.04) | 0.02 |
| North Dorchester | Holland | 0.04 | (0.02,0.06) | 0.03 | (0.02,0.05) | 0.03 | (0.02,0.05) | 0.03 |
| North Dorchester | Holmes | | | 0.01 | (0.00,0.02) | 0.01 | (0.00,0.02) | |
| North Dorchester | Hurley | 0.02 | (0.01,0.04) | 0.01 | (0.00,0.02) | 0.01 | (0.00,0.01) | |
| North Dorchester | Kenny | | | 0.01 | (0.00,0.02) | 0.01 | (0.00,0.02) | |
| North Dorchester | King | | | 0.01 | (0.00,0.02) | 0.01 | (0.00,0.02) | |
| North Dorchester | Lee | 0.01 | (0.00,0.02) | 0.03 | (0.01,0.04) | 0.03 | (0.01,0.04) | 0.03 |
| North Dorchester | Mason | 0.14 | (0.11,0.16) | 0.02 | (0.01,0.04) | 0.02 | (0.01,0.04) | 0.03 |
| North Dorchester | Mather | 0.05 | (0.03,0.07) | 0.07 | (0.05,0.10) | 0.08 | (0.05,0.10) | 0.08 |
| North Dorchester | Mattahunt | 0.01 | (0.00,0.02) | 0.01 | (0.00,0.01) | 0.00 | (0.00,0.01) | |
| North Dorchester | Murphy | 0.17 | (0.13,0.22) | 0.11 | (0.08,0.14) | 0.13 | (0.09,0.16) | 0.16 |

Continued on next page

**Table 6 – continued from previous page**

| Neighborhood | School | Naive mean | Naive (95% C.I.) | Logit mean | Logit (95% C.I.) | Mixed Logit mean | Mixed Logit (95% C.I.) | Actual |
|---|---|---|---|---|---|---|---|---|
| North Dorchester | Orchard Gardens | 0.01 | (0.00,0.02) | 0.01 | (0.00,0.02) | 0.01 | (0.00,0.02) | |
| North Dorchester | Otis | 0.02 | (0.01,0.04) | | | | | |
| North Dorchester | Perry | | | 0.04 | (0.02,0.06) | 0.04 | (0.02,0.06) | 0.02 |
| North Dorchester | Quincy | 0.02 | (0.01,0.04) | 0.01 | (0.00,0.02) | 0.01 | (0.00,0.02) | |
| North Dorchester | Roosevelt | 0.01 | (0.00,0.01) | 0.01 | (0.00,0.02) | 0.01 | (0.00,0.03) | 0.01 |
| North Dorchester | Russell | 0.04 | (0.02,0.06) | 0.07 | (0.05,0.10) | 0.07 | (0.05,0.10) | 0.09 |
| North Dorchester | S. Greenwood | 0.02 | (0.01,0.03) | 0.01 | (0.00,0.02) | 0.01 | (0.00,0.02) | 0.01 |
| North Dorchester | Taylor | | | 0.01 | (0.00,0.01) | 0.00 | (0.00,0.01) | |
| North Dorchester | Tynan | | | 0.02 | (0.01,0.03) | 0.01 | (0.01,0.03) | 0.01 |
| North Dorchester | Winthrop | | | 0.01 | (0.00,0.03) | 0.01 | (0.00,0.02) | |
| North Dorchester | Young Achievers | | | 0.02 | (0.01,0.03) | 0.02 | (0.01,0.03) | 0.02 |
| Roslindale | BTU | 0.01 | (0.00,0.01) | 0.10 | (0.08,0.12) | 0.11 | (0.09,0.12) | 0.11 |
| Roslindale | Bates | 0.01 | (0.00,0.02) | 0.07 | (0.05,0.09) | 0.07 | (0.06,0.09) | 0.06 |
| Roslindale | Beethoven | 0.01 | (0.01,0.02) | 0.09 | (0.07,0.11) | 0.09 | (0.07,0.10) | 0.10 |
| Roslindale | Bradley | 0.00 | (0.00,0.01) | | | | | |
| Roslindale | Chittick | | | 0.01 | (0.00,0.01) | | | |
| Roslindale | Conley | 0.19 | (0.17,0.20) | 0.06 | (0.04,0.07) | 0.05 | (0.04,0.07) | 0.04 |
| Roslindale | Curley | 0.04 | (0.03,0.06) | 0.06 | (0.04,0.08) | 0.06 | (0.04,0.07) | 0.04 |
| Roslindale | Ellis | 0.01 | (0.00,0.02) | 0.01 | (0.00,0.02) | 0.01 | (0.00,0.02) | |
| Roslindale | Hale | 0.01 | (0.00,0.02) | 0.00 | (0.00,0.01) | | | |
| Roslindale | Haley | 0.02 | (0.01,0.03) | 0.06 | (0.04,0.07) | 0.06 | (0.04,0.07) | 0.09 |
| Roslindale | Haynes | 0.07 | (0.06,0.09) | 0.01 | (0.01,0.02) | 0.02 | (0.01,0.03) | 0.02 |
| Roslindale | Henderson | 0.01 | (0.00,0.01) | | | | | |
| Roslindale | Hernandez | 0.03 | (0.02,0.04) | 0.03 | (0.02,0.04) | 0.03 | (0.02,0.04) | 0.05 |
| Roslindale | J.F. Kennedy | | | 0.01 | (0.00,0.02) | 0.01 | (0.00,0.01) | 0.02 |
| Roslindale | Kilmer | 0.01 | (0.00,0.01) | 0.08 | (0.07,0.10) | 0.10 | (0.08,0.12) | 0.08 |
| Roslindale | Lyndon | 0.05 | (0.04,0.06) | 0.09 | (0.07,0.11) | 0.08 | (0.06,0.10) | 0.09 |
| Roslindale | Manning | 0.04 | (0.03,0.05) | 0.04 | (0.03,0.06) | 0.04 | (0.03,0.06) | 0.02 |
| Roslindale | Mattahunt | | | 0.01 | (0.00,0.01) | 0.01 | (0.00,0.01) | |
| Roslindale | Mendell | | | 0.01 | (0.00,0.02) | 0.01 | (0.00,0.01) | 0.01 |
| Roslindale | Mission Hill | | | 0.04 | (0.02,0.05) | 0.03 | (0.02,0.04) | 0.04 |
| Roslindale | Mozart | | | 0.08 | (0.06,0.09) | 0.08 | (0.06,0.09) | 0.07 |
| Roslindale | Philbrick | 0.18 | (0.16,0.20) | 0.05 | (0.03,0.07) | 0.04 | (0.03,0.06) | 0.06 |
| Roslindale | Roosevelt | 0.01 | (0.00,0.02) | 0.01 | (0.00,0.01) | 0.01 | (0.00,0.01) | |
| Roslindale | Sumner | 0.29 | (0.27,0.30) | 0.06 | (0.04,0.08) | 0.07 | (0.05,0.08) | 0.06 |
| Roslindale | West Zone ELC | | | 0.01 | (0.00,0.02) | 0.02 | (0.01,0.02) | 0.01 |
| Roslindale | Young Achievers | | | 0.01 | (0.00,0.01) | 0.01 | (0.00,0.01) | |
| Roxbury | BTU | | | 0.04 | (0.03,0.05) | 0.04 | (0.02,0.05) | 0.03 |
| Roxbury | Baldwin | | | 0.01 | (0.00,0.01) | 0.01 | (0.00,0.01) | 0.01 |
| Roxbury | Bates | | | 0.01 | (0.00,0.01) | 0.01 | (0.00,0.01) | 0.01 |
| Roxbury | Beethoven | | | 0.02 | (0.01,0.03) | 0.02 | (0.01,0.03) | 0.02 |
| Roxbury | Blackstone | 0.02 | (0.01,0.03) | 0.02 | (0.01,0.04) | 0.02 | (0.01,0.03) | 0.02 |
| Roxbury | Clap | | | 0.02 | (0.01,0.03) | 0.02 | (0.01,0.03) | |
| Roxbury | Conley | | | 0.01 | (0.00,0.01) | 0.01 | (0.00,0.01) | |
| Roxbury | Curley | 0.04 | (0.03,0.06) | 0.09 | (0.07,0.11) | 0.09 | (0.07,0.11) | 0.05 |
| Roxbury | Dever | 0.01 | (0.00,0.01) | 0.01 | (0.00,0.01) | 0.01 | (0.00,0.01) | |
| Roxbury | East Boston EEC | | | | | 0.01 | (0.00,0.01) | |
| Roxbury | Edison | 0.02 | (0.01,0.03) | | | | | |
| Roxbury | Eliot | 0.00 | (0.00,0.01) | 0.01 | (0.01,0.02) | 0.01 | (0.00,0.01) | |
| Roxbury | Ellis | 0.03 | (0.01,0.04) | 0.05 | (0.03,0.06) | 0.05 | (0.03,0.06) | 0.03 |
| Roxbury | Ellison/Parks | | | 0.01 | (0.00,0.01) | 0.01 | (0.00,0.01) | 0.01 |
| Roxbury | Everett | | | 0.02 | (0.01,0.03) | 0.02 | (0.01,0.03) | 0.01 |
| Roxbury | Hale | 0.18 | (0.17,0.20) | 0.03 | (0.01,0.04) | 0.02 | (0.01,0.04) | 0.02 |
| Roxbury | Haley | | | 0.02 | (0.01,0.02) | 0.01 | (0.01,0.02) | 0.01 |
| Roxbury | Haynes | 0.07 | (0.06,0.09) | 0.07 | (0.05,0.09) | 0.08 | (0.06,0.10) | 0.10 |

Continued on next page

**Table 6 – continued from previous page**

| Neighborhood | School | Naive mean | Naive (95% C.I.) | Logit mean | Logit (95% C.I.) | Mixed Logit mean | Mixed Logit (95% C.I.) | Actual |
|---|---|---|---|---|---|---|---|---|
| Roxbury | Henderson | 0.04 | (0.03,0.05) | | | | | |
| Roxbury | Hernandez | 0.02 | (0.01,0.03) | 0.07 | (0.05,0.08) | 0.07 | (0.06,0.09) | 0.07 |
| Roxbury | Higginson/Lewis | | | 0.02 | (0.01,0.03) | 0.02 | (0.01,0.03) | 0.03 |
| Roxbury | Holland | | | 0.02 | (0.01,0.03) | 0.02 | (0.01,0.03) | 0.02 |
| Roxbury | Holmes | | | 0.01 | (0.00,0.01) | 0.01 | (0.00,0.02) | |
| Roxbury | Hurley | 0.04 | (0.03,0.06) | 0.02 | (0.01,0.03) | 0.02 | (0.01,0.03) | 0.01 |
| Roxbury | J.F. Kennedy | 0.01 | (0.00,0.01) | 0.02 | (0.01,0.04) | 0.02 | (0.01,0.03) | 0.03 |
| Roxbury | Jackson/Mann | 0.00 | (0.00,0.01) | | | | | |
| Roxbury | Kilmer | | | 0.01 | (0.00,0.02) | 0.01 | (0.01,0.02) | 0.01 |
| Roxbury | King | | | 0.02 | (0.01,0.02) | 0.02 | (0.01,0.02) | 0.02 |
| Roxbury | Lee | 0.01 | (0.00,0.01) | 0.02 | (0.01,0.04) | 0.03 | (0.02,0.04) | 0.02 |
| Roxbury | Lyndon | | | 0.02 | (0.01,0.03) | 0.01 | (0.01,0.02) | 0.02 |
| Roxbury | Manning | 0.10 | (0.08,0.11) | 0.01 | (0.01,0.02) | 0.01 | (0.01,0.02) | |
| Roxbury | Mason | 0.09 | (0.07,0.10) | 0.02 | (0.01,0.03) | 0.02 | (0.01,0.03) | 0.03 |
| Roxbury | Mather | | | 0.01 | (0.01,0.02) | 0.01 | (0.01,0.02) | |
| Roxbury | Mattahunt | 0.00 | (0.00,0.01) | | | | | |
| Roxbury | Mendell | | | 0.03 | (0.01,0.04) | 0.02 | (0.02,0.03) | 0.01 |
| Roxbury | Mission Hill | | | 0.03 | (0.02,0.04) | 0.03 | (0.02,0.04) | 0.05 |
| Roxbury | Mozart | | | 0.01 | (0.01,0.02) | 0.01 | (0.00,0.01) | |
| Roxbury | Murphy | 0.05 | (0.04,0.07) | 0.01 | (0.01,0.02) | 0.01 | (0.01,0.02) | 0.01 |
| Roxbury | Orchard Gardens | | | 0.02 | (0.01,0.04) | 0.02 | (0.01,0.03) | 0.05 |
| Roxbury | Otis | 0.02 | (0.01,0.03) | | | | | |
| Roxbury | Philbrick | 0.08 | (0.07,0.10) | 0.01 | (0.00,0.01) | 0.01 | (0.00,0.01) | |
| Roxbury | Quincy | 0.00 | (0.00,0.01) | 0.01 | (0.01,0.02) | 0.01 | (0.01,0.02) | 0.02 |
| Roxbury | Russell | 0.02 | (0.01,0.03) | 0.02 | (0.01,0.03) | 0.02 | (0.01,0.03) | |
| Roxbury | S. Greenwood | 0.02 | (0.01,0.02) | 0.02 | (0.01,0.03) | 0.02 | (0.01,0.03) | 0.02 |
| Roxbury | Sumner | 0.03 | (0.02,0.04) | 0.01 | (0.01,0.02) | 0.01 | (0.01,0.02) | |
| Roxbury | Taylor | 0.01 | (0.00,0.01) | | | | | |
| Roxbury | Tobin | | | 0.01 | (0.01,0.02) | 0.01 | (0.01,0.02) | 0.01 |
| Roxbury | Trotter | 0.01 | (0.01,0.02) | 0.02 | (0.01,0.03) | 0.02 | (0.01,0.03) | 0.04 |
| Roxbury | West Zone ELC | | | 0.03 | (0.02,0.04) | 0.04 | (0.03,0.05) | 0.03 |
| Roxbury | Winthrop | 0.01 | (0.00,0.01) | 0.02 | (0.01,0.03) | 0.01 | (0.01,0.02) | 0.03 |
| Roxbury | Young Achievers | | | 0.02 | (0.01,0.02) | 0.02 | (0.01,0.02) | 0.02 |
| South Boston | Blackstone | | | 0.03 | (0.01,0.06) | 0.03 | (0.01,0.06) | |
| South Boston | Channing | | | 0.00 | (0.00,0.01) | 0.01 | (0.00,0.02) | |
| South Boston | Chittick | | | 0.00 | (0.00,0.01) | 0.00 | (0.00,0.02) | |
| South Boston | Clap | | | 0.08 | (0.05,0.12) | 0.09 | (0.06,0.12) | 0.05 |
| South Boston | Condon | 0.06 | (0.02,0.10) | 0.15 | (0.11,0.21) | 0.14 | (0.10,0.19) | 0.22 |
| South Boston | Dever | 0.05 | (0.03,0.07) | 0.08 | (0.05,0.11) | 0.08 | (0.05,0.11) | 0.03 |
| South Boston | East Boston EEC | 0.00 | (0.00,0.01) | | | | | |
| South Boston | Edison | 0.00 | (0.00,0.01) | | | | | |
| South Boston | Eliot | 0.00 | (0.00,0.01) | 0.01 | (0.00,0.02) | 0.01 | (0.00,0.02) | 0.01 |
| South Boston | Ellison/Parks | 0.06 | (0.04,0.09) | 0.01 | (0.00,0.03) | 0.02 | (0.00,0.04) | 0.02 |
| South Boston | Everett | | | 0.03 | (0.01,0.06) | 0.03 | (0.01,0.05) | |
| South Boston | Harvard/Kent | 0.01 | (0.00,0.03) | 0.00 | (0.00,0.02) | 0.01 | (0.00,0.02) | 0.02 |
| South Boston | Henderson | 0.15 | (0.12,0.19) | 0.02 | (0.01,0.04) | 0.02 | (0.00,0.03) | |
| South Boston | Hernandez | | | 0.02 | (0.01,0.04) | 0.02 | (0.01,0.04) | 0.01 |
| South Boston | Holland | 0.01 | (0.00,0.02) | 0.01 | (0.00,0.02) | 0.01 | (0.00,0.02) | |
| South Boston | Holmes | 0.00 | (0.00,0.01) | 0.00 | (0.00,0.02) | 0.00 | (0.00,0.01) | |
| South Boston | Hurley | 0.01 | (0.00,0.02) | 0.00 | (0.00,0.01) | 0.00 | (0.00,0.01) | |
| South Boston | Kenny | | | 0.01 | (0.00,0.02) | 0.01 | (0.00,0.02) | |
| South Boston | Lee | 0.02 | (0.00,0.04) | 0.02 | (0.00,0.04) | 0.02 | (0.00,0.03) | 0.02 |
| South Boston | Mason | 0.06 | (0.03,0.08) | 0.01 | (0.00,0.03) | 0.01 | (0.00,0.03) | |
| South Boston | Mather | 0.01 | (0.00,0.02) | 0.02 | (0.00,0.04) | 0.02 | (0.00,0.04) | |
| South Boston | Mattahunt | 0.01 | (0.00,0.02) | 0.00 | (0.00,0.01) | 0.00 | (0.00,0.01) | |

Continued on next page

**Table 6 – continued from previous page**

| Neighborhood | School | Naive mean | Naive (95% C.I.) | Logit mean | Logit (95% C.I.) | Mixed Logit mean | Mixed Logit (95% C.I.) | Actual |
|---|---|---|---|---|---|---|---|---|
| South Boston | Murphy | 0.28 | (0.22,0.35) | 0.09 | (0.05,0.12) | 0.09 | (0.05,0.12) | 0.13 |
| South Boston | Otis | 0.00 | (0.00,0.01) | | | | | |
| South Boston | Perry | 0.02 | (0.01,0.04) | 0.15 | (0.12,0.18) | 0.15 | (0.11,0.18) | 0.18 |
| South Boston | Quincy | 0.14 | (0.08,0.19) | 0.06 | (0.03,0.10) | 0.06 | (0.03,0.10) | 0.05 |
| South Boston | Roosevelt | | | 0.01 | (0.00,0.02) | 0.01 | (0.00,0.03) | 0.01 |
| South Boston | Russell | 0.04 | (0.02,0.07) | 0.05 | (0.03,0.08) | 0.04 | (0.02,0.07) | |
| South Boston | S. Greenwood | 0.04 | (0.02,0.06) | 0.01 | (0.00,0.03) | 0.01 | (0.00,0.03) | |
| South Boston | Taylor | | | 0.00 | (0.00,0.01) | | | |
| South Boston | Tynan | 0.02 | (0.00,0.04) | 0.08 | (0.05,0.10) | 0.08 | (0.05,0.11) | 0.09 |
| South Boston | Young Achievers | | | 0.02 | (0.01,0.04) | 0.02 | (0.01,0.04) | 0.03 |
| South Dorchester | Channing | | | 0.01 | (0.00,0.01) | 0.01 | (0.00,0.01) | |
| South Dorchester | Chittick | | | 0.01 | (0.01,0.02) | 0.01 | (0.01,0.02) | |
| South Dorchester | Clap | | | 0.04 | (0.03,0.05) | 0.03 | (0.02,0.04) | 0.03 |
| South Dorchester | Condon | 0.01 | (0.00,0.01) | 0.03 | (0.02,0.04) | 0.02 | (0.01,0.03) | 0.03 |
| South Dorchester | Dever | 0.02 | (0.01,0.03) | 0.03 | (0.02,0.04) | 0.03 | (0.02,0.04) | 0.03 |
| South Dorchester | Ellison/Parks | 0.09 | (0.08,0.10) | 0.04 | (0.03,0.06) | 0.05 | (0.04,0.07) | 0.05 |
| South Dorchester | Everett | | | 0.04 | (0.03,0.05) | 0.04 | (0.03,0.05) | 0.03 |
| South Dorchester | Haynes | 0.03 | (0.02,0.04) | 0.02 | (0.01,0.03) | 0.02 | (0.01,0.03) | 0.01 |
| South Dorchester | Henderson | 0.24 | (0.22,0.25) | 0.07 | (0.06,0.08) | 0.07 | (0.06,0.09) | 0.09 |
| South Dorchester | Hernandez | | | 0.03 | (0.02,0.04) | 0.02 | (0.02,0.03) | 0.02 |
| South Dorchester | Holland | 0.06 | (0.04,0.07) | 0.05 | (0.04,0.06) | 0.05 | (0.04,0.06) | 0.04 |
| South Dorchester | Holmes | | | 0.02 | (0.01,0.03) | 0.02 | (0.01,0.03) | 0.02 |
| South Dorchester | Kenny | 0.01 | (0.00,0.02) | 0.04 | (0.02,0.05) | 0.04 | (0.03,0.05) | 0.05 |
| South Dorchester | King | | | 0.01 | (0.00,0.01) | 0.01 | (0.00,0.01) | |
| South Dorchester | Lee | 0.03 | (0.02,0.04) | 0.09 | (0.07,0.11) | 0.08 | (0.07,0.10) | 0.10 |
| South Dorchester | Mather | 0.06 | (0.04,0.07) | 0.06 | (0.05,0.08) | 0.07 | (0.05,0.08) | 0.06 |
| South Dorchester | Mattahunt | 0.01 | (0.00,0.01) | 0.01 | (0.01,0.02) | 0.01 | (0.00,0.01) | |
| South Dorchester | Murphy | 0.39 | (0.36,0.42) | 0.23 | (0.20,0.26) | 0.25 | (0.22,0.28) | 0.23 |
| South Dorchester | Perry | | | 0.02 | (0.02,0.03) | 0.02 | (0.01,0.03) | 0.02 |
| South Dorchester | Roosevelt | | | 0.02 | (0.01,0.03) | 0.02 | (0.01,0.03) | 0.01 |
| South Dorchester | Russell | 0.02 | (0.01,0.03) | 0.03 | (0.02,0.03) | 0.03 | (0.02,0.03) | 0.02 |
| South Dorchester | S. Greenwood | 0.02 | (0.01,0.03) | 0.03 | (0.02,0.04) | 0.03 | (0.02,0.04) | 0.02 |
| South Dorchester | Taylor | | | 0.02 | (0.01,0.02) | 0.02 | (0.01,0.02) | 0.01 |
| South Dorchester | Tynan | | | 0.01 | (0.00,0.02) | 0.01 | (0.00,0.01) | 0.01 |
| South Dorchester | Young Achievers | | | 0.04 | (0.03,0.06) | 0.05 | (0.04,0.06) | 0.05 |
| South End | Adams | 0.03 | (0.01,0.05) | | | 0.00 | (0.00,0.01) | |
| South End | Baldwin | 0.01 | (0.00,0.02) | 0.04 | (0.02,0.06) | 0.03 | (0.02,0.06) | 0.03 |
| South End | Blackstone | 0.05 | (0.03,0.08) | 0.14 | (0.11,0.18) | 0.14 | (0.11,0.19) | 0.11 |
| South End | Bradley | | | 0.01 | (0.00,0.01) | 0.01 | (0.00,0.02) | |
| South End | Channing | 0.00 | (0.00,0.01) | | | | | |
| South End | Condon | | | 0.02 | (0.01,0.04) | 0.02 | (0.00,0.03) | |
| South End | East Boston EEC | 0.03 | (0.02,0.05) | 0.01 | (0.00,0.03) | 0.02 | (0.01,0.04) | 0.01 |
| South End | Edison | 0.07 | (0.04,0.10) | 0.02 | (0.01,0.04) | 0.02 | (0.01,0.04) | |
| South End | Eliot | 0.03 | (0.01,0.05) | 0.10 | (0.07,0.14) | 0.10 | (0.07,0.14) | 0.13 |
| South End | Gardner | 0.01 | (0.00,0.02) | 0.02 | (0.01,0.04) | 0.02 | (0.01,0.03) | 0.02 |
| South End | Hale | 0.03 | (0.01,0.04) | 0.01 | (0.00,0.03) | 0.01 | (0.00,0.02) | 0.02 |
| South End | Harvard/Kent | 0.02 | (0.01,0.04) | 0.03 | (0.01,0.05) | 0.02 | (0.01,0.04) | 0.02 |
| South End | Hernandez | 0.01 | (0.00,0.03) | 0.04 | (0.02,0.06) | 0.04 | (0.02,0.06) | 0.03 |
| South End | Higginson/Lewis | | | 0.00 | (0.00,0.01) | 0.00 | (0.00,0.01) | |
| South End | Hurley | 0.23 | (0.20,0.26) | 0.12 | (0.09,0.15) | 0.13 | (0.10,0.16) | 0.20 |
| South End | Jackson/Mann | | | 0.02 | (0.01,0.03) | 0.01 | (0.00,0.02) | 0.01 |
| South End | Kennedy Patrick | | | 0.00 | (0.00,0.01) | 0.00 | (0.00,0.01) | |
| South End | Mason | 0.05 | (0.03,0.07) | 0.03 | (0.01,0.04) | 0.03 | (0.01,0.04) | 0.02 |
| South End | Mission Hill | 0.01 | (0.00,0.01) | 0.00 | (0.00,0.01) | 0.00 | (0.00,0.01) | 0.02 |
| South End | O'Donnell | | | 0.00 | (0.00,0.01) | 0.00 | (0.00,0.01) | |

Continued on next page

**Table 6 – continued from previous page**

| Neighborhood | School | Naive mean | Naive (95% C.I.) | Logit mean | Logit (95% C.I.) | Mixed Logit mean | Mixed Logit (95% C.I.) | Actual |
|---|---|---|---|---|---|---|---|---|
| South End | Orchard Gardens | 0.01 | (0.00,0.03) | 0.06 | (0.03,0.09) | 0.05 | (0.03,0.07) | 0.05 |
| South End | Otis | 0.07 | (0.04,0.10) | 0.01 | (0.00,0.02) | 0.01 | (0.00,0.02) | |
| South End | Quincy | 0.31 | (0.24,0.36) | 0.25 | (0.21,0.30) | 0.26 | (0.21,0.31) | 0.28 |
| South End | Tobin | 0.01 | (0.00,0.03) | 0.03 | (0.02,0.05) | 0.03 | (0.01,0.05) | |
| South End | Tynan | 0.00 | (0.00,0.01) | | | | | |
| South End | Winship | | | 0.01 | (0.00,0.03) | 0.01 | (0.00,0.02) | |
| South End | Winthrop | | | 0.01 | (0.00,0.02) | 0.01 | (0.00,0.01) | |
| West Roxbury | BTU | | | 0.04 | (0.03,0.05) | 0.04 | (0.02,0.05) | 0.02 |
| West Roxbury | Bates | 0.01 | (0.00,0.02) | 0.05 | (0.03,0.06) | 0.05 | (0.03,0.06) | 0.05 |
| West Roxbury | Beethoven | 0.02 | (0.01,0.03) | 0.17 | (0.15,0.20) | 0.18 | (0.16,0.20) | 0.20 |
| West Roxbury | Channing | | | 0.02 | (0.01,0.03) | 0.02 | (0.01,0.03) | 0.01 |
| West Roxbury | Conley | 0.09 | (0.07,0.11) | 0.02 | (0.01,0.04) | 0.02 | (0.01,0.03) | 0.02 |
| West Roxbury | Curley | 0.03 | (0.01,0.04) | 0.03 | (0.02,0.05) | 0.03 | (0.02,0.04) | 0.02 |
| West Roxbury | Ellis | | | | | 0.00 | (0.00,0.01) | |
| West Roxbury | Haley | | | 0.02 | (0.01,0.03) | 0.02 | (0.01,0.03) | 0.02 |
| West Roxbury | Harvard/Kent | 0.01 | (0.00,0.02) | | | | | |
| West Roxbury | Haynes | 0.07 | (0.05,0.08) | 0.01 | (0.00,0.01) | 0.01 | (0.01,0.02) | 0.02 |
| West Roxbury | Hernandez | 0.02 | (0.01,0.03) | 0.01 | (0.01,0.02) | 0.01 | (0.00,0.02) | 0.02 |
| West Roxbury | Holland | 0.00 | (0.00,0.01) | | | | | |
| West Roxbury | J.F. Kennedy | | | 0.00 | (0.00,0.01) | 0.01 | | |
| West Roxbury | Kilmer | 0.27 | (0.25,0.28) | 0.23 | (0.21,0.25) | 0.23 | (0.22,0.25) | 0.25 |
| West Roxbury | Lyndon | 0.28 | (0.27,0.29) | 0.20 | (0.17,0.22) | 0.20 | (0.18,0.22) | 0.23 |
| West Roxbury | Manning | 0.02 | (0.01,0.03) | 0.04 | (0.02,0.05) | 0.04 | (0.02,0.05) | 0.03 |
| West Roxbury | Mather | 0.00 | (0.00,0.01) | | | | | |
| West Roxbury | Mendell | | | 0.01 | (0.00,0.01) | | | |
| West Roxbury | Mission Hill | | | 0.02 | (0.01,0.03) | 0.01 | (0.01,0.02) | 0.02 |
| West Roxbury | Mozart | 0.01 | (0.00,0.01) | 0.07 | (0.05,0.09) | 0.07 | (0.05,0.09) | 0.05 |
| West Roxbury | Philbrick | | | 0.02 | (0.01,0.03) | 0.01 | (0.00,0.02) | 0.01 |
| West Roxbury | Sumner | 0.16 | (0.14,0.18) | 0.02 | (0.01,0.03) | 0.02 | (0.01,0.03) | 0.02 |
| West Roxbury | West Zone ELC | | | 0.01 | (0.00,0.01) | 0.01 | (0.00,0.02) | 0.01 |

## D.2 Predictions for 2014

This section forecasts market shares in 2014. We make these predictions using 2013 data, without looking at 2014 data.

### D.2.1 K2

Table 7: Top Choice Market Share Predictions for 2014 K2

| Neighborhood | School | Naive mean | Naive (95% C.I.) | Logit mean | Logit (95% C.I.) | Mixed Logit mean | Mixed Logit (95% C.I.) |
|---|---|---|---|---|---|---|---|
| Allston-Brighton | Baldwin | 0.15 | (0.12,0.19) | 0.22 | (0.16,0.27) | 0.21 | (0.16,0.27) |
| Allston-Brighton | Blackstone | | | 0.00 | (0.00,0.01) | | |
| Allston-Brighton | Curley | | | 0.00 | (0.00,0.02) | 0.00 | (0.00,0.02) |
| Allston-Brighton | Dudley | | | 0.00 | (0.00,0.01) | 0.01 | (0.00,0.02) |
| Allston-Brighton | Edison | 0.11 | (0.08,0.15) | 0.12 | (0.09,0.17) | 0.11 | (0.07,0.15) |
| Allston-Brighton | Gardner | 0.10 | (0.07,0.14) | 0.15 | (0.11,0.21) | 0.17 | (0.12,0.22) |
| Allston-Brighton | Hennigan | | | 0.00 | (0.00,0.02) | 0.00 | (0.00,0.02) |
| Allston-Brighton | Hernandez | | | 0.01 | (0.00,0.02) | 0.01 | (0.00,0.03) |
| Allston-Brighton | Hurley | | | 0.00 | (0.00,0.01) | | |

Continued on next page

**Table 7 – continued from previous page**

| | | Naive | | Logit | | Mixed Logit | |
|---|---|---|---|---|---|---|---|
| Neighborhood | School | mean | (95% C.I.) | mean | (95% C.I.) | mean | (95% C.I.) |
| Allston-Brighton | Jackson/Mann | 0.16 | (0.12,0.20) | 0.16 | (0.12,0.22) | 0.15 | (0.10,0.19) |
| Allston-Brighton | Kennedy Patrick | 0.01 | (0.00,0.02) | | | | |
| Allston-Brighton | Lyon K-8 | 0.29 | (0.21,0.37) | 0.10 | (0.06,0.15) | 0.13 | (0.07,0.18) |
| Allston-Brighton | Manning | 0.01 | (0.00,0.02) | 0.00 | (0.00,0.01) | 0.00 | (0.00,0.01) |
| Allston-Brighton | Mendell | | | 0.00 | (0.00,0.01) | 0.00 | (0.00,0.01) |
| Allston-Brighton | Quincy | 0.04 | (0.01,0.07) | 0.01 | (0.00,0.02) | 0.01 | (0.00,0.03) |
| Allston-Brighton | Tobin | | | 0.00 | (0.00,0.01) | 0.00 | (0.00,0.01) |
| Allston-Brighton | UP Acad. Dor. | | | | | 0.01 | (0.00,0.02) |
| Allston-Brighton | Warren/Prescott | 0.01 | (0.00,0.02) | | | | |
| Allston-Brighton | Winship | 0.11 | (0.08,0.14) | 0.19 | (0.13,0.24) | 0.18 | (0.13,0.23) |
| Charlestown | Baldwin | 0.01 | (0.00,0.02) | 0.01 | (0.00,0.01) | 0.00 | (0.00,0.01) |
| Charlestown | Blackstone | | | 0.01 | (0.00,0.03) | 0.01 | (0.00,0.03) |
| Charlestown | Dudley | | | 0.01 | (0.00,0.02) | 0.02 | (0.00,0.05) |
| Charlestown | East Boston EEC | | | 0.02 | (0.00,0.04) | 0.02 | (0.00,0.05) |
| Charlestown | Edison | 0.02 | (0.01,0.02) | 0.01 | (0.00,0.02) | 0.01 | (0.00,0.02) |
| Charlestown | Eliot | 0.05 | (0.03,0.07) | 0.27 | (0.20,0.34) | 0.25 | (0.19,0.32) |
| Charlestown | Harvard/Kent | 0.39 | (0.33,0.47) | 0.26 | (0.20,0.33) | 0.26 | (0.19,0.32) |
| Charlestown | Hernandez | | | 0.00 | (0.00,0.01) | 0.00 | (0.00,0.02) |
| Charlestown | Hurley | 0.01 | (0.00,0.03) | 0.01 | (0.00,0.02) | 0.01 | (0.00,0.02) |
| Charlestown | Mario Umana | 0.02 | (0.00,0.04) | 0.01 | (0.00,0.04) | 0.01 | (0.00,0.03) |
| Charlestown | O'Donnell | | | 0.02 | (0.00,0.04) | 0.01 | (0.00,0.03) |
| Charlestown | Orchard Gardens | 0.01 | (0.00,0.03) | 0.00 | (0.00,0.01) | 0.00 | (0.00,0.01) |
| Charlestown | Otis | 0.01 | (0.00,0.03) | 0.01 | (0.00,0.02) | 0.01 | (0.00,0.02) |
| Charlestown | Perkins | | | 0.00 | (0.00,0.02) | 0.00 | (0.00,0.02) |
| Charlestown | Quincy | | | 0.04 | (0.01,0.07) | 0.03 | (0.01,0.06) |
| Charlestown | Tynan | | | 0.01 | (0.00,0.02) | 0.01 | (0.00,0.02) |
| Charlestown | UP Acad. Dor. | | | 0.00 | (0.00,0.01) | 0.01 | (0.00,0.02) |
| Charlestown | Warren/Prescott | 0.45 | (0.37,0.53) | 0.30 | (0.22,0.38) | 0.31 | (0.23,0.39) |
| Downtown | Baldwin | | | 0.01 | (0.00,0.01) | 0.00 | (0.00,0.01) |
| Downtown | Blackstone | | | 0.02 | (0.00,0.05) | 0.02 | (0.00,0.04) |
| Downtown | Condon | | | 0.01 | (0.00,0.03) | 0.01 | (0.00,0.03) |
| Downtown | Curley | | | 0.00 | (0.00,0.01) | 0.00 | (0.00,0.01) |
| Downtown | Dudley | | | 0.01 | (0.00,0.03) | 0.02 | (0.00,0.05) |
| Downtown | East Boston EEC | | | 0.00 | (0.00,0.01) | 0.01 | (0.00,0.02) |
| Downtown | Edison | 0.01 | (0.00,0.03) | 0.00 | (0.00,0.02) | 0.00 | (0.00,0.02) |
| Downtown | Eliot | 0.27 | (0.20,0.33) | 0.31 | (0.24,0.37) | 0.31 | (0.24,0.38) |
| Downtown | Hale | 0.02 | (0.00,0.05) | 0.00 | (0.00,0.01) | 0.00 | (0.00,0.01) |
| Downtown | Harvard/Kent | 0.06 | (0.04,0.09) | 0.07 | (0.04,0.10) | 0.06 | (0.04,0.09) |
| Downtown | Hennigan | 0.01 | (0.00,0.03) | 0.01 | (0.00,0.03) | 0.01 | (0.00,0.03) |
| Downtown | Hernandez | | | 0.01 | (0.00,0.03) | 0.01 | (0.00,0.03) |
| Downtown | Higginson/Lewis | | | 0.00 | (0.00,0.01) | | |
| Downtown | Hurley | 0.09 | (0.05,0.14) | 0.06 | (0.03,0.10) | 0.05 | (0.02,0.08) |
| Downtown | J.F. Kennedy | | | 0.00 | (0.00,0.01) | 0.00 | (0.00,0.01) |
| Downtown | Jackson/Mann | 0.04 | (0.02,0.08) | 0.03 | (0.01,0.05) | 0.02 | (0.01,0.05) |
| Downtown | Mason | | | 0.01 | (0.00,0.03) | 0.01 | (0.00,0.03) |
| Downtown | Orchard Gardens | 0.02 | (0.01,0.04) | 0.04 | (0.02,0.07) | 0.04 | (0.01,0.06) |
| Downtown | Perkins | | | 0.00 | (0.00,0.02) | 0.00 | (0.00,0.02) |
| Downtown | Quincy | 0.43 | (0.35,0.50) | 0.33 | (0.25,0.40) | 0.34 | (0.27,0.42) |
| Downtown | Tobin | 0.01 | (0.00,0.02) | 0.01 | (0.00,0.03) | 0.01 | (0.00,0.03) |
| Downtown | Tynan | | | 0.01 | (0.00,0.02) | 0.01 | (0.00,0.02) |
| Downtown | UP Acad. Dor. | | | 0.00 | (0.00,0.01) | 0.01 | (0.00,0.02) |
| Downtown | Warren/Prescott | 0.01 | (0.00,0.03) | 0.03 | (0.01,0.06) | 0.03 | (0.00,0.05) |
| Downtown | West Zone ELC | | | 0.01 | (0.00,0.03) | 0.01 | (0.00,0.03) |
| Downtown | Winship | | | 0.01 | (0.00,0.02) | 0.00 | (0.00,0.02) |
| Downtown | Winthrop | 0.01 | (0.00,0.01) | 0.01 | (0.00,0.01) | 0.00 | (0.00,0.01) |

Continued on next page

**Table 7 – continued from previous page**

| | | Naive | | Logit | | Mixed Logit | |
|---|---|---|---|---|---|---|---|
| Neighborhood | School | mean | (95% C.I.) | mean | (95% C.I.) | mean | (95% C.I.) |
| East Boston | Adams | 0.05 | (0.04,0.07) | 0.07 | (0.05,0.09) | 0.06 | (0.04,0.08) |
| East Boston | Blackstone | 0.03 | (0.02,0.04) | 0.01 | (0.00,0.02) | 0.01 | (0.00,0.02) |
| East Boston | Bradley | 0.10 | (0.08,0.12) | 0.08 | (0.06,0.10) | 0.09 | (0.07,0.12) |
| East Boston | Dudley | | | | | 0.01 | (0.00,0.02) |
| East Boston | East Boston EEC | 0.04 | (0.03,0.05) | 0.12 | (0.10,0.15) | 0.12 | (0.10,0.15) |
| East Boston | Eliot | 0.00 | (0.00,0.01) | 0.01 | (0.00,0.01) | 0.01 | (0.00,0.01) |
| East Boston | Gardner | 0.00 | (0.00,0.01) | | | | |
| East Boston | Guild | 0.04 | (0.02,0.06) | 0.06 | (0.04,0.08) | 0.05 | (0.03,0.07) |
| East Boston | Harvard/Kent | 0.01 | (0.00,0.02) | 0.01 | (0.00,0.01) | 0.01 | (0.00,0.01) |
| East Boston | Hernandez | 0.01 | (0.00,0.01) | | | 0.01 | (0.00,0.02) |
| East Boston | Hurley | 0.01 | (0.00,0.01) | | | | |
| East Boston | Kennedy Patrick | 0.18 | (0.15,0.22) | 0.17 | (0.14,0.21) | 0.18 | (0.14,0.21) |
| East Boston | Mario Umana | 0.10 | (0.08,0.13) | 0.10 | (0.07,0.13) | 0.10 | (0.07,0.13) |
| East Boston | McKay | 0.04 | (0.02,0.06) | 0.13 | (0.10,0.17) | 0.12 | (0.09,0.16) |
| East Boston | O'Donnell | 0.05 | (0.04,0.06) | 0.15 | (0.12,0.18) | 0.13 | (0.10,0.16) |
| East Boston | Orchard Gardens | 0.01 | (0.01,0.01) | | | | |
| East Boston | Otis | 0.29 | (0.24,0.32) | 0.08 | (0.06,0.10) | 0.07 | (0.05,0.09) |
| East Boston | Tobin | 0.01 | (0.00,0.01) | | | | |
| East Boston | UP Acad. Dor. | | | | | 0.01 | (0.00,0.02) |
| East Boston | Winthrop | 0.02 | (0.01,0.02) | | | | |
| Hyde Park | Bates | | | 0.03 | (0.01,0.06) | 0.03 | (0.01,0.05) |
| Hyde Park | Beethoven | 0.02 | (0.01,0.03) | 0.06 | (0.04,0.09) | 0.06 | (0.03,0.09) |
| Hyde Park | Channing | 0.05 | (0.04,0.07) | 0.08 | (0.05,0.11) | 0.07 | (0.04,0.10) |
| Hyde Park | Chittick | 0.08 | (0.05,0.10) | 0.07 | (0.05,0.10) | 0.07 | (0.04,0.10) |
| Hyde Park | Condon | 0.01 | (0.00,0.02) | | | | |
| Hyde Park | Conley | 0.16 | (0.11,0.20) | 0.04 | (0.02,0.07) | 0.04 | (0.01,0.07) |
| Hyde Park | Dudley | | | 0.01 | (0.00,0.02) | 0.02 | (0.01,0.04) |
| Hyde Park | E Greenwood | 0.03 | (0.01,0.05) | 0.08 | (0.04,0.12) | 0.08 | (0.05,0.12) |
| Hyde Park | Ellison/Parks | 0.01 | (0.01,0.02) | 0.05 | (0.02,0.07) | 0.04 | (0.02,0.07) |
| Hyde Park | Grew | 0.03 | (0.01,0.06) | 0.05 | (0.02,0.08) | 0.04 | (0.02,0.08) |
| Hyde Park | Haley | | | 0.03 | (0.01,0.05) | 0.03 | (0.01,0.05) |
| Hyde Park | Hernandez | 0.02 | (0.01,0.03) | 0.03 | (0.01,0.04) | 0.03 | (0.01,0.04) |
| Hyde Park | Kenny | 0.01 | (0.00,0.02) | | | | |
| Hyde Park | Kilmer | 0.01 | (0.01,0.02) | 0.03 | (0.01,0.05) | 0.03 | (0.01,0.05) |
| Hyde Park | Lee | | | | | 0.01 | (0.00,0.01) |
| Hyde Park | Lyndon | 0.01 | (0.00,0.01) | 0.01 | (0.00,0.01) | 0.01 | (0.00,0.01) |
| Hyde Park | Manning | 0.01 | (0.00,0.01) | | | | |
| Hyde Park | Mather | 0.01 | (0.00,0.03) | | | | |
| Hyde Park | Mattahunt | 0.06 | (0.04,0.08) | 0.04 | (0.02,0.06) | 0.04 | (0.02,0.06) |
| Hyde Park | Mission Hill | 0.00 | (0.00,0.01) | | | | |
| Hyde Park | Mozart | | | 0.02 | (0.01,0.05) | 0.02 | (0.01,0.04) |
| Hyde Park | Philbrick | 0.04 | (0.02,0.07) | 0.03 | (0.01,0.05) | 0.02 | (0.01,0.04) |
| Hyde Park | Roosevelt | 0.29 | (0.25,0.34) | 0.23 | (0.19,0.28) | 0.25 | (0.20,0.30) |
| Hyde Park | S. Greenwood | 0.02 | (0.01,0.03) | 0.01 | (0.00,0.02) | 0.01 | (0.00,0.02) |
| Hyde Park | Sumner | 0.02 | (0.01,0.02) | 0.03 | (0.01,0.05) | 0.03 | (0.01,0.04) |
| Hyde Park | Taylor | 0.02 | (0.01,0.03) | 0.01 | (0.00,0.03) | 0.01 | (0.00,0.02) |
| Hyde Park | UP Acad. Dor. | 0.01 | (0.00,0.01) | 0.01 | (0.00,0.02) | 0.02 | (0.00,0.03) |
| Hyde Park | Young Achievers | 0.03 | (0.02,0.05) | 0.02 | (0.01,0.03) | 0.02 | (0.01,0.03) |
| Jamaica Plain | BTU | 0.02 | (0.01,0.03) | 0.05 | (0.03,0.07) | 0.04 | (0.03,0.07) |
| Jamaica Plain | Bates | 0.01 | (0.00,0.02) | | | | |
| Jamaica Plain | Blackstone | 0.01 | (0.00,0.01) | 0.01 | (0.00,0.02) | 0.01 | (0.00,0.02) |
| Jamaica Plain | Curley | 0.12 | (0.09,0.14) | 0.18 | (0.14,0.21) | 0.17 | (0.13,0.21) |
| Jamaica Plain | Dudley | | | 0.02 | (0.00,0.03) | 0.04 | (0.02,0.06) |
| Jamaica Plain | Edison | 0.02 | (0.01,0.04) | 0.01 | (0.00,0.02) | 0.01 | (0.00,0.02) |
| Jamaica Plain | Ellis | 0.04 | (0.02,0.06) | 0.03 | (0.01,0.05) | 0.03 | (0.01,0.04) |

Continued on next page

**Table 7 – continued from previous page**

| Neighborhood | School | Naive mean | Naive (95% C.I.) | Logit mean | Logit (95% C.I.) | Mixed Logit mean | Mixed Logit (95% C.I.) |
|---|---|---|---|---|---|---|---|
| Jamaica Plain | Hale | 0.24 | (0.19,0.29) | 0.02 | (0.01,0.04) | 0.02 | (0.00,0.04) |
| Jamaica Plain | Haley | 0.01 | (0.00,0.02) | 0.01 | (0.00,0.02) | 0.01 | (0.00,0.02) |
| Jamaica Plain | Hennigan | 0.04 | (0.01,0.06) | 0.07 | (0.04,0.10) | 0.07 | (0.04,0.10) |
| Jamaica Plain | Hernandez | 0.02 | (0.01,0.03) | 0.05 | (0.03,0.08) | 0.06 | (0.04,0.09) |
| Jamaica Plain | Higginson/Lewis | | | 0.00 | (0.00,0.01) | 0.00 | (0.00,0.01) |
| Jamaica Plain | Hurley | 0.05 | (0.02,0.08) | 0.02 | (0.00,0.04) | 0.02 | (0.00,0.04) |
| Jamaica Plain | J.F. Kennedy | 0.03 | (0.02,0.05) | 0.07 | (0.04,0.11) | 0.07 | (0.04,0.10) |
| Jamaica Plain | Jackson/Mann | | | 0.02 | (0.01,0.05) | 0.02 | (0.01,0.04) |
| Jamaica Plain | Lyndon | 0.01 | (0.00,0.02) | 0.01 | (0.00,0.02) | 0.01 | (0.00,0.02) |
| Jamaica Plain | Manning | 0.09 | (0.06,0.12) | 0.04 | (0.01,0.06) | 0.04 | (0.01,0.06) |
| Jamaica Plain | Mason | 0.00 | (0.00,0.01) | 0.01 | (0.00,0.02) | 0.01 | (0.00,0.02) |
| Jamaica Plain | Mather | 0.00 | (0.00,0.01) | | | | |
| Jamaica Plain | Mendell | 0.10 | (0.07,0.12) | 0.11 | (0.08,0.14) | 0.10 | (0.07,0.13) |
| Jamaica Plain | Mission Hill | 0.01 | (0.00,0.03) | 0.07 | (0.04,0.10) | 0.07 | (0.04,0.10) |
| Jamaica Plain | Orchard Gardens | | | 0.02 | (0.01,0.04) | 0.02 | (0.01,0.04) |
| Jamaica Plain | Philbrick | 0.00 | (0.00,0.01) | | | | |
| Jamaica Plain | Quincy | 0.02 | (0.00,0.03) | 0.01 | (0.00,0.03) | 0.01 | (0.00,0.03) |
| Jamaica Plain | Sumner | 0.02 | (0.00,0.03) | 0.01 | (0.00,0.02) | 0.01 | (0.00,0.02) |
| Jamaica Plain | Tobin | 0.00 | (0.00,0.02) | 0.03 | (0.01,0.06) | 0.03 | (0.01,0.06) |
| Jamaica Plain | Trotter | 0.03 | (0.02,0.04) | 0.02 | (0.01,0.04) | 0.02 | (0.01,0.04) |
| Jamaica Plain | UP Acad. Dor. | | | 0.01 | (0.00,0.03) | 0.02 | (0.00,0.03) |
| Jamaica Plain | Warren/Prescott | 0.00 | (0.00,0.02) | | | | |
| Jamaica Plain | West Zone ELC | 0.04 | (0.02,0.06) | 0.07 | (0.04,0.09) | 0.07 | (0.04,0.09) |
| Mattapan | BTU | | | 0.03 | (0.01,0.05) | 0.03 | (0.01,0.05) |
| Mattapan | Bates | 0.00 | (0.00,0.01) | | | | |
| Mattapan | Beethoven | 0.01 | (0.00,0.02) | 0.00 | (0.00,0.01) | 0.00 | (0.00,0.01) |
| Mattapan | Channing | 0.02 | (0.01,0.04) | 0.02 | (0.01,0.03) | 0.02 | (0.01,0.03) |
| Mattapan | Chittick | 0.02 | (0.01,0.04) | 0.03 | (0.01,0.04) | 0.02 | (0.01,0.04) |
| Mattapan | Condon | 0.01 | (0.00,0.02) | | | | |
| Mattapan | Conley | 0.00 | (0.00,0.02) | 0.01 | (0.00,0.02) | 0.01 | (0.00,0.02) |
| Mattapan | Curley | 0.00 | (0.00,0.02) | | | | |
| Mattapan | Dever | 0.04 | (0.03,0.06) | 0.03 | (0.02,0.04) | 0.03 | (0.02,0.04) |
| Mattapan | Dudley | 0.02 | (0.01,0.03) | 0.03 | (0.01,0.05) | 0.06 | (0.04,0.09) |
| Mattapan | E Greenwood | 0.02 | (0.00,0.04) | 0.02 | (0.00,0.03) | 0.02 | (0.00,0.04) |
| Mattapan | Edison | 0.00 | (0.00,0.01) | | | | |
| Mattapan | Ellison/Parks | 0.02 | (0.01,0.03) | 0.10 | (0.06,0.13) | 0.10 | (0.07,0.14) |
| Mattapan | Everett | 0.00 | (0.00,0.01) | | | | |
| Mattapan | Grew | 0.00 | (0.00,0.01) | | | | |
| Mattapan | Haley | 0.01 | (0.00,0.02) | 0.07 | (0.04,0.10) | 0.06 | (0.04,0.09) |
| Mattapan | Henderson | 0.23 | (0.18,0.28) | 0.02 | (0.00,0.03) | 0.02 | (0.00,0.04) |
| Mattapan | Hernandez | 0.02 | (0.01,0.03) | 0.05 | (0.03,0.08) | 0.04 | (0.03,0.07) |
| Mattapan | Holland | 0.03 | (0.02,0.05) | 0.02 | (0.01,0.04) | 0.02 | (0.01,0.04) |
| Mattapan | Holmes | 0.02 | (0.01,0.03) | 0.02 | (0.01,0.04) | 0.02 | (0.01,0.03) |
| Mattapan | Jackson/Mann | | | 0.01 | (0.00,0.02) | 0.01 | (0.00,0.02) |
| Mattapan | Kenny | 0.01 | (0.00,0.03) | 0.02 | (0.01,0.03) | 0.02 | (0.00,0.03) |
| Mattapan | Lee | 0.01 | (0.00,0.02) | 0.03 | (0.00,0.06) | 0.02 | (0.00,0.05) |
| Mattapan | Mather | 0.02 | (0.01,0.02) | 0.01 | (0.00,0.02) | 0.01 | (0.00,0.02) |
| Mattapan | Mattahunt | 0.05 | (0.03,0.07) | 0.05 | (0.03,0.07) | 0.04 | (0.02,0.06) |
| Mattapan | Murphy | 0.00 | (0.00,0.01) | 0.02 | (0.00,0.03) | 0.02 | (0.00,0.04) |
| Mattapan | Philbrick | 0.17 | (0.13,0.22) | 0.02 | (0.00,0.04) | 0.02 | (0.00,0.04) |
| Mattapan | Russell | 0.02 | (0.01,0.03) | 0.02 | (0.00,0.03) | 0.02 | (0.01,0.03) |
| Mattapan | S. Greenwood | 0.05 | (0.03,0.07) | 0.06 | (0.04,0.08) | 0.05 | (0.03,0.08) |
| Mattapan | Sumner | 0.01 | (0.00,0.02) | 0.01 | (0.00,0.02) | 0.01 | (0.00,0.02) |
| Mattapan | Taylor | 0.05 | (0.03,0.07) | 0.07 | (0.04,0.10) | 0.06 | (0.04,0.09) |
| Mattapan | UP Acad. Dor. | 0.03 | (0.01,0.03) | 0.05 | (0.03,0.07) | 0.06 | (0.04,0.09) |

Continued on next page

**Table 7 – continued from previous page**

| Neighborhood | School | Naive | | Logit | | Mixed Logit | |
|---|---|---|---|---|---|---|---|
| | | mean | (95% C.I.) | mean | (95% C.I.) | mean | (95% C.I.) |
| Mattapan | Young Achievers | 0.04 | (0.03,0.06) | 0.15 | (0.11,0.19) | 0.15 | (0.11,0.19) |
| North Dorchester | Blackstone | | | 0.01 | (0.00,0.01) | 0.00 | (0.00,0.01) |
| North Dorchester | Clap | 0.02 | (0.01,0.02) | 0.06 | (0.03,0.10) | 0.06 | (0.03,0.09) |
| North Dorchester | Condon | 0.11 | (0.08,0.16) | 0.05 | (0.03,0.08) | 0.05 | (0.03,0.08) |
| North Dorchester | Dever | 0.04 | (0.02,0.05) | 0.07 | (0.04,0.10) | 0.06 | (0.04,0.09) |
| North Dorchester | Dudley | 0.04 | (0.02,0.06) | 0.06 | (0.03,0.09) | 0.11 | (0.07,0.15) |
| North Dorchester | Edison | 0.01 | (0.00,0.03) | | | | |
| North Dorchester | Everett | | | 0.07 | (0.03,0.11) | 0.07 | (0.03,0.10) |
| North Dorchester | Hale | | | 0.00 | (0.00,0.01) | | |
| North Dorchester | Haynes | | | 0.03 | (0.01,0.06) | 0.03 | (0.01,0.05) |
| North Dorchester | Henderson | 0.06 | (0.03,0.10) | 0.02 | (0.00,0.04) | 0.02 | (0.00,0.04) |
| North Dorchester | Hernandez | | | 0.02 | (0.01,0.04) | 0.02 | (0.01,0.04) |
| North Dorchester | Holland | 0.03 | (0.02,0.05) | 0.05 | (0.03,0.07) | 0.04 | (0.02,0.06) |
| North Dorchester | Holmes | 0.01 | (0.00,0.03) | 0.00 | (0.00,0.01) | 0.00 | (0.00,0.01) |
| North Dorchester | Hurley | | | 0.00 | (0.00,0.02) | 0.00 | (0.00,0.01) |
| North Dorchester | Jackson/Mann | | | 0.01 | (0.00,0.02) | 0.01 | (0.00,0.03) |
| North Dorchester | King | 0.02 | (0.01,0.04) | 0.02 | (0.01,0.04) | 0.01 | (0.00,0.03) |
| North Dorchester | Lee | 0.00 | (0.00,0.01) | 0.00 | (0.00,0.01) | 0.00 | (0.00,0.01) |
| North Dorchester | Mason | 0.24 | (0.17,0.32) | 0.05 | (0.02,0.08) | 0.05 | (0.02,0.07) |
| North Dorchester | Mather | 0.07 | (0.05,0.10) | 0.10 | (0.06,0.13) | 0.09 | (0.06,0.12) |
| North Dorchester | Murphy | 0.05 | (0.02,0.07) | 0.04 | (0.02,0.06) | 0.04 | (0.02,0.06) |
| North Dorchester | Orchard Gardens | 0.05 | (0.03,0.07) | 0.05 | (0.03,0.08) | 0.05 | (0.03,0.08) |
| North Dorchester | Perkins | | | 0.01 | (0.00,0.03) | 0.01 | (0.00,0.02) |
| North Dorchester | Perry | | | 0.01 | (0.00,0.03) | 0.01 | (0.00,0.03) |
| North Dorchester | Russell | 0.10 | (0.07,0.13) | 0.12 | (0.09,0.16) | 0.12 | (0.08,0.15) |
| North Dorchester | S. Greenwood | 0.03 | (0.01,0.05) | 0.01 | (0.00,0.03) | 0.01 | (0.00,0.03) |
| North Dorchester | Sumner | 0.01 | (0.00,0.02) | | | | |
| North Dorchester | Taylor | 0.01 | (0.00,0.02) | | | | |
| North Dorchester | Trotter | 0.01 | (0.00,0.02) | 0.00 | (0.00,0.02) | 0.00 | (0.00,0.01) |
| North Dorchester | Tynan | 0.01 | (0.00,0.02) | 0.00 | (0.00,0.02) | 0.00 | (0.00,0.01) |
| North Dorchester | UP Acad. Dor. | 0.01 | (0.00,0.01) | 0.03 | (0.01,0.06) | 0.05 | (0.02,0.08) |
| North Dorchester | Winthrop | 0.04 | (0.02,0.05) | 0.05 | (0.03,0.08) | 0.05 | (0.02,0.07) |
| North Dorchester | Young Achievers | 0.01 | (0.00,0.01) | 0.01 | (0.00,0.01) | 0.01 | (0.00,0.01) |
| Roslindale | BTU | 0.03 | (0.02,0.03) | 0.11 | (0.08,0.14) | 0.11 | (0.08,0.14) |
| Roslindale | Bates | 0.01 | (0.00,0.02) | 0.07 | (0.04,0.10) | 0.07 | (0.04,0.10) |
| Roslindale | Beethoven | 0.05 | (0.03,0.07) | 0.05 | (0.04,0.07) | 0.05 | (0.03,0.07) |
| Roslindale | Channing | 0.01 | (0.00,0.01) | 0.01 | (0.00,0.01) | 0.01 | (0.00,0.01) |
| Roslindale | Chittick | | | 0.00 | (0.00,0.01) | 0.00 | (0.00,0.01) |
| Roslindale | Conley | 0.08 | (0.05,0.11) | 0.05 | (0.02,0.07) | 0.04 | (0.02,0.07) |
| Roslindale | Curley | 0.03 | (0.02,0.05) | 0.02 | (0.01,0.03) | 0.02 | (0.01,0.03) |
| Roslindale | Dudley | | | 0.01 | (0.00,0.02) | 0.02 | (0.01,0.04) |
| Roslindale | E Greenwood | 0.01 | (0.00,0.02) | 0.03 | (0.01,0.05) | 0.03 | (0.01,0.05) |
| Roslindale | Ellis | 0.02 | (0.01,0.02) | 0.01 | (0.00,0.02) | 0.01 | (0.00,0.02) |
| Roslindale | Ellison/Parks | | | 0.01 | (0.00,0.03) | 0.01 | (0.00,0.03) |
| Roslindale | Grew | | | 0.01 | (0.00,0.02) | 0.00 | (0.00,0.01) |
| Roslindale | Hale | 0.01 | (0.01,0.02) | 0.01 | (0.00,0.01) | 0.01 | (0.00,0.01) |
| Roslindale | Haley | 0.04 | (0.03,0.05) | 0.08 | (0.06,0.10) | 0.08 | (0.06,0.11) |
| Roslindale | Hennigan | 0.01 | (0.00,0.02) | 0.00 | (0.00,0.01) | 0.00 | (0.00,0.01) |
| Roslindale | Hernandez | 0.02 | (0.01,0.03) | 0.04 | (0.02,0.05) | 0.04 | (0.02,0.06) |
| Roslindale | Higginson/Lewis | 0.02 | (0.01,0.03) | 0.01 | (0.00,0.01) | 0.01 | (0.00,0.01) |
| Roslindale | J.F. Kennedy | 0.01 | (0.00,0.01) | 0.01 | (0.00,0.01) | 0.01 | (0.00,0.01) |
| Roslindale | Jackson/Mann | 0.01 | (0.00,0.02) | | | | |
| Roslindale | Kilmer | 0.02 | (0.01,0.03) | 0.03 | (0.02,0.04) | 0.03 | (0.02,0.04) |
| Roslindale | King | 0.01 | (0.00,0.02) | 0.00 | (0.00,0.01) | 0.00 | (0.00,0.01) |
| Roslindale | Lyndon | 0.06 | (0.04,0.08) | 0.07 | (0.05,0.10) | 0.07 | (0.05,0.09) |

Continued on next page

**Table 7 – continued from previous page**

| Neighborhood | School | Naive mean | Naive (95% C.I.) | Logit mean | Logit (95% C.I.) | Mixed Logit mean | Mixed Logit (95% C.I.) |
|---|---|---|---|---|---|---|---|
| Roslindale | Manning | 0.01 | (0.00,0.02) | 0.02 | (0.01,0.03) | 0.02 | (0.00,0.03) |
| Roslindale | Mattahunt | | | 0.01 | (0.00,0.03) | 0.01 | (0.00,0.03) |
| Roslindale | Mendell | 0.01 | (0.01,0.02) | 0.01 | (0.00,0.02) | 0.01 | (0.00,0.02) |
| Roslindale | Mission Hill | 0.00 | (0.00,0.01) | 0.01 | (0.00,0.03) | 0.01 | (0.00,0.03) |
| Roslindale | Mozart | 0.04 | (0.03,0.05) | 0.09 | (0.06,0.12) | 0.09 | (0.06,0.12) |
| Roslindale | Philbrick | 0.11 | (0.08,0.15) | 0.06 | (0.03,0.09) | 0.05 | (0.03,0.08) |
| Roslindale | Roosevelt | 0.01 | (0.00,0.02) | 0.00 | (0.00,0.01) | 0.00 | (0.00,0.01) |
| Roslindale | Sumner | 0.29 | (0.24,0.34) | 0.12 | (0.09,0.15) | 0.12 | (0.09,0.15) |
| Roslindale | Taylor | 0.01 | (0.00,0.01) | | | | |
| Roslindale | Trotter | 0.03 | (0.02,0.05) | 0.01 | (0.00,0.02) | 0.01 | (0.00,0.02) |
| Roslindale | UP Acad. Dor. | 0.00 | (0.00,0.01) | 0.01 | (0.00,0.02) | 0.01 | (0.00,0.03) |
| Roslindale | West Zone ELC | 0.01 | (0.00,0.02) | 0.01 | (0.00,0.01) | 0.01 | (0.00,0.01) |
| Roslindale | Young Achievers | 0.01 | (0.00,0.02) | 0.02 | (0.00,0.03) | 0.02 | (0.00,0.03) |
| Roxbury | BTU | 0.01 | (0.01,0.02) | 0.01 | (0.01,0.02) | 0.01 | (0.01,0.02) |
| Roxbury | Beethoven | 0.01 | (0.01,0.02) | 0.01 | (0.00,0.01) | | |
| Roxbury | Blackstone | | | 0.01 | (0.01,0.02) | 0.01 | (0.00,0.02) |
| Roxbury | Clap | | | 0.01 | (0.00,0.02) | 0.01 | (0.00,0.02) |
| Roxbury | Condon | 0.01 | (0.00,0.02) | | | | |
| Roxbury | Curley | 0.03 | (0.02,0.04) | 0.03 | (0.02,0.05) | 0.03 | (0.02,0.04) |
| Roxbury | Dudley | 0.02 | (0.01,0.03) | 0.05 | (0.03,0.07) | 0.11 | (0.08,0.13) |
| Roxbury | Ellis | 0.04 | (0.03,0.05) | 0.04 | (0.03,0.06) | 0.04 | (0.03,0.05) |
| Roxbury | Everett | | | 0.02 | (0.01,0.03) | 0.01 | (0.01,0.03) |
| Roxbury | Hale | 0.17 | (0.14,0.20) | 0.04 | (0.03,0.05) | 0.03 | (0.02,0.05) |
| Roxbury | Haley | 0.01 | (0.01,0.01) | 0.01 | (0.01,0.02) | 0.01 | (0.01,0.02) |
| Roxbury | Haynes | | | 0.04 | (0.03,0.06) | 0.04 | (0.02,0.05) |
| Roxbury | Henderson | 0.06 | (0.04,0.08) | 0.00 | (0.00,0.01) | 0.01 | (0.00,0.01) |
| Roxbury | Hennigan | 0.02 | (0.01,0.03) | 0.02 | (0.01,0.04) | 0.02 | (0.01,0.03) |
| Roxbury | Hernandez | 0.02 | (0.01,0.03) | 0.06 | (0.04,0.08) | 0.07 | (0.05,0.09) |
| Roxbury | Higginson/Lewis | 0.04 | (0.03,0.05) | 0.03 | (0.02,0.05) | 0.03 | (0.01,0.04) |
| Roxbury | Holland | 0.03 | (0.02,0.04) | 0.04 | (0.02,0.05) | 0.03 | (0.02,0.05) |
| Roxbury | Holmes | 0.01 | (0.01,0.02) | 0.01 | (0.01,0.02) | 0.01 | (0.01,0.02) |
| Roxbury | Hurley | 0.04 | (0.03,0.06) | 0.02 | (0.01,0.03) | 0.02 | (0.01,0.03) |
| Roxbury | J.F. Kennedy | 0.02 | (0.01,0.04) | 0.04 | (0.02,0.05) | 0.03 | (0.02,0.05) |
| Roxbury | Jackson/Mann | 0.01 | (0.00,0.02) | 0.02 | (0.01,0.03) | 0.02 | (0.01,0.03) |
| Roxbury | King | 0.02 | (0.01,0.03) | 0.02 | (0.01,0.04) | 0.02 | (0.01,0.03) |
| Roxbury | Lee | 0.00 | (0.00,0.01) | 0.01 | (0.00,0.01) | 0.01 | (0.00,0.01) |
| Roxbury | Lyndon | 0.01 | (0.00,0.01) | | | | |
| Roxbury | Mason | 0.12 | (0.09,0.15) | 0.05 | (0.03,0.07) | 0.04 | (0.03,0.06) |
| Roxbury | Mather | | | 0.02 | (0.01,0.03) | 0.01 | (0.01,0.03) |
| Roxbury | Mendell | 0.01 | (0.00,0.01) | 0.02 | (0.01,0.03) | 0.02 | (0.01,0.03) |
| Roxbury | Mission Hill | | | 0.01 | (0.01,0.03) | 0.01 | (0.00,0.02) |
| Roxbury | Murphy | | | | | 0.00 | (0.00,0.01) |
| Roxbury | Orchard Gardens | 0.06 | (0.04,0.07) | 0.08 | (0.06,0.10) | 0.07 | (0.05,0.09) |
| Roxbury | Perkins | 0.00 | (0.00,0.01) | | | | |
| Roxbury | Quincy | 0.00 | (0.00,0.01) | | | | |
| Roxbury | Russell | | | 0.02 | (0.01,0.03) | 0.02 | (0.01,0.03) |
| Roxbury | S. Greenwood | 0.02 | (0.01,0.02) | 0.03 | (0.02,0.04) | 0.03 | (0.01,0.04) |
| Roxbury | Sumner | 0.01 | (0.00,0.01) | | | | |
| Roxbury | Taylor | 0.01 | (0.00,0.01) | | | | |
| Roxbury | Tobin | | | 0.01 | (0.00,0.03) | 0.01 | (0.00,0.02) |
| Roxbury | Trotter | 0.04 | (0.03,0.05) | 0.06 | (0.04,0.08) | 0.05 | (0.04,0.07) |
| Roxbury | UP Acad. Dor. | 0.02 | (0.01,0.02) | 0.03 | (0.02,0.05) | 0.05 | (0.03,0.07) |
| Roxbury | West Zone ELC | 0.01 | (0.01,0.02) | 0.02 | (0.01,0.03) | 0.02 | (0.01,0.03) |
| Roxbury | Winthrop | 0.03 | (0.03,0.04) | 0.05 | (0.03,0.06) | 0.04 | (0.03,0.06) |
| Roxbury | Young Achievers | 0.01 | (0.00,0.02) | 0.01 | (0.00,0.01) | 0.01 | (0.00,0.01) |

Continued on next page

**Table 7 – continued from previous page**

| Neighborhood | School | Naive mean | Naive (95% C.I.) | Logit mean | Logit (95% C.I.) | Mixed Logit mean | Mixed Logit (95% C.I.) |
|---|---|---|---|---|---|---|---|
| South Boston | Blackstone | | | 0.03 | (0.01,0.06) | 0.02 | (0.00,0.05) |
| South Boston | Clap | 0.01 | (0.00,0.02) | 0.05 | (0.02,0.08) | 0.04 | (0.01,0.08) |
| South Boston | Condon | 0.20 | (0.15,0.26) | 0.20 | (0.14,0.26) | 0.19 | (0.14,0.25) |
| South Boston | Dever | 0.01 | (0.00,0.03) | 0.04 | (0.01,0.08) | 0.04 | (0.01,0.07) |
| South Boston | Dudley | 0.01 | (0.00,0.02) | 0.03 | (0.01,0.06) | 0.07 | (0.03,0.11) |
| South Boston | E Greenwood | 0.01 | (0.00,0.03) | | | | |
| South Boston | Eliot | 0.01 | (0.00,0.03) | 0.01 | (0.00,0.03) | 0.01 | (0.00,0.03) |
| South Boston | Everett | | | 0.01 | (0.00,0.04) | 0.01 | (0.00,0.03) |
| South Boston | Harvard/Kent | 0.02 | (0.01,0.03) | 0.02 | (0.00,0.03) | 0.02 | (0.00,0.03) |
| South Boston | Haynes | | | 0.01 | (0.00,0.03) | 0.01 | (0.00,0.03) |
| South Boston | Hernandez | | | 0.02 | (0.00,0.03) | 0.01 | (0.00,0.03) |
| South Boston | Holland | 0.01 | (0.00,0.03) | 0.01 | (0.00,0.02) | 0.00 | (0.00,0.02) |
| South Boston | Hurley | | | 0.02 | (0.00,0.05) | 0.02 | (0.00,0.04) |
| South Boston | Jackson/Mann | | | 0.01 | (0.00,0.03) | 0.01 | (0.00,0.03) |
| South Boston | Mason | 0.18 | (0.12,0.25) | 0.04 | (0.01,0.07) | 0.03 | (0.01,0.06) |
| South Boston | Mather | | | 0.00 | (0.00,0.02) | 0.00 | (0.00,0.02) |
| South Boston | Mission Hill | 0.01 | (0.00,0.03) | | | | |
| South Boston | Murphy | 0.02 | (0.00,0.05) | 0.01 | (0.00,0.03) | 0.01 | (0.00,0.03) |
| South Boston | Orchard Gardens | 0.04 | (0.01,0.07) | 0.03 | (0.01,0.07) | 0.04 | (0.01,0.07) |
| South Boston | Perkins | 0.03 | (0.00,0.06) | 0.05 | (0.01,0.09) | 0.05 | (0.01,0.09) |
| South Boston | Perry | 0.11 | (0.08,0.14) | 0.20 | (0.15,0.26) | 0.20 | (0.15,0.26) |
| South Boston | Quincy | 0.21 | (0.14,0.28) | 0.08 | (0.04,0.12) | 0.08 | (0.04,0.13) |
| South Boston | Roosevelt | 0.01 | (0.00,0.03) | | | 0.00 | (0.00,0.01) |
| South Boston | Russell | 0.02 | (0.01,0.03) | 0.04 | (0.01,0.08) | 0.03 | (0.01,0.07) |
| South Boston | Taylor | 0.01 | (0.00,0.03) | | | | |
| South Boston | Tynan | 0.01 | (0.00,0.03) | 0.05 | (0.02,0.09) | 0.05 | (0.01,0.09) |
| South Boston | UP Acad. Dor. | 0.03 | (0.01,0.04) | 0.02 | (0.01,0.05) | 0.03 | (0.01,0.06) |
| South Boston | Winthrop | | | 0.01 | (0.00,0.02) | 0.00 | (0.00,0.02) |
| South Dorchester | Channing | 0.01 | (0.00,0.01) | | | | |
| South Dorchester | Clap | 0.01 | (0.00,0.01) | 0.01 | (0.00,0.02) | 0.01 | (0.00,0.02) |
| South Dorchester | Condon | 0.04 | (0.03,0.06) | 0.03 | (0.02,0.04) | 0.03 | (0.02,0.04) |
| South Dorchester | Dever | 0.01 | (0.01,0.02) | 0.01 | (0.01,0.02) | 0.01 | (0.01,0.02) |
| South Dorchester | Dudley | 0.02 | (0.01,0.02) | 0.03 | (0.02,0.05) | 0.06 | (0.04,0.09) |
| South Dorchester | E Greenwood | 0.00 | (0.00,0.01) | | | | |
| South Dorchester | Ellison/Parks | | | 0.02 | (0.01,0.03) | 0.02 | (0.01,0.03) |
| South Dorchester | Everett | 0.01 | (0.00,0.02) | 0.02 | (0.01,0.04) | 0.02 | (0.01,0.03) |
| South Dorchester | Haynes | | | 0.02 | (0.01,0.03) | 0.01 | (0.00,0.02) |
| South Dorchester | Henderson | 0.28 | (0.23,0.32) | 0.06 | (0.04,0.09) | 0.06 | (0.04,0.08) |
| South Dorchester | Hernandez | 0.01 | (0.01,0.01) | 0.04 | (0.02,0.05) | 0.03 | (0.02,0.05) |
| South Dorchester | Holland | 0.05 | (0.04,0.06) | 0.07 | (0.05,0.09) | 0.06 | (0.05,0.08) |
| South Dorchester | Holmes | 0.03 | (0.02,0.04) | 0.04 | (0.03,0.06) | 0.04 | (0.02,0.05) |
| South Dorchester | Jackson/Mann | | | 0.01 | (0.00,0.02) | 0.01 | (0.00,0.02) |
| South Dorchester | Kenny | 0.04 | (0.03,0.06) | 0.05 | (0.04,0.07) | 0.05 | (0.03,0.06) |
| South Dorchester | King | 0.01 | (0.01,0.01) | 0.01 | (0.01,0.02) | 0.01 | (0.01,0.02) |
| South Dorchester | Lee | 0.01 | (0.00,0.02) | 0.03 | (0.01,0.06) | 0.02 | (0.00,0.05) |
| South Dorchester | Mason | 0.00 | (0.00,0.01) | | | | |
| South Dorchester | Mather | 0.11 | (0.09,0.14) | 0.10 | (0.08,0.12) | 0.09 | (0.07,0.11) |
| South Dorchester | Mattahunt | 0.01 | (0.00,0.01) | | | | |
| South Dorchester | Murphy | 0.13 | (0.11,0.16) | 0.19 | (0.16,0.23) | 0.21 | (0.17,0.25) |
| South Dorchester | Orchard Gardens | 0.00 | (0.00,0.01) | | | | |
| South Dorchester | Perkins | 0.01 | (0.00,0.02) | | | | |
| South Dorchester | Perry | 0.01 | (0.01,0.02) | 0.01 | (0.00,0.01) | 0.01 | (0.00,0.01) |
| South Dorchester | Russell | 0.02 | (0.02,0.03) | 0.02 | (0.01,0.03) | 0.02 | (0.01,0.03) |
| South Dorchester | S. Greenwood | 0.06 | (0.04,0.07) | 0.06 | (0.04,0.08) | 0.05 | (0.04,0.07) |
| South Dorchester | Taylor | 0.00 | (0.00,0.01) | 0.01 | (0.00,0.03) | 0.01 | (0.00,0.03) |

Continued on next page

**Table 7 – continued from previous page**

| | | Naive | | Logit | | Mixed Logit | |
|---|---|---|---|---|---|---|---|
| Neighborhood | School | mean | (95% C.I.) | mean | (95% C.I.) | mean | (95% C.I.) |
| South Dorchester | Tynan | 0.01 | (0.00,0.01) | | | | |
| South Dorchester | UP Acad. Dor. | 0.02 | (0.02,0.03) | 0.05 | (0.04,0.07) | 0.08 | (0.06,0.11) |
| South Dorchester | Young Achievers | 0.02 | (0.01,0.03) | 0.03 | (0.02,0.04) | 0.03 | (0.02,0.04) |
| South End | Baldwin | 0.01 | (0.01,0.02) | 0.01 | (0.00,0.02) | 0.01 | (0.00,0.02) |
| South End | Blackstone | 0.08 | (0.06,0.10) | 0.13 | (0.09,0.17) | 0.12 | (0.08,0.16) |
| South End | Clap | | | 0.00 | (0.00,0.01) | 0.00 | (0.00,0.01) |
| South End | Condon | 0.04 | (0.01,0.06) | 0.03 | (0.01,0.06) | 0.03 | (0.01,0.05) |
| South End | Dever | 0.01 | (0.00,0.02) | 0.00 | (0.00,0.01) | 0.00 | (0.00,0.01) |
| South End | Dudley | | | 0.03 | (0.01,0.05) | 0.07 | (0.04,0.11) |
| South End | Edison | 0.02 | (0.01,0.04) | 0.01 | (0.00,0.02) | 0.01 | (0.00,0.02) |
| South End | Eliot | 0.03 | (0.01,0.04) | 0.03 | (0.01,0.04) | 0.03 | (0.01,0.04) |
| South End | Gardner | 0.01 | (0.01,0.02) | 0.01 | (0.01,0.02) | 0.01 | (0.00,0.02) |
| South End | Hale | 0.02 | (0.01,0.03) | 0.02 | (0.01,0.04) | 0.02 | (0.01,0.04) |
| South End | Harvard/Kent | 0.02 | (0.01,0.03) | 0.01 | (0.01,0.02) | 0.01 | (0.00,0.02) |
| South End | Haynes | | | 0.01 | (0.00,0.02) | 0.01 | (0.00,0.02) |
| South End | Hennigan | | | 0.01 | (0.00,0.02) | 0.01 | (0.00,0.02) |
| South End | Hernandez | | | 0.03 | (0.01,0.04) | 0.02 | (0.01,0.04) |
| South End | Higginson/Lewis | 0.01 | (0.00,0.01) | 0.01 | (0.00,0.03) | 0.01 | (0.00,0.02) |
| South End | Hurley | 0.38 | (0.32,0.45) | 0.17 | (0.12,0.21) | 0.16 | (0.12,0.21) |
| South End | J.F. Kennedy | | | 0.00 | (0.00,0.01) | 0.00 | (0.00,0.01) |
| South End | Jackson/Mann | 0.02 | (0.01,0.04) | 0.03 | (0.01,0.05) | 0.02 | (0.01,0.04) |
| South End | Lyon K-8 | 0.01 | (0.00,0.02) | | | | |
| South End | Mario Umana | 0.01 | (0.00,0.03) | 0.00 | (0.00,0.01) | | |
| South End | Mason | 0.02 | (0.01,0.03) | 0.06 | (0.03,0.09) | 0.04 | (0.02,0.07) |
| South End | Orchard Gardens | 0.07 | (0.05,0.11) | 0.11 | (0.07,0.15) | 0.10 | (0.06,0.14) |
| South End | Perkins | | | 0.01 | (0.00,0.02) | 0.01 | (0.00,0.02) |
| South End | Quincy | 0.19 | (0.15,0.24) | 0.21 | (0.16,0.27) | 0.23 | (0.17,0.28) |
| South End | Russell | | | 0.00 | (0.00,0.01) | 0.00 | (0.00,0.01) |
| South End | Tobin | 0.01 | (0.00,0.03) | 0.03 | (0.01,0.06) | 0.02 | (0.01,0.04) |
| South End | Tynan | | | 0.00 | (0.00,0.01) | 0.00 | (0.00,0.01) |
| South End | UP Acad. Dor. | | | 0.01 | (0.00,0.03) | 0.01 | (0.00,0.04) |
| South End | Warren/Prescott | 0.01 | (0.00,0.03) | 0.00 | (0.00,0.01) | 0.00 | (0.00,0.01) |
| South End | West Zone ELC | | | 0.01 | (0.00,0.03) | 0.01 | (0.00,0.02) |
| South End | Winship | | | 0.00 | (0.00,0.01) | 0.00 | (0.00,0.01) |
| South End | Winthrop | 0.01 | (0.01,0.02) | 0.02 | (0.01,0.03) | 0.02 | (0.01,0.03) |
| West Roxbury | BTU | 0.01 | (0.00,0.02) | 0.01 | (0.00,0.02) | 0.01 | (0.00,0.02) |
| West Roxbury | Bates | | | 0.02 | (0.01,0.05) | 0.02 | (0.00,0.04) |
| West Roxbury | Beethoven | 0.13 | (0.10,0.16) | 0.23 | (0.19,0.28) | 0.23 | (0.18,0.28) |
| West Roxbury | Channing | 0.01 | (0.01,0.02) | 0.03 | (0.01,0.05) | 0.03 | (0.01,0.05) |
| West Roxbury | Conley | 0.01 | (0.00,0.03) | 0.01 | (0.00,0.03) | 0.01 | (0.00,0.02) |
| West Roxbury | Dudley | | | | | 0.01 | (0.00,0.03) |
| West Roxbury | E Greenwood | | | 0.01 | (0.00,0.03) | 0.01 | (0.00,0.03) |
| West Roxbury | Ellis | 0.01 | (0.00,0.02) | | | | |
| West Roxbury | Ellison/Parks | | | 0.00 | (0.00,0.02) | 0.00 | (0.00,0.01) |
| West Roxbury | Grew | 0.00 | (0.00,0.02) | 0.02 | (0.00,0.04) | 0.01 | (0.00,0.03) |
| West Roxbury | Hale | 0.02 | (0.01,0.03) | | | | |
| West Roxbury | Haley | 0.01 | (0.00,0.01) | 0.01 | (0.00,0.01) | 0.01 | (0.00,0.01) |
| West Roxbury | Hernandez | | | 0.00 | (0.00,0.02) | 0.01 | (0.00,0.02) |
| West Roxbury | J.F. Kennedy | 0.01 | (0.01,0.02) | 0.01 | (0.00,0.02) | 0.01 | (0.00,0.01) |
| West Roxbury | Kilmer | 0.29 | (0.24,0.33) | 0.27 | (0.22,0.33) | 0.29 | (0.24,0.34) |
| West Roxbury | Lyndon | 0.36 | (0.30,0.41) | 0.22 | (0.17,0.28) | 0.21 | (0.17,0.26) |
| West Roxbury | Manning | 0.00 | (0.00,0.01) | 0.01 | (0.00,0.02) | 0.01 | (0.00,0.02) |
| West Roxbury | Mozart | 0.04 | (0.03,0.06) | 0.07 | (0.04,0.10) | 0.06 | (0.04,0.09) |
| West Roxbury | Philbrick | 0.01 | (0.00,0.01) | | | | |
| West Roxbury | Roosevelt | | | 0.01 | (0.00,0.02) | 0.01 | (0.00,0.03) |

Continued on next page

**Table 7 – continued from previous page**

| Neighborhood | School | Naive mean | Naive (95% C.I.) | Logit mean | Logit (95% C.I.) | Mixed Logit mean | Mixed Logit (95% C.I.) |
|---|---|---|---|---|---|---|---|
| West Roxbury | Sumner | 0.04 | (0.02,0.06) | 0.02 | (0.01,0.04) | 0.02 | (0.01,0.03) |
| West Roxbury | Trotter | 0.01 | (0.00,0.01) | | | | |
| West Roxbury | UP Acad. Dor. | | | | | 0.01 | (0.00,0.02) |
| West Roxbury | West Zone ELC | 0.01 | (0.00,0.02) | 0.01 | (0.00,0.01) | 0.01 | (0.00,0.01) |

Table 8: Top 2 Choices Market Share Predictions for 2014 K2

| Neighborhood | School | Naive mean | Naive (95% C.I.) | Logit mean | Logit (95% C.I.) | Mixed Logit mean | Mixed Logit (95% C.I.) |
|---|---|---|---|---|---|---|---|
| Allston-Brighton | Baldwin | 0.08 | (0.06,0.10) | 0.17 | (0.14,0.20) | 0.17 | (0.14,0.20) |
| Allston-Brighton | Curley | | | 0.01 | (0.00,0.02) | 0.01 | (0.00,0.02) |
| Allston-Brighton | Dudley | | | | | 0.01 | (0.00,0.02) |
| Allston-Brighton | Edison | 0.11 | (0.07,0.14) | 0.12 | (0.09,0.15) | 0.10 | (0.08,0.14) |
| Allston-Brighton | Gardner | 0.07 | (0.05,0.09) | 0.16 | (0.12,0.19) | 0.17 | (0.13,0.20) |
| Allston-Brighton | Hale | 0.03 | (0.01,0.05) | | | | |
| Allston-Brighton | Hennigan | | | 0.01 | (0.00,0.02) | 0.01 | (0.00,0.02) |
| Allston-Brighton | Hernandez | 0.03 | (0.01,0.04) | 0.01 | (0.00,0.02) | 0.01 | (0.00,0.02) |
| Allston-Brighton | Hurley | 0.02 | (0.01,0.04) | | | | |
| Allston-Brighton | Jackson/Mann | 0.17 | (0.13,0.20) | 0.17 | (0.13,0.21) | 0.16 | (0.12,0.20) |
| Allston-Brighton | Kennedy Patrick | 0.00 | (0.00,0.01) | | | | |
| Allston-Brighton | Lyon K-8 | 0.25 | (0.23,0.29) | 0.13 | (0.10,0.17) | 0.15 | (0.11,0.19) |
| Allston-Brighton | Manning | 0.09 | (0.06,0.12) | 0.00 | (0.00,0.01) | 0.00 | (0.00,0.01) |
| Allston-Brighton | Mason | 0.01 | (0.00,0.01) | | | | |
| Allston-Brighton | Mendell | | | 0.00 | (0.00,0.01) | 0.00 | (0.00,0.01) |
| Allston-Brighton | Quincy | 0.03 | (0.02,0.05) | 0.01 | (0.00,0.02) | 0.01 | (0.00,0.02) |
| Allston-Brighton | Tobin | | | 0.00 | (0.00,0.01) | 0.00 | (0.00,0.01) |
| Allston-Brighton | UP Acad. Dor. | | | | | 0.01 | (0.00,0.02) |
| Allston-Brighton | Warren/Prescott | 0.01 | (0.00,0.01) | | | | |
| Allston-Brighton | Winship | 0.09 | (0.07,0.12) | 0.19 | (0.15,0.23) | 0.18 | (0.14,0.21) |
| Charlestown | Adams | 0.00 | (0.00,0.01) | | | | |
| Charlestown | Baldwin | 0.01 | (0.00,0.01) | | | | |
| Charlestown | Blackstone | | | 0.01 | (0.00,0.03) | 0.02 | (0.00,0.03) |
| Charlestown | Dudley | | | 0.01 | (0.00,0.02) | 0.02 | (0.01,0.04) |
| Charlestown | East Boston EEC | | | 0.02 | (0.01,0.04) | 0.03 | (0.01,0.05) |
| Charlestown | Edison | 0.01 | (0.00,0.01) | 0.01 | (0.00,0.01) | 0.01 | (0.00,0.01) |
| Charlestown | Eliot | 0.05 | (0.03,0.07) | 0.32 | (0.28,0.38) | 0.32 | (0.27,0.37) |
| Charlestown | Harvard/Kent | 0.45 | (0.43,0.47) | 0.22 | (0.18,0.26) | 0.21 | (0.17,0.25) |
| Charlestown | Hernandez | | | 0.01 | (0.00,0.01) | 0.01 | (0.00,0.02) |
| Charlestown | Hurley | 0.01 | (0.00,0.02) | 0.00 | (0.00,0.01) | 0.00 | (0.00,0.01) |
| Charlestown | Kennedy Patrick | 0.00 | (0.00,0.01) | | | | |
| Charlestown | Mario Umana | 0.01 | (0.00,0.02) | 0.02 | (0.00,0.04) | 0.01 | (0.00,0.03) |
| Charlestown | O'Donnell | | | 0.02 | (0.01,0.04) | 0.02 | (0.00,0.03) |
| Charlestown | Orchard Gardens | 0.01 | (0.00,0.02) | 0.00 | (0.00,0.01) | 0.00 | (0.00,0.01) |
| Charlestown | Otis | 0.03 | (0.01,0.04) | 0.01 | (0.00,0.02) | 0.01 | (0.00,0.02) |
| Charlestown | Perkins | | | 0.01 | (0.00,0.02) | 0.01 | (0.00,0.02) |
| Charlestown | Quincy | | | 0.05 | (0.02,0.07) | 0.05 | (0.02,0.07) |
| Charlestown | Tynan | | | 0.01 | (0.00,0.02) | 0.01 | (0.00,0.02) |
| Charlestown | UP Acad. Dor. | | | 0.00 | (0.00,0.01) | 0.01 | (0.00,0.02) |
| Charlestown | Warren/Prescott | 0.39 | (0.37,0.42) | 0.27 | (0.22,0.31) | 0.27 | (0.23,0.31) |
| Charlestown | Winship | 0.01 | (0.00,0.01) | | | | |
| Downtown | Blackstone | | | 0.03 | (0.01,0.05) | 0.02 | (0.01,0.04) |
| Downtown | Condon | | | 0.02 | (0.00,0.03) | 0.01 | (0.00,0.03) |

Continued on next page

Table 8 – continued from previous page

| Neighborhood | School | Naive mean | Naive (95% C.I.) | Logit mean | Logit (95% C.I.) | Mixed Logit mean | Mixed Logit (95% C.I.) |
|---|---|---|---|---|---|---|---|
| Downtown | Dudley | | | 0.01 | (0.00,0.02) | 0.03 | (0.01,0.05) |
| Downtown | East Boston EEC | | | 0.00 | (0.00,0.01) | 0.01 | (0.00,0.02) |
| Downtown | Edison | 0.00 | (0.00,0.01) | 0.01 | (0.00,0.02) | 0.01 | (0.00,0.02) |
| Downtown | Eliot | 0.32 | (0.25,0.38) | 0.31 | (0.26,0.36) | 0.32 | (0.27,0.38) |
| Downtown | Hale | 0.02 | (0.00,0.03) | 0.00 | (0.00,0.01) | 0.00 | (0.00,0.01) |
| Downtown | Harvard/Kent | 0.05 | (0.03,0.07) | 0.05 | (0.03,0.07) | 0.05 | (0.03,0.07) |
| Downtown | Hennigan | 0.00 | (0.00,0.01) | 0.01 | (0.00,0.03) | 0.01 | (0.00,0.02) |
| Downtown | Hernandez | | | 0.01 | (0.00,0.02) | 0.01 | (0.00,0.02) |
| Downtown | Higginson/Lewis | | | 0.00 | (0.00,0.01) | | |
| Downtown | Hurley | 0.13 | (0.09,0.16) | 0.06 | (0.04,0.08) | 0.05 | (0.03,0.08) |
| Downtown | J.F. Kennedy | | | 0.00 | (0.00,0.01) | 0.00 | (0.00,0.01) |
| Downtown | Jackson/Mann | 0.13 | (0.09,0.17) | 0.03 | (0.01,0.04) | 0.02 | (0.01,0.05) |
| Downtown | Mason | | | 0.01 | (0.00,0.03) | 0.01 | (0.00,0.02) |
| Downtown | Orchard Gardens | 0.02 | (0.01,0.03) | 0.04 | (0.02,0.06) | 0.03 | (0.02,0.05) |
| Downtown | Perkins | | | 0.01 | (0.00,0.02) | 0.01 | (0.00,0.02) |
| Downtown | Quincy | 0.29 | (0.24,0.34) | 0.30 | (0.24,0.35) | 0.30 | (0.25,0.35) |
| Downtown | Tobin | 0.00 | (0.00,0.01) | 0.01 | (0.00,0.03) | 0.01 | (0.00,0.03) |
| Downtown | Tynan | | | 0.01 | (0.00,0.02) | 0.01 | (0.00,0.02) |
| Downtown | UP Acad. Dor. | 0.00 | (0.00,0.01) | 0.01 | (0.00,0.01) | 0.01 | (0.00,0.02) |
| Downtown | Warren/Prescott | 0.01 | (0.00,0.02) | 0.04 | (0.02,0.06) | 0.03 | (0.01,0.05) |
| Downtown | West Zone ELC | | | 0.01 | (0.00,0.02) | 0.01 | (0.00,0.02) |
| Downtown | Winship | | | 0.01 | (0.00,0.02) | 0.01 | (0.00,0.02) |
| Downtown | Winthrop | 0.01 | (0.00,0.01) | | | | |
| East Boston | Adams | 0.06 | (0.05,0.07) | 0.06 | (0.04,0.07) | 0.05 | (0.04,0.06) |
| East Boston | Blackstone | 0.03 | (0.02,0.04) | 0.01 | (0.00,0.01) | 0.01 | (0.01,0.02) |
| East Boston | Bradley | 0.18 | (0.16,0.20) | 0.07 | (0.06,0.09) | 0.08 | (0.07,0.10) |
| East Boston | Dudley | | | | | 0.01 | (0.00,0.02) |
| East Boston | East Boston EEC | 0.04 | (0.03,0.05) | 0.13 | (0.11,0.15) | 0.13 | (0.10,0.15) |
| East Boston | Eliot | 0.01 | (0.00,0.01) | 0.01 | (0.00,0.01) | 0.01 | (0.00,0.01) |
| East Boston | Gardner | 0.00 | (0.00,0.01) | | | | |
| East Boston | Guild | 0.03 | (0.02,0.04) | 0.06 | (0.05,0.08) | 0.06 | (0.04,0.08) |
| East Boston | Harvard/Kent | 0.01 | (0.00,0.01) | 0.01 | (0.00,0.01) | 0.01 | (0.00,0.01) |
| East Boston | Hernandez | | | | | 0.01 | (0.00,0.02) |
| East Boston | Hurley | 0.01 | (0.00,0.01) | | | | |
| East Boston | Jackson/Mann | 0.00 | (0.00,0.01) | | | | |
| East Boston | Kennedy Patrick | 0.15 | (0.13,0.17) | 0.17 | (0.15,0.19) | 0.17 | (0.15,0.19) |
| East Boston | Mario Umana | 0.13 | (0.11,0.15) | 0.10 | (0.08,0.12) | 0.11 | (0.08,0.13) |
| East Boston | McKay | 0.03 | (0.02,0.04) | 0.14 | (0.12,0.17) | 0.13 | (0.11,0.16) |
| East Boston | O'Donnell | 0.05 | (0.04,0.06) | 0.15 | (0.13,0.17) | 0.14 | (0.12,0.16) |
| East Boston | Otis | 0.24 | (0.21,0.26) | 0.08 | (0.06,0.09) | 0.07 | (0.06,0.09) |
| East Boston | Tobin | 0.01 | (0.00,0.01) | | | | |
| East Boston | UP Acad. Dor. | | | | | 0.01 | (0.00,0.02) |
| East Boston | Winthrop | 0.02 | (0.01,0.02) | | | | |
| Hyde Park | Bates | | | 0.05 | (0.03,0.07) | 0.04 | (0.02,0.06) |
| Hyde Park | Beethoven | 0.02 | (0.01,0.03) | 0.08 | (0.06,0.10) | 0.07 | (0.05,0.09) |
| Hyde Park | Channing | 0.03 | (0.02,0.04) | 0.07 | (0.05,0.10) | 0.07 | (0.05,0.09) |
| Hyde Park | Chittick | 0.04 | (0.03,0.05) | 0.05 | (0.04,0.07) | 0.05 | (0.03,0.07) |
| Hyde Park | Condon | 0.01 | (0.00,0.01) | | | | |
| Hyde Park | Conley | 0.28 | (0.25,0.30) | 0.06 | (0.04,0.08) | 0.05 | (0.03,0.08) |
| Hyde Park | Dudley | | | 0.01 | (0.00,0.02) | 0.03 | (0.01,0.04) |
| Hyde Park | E Greenwood | 0.06 | (0.04,0.08) | 0.11 | (0.08,0.14) | 0.11 | (0.08,0.14) |
| Hyde Park | Ellison/Parks | | | 0.05 | (0.03,0.07) | 0.04 | (0.03,0.06) |
| Hyde Park | Grew | 0.02 | (0.01,0.03) | 0.06 | (0.04,0.08) | 0.06 | (0.04,0.08) |
| Hyde Park | Haley | | | 0.03 | (0.02,0.05) | 0.04 | (0.02,0.05) |
| Hyde Park | Hernandez | 0.02 | (0.01,0.03) | 0.03 | (0.01,0.04) | 0.02 | (0.01,0.04) |

Continued on next page

**Table 8 – continued from previous page**

| | | Naive | | Logit | | Mixed Logit | |
|---|---|---|---|---|---|---|---|
| Neighborhood | School | mean | (95% C.I.) | mean | (95% C.I.) | mean | (95% C.I.) |
| Hyde Park | Holland | 0.00 | (0.00,0.01) | | | | |
| Hyde Park | Kilmer | 0.02 | (0.01,0.03) | 0.03 | (0.02,0.05) | 0.04 | (0.02,0.05) |
| Hyde Park | Mather | 0.01 | (0.00,0.01) | | | | |
| Hyde Park | Mattahunt | 0.04 | (0.03,0.05) | 0.03 | (0.02,0.05) | 0.04 | (0.02,0.05) |
| Hyde Park | Mozart | | | 0.03 | (0.02,0.05) | 0.03 | (0.01,0.05) |
| Hyde Park | Philbrick | 0.10 | (0.07,0.13) | 0.03 | (0.02,0.05) | 0.03 | (0.01,0.04) |
| Hyde Park | Roosevelt | 0.21 | (0.18,0.24) | 0.17 | (0.14,0.20) | 0.18 | (0.15,0.21) |
| Hyde Park | Russell | 0.01 | (0.00,0.01) | | | | |
| Hyde Park | S. Greenwood | 0.02 | (0.01,0.02) | 0.01 | (0.00,0.01) | 0.01 | (0.00,0.01) |
| Hyde Park | Sumner | 0.02 | (0.01,0.04) | 0.03 | (0.01,0.04) | 0.02 | (0.01,0.04) |
| Hyde Park | Taylor | 0.02 | (0.01,0.02) | 0.01 | (0.01,0.02) | 0.01 | (0.00,0.02) |
| Hyde Park | UP Acad. Dor. | 0.02 | (0.01,0.03) | 0.01 | (0.00,0.03) | 0.02 | (0.01,0.04) |
| Hyde Park | Young Achievers | 0.03 | (0.02,0.04) | 0.02 | (0.01,0.03) | 0.02 | (0.01,0.03) |
| Jamaica Plain | BTU | 0.01 | (0.01,0.01) | 0.05 | (0.03,0.07) | 0.04 | (0.03,0.06) |
| Jamaica Plain | Bates | 0.01 | (0.00,0.01) | | | | |
| Jamaica Plain | Blackstone | | | 0.01 | (0.00,0.01) | 0.01 | (0.00,0.01) |
| Jamaica Plain | Curley | 0.08 | (0.06,0.10) | 0.14 | (0.12,0.17) | 0.14 | (0.11,0.16) |
| Jamaica Plain | Dudley | | | 0.02 | (0.01,0.03) | 0.04 | (0.03,0.06) |
| Jamaica Plain | Edison | 0.01 | (0.00,0.02) | 0.01 | (0.00,0.01) | 0.01 | (0.00,0.01) |
| Jamaica Plain | Ellis | 0.03 | (0.02,0.04) | 0.03 | (0.02,0.04) | 0.02 | (0.01,0.03) |
| Jamaica Plain | Hale | 0.26 | (0.23,0.28) | 0.02 | (0.01,0.04) | 0.02 | (0.01,0.03) |
| Jamaica Plain | Haley | 0.01 | (0.00,0.01) | 0.01 | (0.00,0.02) | 0.01 | (0.00,0.02) |
| Jamaica Plain | Harvard/Kent | 0.01 | (0.00,0.01) | | | | |
| Jamaica Plain | Hennigan | 0.05 | (0.04,0.07) | 0.09 | (0.07,0.12) | 0.09 | (0.06,0.11) |
| Jamaica Plain | Hernandez | 0.01 | (0.01,0.02) | 0.06 | (0.04,0.08) | 0.07 | (0.05,0.09) |
| Jamaica Plain | Higginson/Lewis | | | 0.01 | (0.00,0.01) | 0.00 | (0.00,0.01) |
| Jamaica Plain | Hurley | 0.06 | (0.04,0.09) | 0.02 | (0.01,0.04) | 0.02 | (0.01,0.04) |
| Jamaica Plain | J.F. Kennedy | 0.05 | (0.03,0.07) | 0.08 | (0.06,0.11) | 0.07 | (0.05,0.10) |
| Jamaica Plain | Jackson/Mann | 0.01 | (0.00,0.01) | 0.03 | (0.01,0.04) | 0.03 | (0.01,0.04) |
| Jamaica Plain | Lyndon | 0.01 | (0.00,0.01) | 0.01 | (0.00,0.01) | 0.01 | (0.00,0.01) |
| Jamaica Plain | Manning | 0.17 | (0.14,0.19) | 0.05 | (0.03,0.07) | 0.05 | (0.03,0.07) |
| Jamaica Plain | Mason | 0.03 | (0.01,0.05) | 0.01 | (0.00,0.01) | 0.01 | (0.00,0.01) |
| Jamaica Plain | Mendell | 0.05 | (0.04,0.06) | 0.08 | (0.06,0.10) | 0.08 | (0.06,0.10) |
| Jamaica Plain | Mission Hill | 0.01 | (0.00,0.02) | 0.09 | (0.06,0.11) | 0.09 | (0.06,0.11) |
| Jamaica Plain | Murphy | 0.01 | (0.01,0.01) | | | | |
| Jamaica Plain | Orchard Gardens | | | 0.02 | (0.01,0.04) | 0.02 | (0.01,0.04) |
| Jamaica Plain | Philbrick | 0.01 | (0.00,0.02) | 0.00 | (0.00,0.01) | | |
| Jamaica Plain | Quincy | 0.02 | (0.00,0.03) | 0.01 | (0.00,0.02) | 0.01 | (0.00,0.02) |
| Jamaica Plain | Sumner | 0.02 | (0.01,0.04) | 0.01 | (0.00,0.01) | 0.01 | (0.00,0.01) |
| Jamaica Plain | Tobin | 0.01 | (0.00,0.02) | 0.04 | (0.02,0.06) | 0.04 | (0.02,0.06) |
| Jamaica Plain | Trotter | 0.01 | (0.01,0.02) | 0.02 | (0.01,0.03) | 0.02 | (0.01,0.03) |
| Jamaica Plain | UP Acad. Dor. | 0.01 | (0.00,0.02) | 0.01 | (0.00,0.03) | 0.02 | (0.01,0.04) |
| Jamaica Plain | West Zone ELC | 0.02 | (0.01,0.03) | 0.06 | (0.04,0.08) | 0.06 | (0.04,0.08) |
| Mattapan | BTU | | | 0.04 | (0.02,0.05) | 0.04 | (0.02,0.05) |
| Mattapan | Beethoven | 0.00 | (0.00,0.01) | | | | |
| Mattapan | Channing | 0.01 | (0.01,0.02) | 0.01 | (0.01,0.01) | 0.01 | (0.00,0.01) |
| Mattapan | Chittick | 0.01 | (0.01,0.02) | 0.02 | (0.01,0.04) | 0.02 | (0.01,0.03) |
| Mattapan | Condon | 0.01 | (0.00,0.01) | | | | |
| Mattapan | Conley | 0.06 | (0.04,0.08) | 0.01 | (0.00,0.02) | 0.01 | (0.00,0.02) |
| Mattapan | Dever | 0.03 | (0.02,0.04) | 0.02 | (0.01,0.03) | 0.02 | (0.01,0.03) |
| Mattapan | Dudley | 0.01 | (0.01,0.01) | 0.03 | (0.02,0.05) | 0.07 | (0.05,0.09) |
| Mattapan | E Greenwood | 0.02 | (0.01,0.03) | 0.02 | (0.01,0.03) | 0.02 | (0.01,0.03) |
| Mattapan | Ellis | 0.00 | (0.00,0.01) | | | | |
| Mattapan | Ellison/Parks | 0.01 | (0.01,0.02) | 0.11 | (0.08,0.14) | 0.11 | (0.09,0.14) |
| Mattapan | Haley | | | 0.08 | (0.06,0.10) | 0.07 | (0.05,0.09) |

Continued on next page

**Table 8 – continued from previous page**

| Neighborhood | School | Naive mean | Naive (95% C.I.) | Logit mean | Logit (95% C.I.) | Mixed Logit mean | Mixed Logit (95% C.I.) |
|---|---|---|---|---|---|---|---|
| Mattapan | Henderson | 0.20 | (0.18,0.23) | 0.02 | (0.01,0.03) | 0.03 | (0.01,0.04) |
| Mattapan | Hernandez | 0.02 | (0.01,0.02) | 0.05 | (0.04,0.07) | 0.05 | (0.03,0.06) |
| Mattapan | Holland | 0.03 | (0.02,0.04) | 0.02 | (0.01,0.03) | 0.02 | (0.01,0.03) |
| Mattapan | Holmes | 0.01 | (0.01,0.02) | 0.02 | (0.01,0.03) | 0.02 | (0.01,0.03) |
| Mattapan | Jackson/Mann | | | 0.01 | (0.00,0.02) | 0.01 | (0.00,0.02) |
| Mattapan | Kenny | 0.01 | (0.01,0.02) | 0.02 | (0.01,0.03) | 0.02 | (0.01,0.03) |
| Mattapan | Lee | 0.01 | (0.00,0.01) | 0.03 | (0.01,0.06) | 0.03 | (0.01,0.05) |
| Mattapan | Mather | 0.01 | (0.00,0.01) | 0.01 | (0.00,0.01) | 0.01 | (0.00,0.01) |
| Mattapan | Mattahunt | 0.03 | (0.02,0.04) | 0.04 | (0.03,0.06) | 0.04 | (0.02,0.05) |
| Mattapan | Murphy | 0.06 | (0.04,0.08) | 0.02 | (0.01,0.04) | 0.03 | (0.01,0.04) |
| Mattapan | Philbrick | 0.24 | (0.21,0.26) | 0.03 | (0.02,0.05) | 0.03 | (0.01,0.04) |
| Mattapan | Russell | 0.02 | (0.01,0.02) | 0.01 | (0.01,0.01) | 0.01 | (0.01,0.01) |
| Mattapan | S. Greenwood | 0.04 | (0.02,0.05) | 0.06 | (0.04,0.07) | 0.05 | (0.04,0.07) |
| Mattapan | Sumner | 0.03 | (0.01,0.04) | 0.01 | (0.00,0.02) | 0.01 | (0.00,0.01) |
| Mattapan | Taylor | 0.05 | (0.03,0.06) | 0.06 | (0.05,0.09) | 0.06 | (0.04,0.08) |
| Mattapan | UP Acad. Dor. | 0.01 | (0.01,0.02) | 0.05 | (0.03,0.06) | 0.07 | (0.05,0.09) |
| Mattapan | Young Achievers | 0.03 | (0.02,0.04) | 0.15 | (0.12,0.18) | 0.14 | (0.12,0.17) |
| North Dorchester | Blackstone | | | 0.00 | (0.00,0.01) | 0.00 | (0.00,0.01) |
| North Dorchester | Clap | 0.01 | (0.00,0.01) | 0.07 | (0.05,0.10) | 0.06 | (0.04,0.09) |
| North Dorchester | Condon | 0.11 | (0.09,0.14) | 0.05 | (0.03,0.07) | 0.05 | (0.03,0.07) |
| North Dorchester | Dever | 0.02 | (0.01,0.03) | 0.07 | (0.04,0.09) | 0.06 | (0.04,0.08) |
| North Dorchester | Dudley | 0.02 | (0.01,0.03) | 0.05 | (0.03,0.07) | 0.10 | (0.08,0.13) |
| North Dorchester | Edison | 0.01 | (0.00,0.01) | | | | |
| North Dorchester | Everett | | | 0.09 | (0.06,0.12) | 0.08 | (0.06,0.11) |
| North Dorchester | Harvard/Kent | 0.01 | (0.00,0.01) | | | | |
| North Dorchester | Haynes | | | 0.04 | (0.02,0.06) | 0.04 | (0.02,0.06) |
| North Dorchester | Henderson | 0.06 | (0.04,0.08) | 0.02 | (0.01,0.04) | 0.02 | (0.01,0.04) |
| North Dorchester | Hernandez | | | 0.03 | (0.01,0.04) | 0.02 | (0.01,0.04) |
| North Dorchester | Holland | 0.03 | (0.01,0.04) | 0.04 | (0.03,0.06) | 0.03 | (0.02,0.05) |
| North Dorchester | Holmes | 0.01 | (0.00,0.01) | | | | |
| North Dorchester | Hurley | | | 0.01 | (0.00,0.01) | 0.01 | (0.00,0.01) |
| North Dorchester | Jackson/Mann | | | 0.01 | (0.00,0.03) | 0.01 | (0.00,0.03) |
| North Dorchester | King | 0.01 | (0.00,0.02) | 0.02 | (0.01,0.03) | 0.01 | (0.01,0.03) |
| North Dorchester | Mason | 0.37 | (0.30,0.44) | 0.06 | (0.04,0.09) | 0.06 | (0.04,0.08) |
| North Dorchester | Mather | 0.05 | (0.03,0.06) | 0.08 | (0.06,0.10) | 0.08 | (0.06,0.10) |
| North Dorchester | Murphy | 0.03 | (0.02,0.05) | 0.03 | (0.02,0.04) | 0.03 | (0.02,0.05) |
| North Dorchester | Orchard Gardens | 0.04 | (0.03,0.06) | 0.06 | (0.04,0.08) | 0.06 | (0.04,0.08) |
| North Dorchester | Perkins | | | 0.01 | (0.00,0.03) | 0.01 | (0.00,0.02) |
| North Dorchester | Perry | | | 0.01 | (0.00,0.02) | 0.01 | (0.00,0.02) |
| North Dorchester | Russell | 0.07 | (0.05,0.09) | 0.10 | (0.08,0.12) | 0.09 | (0.07,0.12) |
| North Dorchester | S. Greenwood | 0.02 | (0.01,0.03) | 0.01 | (0.00,0.02) | 0.01 | (0.00,0.02) |
| North Dorchester | Sumner | 0.00 | (0.00,0.01) | | | | |
| North Dorchester | Taylor | 0.00 | (0.00,0.01) | | | | |
| North Dorchester | Trotter | 0.00 | (0.00,0.01) | 0.00 | (0.00,0.01) | | |
| North Dorchester | Tynan | 0.00 | (0.00,0.01) | 0.01 | (0.00,0.01) | 0.00 | (0.00,0.01) |
| North Dorchester | UP Acad. Dor. | 0.02 | (0.01,0.03) | 0.04 | (0.02,0.06) | 0.06 | (0.04,0.09) |
| North Dorchester | Winthrop | 0.07 | (0.05,0.09) | 0.06 | (0.04,0.08) | 0.04 | (0.03,0.06) |
| Roslindale | BTU | 0.01 | (0.01,0.02) | 0.11 | (0.09,0.14) | 0.11 | (0.09,0.14) |
| Roslindale | Bates | 0.01 | (0.00,0.01) | 0.09 | (0.06,0.11) | 0.08 | (0.06,0.11) |
| Roslindale | Beethoven | 0.04 | (0.03,0.06) | 0.04 | (0.03,0.06) | 0.04 | (0.03,0.06) |
| Roslindale | Channing | | | 0.00 | (0.00,0.01) | 0.00 | (0.00,0.01) |
| Roslindale | Chittick | | | 0.01 | (0.00,0.01) | 0.00 | (0.00,0.01) |
| Roslindale | Conley | 0.14 | (0.11,0.16) | 0.06 | (0.04,0.08) | 0.05 | (0.04,0.07) |
| Roslindale | Curley | 0.03 | (0.02,0.04) | 0.01 | (0.01,0.02) | 0.02 | (0.01,0.02) |
| Roslindale | Dudley | | | 0.01 | (0.00,0.02) | 0.03 | (0.01,0.04) |

Continued on next page

**Table 8 – continued from previous page**

| Neighborhood | School | Naive mean | Naive (95% C.I.) | Logit mean | Logit (95% C.I.) | Mixed Logit mean | Mixed Logit (95% C.I.) |
|---|---|---|---|---|---|---|---|
| Roslindale | E Greenwood | 0.02 | (0.01,0.03) | 0.04 | (0.02,0.06) | 0.04 | (0.02,0.06) |
| Roslindale | Ellis | 0.01 | (0.01,0.02) | 0.01 | (0.00,0.01) | 0.01 | (0.00,0.01) |
| Roslindale | Ellison/Parks | | | 0.02 | (0.01,0.03) | 0.02 | (0.01,0.03) |
| Roslindale | Grew | | | 0.01 | (0.00,0.01) | 0.01 | (0.00,0.01) |
| Roslindale | Haley | 0.02 | (0.01,0.03) | 0.07 | (0.05,0.09) | 0.07 | (0.06,0.09) |
| Roslindale | Hennigan | 0.01 | (0.00,0.02) | | | | |
| Roslindale | Hernandez | 0.02 | (0.01,0.03) | 0.04 | (0.02,0.05) | 0.04 | (0.03,0.05) |
| Roslindale | Higginson/Lewis | 0.01 | (0.00,0.01) | | | | |
| Roslindale | J.F. Kennedy | 0.01 | (0.00,0.01) | | | | |
| Roslindale | Jackson/Mann | 0.01 | (0.00,0.02) | | | | |
| Roslindale | Kilmer | 0.01 | (0.01,0.02) | 0.02 | (0.01,0.03) | 0.02 | (0.01,0.03) |
| Roslindale | King | 0.01 | (0.00,0.01) | | | | |
| Roslindale | Lyndon | 0.05 | (0.04,0.06) | 0.07 | (0.05,0.09) | 0.06 | (0.05,0.08) |
| Roslindale | Manning | 0.01 | (0.01,0.03) | 0.02 | (0.01,0.03) | 0.02 | (0.01,0.03) |
| Roslindale | Mattahunt | | | 0.01 | (0.01,0.02) | 0.01 | (0.01,0.03) |
| Roslindale | Mendell | 0.01 | (0.00,0.01) | 0.01 | (0.00,0.01) | 0.01 | (0.00,0.01) |
| Roslindale | Mission Hill | | | 0.02 | (0.01,0.03) | 0.02 | (0.01,0.03) |
| Roslindale | Mozart | 0.02 | (0.01,0.02) | 0.09 | (0.07,0.11) | 0.09 | (0.07,0.11) |
| Roslindale | Philbrick | 0.17 | (0.14,0.19) | 0.08 | (0.06,0.10) | 0.07 | (0.04,0.09) |
| Roslindale | Sumner | 0.30 | (0.28,0.33) | 0.10 | (0.07,0.12) | 0.10 | (0.08,0.12) |
| Roslindale | Trotter | 0.02 | (0.01,0.02) | 0.01 | (0.01,0.01) | 0.01 | (0.00,0.01) |
| Roslindale | UP Acad. Dor. | 0.01 | (0.00,0.02) | 0.01 | (0.00,0.02) | 0.02 | (0.01,0.03) |
| Roslindale | Young Achievers | 0.01 | (0.00,0.02) | 0.02 | (0.01,0.03) | 0.02 | (0.01,0.04) |
| Roxbury | BTU | 0.01 | (0.00,0.01) | 0.01 | (0.01,0.01) | 0.01 | (0.01,0.01) |
| Roxbury | Beethoven | 0.01 | (0.00,0.01) | | | | |
| Roxbury | Blackstone | | | 0.01 | (0.01,0.02) | 0.01 | (0.01,0.02) |
| Roxbury | Clap | | | 0.01 | (0.01,0.02) | 0.01 | (0.00,0.01) |
| Roxbury | Condon | 0.02 | (0.01,0.02) | | | | |
| Roxbury | Curley | 0.03 | (0.02,0.03) | 0.03 | (0.02,0.04) | 0.03 | (0.02,0.04) |
| Roxbury | Dudley | 0.01 | (0.01,0.01) | 0.05 | (0.04,0.06) | 0.11 | (0.09,0.13) |
| Roxbury | Ellis | 0.03 | (0.03,0.04) | 0.03 | (0.03,0.04) | 0.03 | (0.03,0.04) |
| Roxbury | Everett | | | 0.02 | (0.01,0.03) | 0.02 | (0.01,0.03) |
| Roxbury | Hale | 0.18 | (0.16,0.19) | 0.04 | (0.03,0.04) | 0.03 | (0.02,0.04) |
| Roxbury | Haley | | | 0.01 | (0.01,0.01) | 0.01 | (0.00,0.01) |
| Roxbury | Haynes | | | 0.05 | (0.03,0.06) | 0.04 | (0.03,0.05) |
| Roxbury | Henderson | 0.06 | (0.05,0.07) | 0.01 | (0.00,0.01) | 0.01 | (0.00,0.01) |
| Roxbury | Hennigan | 0.03 | (0.02,0.04) | 0.03 | (0.02,0.04) | 0.03 | (0.02,0.04) |
| Roxbury | Hernandez | 0.02 | (0.01,0.02) | 0.06 | (0.05,0.08) | 0.07 | (0.06,0.09) |
| Roxbury | Higginson/Lewis | 0.02 | (0.02,0.03) | 0.03 | (0.02,0.04) | 0.02 | (0.02,0.03) |
| Roxbury | Holland | 0.02 | (0.01,0.03) | 0.03 | (0.03,0.05) | 0.03 | (0.02,0.04) |
| Roxbury | Holmes | | | 0.01 | (0.01,0.02) | 0.01 | (0.01,0.02) |
| Roxbury | Hurley | 0.04 | (0.03,0.05) | 0.02 | (0.01,0.03) | 0.02 | (0.01,0.03) |
| Roxbury | J.F. Kennedy | 0.03 | (0.02,0.04) | 0.04 | (0.03,0.05) | 0.03 | (0.02,0.05) |
| Roxbury | Jackson/Mann | 0.01 | (0.01,0.02) | 0.02 | (0.01,0.03) | 0.02 | (0.01,0.03) |
| Roxbury | King | 0.01 | (0.01,0.02) | 0.02 | (0.01,0.03) | 0.02 | (0.01,0.03) |
| Roxbury | Lee | | | 0.01 | (0.00,0.01) | 0.01 | (0.00,0.01) |
| Roxbury | Lyndon | 0.01 | (0.00,0.01) | | | | |
| Roxbury | Mason | 0.23 | (0.20,0.26) | 0.05 | (0.04,0.07) | 0.05 | (0.04,0.07) |
| Roxbury | Mather | | | 0.02 | (0.01,0.03) | 0.02 | (0.01,0.02) |
| Roxbury | Mendell | | | 0.02 | (0.01,0.03) | 0.02 | (0.01,0.03) |
| Roxbury | Mission Hill | | | 0.02 | (0.01,0.02) | 0.02 | (0.01,0.02) |
| Roxbury | Murphy | 0.02 | (0.01,0.03) | | | 0.01 | (0.00,0.01) |
| Roxbury | Orchard Gardens | 0.04 | (0.03,0.05) | 0.07 | (0.06,0.09) | 0.06 | (0.05,0.08) |
| Roxbury | Russell | 0.01 | (0.00,0.01) | 0.02 | (0.01,0.03) | 0.02 | (0.01,0.03) |
| Roxbury | S. Greenwood | 0.01 | (0.01,0.02) | 0.03 | (0.02,0.04) | 0.03 | (0.02,0.03) |

Continued on next page

**Table 8 – continued from previous page**

| Neighborhood | School | Naive mean | Naive (95% C.I.) | Logit mean | Logit (95% C.I.) | Mixed Logit mean | Mixed Logit (95% C.I.) |
|---|---|---|---|---|---|---|---|
| Roxbury | Tobin | | | 0.02 | (0.01,0.03) | 0.02 | (0.01,0.03) |
| Roxbury | Trotter | 0.02 | (0.02,0.03) | 0.05 | (0.04,0.07) | 0.04 | (0.03,0.05) |
| Roxbury | UP Acad. Dor. | 0.02 | (0.01,0.02) | 0.04 | (0.03,0.05) | 0.06 | (0.04,0.07) |
| Roxbury | West Zone ELC | | | 0.02 | (0.01,0.02) | 0.01 | (0.01,0.02) |
| Roxbury | Winthrop | 0.03 | (0.02,0.04) | 0.04 | (0.03,0.05) | 0.04 | (0.03,0.05) |
| South Boston | Blackstone | | | 0.03 | (0.01,0.05) | 0.03 | (0.01,0.05) |
| South Boston | Clap | 0.01 | (0.00,0.02) | 0.05 | (0.03,0.08) | 0.05 | (0.03,0.07) |
| South Boston | Condon | 0.13 | (0.10,0.17) | 0.17 | (0.12,0.21) | 0.16 | (0.12,0.20) |
| South Boston | Dever | 0.00 | (0.00,0.01) | 0.05 | (0.02,0.08) | 0.04 | (0.02,0.07) |
| South Boston | Dudley | | | 0.03 | (0.01,0.05) | 0.07 | (0.04,0.10) |
| South Boston | E Greenwood | 0.01 | (0.00,0.03) | | | | |
| South Boston | Eliot | 0.01 | (0.00,0.03) | 0.01 | (0.00,0.03) | 0.01 | (0.00,0.03) |
| South Boston | Everett | | | 0.02 | (0.00,0.04) | 0.01 | (0.00,0.03) |
| South Boston | Harvard/Kent | 0.02 | (0.01,0.03) | 0.01 | (0.00,0.02) | 0.01 | (0.00,0.02) |
| South Boston | Haynes | | | 0.01 | (0.00,0.03) | 0.01 | (0.00,0.03) |
| South Boston | Hernandez | | | 0.02 | (0.00,0.04) | 0.01 | (0.00,0.03) |
| South Boston | Holland | 0.01 | (0.00,0.02) | | | | |
| South Boston | Hurley | 0.04 | (0.02,0.07) | 0.03 | (0.01,0.05) | 0.03 | (0.01,0.05) |
| South Boston | Jackson/Mann | | | 0.01 | (0.00,0.03) | 0.01 | (0.00,0.03) |
| South Boston | Mason | 0.31 | (0.24,0.37) | 0.04 | (0.02,0.07) | 0.04 | (0.01,0.06) |
| South Boston | Mather | | | 0.00 | (0.00,0.01) | 0.00 | (0.00,0.01) |
| South Boston | Mission Hill | 0.00 | (0.00,0.01) | | | | |
| South Boston | Murphy | 0.01 | (0.00,0.02) | 0.01 | (0.00,0.02) | 0.01 | (0.00,0.02) |
| South Boston | Orchard Gardens | 0.02 | (0.01,0.04) | 0.04 | (0.02,0.06) | 0.04 | (0.02,0.07) |
| South Boston | Perkins | 0.01 | (0.00,0.03) | 0.06 | (0.03,0.09) | 0.06 | (0.03,0.09) |
| South Boston | Perry | 0.06 | (0.04,0.07) | 0.16 | (0.12,0.19) | 0.15 | (0.12,0.19) |
| South Boston | Quincy | 0.22 | (0.18,0.26) | 0.09 | (0.06,0.13) | 0.10 | (0.07,0.14) |
| South Boston | Roosevelt | 0.01 | (0.00,0.02) | | | | |
| South Boston | Russell | 0.03 | (0.01,0.04) | 0.04 | (0.02,0.07) | 0.03 | (0.01,0.05) |
| South Boston | S. Greenwood | 0.01 | (0.00,0.01) | | | | |
| South Boston | Taylor | 0.00 | (0.00,0.01) | | | | |
| South Boston | Tynan | 0.01 | (0.00,0.03) | 0.07 | (0.04,0.10) | 0.07 | (0.04,0.10) |
| South Boston | UP Acad. Dor. | 0.03 | (0.01,0.04) | 0.02 | (0.01,0.04) | 0.03 | (0.01,0.05) |
| South Boston | Winthrop | 0.02 | (0.00,0.04) | 0.01 | (0.00,0.02) | 0.01 | (0.00,0.02) |
| South Dorchester | Channing | 0.01 | (0.00,0.01) | | | | |
| South Dorchester | Clap | | | 0.01 | (0.00,0.01) | 0.01 | (0.00,0.01) |
| South Dorchester | Condon | 0.03 | (0.02,0.04) | 0.02 | (0.01,0.03) | 0.02 | (0.01,0.02) |
| South Dorchester | Dever | 0.01 | (0.01,0.01) | 0.01 | (0.00,0.01) | | |
| South Dorchester | Dudley | 0.01 | (0.01,0.01) | 0.03 | (0.02,0.05) | 0.07 | (0.05,0.08) |
| South Dorchester | Ellison/Parks | | | 0.02 | (0.01,0.03) | 0.02 | (0.01,0.03) |
| South Dorchester | Everett | 0.01 | (0.00,0.01) | 0.03 | (0.02,0.04) | 0.02 | (0.01,0.03) |
| South Dorchester | Haynes | | | 0.02 | (0.01,0.03) | 0.02 | (0.01,0.02) |
| South Dorchester | Henderson | 0.31 | (0.29,0.32) | 0.09 | (0.07,0.11) | 0.08 | (0.06,0.10) |
| South Dorchester | Hernandez | 0.01 | (0.00,0.01) | 0.04 | (0.03,0.05) | 0.04 | (0.03,0.05) |
| South Dorchester | Holland | 0.06 | (0.05,0.07) | 0.07 | (0.05,0.08) | 0.06 | (0.05,0.07) |
| South Dorchester | Holmes | 0.02 | (0.01,0.02) | 0.04 | (0.03,0.05) | 0.03 | (0.02,0.04) |
| South Dorchester | Jackson/Mann | | | 0.01 | (0.00,0.02) | 0.01 | (0.01,0.02) |
| South Dorchester | Kenny | 0.02 | (0.02,0.03) | 0.05 | (0.04,0.06) | 0.04 | (0.03,0.06) |
| South Dorchester | King | | | 0.01 | (0.01,0.02) | 0.01 | (0.01,0.02) |
| South Dorchester | Lee | 0.01 | (0.00,0.01) | 0.03 | (0.01,0.06) | 0.03 | (0.01,0.05) |
| South Dorchester | Mason | 0.02 | (0.01,0.02) | | | | |
| South Dorchester | Mather | 0.08 | (0.07,0.09) | 0.08 | (0.07,0.10) | 0.07 | (0.06,0.09) |
| South Dorchester | Mattahunt | 0.01 | (0.00,0.01) | | | | |
| South Dorchester | Murphy | 0.24 | (0.22,0.26) | 0.20 | (0.18,0.22) | 0.20 | (0.18,0.23) |
| South Dorchester | Orchard Gardens | 0.01 | (0.00,0.01) | | | | |

Continued on next page

**Table 8 – continued from previous page**

| | | Naive | | Logit | | Mixed Logit | |
|---|---|---|---|---|---|---|---|
| Neighborhood | School | mean | (95% C.I.) | mean | (95% C.I.) | mean | (95% C.I.) |
| South Dorchester | Russell | 0.02 | (0.01,0.02) | 0.02 | (0.01,0.02) | 0.02 | (0.01,0.02) |
| South Dorchester | S. Greenwood | 0.04 | (0.03,0.05) | 0.06 | (0.04,0.07) | 0.05 | (0.04,0.06) |
| South Dorchester | Taylor | 0.01 | (0.00,0.01) | 0.02 | (0.01,0.03) | 0.02 | (0.01,0.03) |
| South Dorchester | Tynan | 0.01 | (0.00,0.01) | | | | |
| South Dorchester | UP Acad. Dor. | 0.03 | (0.02,0.04) | 0.06 | (0.04,0.07) | 0.10 | (0.08,0.12) |
| South Dorchester | Young Achievers | 0.01 | (0.01,0.02) | 0.02 | (0.01,0.03) | 0.02 | (0.01,0.03) |
| South End | Blackstone | 0.06 | (0.04,0.08) | 0.12 | (0.09,0.15) | 0.11 | (0.08,0.14) |
| South End | Clap | | | 0.00 | (0.00,0.01) | 0.01 | (0.00,0.01) |
| South End | Condon | 0.03 | (0.02,0.05) | 0.04 | (0.02,0.06) | 0.04 | (0.02,0.06) |
| South End | Dever | | | 0.00 | (0.00,0.01) | 0.00 | (0.00,0.01) |
| South End | Dudley | | | 0.03 | (0.01,0.05) | 0.08 | (0.06,0.11) |
| South End | Edison | 0.02 | (0.01,0.03) | 0.01 | (0.00,0.02) | 0.01 | (0.00,0.01) |
| South End | Eliot | 0.03 | (0.01,0.04) | 0.02 | (0.01,0.04) | 0.02 | (0.01,0.04) |
| South End | Hale | 0.04 | (0.03,0.06) | 0.02 | (0.01,0.03) | 0.02 | (0.01,0.03) |
| South End | Harvard/Kent | 0.02 | (0.01,0.02) | 0.01 | (0.00,0.01) | 0.01 | (0.00,0.01) |
| South End | Haynes | | | 0.01 | (0.00,0.02) | 0.01 | (0.00,0.02) |
| South End | Hennigan | 0.01 | (0.01,0.02) | 0.01 | (0.00,0.02) | 0.01 | (0.00,0.02) |
| South End | Hernandez | | | 0.03 | (0.02,0.05) | 0.03 | (0.01,0.04) |
| South End | Higginson/Lewis | | | 0.01 | (0.00,0.02) | 0.01 | (0.00,0.02) |
| South End | Hurley | 0.32 | (0.29,0.35) | 0.16 | (0.13,0.19) | 0.16 | (0.12,0.19) |
| South End | J.F. Kennedy | 0.01 | (0.00,0.02) | 0.00 | (0.00,0.01) | | |
| South End | Jackson/Mann | 0.04 | (0.03,0.06) | 0.03 | (0.01,0.05) | 0.03 | (0.01,0.04) |
| South End | Mario Umana | 0.01 | (0.00,0.01) | | | | |
| South End | Mason | 0.05 | (0.03,0.07) | 0.06 | (0.04,0.09) | 0.05 | (0.03,0.07) |
| South End | Orchard Gardens | 0.04 | (0.03,0.06) | 0.11 | (0.09,0.14) | 0.10 | (0.08,0.13) |
| South End | Perkins | | | 0.01 | (0.00,0.02) | 0.01 | (0.00,0.02) |
| South End | Quincy | 0.22 | (0.19,0.26) | 0.20 | (0.16,0.23) | 0.20 | (0.16,0.24) |
| South End | Russell | 0.01 | (0.00,0.02) | | | | |
| South End | Tobin | 0.01 | (0.00,0.02) | 0.03 | (0.02,0.05) | 0.03 | (0.01,0.04) |
| South End | Tynan | | | 0.00 | (0.00,0.01) | 0.00 | (0.00,0.01) |
| South End | UP Acad. Dor. | | | 0.01 | (0.00,0.03) | 0.02 | (0.01,0.04) |
| South End | Warren/Prescott | 0.01 | (0.00,0.02) | | | | |
| South End | West Zone ELC | | | 0.01 | (0.00,0.02) | 0.01 | (0.00,0.02) |
| South End | Winship | | | 0.00 | (0.00,0.01) | 0.00 | (0.00,0.01) |
| South End | Winthrop | 0.02 | (0.01,0.03) | 0.02 | (0.01,0.03) | 0.01 | (0.01,0.02) |
| West Roxbury | BTU | 0.01 | (0.00,0.01) | 0.01 | (0.00,0.02) | 0.01 | (0.00,0.02) |
| West Roxbury | Bates | | | 0.04 | (0.02,0.06) | 0.03 | (0.02,0.05) |
| West Roxbury | Beethoven | 0.13 | (0.11,0.15) | 0.23 | (0.20,0.26) | 0.22 | (0.19,0.26) |
| West Roxbury | Channing | | | 0.03 | (0.02,0.05) | 0.03 | (0.02,0.04) |
| West Roxbury | Conley | 0.02 | (0.01,0.03) | 0.02 | (0.00,0.03) | 0.01 | (0.00,0.03) |
| West Roxbury | Dudley | | | | | 0.01 | (0.00,0.03) |
| West Roxbury | E Greenwood | | | 0.01 | (0.01,0.03) | 0.01 | (0.00,0.03) |
| West Roxbury | Ellis | 0.01 | (0.00,0.01) | | | | |
| West Roxbury | Ellison/Parks | | | 0.01 | (0.00,0.01) | 0.01 | (0.00,0.01) |
| West Roxbury | Grew | | | 0.02 | (0.01,0.03) | 0.02 | (0.01,0.03) |
| West Roxbury | Hale | 0.01 | (0.00,0.01) | | | | |
| West Roxbury | Hernandez | | | 0.01 | (0.00,0.02) | 0.01 | (0.00,0.02) |
| West Roxbury | J.F. Kennedy | 0.01 | (0.00,0.01) | 0.01 | (0.00,0.01) | | |
| West Roxbury | Kilmer | 0.31 | (0.28,0.33) | 0.25 | (0.22,0.28) | 0.26 | (0.23,0.29) |
| West Roxbury | Lyndon | 0.33 | (0.30,0.35) | 0.22 | (0.19,0.26) | 0.22 | (0.19,0.25) |
| West Roxbury | Manning | 0.01 | (0.01,0.02) | 0.01 | (0.01,0.02) | 0.01 | (0.00,0.02) |
| West Roxbury | Mozart | 0.02 | (0.02,0.03) | 0.07 | (0.05,0.10) | 0.07 | (0.05,0.09) |
| West Roxbury | Roosevelt | 0.02 | (0.01,0.04) | 0.01 | (0.00,0.02) | 0.02 | (0.01,0.03) |
| West Roxbury | Sumner | 0.07 | (0.05,0.09) | 0.02 | (0.01,0.03) | 0.02 | (0.01,0.03) |
| West Roxbury | UP Acad. Dor. | 0.01 | (0.00,0.02) | | | 0.01 | (0.00,0.02) |

Continued on next page

**Table 8 – continued from previous page**

| Neighborhood | School | Naive mean | Naive (95% C.I.) | Logit mean | Logit (95% C.I.) | Mixed Logit mean | Mixed Logit (95% C.I.) |
|---|---|---|---|---|---|---|---|
| West Roxbury | West Zone ELC | 0.01 | (0.00,0.01) | | | | |

Table 9: Top 3 Choices Market Share Predictions for 2014 K2

| Neighborhood | School | Naive mean | Naive (95% C.I.) | Logit mean | Logit (95% C.I.) | Mixed Logit mean | Mixed Logit (95% C.I.) |
|---|---|---|---|---|---|---|---|
| Allston-Brighton | Baldwin | 0.05 | (0.04,0.06) | 0.15 | (0.13,0.18) | 0.15 | (0.12,0.17) |
| Allston-Brighton | Curley | | | 0.01 | (0.00,0.02) | 0.01 | (0.00,0.02) |
| Allston-Brighton | Dudley | | | | | 0.01 | (0.00,0.02) |
| Allston-Brighton | Edison | 0.15 | (0.12,0.17) | 0.12 | (0.09,0.14) | 0.11 | (0.08,0.13) |
| Allston-Brighton | Gardner | 0.06 | (0.04,0.07) | 0.15 | (0.12,0.18) | 0.16 | (0.13,0.19) |
| Allston-Brighton | Hale | 0.04 | (0.03,0.05) | | | | |
| Allston-Brighton | Hennigan | | | 0.01 | (0.00,0.02) | 0.01 | (0.00,0.02) |
| Allston-Brighton | Hernandez | 0.03 | (0.02,0.04) | 0.01 | (0.00,0.02) | 0.01 | (0.01,0.02) |
| Allston-Brighton | Hurley | 0.03 | (0.01,0.04) | | | | |
| Allston-Brighton | Jackson/Mann | 0.24 | (0.21,0.27) | 0.18 | (0.15,0.21) | 0.17 | (0.14,0.20) |
| Allston-Brighton | Lyon K-8 | 0.18 | (0.16,0.20) | 0.13 | (0.10,0.16) | 0.14 | (0.12,0.17) |
| Allston-Brighton | Manning | 0.10 | (0.08,0.12) | 0.00 | (0.00,0.01) | 0.00 | (0.00,0.01) |
| Allston-Brighton | Mendell | | | 0.01 | (0.00,0.01) | 0.00 | (0.00,0.01) |
| Allston-Brighton | Quincy | 0.03 | (0.02,0.04) | 0.01 | (0.00,0.02) | 0.01 | (0.00,0.02) |
| Allston-Brighton | Tobin | | | 0.01 | (0.00,0.01) | 0.01 | (0.00,0.01) |
| Allston-Brighton | UP Acad. Dor. | | | | | 0.01 | (0.00,0.02) |
| Allston-Brighton | Winship | 0.08 | (0.06,0.10) | 0.19 | (0.15,0.22) | 0.18 | (0.15,0.21) |
| Charlestown | Adams | 0.02 | (0.01,0.03) | | | | |
| Charlestown | Blackstone | | | 0.02 | (0.01,0.03) | 0.02 | (0.01,0.03) |
| Charlestown | Dudley | | | 0.01 | (0.00,0.02) | 0.02 | (0.01,0.04) |
| Charlestown | East Boston EEC | | | 0.03 | (0.01,0.04) | 0.03 | (0.02,0.05) |
| Charlestown | Eliot | 0.29 | (0.27,0.31) | 0.35 | (0.31,0.39) | 0.35 | (0.31,0.39) |
| Charlestown | Harvard/Kent | 0.31 | (0.30,0.33) | 0.20 | (0.17,0.23) | 0.20 | (0.16,0.22) |
| Charlestown | Hernandez | | | 0.01 | (0.00,0.01) | 0.01 | (0.00,0.01) |
| Charlestown | Hurley | 0.01 | (0.00,0.01) | | | | |
| Charlestown | Kennedy Patrick | 0.00 | (0.00,0.01) | | | | |
| Charlestown | Mario Umana | 0.01 | (0.00,0.02) | 0.02 | (0.01,0.04) | 0.02 | (0.01,0.03) |
| Charlestown | O'Donnell | | | 0.03 | (0.01,0.04) | 0.02 | (0.01,0.03) |
| Charlestown | Orchard Gardens | 0.00 | (0.00,0.01) | | | | |
| Charlestown | Otis | 0.02 | (0.01,0.04) | 0.01 | (0.00,0.02) | 0.01 | (0.00,0.02) |
| Charlestown | Perkins | | | 0.01 | (0.00,0.02) | 0.01 | (0.00,0.01) |
| Charlestown | Quincy | | | 0.06 | (0.03,0.08) | 0.05 | (0.03,0.08) |
| Charlestown | Tynan | | | 0.01 | (0.00,0.02) | 0.01 | (0.00,0.02) |
| Charlestown | UP Acad. Dor. | | | | | 0.01 | (0.00,0.02) |
| Charlestown | Warren/Prescott | 0.29 | (0.28,0.30) | 0.23 | (0.20,0.26) | 0.23 | (0.20,0.26) |
| Downtown | Blackstone | | | 0.03 | (0.02,0.05) | 0.03 | (0.02,0.05) |
| Downtown | Condon | | | 0.02 | (0.01,0.03) | 0.02 | (0.01,0.03) |
| Downtown | Dudley | | | 0.01 | (0.00,0.02) | 0.03 | (0.02,0.05) |
| Downtown | East Boston EEC | | | | | 0.01 | (0.00,0.02) |
| Downtown | Edison | 0.06 | (0.04,0.09) | 0.01 | (0.00,0.02) | 0.01 | (0.00,0.02) |
| Downtown | Eliot | 0.28 | (0.23,0.33) | 0.30 | (0.25,0.34) | 0.31 | (0.27,0.35) |
| Downtown | Hale | 0.02 | (0.01,0.04) | 0.01 | (0.00,0.01) | 0.00 | (0.00,0.01) |
| Downtown | Harvard/Kent | 0.07 | (0.05,0.09) | 0.05 | (0.04,0.07) | 0.05 | (0.03,0.07) |
| Downtown | Hennigan | 0.01 | (0.00,0.01) | 0.01 | (0.00,0.02) | 0.01 | (0.00,0.02) |
| Downtown | Hernandez | | | 0.01 | (0.00,0.03) | 0.01 | (0.00,0.02) |
| Downtown | Hurley | 0.09 | (0.06,0.11) | 0.06 | (0.04,0.08) | 0.06 | (0.04,0.08) |

Continued on next page

**Table 9 – continued from previous page**

| Neighborhood | School | Naive | | Logit | | Mixed Logit | |
|---|---|---|---|---|---|---|---|
| | | mean | (95% C.I.) | mean | (95% C.I.) | mean | (95% C.I.) |
| Downtown | Jackson/Mann | 0.12 | (0.09,0.15) | 0.03 | (0.01,0.04) | 0.02 | (0.01,0.04) |
| Downtown | Mason | 0.03 | (0.01,0.04) | 0.02 | (0.00,0.03) | 0.01 | (0.00,0.03) |
| Downtown | Orchard Gardens | 0.02 | (0.01,0.03) | 0.04 | (0.02,0.05) | 0.03 | (0.02,0.05) |
| Downtown | Perkins | | | 0.01 | (0.00,0.02) | 0.01 | (0.00,0.02) |
| Downtown | Quincy | 0.26 | (0.23,0.29) | 0.26 | (0.23,0.30) | 0.26 | (0.23,0.30) |
| Downtown | Tobin | 0.01 | (0.00,0.01) | 0.02 | (0.01,0.03) | 0.01 | (0.01,0.03) |
| Downtown | Tynan | | | 0.01 | (0.00,0.02) | 0.01 | (0.00,0.02) |
| Downtown | UP Acad. Dor. | | | 0.01 | (0.00,0.02) | 0.01 | (0.00,0.02) |
| Downtown | Warren/Prescott | 0.01 | (0.00,0.02) | 0.05 | (0.03,0.07) | 0.04 | (0.03,0.06) |
| Downtown | West Zone ELC | | | 0.01 | (0.00,0.02) | 0.01 | (0.00,0.02) |
| Downtown | Winship | | | 0.01 | (0.00,0.02) | 0.01 | (0.00,0.02) |
| Downtown | Winthrop | 0.01 | (0.00,0.01) | | | | |
| East Boston | Adams | 0.06 | (0.05,0.07) | 0.05 | (0.04,0.07) | 0.04 | (0.04,0.06) |
| East Boston | Blackstone | 0.02 | (0.01,0.03) | 0.01 | (0.01,0.01) | 0.01 | (0.01,0.01) |
| East Boston | Bradley | 0.15 | (0.14,0.16) | 0.07 | (0.06,0.08) | 0.07 | (0.06,0.09) |
| East Boston | Dudley | | | | | 0.01 | (0.01,0.02) |
| East Boston | East Boston EEC | 0.04 | (0.03,0.05) | 0.13 | (0.12,0.15) | 0.13 | (0.11,0.15) |
| East Boston | Eliot | 0.02 | (0.02,0.03) | 0.01 | (0.00,0.01) | 0.01 | (0.00,0.01) |
| East Boston | Guild | 0.12 | (0.10,0.13) | 0.07 | (0.05,0.08) | 0.07 | (0.05,0.08) |
| East Boston | Harvard/Kent | 0.05 | (0.04,0.06) | 0.01 | (0.00,0.01) | 0.01 | (0.00,0.01) |
| East Boston | Hernandez | | | | | 0.01 | (0.01,0.02) |
| East Boston | Kennedy Patrick | 0.13 | (0.12,0.14) | 0.17 | (0.15,0.19) | 0.16 | (0.15,0.18) |
| East Boston | Mario Umana | 0.12 | (0.11,0.14) | 0.11 | (0.09,0.13) | 0.11 | (0.09,0.13) |
| East Boston | McKay | 0.02 | (0.02,0.04) | 0.14 | (0.12,0.16) | 0.13 | (0.11,0.15) |
| East Boston | O'Donnell | 0.03 | (0.03,0.04) | 0.15 | (0.13,0.17) | 0.14 | (0.12,0.16) |
| East Boston | Otis | 0.18 | (0.17,0.19) | 0.08 | (0.06,0.09) | 0.07 | (0.06,0.09) |
| East Boston | UP Acad. Dor. | | | | | 0.01 | (0.00,0.01) |
| East Boston | Winthrop | 0.01 | (0.01,0.01) | | | | |
| Hyde Park | Bates | | | 0.05 | (0.04,0.07) | 0.05 | (0.03,0.06) |
| Hyde Park | Beethoven | 0.01 | (0.01,0.02) | 0.08 | (0.06,0.10) | 0.07 | (0.06,0.09) |
| Hyde Park | Channing | 0.02 | (0.01,0.02) | 0.07 | (0.06,0.09) | 0.07 | (0.06,0.09) |
| Hyde Park | Chittick | 0.03 | (0.02,0.03) | 0.05 | (0.03,0.06) | 0.04 | (0.03,0.06) |
| Hyde Park | Condon | 0.01 | (0.00,0.01) | | | | |
| Hyde Park | Conley | 0.25 | (0.24,0.26) | 0.06 | (0.05,0.08) | 0.06 | (0.04,0.08) |
| Hyde Park | Dudley | | | 0.01 | (0.00,0.02) | 0.03 | (0.02,0.04) |
| Hyde Park | E Greenwood | 0.05 | (0.04,0.07) | 0.12 | (0.09,0.15) | 0.12 | (0.10,0.14) |
| Hyde Park | Ellison/Parks | | | 0.05 | (0.04,0.07) | 0.05 | (0.03,0.06) |
| Hyde Park | Grew | 0.01 | (0.01,0.02) | 0.06 | (0.04,0.08) | 0.07 | (0.05,0.09) |
| Hyde Park | Haley | | | 0.04 | (0.02,0.05) | 0.04 | (0.03,0.05) |
| Hyde Park | Hernandez | 0.02 | (0.01,0.03) | 0.03 | (0.02,0.04) | 0.02 | (0.01,0.04) |
| Hyde Park | Kilmer | 0.06 | (0.04,0.07) | 0.03 | (0.02,0.04) | 0.04 | (0.02,0.05) |
| Hyde Park | Mattahunt | 0.03 | (0.02,0.04) | 0.03 | (0.02,0.04) | 0.03 | (0.02,0.04) |
| Hyde Park | Mozart | | | 0.04 | (0.03,0.05) | 0.03 | (0.02,0.05) |
| Hyde Park | Philbrick | 0.15 | (0.13,0.16) | 0.04 | (0.02,0.05) | 0.03 | (0.02,0.04) |
| Hyde Park | Roosevelt | 0.15 | (0.14,0.17) | 0.14 | (0.12,0.16) | 0.14 | (0.12,0.16) |
| Hyde Park | S. Greenwood | 0.01 | (0.01,0.01) | 0.01 | (0.00,0.01) | | |
| Hyde Park | Sumner | 0.07 | (0.06,0.09) | 0.02 | (0.01,0.03) | 0.02 | (0.01,0.03) |
| Hyde Park | Taylor | 0.01 | (0.01,0.02) | 0.01 | (0.01,0.02) | 0.01 | (0.00,0.02) |
| Hyde Park | UP Acad. Dor. | 0.04 | (0.03,0.05) | 0.02 | (0.01,0.03) | 0.03 | (0.01,0.04) |
| Hyde Park | Young Achievers | 0.03 | (0.03,0.04) | 0.02 | (0.01,0.03) | 0.02 | (0.01,0.03) |
| Jamaica Plain | BTU | 0.01 | (0.01,0.01) | 0.05 | (0.04,0.07) | 0.05 | (0.03,0.06) |
| Jamaica Plain | Curley | 0.09 | (0.07,0.10) | 0.13 | (0.11,0.15) | 0.13 | (0.11,0.15) |
| Jamaica Plain | Dudley | | | 0.02 | (0.01,0.03) | 0.05 | (0.03,0.06) |
| Jamaica Plain | Edison | 0.01 | (0.00,0.01) | | | | |
| Jamaica Plain | Ellis | 0.02 | (0.01,0.03) | 0.02 | (0.02,0.04) | 0.02 | (0.01,0.03) |

Continued on next page

**Table 9 – continued from previous page**

| Neighborhood | School | Naive mean | Naive (95% C.I.) | Logit mean | Logit (95% C.I.) | Mixed Logit mean | Mixed Logit (95% C.I.) |
|---|---|---|---|---|---|---|---|
| Jamaica Plain | Hale | 0.20 | (0.18,0.21) | 0.03 | (0.02,0.04) | 0.02 | (0.01,0.03) |
| Jamaica Plain | Haley | | | 0.01 | (0.00,0.02) | 0.01 | (0.00,0.02) |
| Jamaica Plain | Hennigan | 0.05 | (0.04,0.06) | 0.10 | (0.07,0.12) | 0.09 | (0.07,0.12) |
| Jamaica Plain | Hernandez | 0.01 | (0.01,0.01) | 0.06 | (0.04,0.08) | 0.07 | (0.06,0.09) |
| Jamaica Plain | Higginson/Lewis | | | 0.01 | (0.00,0.01) | 0.00 | (0.00,0.01) |
| Jamaica Plain | Hurley | 0.08 | (0.07,0.10) | 0.03 | (0.01,0.04) | 0.03 | (0.01,0.04) |
| Jamaica Plain | J.F. Kennedy | 0.08 | (0.06,0.09) | 0.08 | (0.07,0.10) | 0.08 | (0.06,0.09) |
| Jamaica Plain | Jackson/Mann | 0.01 | (0.00,0.01) | 0.03 | (0.02,0.05) | 0.03 | (0.02,0.04) |
| Jamaica Plain | Lyndon | 0.01 | (0.00,0.01) | | | | |
| Jamaica Plain | Manning | 0.15 | (0.13,0.16) | 0.05 | (0.04,0.07) | 0.05 | (0.03,0.06) |
| Jamaica Plain | Mason | 0.06 | (0.04,0.08) | 0.01 | (0.00,0.01) | 0.01 | (0.00,0.01) |
| Jamaica Plain | Mendell | 0.03 | (0.03,0.04) | 0.07 | (0.06,0.09) | 0.07 | (0.05,0.08) |
| Jamaica Plain | Mission Hill | 0.04 | (0.02,0.05) | 0.09 | (0.07,0.11) | 0.09 | (0.07,0.11) |
| Jamaica Plain | Murphy | 0.01 | (0.00,0.01) | | | | |
| Jamaica Plain | Orchard Gardens | | | 0.03 | (0.01,0.04) | 0.02 | (0.01,0.04) |
| Jamaica Plain | Philbrick | 0.03 | (0.02,0.04) | | | | |
| Jamaica Plain | Quincy | 0.01 | (0.00,0.02) | 0.01 | (0.00,0.02) | 0.01 | (0.00,0.02) |
| Jamaica Plain | Sumner | 0.02 | (0.01,0.03) | | | 0.01 | (0.00,0.01) |
| Jamaica Plain | Tobin | 0.01 | (0.00,0.01) | 0.04 | (0.03,0.06) | 0.04 | (0.03,0.06) |
| Jamaica Plain | Trotter | 0.01 | (0.01,0.01) | 0.02 | (0.01,0.02) | 0.01 | (0.01,0.02) |
| Jamaica Plain | UP Acad. Dor. | 0.03 | (0.03,0.04) | 0.02 | (0.01,0.03) | 0.02 | (0.01,0.04) |
| Jamaica Plain | West Zone ELC | 0.01 | (0.01,0.02) | 0.06 | (0.05,0.08) | 0.06 | (0.04,0.08) |
| Mattapan | BTU | | | 0.04 | (0.03,0.05) | 0.04 | (0.03,0.05) |
| Mattapan | Channing | 0.01 | (0.00,0.01) | 0.01 | (0.00,0.01) | 0.01 | (0.00,0.01) |
| Mattapan | Chittick | 0.01 | (0.01,0.01) | 0.02 | (0.01,0.03) | 0.02 | (0.01,0.03) |
| Mattapan | Conley | 0.07 | (0.05,0.08) | 0.01 | (0.01,0.02) | 0.01 | (0.00,0.02) |
| Mattapan | Dever | 0.02 | (0.02,0.03) | 0.01 | (0.01,0.02) | 0.01 | (0.01,0.02) |
| Mattapan | Dudley | | | 0.03 | (0.02,0.05) | 0.07 | (0.05,0.09) |
| Mattapan | E Greenwood | 0.01 | (0.01,0.02) | 0.02 | (0.01,0.02) | 0.02 | (0.01,0.03) |
| Mattapan | Ellison/Parks | 0.01 | (0.01,0.02) | 0.11 | (0.09,0.13) | 0.11 | (0.09,0.13) |
| Mattapan | Haley | | | 0.09 | (0.07,0.10) | 0.07 | (0.06,0.09) |
| Mattapan | Henderson | 0.16 | (0.14,0.18) | 0.02 | (0.01,0.04) | 0.03 | (0.02,0.04) |
| Mattapan | Hernandez | 0.02 | (0.01,0.03) | 0.05 | (0.04,0.07) | 0.05 | (0.03,0.06) |
| Mattapan | Holland | 0.02 | (0.02,0.03) | 0.02 | (0.01,0.02) | 0.02 | (0.01,0.02) |
| Mattapan | Holmes | 0.01 | (0.01,0.01) | 0.02 | (0.01,0.03) | 0.01 | (0.01,0.02) |
| Mattapan | Jackson/Mann | | | 0.01 | (0.00,0.02) | 0.01 | (0.01,0.02) |
| Mattapan | Kenny | 0.02 | (0.01,0.03) | 0.02 | (0.01,0.03) | 0.02 | (0.01,0.03) |
| Mattapan | Lee | 0.01 | (0.00,0.01) | 0.04 | (0.01,0.06) | 0.03 | (0.01,0.05) |
| Mattapan | Mattahunt | 0.02 | (0.01,0.03) | 0.04 | (0.03,0.05) | 0.04 | (0.03,0.05) |
| Mattapan | Murphy | 0.07 | (0.05,0.08) | 0.03 | (0.02,0.04) | 0.03 | (0.02,0.04) |
| Mattapan | Philbrick | 0.20 | (0.18,0.21) | 0.03 | (0.02,0.05) | 0.03 | (0.02,0.04) |
| Mattapan | Russell | 0.01 | (0.01,0.02) | 0.01 | (0.00,0.01) | 0.01 | (0.00,0.01) |
| Mattapan | S. Greenwood | 0.08 | (0.06,0.09) | 0.06 | (0.04,0.07) | 0.05 | (0.04,0.07) |
| Mattapan | Sumner | 0.04 | (0.03,0.05) | 0.01 | (0.00,0.01) | 0.01 | (0.00,0.01) |
| Mattapan | Taylor | 0.12 | (0.10,0.14) | 0.06 | (0.05,0.08) | 0.06 | (0.04,0.07) |
| Mattapan | UP Acad. Dor. | 0.02 | (0.01,0.02) | 0.05 | (0.03,0.06) | 0.07 | (0.05,0.09) |
| Mattapan | Young Achievers | 0.02 | (0.01,0.03) | 0.14 | (0.12,0.16) | 0.14 | (0.12,0.16) |
| North Dorchester | Blackstone | | | 0.01 | (0.00,0.01) | 0.00 | (0.00,0.01) |
| North Dorchester | Clap | | | 0.07 | (0.05,0.09) | 0.07 | (0.05,0.09) |
| North Dorchester | Condon | 0.10 | (0.09,0.12) | 0.05 | (0.03,0.07) | 0.05 | (0.03,0.06) |
| North Dorchester | Dever | 0.02 | (0.01,0.03) | 0.06 | (0.05,0.09) | 0.06 | (0.04,0.07) |
| North Dorchester | Dudley | 0.01 | (0.01,0.02) | 0.05 | (0.04,0.07) | 0.10 | (0.08,0.12) |
| North Dorchester | Ellison/Parks | 0.01 | (0.00,0.01) | | | | |
| North Dorchester | Everett | | | 0.09 | (0.07,0.12) | 0.09 | (0.07,0.11) |
| North Dorchester | Hale | 0.02 | (0.01,0.03) | | | | |

Continued on next page

**Table 9 – continued from previous page**

| Neighborhood | School | Naive mean | Naive (95% C.I.) | Logit mean | Logit (95% C.I.) | Mixed Logit mean | Mixed Logit (95% C.I.) |
|---|---|---|---|---|---|---|---|
| North Dorchester | Haynes | 0.02 | (0.01,0.03) | 0.05 | (0.03,0.07) | 0.04 | (0.03,0.06) |
| North Dorchester | Henderson | 0.07 | (0.05,0.09) | 0.02 | (0.01,0.04) | 0.02 | (0.01,0.04) |
| North Dorchester | Hernandez | | | 0.03 | (0.02,0.05) | 0.03 | (0.01,0.04) |
| North Dorchester | Holland | 0.02 | (0.01,0.03) | 0.04 | (0.03,0.05) | 0.03 | (0.02,0.04) |
| North Dorchester | Hurley | 0.01 | (0.00,0.02) | 0.01 | (0.00,0.01) | 0.01 | (0.00,0.01) |
| North Dorchester | Jackson/Mann | | | 0.01 | (0.01,0.02) | 0.02 | (0.01,0.03) |
| North Dorchester | King | 0.01 | (0.00,0.01) | 0.02 | (0.01,0.03) | 0.01 | (0.01,0.02) |
| North Dorchester | Mason | 0.35 | (0.31,0.40) | 0.07 | (0.05,0.09) | 0.06 | (0.04,0.09) |
| North Dorchester | Mather | 0.03 | (0.02,0.04) | 0.08 | (0.06,0.10) | 0.07 | (0.06,0.09) |
| North Dorchester | Murphy | 0.04 | (0.03,0.06) | 0.03 | (0.02,0.04) | 0.03 | (0.02,0.04) |
| North Dorchester | Orchard Gardens | 0.05 | (0.03,0.06) | 0.06 | (0.04,0.07) | 0.05 | (0.04,0.07) |
| North Dorchester | Perkins | | | 0.02 | (0.01,0.03) | 0.01 | (0.01,0.02) |
| North Dorchester | Perry | | | 0.01 | (0.00,0.02) | 0.01 | (0.00,0.02) |
| North Dorchester | Russell | 0.05 | (0.03,0.06) | 0.09 | (0.07,0.11) | 0.09 | (0.07,0.11) |
| North Dorchester | S. Greenwood | 0.01 | (0.01,0.02) | 0.01 | (0.00,0.01) | 0.01 | (0.00,0.01) |
| North Dorchester | Trotter | | | 0.00 | (0.00,0.01) | | |
| North Dorchester | Tynan | | | 0.01 | (0.00,0.01) | 0.01 | (0.00,0.01) |
| North Dorchester | UP Acad. Dor. | 0.03 | (0.02,0.04) | 0.04 | (0.03,0.06) | 0.07 | (0.04,0.09) |
| North Dorchester | Winthrop | 0.07 | (0.06,0.09) | 0.05 | (0.04,0.07) | 0.04 | (0.03,0.06) |
| Roslindale | BTU | 0.01 | (0.01,0.01) | 0.11 | (0.09,0.13) | 0.11 | (0.09,0.13) |
| Roslindale | Bates | 0.01 | (0.00,0.01) | 0.09 | (0.08,0.11) | 0.09 | (0.07,0.11) |
| Roslindale | Beethoven | 0.03 | (0.03,0.04) | 0.04 | (0.03,0.05) | 0.04 | (0.03,0.05) |
| Roslindale | Chittick | | | 0.01 | (0.00,0.01) | | |
| Roslindale | Conley | 0.16 | (0.14,0.18) | 0.07 | (0.05,0.09) | 0.06 | (0.04,0.08) |
| Roslindale | Curley | 0.02 | (0.01,0.02) | 0.01 | (0.01,0.02) | 0.01 | (0.01,0.02) |
| Roslindale | Dudley | | | 0.01 | (0.00,0.01) | 0.03 | (0.02,0.04) |
| Roslindale | E Greenwood | 0.02 | (0.01,0.03) | 0.05 | (0.03,0.06) | 0.04 | (0.03,0.06) |
| Roslindale | Ellis | 0.01 | (0.00,0.01) | | | | |
| Roslindale | Ellison/Parks | | | 0.02 | (0.01,0.03) | 0.02 | (0.01,0.03) |
| Roslindale | Grew | | | 0.01 | (0.00,0.01) | 0.01 | (0.00,0.01) |
| Roslindale | Haley | 0.01 | (0.01,0.02) | 0.07 | (0.05,0.08) | 0.07 | (0.06,0.09) |
| Roslindale | Hennigan | 0.01 | (0.00,0.01) | | | | |
| Roslindale | Hernandez | 0.02 | (0.01,0.03) | 0.04 | (0.03,0.05) | 0.04 | (0.03,0.05) |
| Roslindale | Jackson/Mann | 0.00 | (0.00,0.01) | | | | |
| Roslindale | Kilmer | 0.01 | (0.01,0.01) | 0.01 | (0.01,0.02) | 0.01 | (0.01,0.02) |
| Roslindale | King | 0.01 | (0.00,0.01) | | | | |
| Roslindale | Lyndon | 0.06 | (0.04,0.07) | 0.06 | (0.05,0.07) | 0.06 | (0.04,0.07) |
| Roslindale | Manning | 0.04 | (0.03,0.06) | 0.02 | (0.01,0.03) | 0.02 | (0.01,0.03) |
| Roslindale | Mattahunt | | | 0.02 | (0.01,0.02) | 0.02 | (0.01,0.03) |
| Roslindale | Mendell | | | 0.01 | (0.00,0.01) | 0.01 | (0.00,0.01) |
| Roslindale | Mission Hill | | | 0.02 | (0.01,0.03) | 0.02 | (0.01,0.03) |
| Roslindale | Mozart | 0.01 | (0.01,0.02) | 0.08 | (0.07,0.10) | 0.09 | (0.07,0.10) |
| Roslindale | Philbrick | 0.18 | (0.16,0.19) | 0.08 | (0.07,0.10) | 0.07 | (0.06,0.09) |
| Roslindale | Sumner | 0.29 | (0.28,0.30) | 0.09 | (0.07,0.11) | 0.09 | (0.07,0.11) |
| Roslindale | Trotter | 0.01 | (0.01,0.01) | 0.01 | (0.00,0.01) | 0.01 | (0.00,0.01) |
| Roslindale | UP Acad. Dor. | 0.03 | (0.02,0.04) | 0.01 | (0.01,0.02) | 0.02 | (0.01,0.03) |
| Roslindale | Young Achievers | 0.02 | (0.01,0.02) | 0.02 | (0.01,0.04) | 0.03 | (0.02,0.04) |
| Roxbury | BTU | | | 0.01 | (0.01,0.01) | 0.01 | (0.00,0.01) |
| Roxbury | Blackstone | | | 0.01 | (0.01,0.02) | 0.01 | (0.01,0.02) |
| Roxbury | Clap | | | 0.01 | (0.01,0.02) | 0.01 | (0.01,0.01) |
| Roxbury | Condon | 0.02 | (0.01,0.02) | | | | |
| Roxbury | Curley | 0.02 | (0.02,0.03) | 0.03 | (0.02,0.04) | 0.03 | (0.02,0.04) |
| Roxbury | Dudley | | | 0.05 | (0.04,0.06) | 0.10 | (0.09,0.12) |
| Roxbury | Ellis | 0.02 | (0.02,0.03) | 0.03 | (0.02,0.04) | 0.03 | (0.02,0.04) |
| Roxbury | Everett | | | 0.02 | (0.02,0.03) | 0.02 | (0.01,0.03) |

Continued on next page

**Table 9 – continued from previous page**

| Neighborhood | School | Naive mean | Naive (95% C.I.) | Logit mean | Logit (95% C.I.) | Mixed Logit mean | Mixed Logit (95% C.I.) |
|---|---|---|---|---|---|---|---|
| Roxbury | Hale | 0.17 | (0.16,0.18) | 0.03 | (0.03,0.04) | 0.03 | (0.02,0.04) |
| Roxbury | Haley | | | 0.01 | (0.00,0.01) | 0.01 | (0.00,0.01) |
| Roxbury | Haynes | 0.01 | (0.01,0.01) | 0.05 | (0.04,0.06) | 0.05 | (0.04,0.06) |
| Roxbury | Henderson | 0.05 | (0.04,0.05) | 0.01 | (0.00,0.01) | 0.01 | (0.00,0.01) |
| Roxbury | Hennigan | 0.03 | (0.02,0.03) | 0.03 | (0.02,0.04) | 0.03 | (0.02,0.04) |
| Roxbury | Hernandez | 0.01 | (0.01,0.02) | 0.07 | (0.06,0.08) | 0.08 | (0.06,0.09) |
| Roxbury | Higginson/Lewis | 0.01 | (0.01,0.02) | 0.03 | (0.02,0.04) | 0.02 | (0.02,0.03) |
| Roxbury | Holland | 0.02 | (0.01,0.02) | 0.03 | (0.03,0.04) | 0.03 | (0.02,0.04) |
| Roxbury | Holmes | | | 0.01 | (0.01,0.02) | 0.01 | (0.01,0.01) |
| Roxbury | Hurley | 0.04 | (0.04,0.05) | 0.02 | (0.02,0.03) | 0.02 | (0.01,0.03) |
| Roxbury | J.F. Kennedy | 0.02 | (0.01,0.03) | 0.04 | (0.03,0.05) | 0.03 | (0.03,0.04) |
| Roxbury | Jackson/Mann | 0.01 | (0.00,0.01) | 0.03 | (0.02,0.04) | 0.03 | (0.02,0.04) |
| Roxbury | King | 0.01 | (0.01,0.01) | 0.02 | (0.01,0.03) | 0.02 | (0.01,0.02) |
| Roxbury | Lee | | | 0.01 | (0.00,0.01) | 0.01 | (0.00,0.01) |
| Roxbury | Manning | 0.01 | (0.00,0.01) | | | | |
| Roxbury | Mason | 0.29 | (0.27,0.31) | 0.06 | (0.04,0.07) | 0.05 | (0.04,0.07) |
| Roxbury | Mather | | | 0.02 | (0.01,0.03) | 0.02 | (0.01,0.02) |
| Roxbury | Mendell | | | 0.02 | (0.01,0.03) | 0.02 | (0.01,0.03) |
| Roxbury | Mission Hill | | | 0.02 | (0.01,0.02) | 0.02 | (0.01,0.02) |
| Roxbury | Murphy | 0.02 | (0.01,0.03) | | | | |
| Roxbury | Orchard Gardens | 0.04 | (0.03,0.04) | 0.07 | (0.06,0.08) | 0.06 | (0.05,0.07) |
| Roxbury | Russell | 0.01 | (0.01,0.01) | 0.02 | (0.01,0.03) | 0.02 | (0.01,0.03) |
| Roxbury | S. Greenwood | 0.03 | (0.03,0.04) | 0.03 | (0.02,0.04) | 0.03 | (0.02,0.03) |
| Roxbury | Tobin | | | 0.02 | (0.01,0.03) | 0.02 | (0.01,0.03) |
| Roxbury | Trotter | 0.02 | (0.01,0.02) | 0.05 | (0.04,0.06) | 0.04 | (0.03,0.05) |
| Roxbury | UP Acad. Dor. | 0.02 | (0.02,0.03) | 0.04 | (0.03,0.05) | 0.06 | (0.05,0.07) |
| Roxbury | West Zone ELC | | | 0.01 | (0.01,0.02) | 0.01 | (0.01,0.02) |
| Roxbury | Winthrop | 0.02 | (0.02,0.03) | 0.04 | (0.03,0.05) | 0.03 | (0.03,0.04) |
| South Boston | Blackstone | | | 0.03 | (0.02,0.05) | 0.03 | (0.02,0.05) |
| South Boston | Clap | 0.01 | (0.00,0.01) | 0.06 | (0.04,0.08) | 0.06 | (0.04,0.08) |
| South Boston | Condon | 0.10 | (0.07,0.12) | 0.15 | (0.12,0.18) | 0.14 | (0.11,0.17) |
| South Boston | Dever | 0.01 | (0.00,0.03) | 0.05 | (0.03,0.07) | 0.05 | (0.03,0.07) |
| South Boston | Dudley | | | 0.03 | (0.01,0.04) | 0.07 | (0.04,0.09) |
| South Boston | E Greenwood | 0.01 | (0.00,0.02) | | | | |
| South Boston | Eliot | 0.01 | (0.00,0.03) | 0.02 | (0.01,0.03) | 0.01 | (0.00,0.03) |
| South Boston | Everett | | | 0.02 | (0.01,0.03) | 0.01 | (0.00,0.03) |
| South Boston | Harvard/Kent | 0.02 | (0.01,0.02) | 0.01 | (0.00,0.01) | 0.01 | (0.00,0.01) |
| South Boston | Haynes | 0.01 | (0.00,0.02) | 0.01 | (0.00,0.03) | 0.02 | (0.01,0.03) |
| South Boston | Hernandez | | | 0.02 | (0.01,0.03) | 0.02 | (0.01,0.03) |
| South Boston | Holland | 0.00 | (0.00,0.01) | | | | |
| South Boston | Hurley | 0.08 | (0.06,0.11) | 0.03 | (0.01,0.05) | 0.03 | (0.01,0.05) |
| South Boston | Jackson/Mann | | | 0.01 | (0.00,0.03) | 0.01 | (0.00,0.03) |
| South Boston | Mason | 0.37 | (0.32,0.42) | 0.05 | (0.03,0.07) | 0.04 | (0.02,0.06) |
| South Boston | Mather | | | 0.00 | (0.00,0.01) | 0.00 | (0.00,0.01) |
| South Boston | Murphy | 0.01 | (0.00,0.02) | 0.01 | (0.00,0.01) | 0.01 | (0.00,0.01) |
| South Boston | Orchard Gardens | 0.03 | (0.02,0.04) | 0.04 | (0.02,0.06) | 0.04 | (0.02,0.06) |
| South Boston | Perkins | 0.01 | (0.01,0.02) | 0.06 | (0.04,0.09) | 0.06 | (0.04,0.09) |
| South Boston | Perry | 0.04 | (0.03,0.05) | 0.13 | (0.10,0.15) | 0.13 | (0.10,0.15) |
| South Boston | Quincy | 0.18 | (0.15,0.21) | 0.10 | (0.07,0.12) | 0.10 | (0.07,0.13) |
| South Boston | Roosevelt | 0.00 | (0.00,0.01) | | | | |
| South Boston | Russell | 0.02 | (0.01,0.03) | 0.04 | (0.03,0.06) | 0.03 | (0.02,0.05) |
| South Boston | Tynan | 0.01 | (0.00,0.02) | 0.08 | (0.06,0.10) | 0.08 | (0.05,0.10) |
| South Boston | UP Acad. Dor. | 0.02 | (0.01,0.03) | 0.02 | (0.01,0.04) | 0.03 | (0.01,0.05) |
| South Boston | Winthrop | 0.02 | (0.01,0.04) | 0.01 | (0.00,0.02) | 0.01 | (0.00,0.01) |
| South Dorchester | Condon | 0.02 | (0.02,0.03) | 0.01 | (0.01,0.02) | 0.01 | (0.01,0.02) |

Continued on next page

**Table 9 – continued from previous page**

| Neighborhood | School | Naive mean | Naive (95% C.I.) | Logit mean | Logit (95% C.I.) | Mixed Logit mean | Mixed Logit (95% C.I.) |
|---|---|---|---|---|---|---|---|
| South Dorchester | Dudley | | | 0.03 | (0.02,0.05) | 0.07 | (0.06,0.08) |
| South Dorchester | Ellison/Parks | 0.01 | (0.01,0.02) | 0.03 | (0.02,0.04) | 0.03 | (0.02,0.04) |
| South Dorchester | Everett | | | 0.03 | (0.02,0.04) | 0.03 | (0.02,0.03) |
| South Dorchester | Haynes | | | 0.02 | (0.01,0.03) | 0.02 | (0.01,0.03) |
| South Dorchester | Henderson | 0.23 | (0.22,0.24) | 0.10 | (0.08,0.11) | 0.09 | (0.07,0.11) |
| South Dorchester | Hernandez | 0.01 | (0.01,0.02) | 0.04 | (0.04,0.06) | 0.04 | (0.03,0.05) |
| South Dorchester | Holland | 0.06 | (0.05,0.07) | 0.07 | (0.06,0.08) | 0.06 | (0.05,0.07) |
| South Dorchester | Holmes | 0.01 | (0.01,0.01) | 0.04 | (0.03,0.05) | 0.03 | (0.03,0.04) |
| South Dorchester | Jackson/Mann | | | 0.01 | (0.01,0.02) | 0.02 | (0.01,0.02) |
| South Dorchester | Kenny | 0.06 | (0.05,0.08) | 0.05 | (0.04,0.06) | 0.05 | (0.04,0.06) |
| South Dorchester | King | | | 0.01 | (0.01,0.02) | 0.01 | (0.01,0.01) |
| South Dorchester | Lee | 0.01 | (0.00,0.01) | 0.04 | (0.01,0.06) | 0.03 | (0.01,0.05) |
| South Dorchester | Mason | 0.02 | (0.01,0.03) | | | | |
| South Dorchester | Mather | 0.08 | (0.07,0.09) | 0.08 | (0.06,0.09) | 0.07 | (0.06,0.08) |
| South Dorchester | Murphy | 0.26 | (0.25,0.27) | 0.19 | (0.17,0.20) | 0.18 | (0.17,0.20) |
| South Dorchester | Russell | 0.01 | (0.01,0.01) | 0.01 | (0.01,0.02) | 0.01 | (0.01,0.02) |
| South Dorchester | S. Greenwood | 0.08 | (0.06,0.09) | 0.06 | (0.05,0.07) | 0.05 | (0.04,0.06) |
| South Dorchester | Taylor | 0.02 | (0.01,0.03) | 0.02 | (0.01,0.03) | 0.02 | (0.01,0.03) |
| South Dorchester | UP Acad. Dor. | 0.04 | (0.03,0.04) | 0.06 | (0.05,0.08) | 0.10 | (0.09,0.12) |
| South Dorchester | Young Achievers | 0.01 | (0.01,0.01) | 0.02 | (0.01,0.03) | 0.02 | (0.01,0.03) |
| South End | Blackstone | 0.04 | (0.03,0.06) | 0.11 | (0.09,0.14) | 0.11 | (0.09,0.13) |
| South End | Clap | | | 0.01 | (0.00,0.01) | 0.01 | (0.00,0.01) |
| South End | Condon | 0.04 | (0.03,0.05) | 0.05 | (0.03,0.06) | 0.05 | (0.03,0.06) |
| South End | Curley | 0.01 | (0.00,0.01) | | | | |
| South End | Dever | 0.01 | (0.00,0.02) | | | | |
| South End | Dudley | | | 0.03 | (0.02,0.05) | 0.08 | (0.06,0.11) |
| South End | Edison | 0.02 | (0.01,0.03) | 0.01 | (0.00,0.01) | 0.01 | (0.00,0.01) |
| South End | Eliot | 0.02 | (0.01,0.04) | 0.02 | (0.01,0.03) | 0.02 | (0.01,0.04) |
| South End | Hale | 0.04 | (0.03,0.06) | 0.02 | (0.01,0.03) | 0.02 | (0.01,0.03) |
| South End | Harvard/Kent | 0.01 | (0.00,0.02) | 0.01 | (0.00,0.01) | 0.01 | (0.00,0.01) |
| South End | Haynes | 0.01 | (0.00,0.02) | 0.01 | (0.00,0.02) | 0.01 | (0.01,0.02) |
| South End | Hennigan | 0.01 | (0.01,0.02) | 0.01 | (0.00,0.02) | 0.01 | (0.00,0.02) |
| South End | Hernandez | | | 0.04 | (0.02,0.05) | 0.03 | (0.02,0.05) |
| South End | Higginson/Lewis | | | 0.01 | (0.01,0.02) | 0.01 | (0.00,0.02) |
| South End | Hurley | 0.25 | (0.23,0.26) | 0.15 | (0.13,0.17) | 0.15 | (0.13,0.17) |
| South End | J.F. Kennedy | 0.01 | (0.00,0.01) | | | | |
| South End | Jackson/Mann | 0.04 | (0.02,0.06) | 0.03 | (0.02,0.05) | 0.03 | (0.01,0.04) |
| South End | Mason | 0.19 | (0.17,0.22) | 0.07 | (0.05,0.10) | 0.06 | (0.04,0.08) |
| South End | Orchard Gardens | 0.04 | (0.03,0.05) | 0.11 | (0.09,0.14) | 0.10 | (0.08,0.13) |
| South End | Perkins | | | 0.01 | (0.00,0.02) | 0.01 | (0.00,0.02) |
| South End | Quincy | 0.17 | (0.15,0.19) | 0.16 | (0.14,0.19) | 0.16 | (0.14,0.19) |
| South End | Russell | 0.01 | (0.00,0.02) | | | | |
| South End | Tobin | 0.01 | (0.00,0.02) | 0.04 | (0.02,0.05) | 0.03 | (0.02,0.04) |
| South End | Tynan | | | 0.00 | (0.00,0.01) | 0.00 | (0.00,0.01) |
| South End | UP Acad. Dor. | 0.01 | (0.01,0.02) | 0.02 | (0.01,0.03) | 0.02 | (0.01,0.04) |
| South End | Warren/Prescott | 0.01 | (0.00,0.01) | | | | |
| South End | West Zone ELC | | | 0.01 | (0.01,0.02) | 0.01 | (0.00,0.02) |
| South End | Winship | 0.01 | (0.00,0.01) | 0.01 | (0.00,0.01) | | |
| South End | Winthrop | 0.02 | (0.01,0.03) | 0.02 | (0.01,0.03) | 0.01 | (0.01,0.02) |
| West Roxbury | BTU | | | 0.01 | (0.00,0.01) | 0.01 | (0.00,0.01) |
| West Roxbury | Bates | | | 0.05 | (0.04,0.07) | 0.05 | (0.04,0.07) |
| West Roxbury | Beethoven | 0.09 | (0.08,0.11) | 0.22 | (0.20,0.24) | 0.22 | (0.20,0.24) |
| West Roxbury | Channing | | | 0.03 | (0.02,0.04) | 0.03 | (0.02,0.04) |
| West Roxbury | Conley | 0.11 | (0.09,0.13) | 0.02 | (0.01,0.03) | 0.02 | (0.01,0.03) |
| West Roxbury | Dudley | | | | | 0.01 | (0.01,0.02) |

Continued on next page

**Table 9 – continued from previous page**

| Neighborhood | School | Naive mean | Naive (95% C.I.) | Logit mean | Logit (95% C.I.) | Mixed Logit mean | Mixed Logit (95% C.I.) |
|---|---|---|---|---|---|---|---|
| West Roxbury | E Greenwood | | | 0.02 | (0.01,0.03) | 0.02 | (0.01,0.03) |
| West Roxbury | Ellison/Parks | | | 0.01 | (0.00,0.02) | 0.01 | (0.00,0.01) |
| West Roxbury | Grew | | | 0.02 | (0.01,0.04) | 0.02 | (0.01,0.04) |
| West Roxbury | Hernandez | | | 0.01 | (0.00,0.02) | 0.01 | (0.00,0.02) |
| West Roxbury | Kilmer | 0.25 | (0.24,0.27) | 0.22 | (0.20,0.23) | 0.21 | (0.19,0.23) |
| West Roxbury | Lyndon | 0.26 | (0.25,0.27) | 0.21 | (0.19,0.23) | 0.21 | (0.18,0.23) |
| West Roxbury | Manning | 0.02 | (0.01,0.03) | 0.02 | (0.01,0.03) | 0.02 | (0.01,0.03) |
| West Roxbury | Mozart | 0.02 | (0.01,0.02) | 0.09 | (0.07,0.11) | 0.09 | (0.07,0.11) |
| West Roxbury | Roosevelt | 0.03 | (0.02,0.04) | 0.01 | (0.01,0.02) | 0.02 | (0.01,0.03) |
| West Roxbury | Sumner | 0.12 | (0.11,0.14) | 0.02 | (0.01,0.03) | 0.02 | (0.01,0.03) |
| West Roxbury | UP Acad. Dor. | 0.05 | (0.04,0.06) | | | 0.01 | (0.00,0.02) |

### D.2.2 K1

Table 10: Top Choice Market Share Predictions for 2014 K1

| Neighborhood | School | Naive mean | Naive (95% C.I.) | Logit mean | Logit (95% C.I.) | Mixed Logit mean | Mixed Logit (95% C.I.) |
|---|---|---|---|---|---|---|---|
| Allston-Brighton | Baldwin | 0.15 | (0.11,0.19) | 0.29 | (0.22,0.37) | 0.30 | (0.23,0.38) |
| Allston-Brighton | Blackstone | 0.01 | (0.00,0.03) | 0.01 | (0.00,0.03) | 0.01 | (0.00,0.04) |
| Allston-Brighton | Curley | | | 0.02 | (0.00,0.05) | 0.02 | (0.00,0.04) |
| Allston-Brighton | Edison | 0.29 | (0.20,0.36) | 0.19 | (0.12,0.25) | 0.18 | (0.12,0.25) |
| Allston-Brighton | Ellis | | | | | 0.00 | (0.00,0.01) |
| Allston-Brighton | Gardner | 0.06 | (0.03,0.10) | 0.14 | (0.09,0.21) | 0.16 | (0.09,0.23) |
| Allston-Brighton | Hale | 0.02 | (0.00,0.05) | 0.00 | (0.00,0.01) | | |
| Allston-Brighton | Hernandez | 0.09 | (0.04,0.14) | 0.02 | (0.00,0.06) | 0.03 | (0.00,0.07) |
| Allston-Brighton | Hurley | 0.05 | (0.01,0.09) | 0.00 | (0.00,0.01) | 0.00 | (0.00,0.02) |
| Allston-Brighton | J.F. Kennedy | | | 0.00 | (0.00,0.01) | | |
| Allston-Brighton | Jackson/Mann | 0.11 | (0.05,0.17) | 0.15 | (0.10,0.22) | 0.14 | (0.08,0.21) |
| Allston-Brighton | Manning | 0.16 | (0.10,0.23) | 0.01 | (0.00,0.02) | 0.00 | (0.00,0.02) |
| Allston-Brighton | Mendell | | | 0.01 | (0.00,0.02) | 0.00 | (0.00,0.02) |
| Allston-Brighton | Tobin | | | 0.00 | (0.00,0.02) | 0.01 | (0.00,0.02) |
| Allston-Brighton | Winship | 0.06 | (0.02,0.11) | 0.15 | (0.09,0.22) | 0.14 | (0.08,0.21) |
| Charlestown | Adams | 0.03 | (0.00,0.07) | 0.00 | (0.00,0.01) | 0.00 | (0.00,0.01) |
| Charlestown | Baldwin | 0.03 | (0.00,0.07) | 0.01 | (0.00,0.03) | 0.01 | (0.00,0.03) |
| Charlestown | Blackstone | 0.02 | (0.00,0.05) | 0.03 | (0.00,0.07) | 0.03 | (0.00,0.07) |
| Charlestown | East Boston EEC | | | 0.02 | (0.00,0.04) | 0.03 | (0.00,0.07) |
| Charlestown | Eliot | 0.05 | (0.00,0.10) | 0.48 | (0.37,0.59) | 0.47 | (0.36,0.58) |
| Charlestown | Harvard/Kent | 0.81 | (0.72,0.89) | 0.29 | (0.19,0.40) | 0.30 | (0.20,0.41) |
| Charlestown | Hernandez | | | 0.00 | (0.00,0.03) | 0.01 | (0.00,0.03) |
| Charlestown | O'Donnell | | | 0.01 | (0.00,0.04) | 0.01 | (0.00,0.04) |
| Charlestown | Otis | 0.05 | (0.01,0.09) | 0.01 | (0.00,0.05) | 0.01 | (0.00,0.04) |
| Charlestown | Quincy | 0.02 | (0.00,0.05) | 0.13 | (0.06,0.20) | 0.12 | (0.05,0.20) |
| Charlestown | Tynan | | | 0.01 | (0.00,0.04) | 0.01 | (0.00,0.03) |
| Downtown | Adams | 0.01 | (0.00,0.04) | 0.00 | (0.00,0.01) | 0.00 | (0.00,0.01) |
| Downtown | Baldwin | 0.01 | (0.00,0.03) | 0.01 | (0.00,0.03) | 0.01 | (0.00,0.03) |
| Downtown | Blackstone | | | 0.05 | (0.01,0.10) | 0.05 | (0.01,0.10) |
| Downtown | Clap | | | 0.00 | (0.00,0.01) | | |
| Downtown | Condon | | | 0.02 | (0.00,0.05) | 0.02 | (0.00,0.05) |
| Downtown | Curley | | | 0.01 | (0.00,0.02) | 0.00 | (0.00,0.02) |
| Downtown | East Boston EEC | | | 0.01 | (0.00,0.03) | 0.02 | (0.00,0.05) |
| Downtown | Edison | 0.19 | (0.11,0.29) | 0.01 | (0.00,0.03) | 0.01 | (0.00,0.03) |

Continued on next page

**Table 10 – continued from previous page**

| Neighborhood | School | Naive mean | Naive (95% C.I.) | Logit mean | Logit (95% C.I.) | Mixed Logit mean | Mixed Logit (95% C.I.) |
|---|---|---|---|---|---|---|---|
| Downtown | Eliot | 0.34 | (0.25,0.44) | 0.40 | (0.30,0.51) | 0.40 | (0.30,0.51) |
| Downtown | Gardner | | | 0.00 | (0.00,0.01) | 0.00 | (0.00,0.01) |
| Downtown | Hale | 0.02 | (0.00,0.06) | 0.01 | (0.00,0.03) | 0.00 | (0.00,0.02) |
| Downtown | Harvard/Kent | 0.01 | (0.00,0.04) | 0.04 | (0.00,0.08) | 0.03 | (0.00,0.07) |
| Downtown | Haynes | 0.01 | (0.00,0.04) | | | 0.00 | (0.00,0.01) |
| Downtown | Hernandez | 0.01 | (0.00,0.04) | 0.02 | (0.00,0.05) | 0.02 | (0.00,0.05) |
| Downtown | Higginson/Lewis | | | 0.00 | (0.00,0.01) | 0.00 | (0.00,0.01) |
| Downtown | Hurley | 0.11 | (0.05,0.18) | 0.06 | (0.01,0.11) | 0.06 | (0.01,0.11) |
| Downtown | J.F. Kennedy | | | 0.00 | (0.00,0.02) | 0.00 | (0.00,0.02) |
| Downtown | Jackson/Mann | | | 0.00 | (0.00,0.02) | 0.00 | (0.00,0.02) |
| Downtown | Mason | | | 0.00 | (0.00,0.02) | 0.00 | (0.00,0.02) |
| Downtown | Mendell | | | 0.00 | (0.00,0.01) | 0.00 | (0.00,0.01) |
| Downtown | Orchard Gardens | 0.01 | (0.00,0.04) | 0.02 | (0.00,0.06) | 0.02 | (0.00,0.05) |
| Downtown | Otis | 0.11 | (0.05,0.18) | 0.00 | (0.00,0.01) | 0.00 | (0.00,0.02) |
| Downtown | Quincy | 0.14 | (0.08,0.23) | 0.31 | (0.22,0.41) | 0.31 | (0.22,0.42) |
| Downtown | Russell | 0.01 | (0.00,0.04) | | | | |
| Downtown | Tobin | | | 0.01 | (0.00,0.03) | 0.01 | (0.00,0.04) |
| Downtown | Tynan | | | 0.01 | (0.00,0.03) | 0.01 | (0.00,0.03) |
| Downtown | West Zone ELC | | | 0.01 | (0.00,0.04) | 0.01 | (0.00,0.04) |
| East Boston | Adams | 0.48 | (0.42,0.53) | 0.13 | (0.09,0.17) | 0.11 | (0.07,0.14) |
| East Boston | Baldwin | 0.01 | (0.01,0.02) | | | | |
| East Boston | Blackstone | 0.02 | (0.01,0.04) | 0.01 | (0.00,0.01) | 0.01 | (0.00,0.03) |
| East Boston | Bradley | 0.07 | (0.04,0.10) | 0.15 | (0.12,0.19) | 0.17 | (0.13,0.22) |
| East Boston | East Boston EEC | 0.06 | (0.04,0.08) | 0.26 | (0.21,0.31) | 0.27 | (0.22,0.32) |
| East Boston | Edison | 0.00 | (0.00,0.01) | | | | |
| East Boston | Eliot | | | 0.01 | (0.00,0.03) | 0.01 | (0.00,0.02) |
| East Boston | Harvard/Kent | 0.01 | (0.00,0.02) | 0.01 | (0.00,0.02) | 0.00 | (0.00,0.01) |
| East Boston | Hernandez | | | 0.00 | (0.00,0.01) | 0.03 | (0.01,0.04) |
| East Boston | Hurley | 0.00 | (0.00,0.01) | | | | |
| East Boston | Jackson/Mann | 0.01 | (0.00,0.02) | | | | |
| East Boston | Kennedy Patrick | 0.03 | (0.01,0.05) | 0.11 | (0.08,0.15) | 0.10 | (0.07,0.14) |
| East Boston | Lyndon | 0.00 | (0.00,0.01) | | | | |
| East Boston | O'Donnell | 0.03 | (0.01,0.05) | 0.09 | (0.06,0.13) | 0.07 | (0.04,0.10) |
| East Boston | Orchard Gardens | 0.01 | (0.00,0.02) | | | | |
| East Boston | Otis | 0.25 | (0.20,0.29) | 0.21 | (0.17,0.26) | 0.21 | (0.16,0.25) |
| East Boston | Quincy | 0.01 | (0.00,0.02) | | | 0.00 | (0.00,0.01) |
| East Boston | Tobin | 0.00 | (0.00,0.01) | | | | |
| East Boston | Tynan | | | | | 0.00 | (0.00,0.01) |
| Hyde Park | BTU | | | 0.00 | (0.00,0.01) | 0.00 | (0.00,0.01) |
| Hyde Park | Bates | 0.01 | (0.00,0.02) | 0.06 | (0.03,0.10) | 0.05 | (0.02,0.09) |
| Hyde Park | Beethoven | 0.01 | (0.00,0.03) | 0.09 | (0.06,0.14) | 0.08 | (0.04,0.12) |
| Hyde Park | Channing | 0.02 | (0.01,0.05) | 0.08 | (0.04,0.12) | 0.08 | (0.04,0.12) |
| Hyde Park | Chittick | 0.06 | (0.03,0.09) | 0.08 | (0.04,0.12) | 0.07 | (0.04,0.11) |
| Hyde Park | Clap | 0.01 | (0.00,0.02) | | | | |
| Hyde Park | Condon | 0.01 | (0.00,0.02) | | | | |
| Hyde Park | Conley | 0.27 | (0.21,0.33) | 0.08 | (0.05,0.12) | 0.08 | (0.04,0.13) |
| Hyde Park | Ellison/Parks | 0.01 | (0.00,0.01) | 0.06 | (0.03,0.09) | 0.05 | (0.02,0.09) |
| Hyde Park | Haley | | | 0.03 | (0.01,0.06) | 0.04 | (0.02,0.07) |
| Hyde Park | Henderson | 0.01 | (0.00,0.01) | 0.00 | (0.00,0.01) | 0.00 | (0.00,0.01) |
| Hyde Park | Hernandez | 0.01 | (0.00,0.03) | 0.03 | (0.01,0.07) | 0.03 | (0.01,0.06) |
| Hyde Park | Kilmer | 0.02 | (0.00,0.04) | 0.04 | (0.01,0.07) | 0.04 | (0.02,0.07) |
| Hyde Park | Lee | 0.00 | (0.00,0.01) | 0.01 | (0.00,0.01) | 0.01 | (0.00,0.01) |
| Hyde Park | Mattahunt | 0.02 | (0.00,0.04) | 0.03 | (0.01,0.06) | 0.03 | (0.01,0.06) |
| Hyde Park | Mozart | | | 0.04 | (0.02,0.08) | 0.05 | (0.02,0.08) |
| Hyde Park | Philbrick | 0.05 | (0.02,0.09) | 0.04 | (0.01,0.07) | 0.03 | (0.01,0.06) |

Continued on next page

**Table 10 – continued from previous page**

| Neighborhood | School | Naive mean | Naive (95% C.I.) | Logit mean | Logit (95% C.I.) | Mixed Logit mean | Mixed Logit (95% C.I.) |
|---|---|---|---|---|---|---|---|
| Hyde Park | Roosevelt | 0.37 | (0.30,0.45) | 0.25 | (0.18,0.31) | 0.27 | (0.21,0.34) |
| Hyde Park | S. Greenwood | 0.01 | (0.00,0.02) | 0.00 | (0.00,0.01) | 0.00 | (0.00,0.01) |
| Hyde Park | Sumner | 0.01 | (0.00,0.03) | 0.02 | (0.01,0.05) | 0.02 | (0.01,0.05) |
| Hyde Park | Taylor | | | 0.00 | (0.00,0.02) | 0.00 | (0.00,0.01) |
| Hyde Park | West Zone ELC | 0.01 | (0.00,0.02) | | | | |
| Hyde Park | Young Achievers | 0.10 | (0.06,0.15) | 0.03 | (0.01,0.06) | 0.04 | (0.01,0.07) |
| Jamaica Plain | BTU | 0.02 | (0.00,0.04) | 0.07 | (0.03,0.11) | 0.06 | (0.03,0.10) |
| Jamaica Plain | Baldwin | 0.01 | (0.00,0.01) | 0.01 | (0.00,0.01) | 0.01 | (0.00,0.01) |
| Jamaica Plain | Bates | 0.00 | (0.00,0.02) | | | | |
| Jamaica Plain | Beethoven | 0.00 | (0.00,0.02) | | | | |
| Jamaica Plain | Blackstone | 0.01 | (0.00,0.01) | 0.01 | (0.00,0.02) | 0.01 | (0.00,0.02) |
| Jamaica Plain | Curley | 0.07 | (0.03,0.10) | 0.26 | (0.20,0.32) | 0.25 | (0.19,0.31) |
| Jamaica Plain | Ellis | 0.02 | (0.00,0.03) | 0.03 | (0.01,0.05) | 0.02 | (0.01,0.05) |
| Jamaica Plain | Ellison/Parks | 0.03 | (0.01,0.06) | 0.00 | (0.00,0.01) | 0.01 | (0.00,0.02) |
| Jamaica Plain | Hale | 0.33 | (0.26,0.39) | 0.02 | (0.00,0.04) | 0.01 | (0.00,0.03) |
| Jamaica Plain | Haley | | | 0.01 | (0.00,0.03) | 0.01 | (0.00,0.02) |
| Jamaica Plain | Hernandez | | | 0.07 | (0.03,0.10) | 0.09 | (0.05,0.13) |
| Jamaica Plain | Higginson/Lewis | 0.00 | (0.00,0.02) | 0.00 | (0.00,0.02) | 0.00 | (0.00,0.01) |
| Jamaica Plain | Hurley | 0.08 | (0.04,0.12) | 0.03 | (0.01,0.06) | 0.03 | (0.01,0.06) |
| Jamaica Plain | J.F. Kennedy | 0.01 | (0.00,0.03) | 0.06 | (0.03,0.10) | 0.05 | (0.03,0.09) |
| Jamaica Plain | Jackson/Mann | 0.01 | (0.00,0.03) | 0.03 | (0.01,0.06) | 0.03 | (0.01,0.06) |
| Jamaica Plain | Kilmer | 0.01 | (0.00,0.03) | 0.00 | (0.00,0.01) | 0.00 | (0.00,0.01) |
| Jamaica Plain | Lyndon | 0.01 | (0.00,0.02) | | | | |
| Jamaica Plain | Manning | 0.27 | (0.21,0.34) | 0.09 | (0.05,0.14) | 0.09 | (0.05,0.14) |
| Jamaica Plain | Mason | | | 0.00 | (0.00,0.01) | 0.00 | (0.00,0.01) |
| Jamaica Plain | Mendell | 0.02 | (0.01,0.04) | 0.05 | (0.02,0.08) | 0.04 | (0.02,0.08) |
| Jamaica Plain | Mission Hill | 0.03 | (0.01,0.06) | 0.12 | (0.08,0.18) | 0.13 | (0.08,0.18) |
| Jamaica Plain | Orchard Gardens | 0.00 | (0.00,0.02) | 0.02 | (0.01,0.05) | 0.02 | (0.01,0.05) |
| Jamaica Plain | Philbrick | 0.01 | (0.00,0.04) | 0.01 | (0.00,0.03) | 0.01 | (0.00,0.02) |
| Jamaica Plain | Quincy | 0.00 | (0.00,0.02) | 0.00 | (0.00,0.01) | 0.00 | (0.00,0.01) |
| Jamaica Plain | S. Greenwood | 0.02 | (0.01,0.04) | 0.00 | (0.00,0.01) | 0.00 | (0.00,0.01) |
| Jamaica Plain | Tobin | 0.02 | (0.00,0.04) | 0.03 | (0.01,0.06) | 0.04 | (0.01,0.06) |
| Jamaica Plain | Trotter | | | 0.00 | (0.00,0.02) | 0.00 | (0.00,0.02) |
| Jamaica Plain | West Zone ELC | | | 0.05 | (0.02,0.08) | 0.06 | (0.02,0.09) |
| Mattapan | BTU | 0.01 | (0.00,0.03) | 0.05 | (0.02,0.09) | 0.05 | (0.02,0.09) |
| Mattapan | Bates | | | 0.00 | (0.00,0.01) | 0.00 | (0.00,0.01) |
| Mattapan | Channing | 0.02 | (0.01,0.05) | 0.01 | (0.00,0.02) | 0.01 | (0.00,0.02) |
| Mattapan | Chittick | 0.01 | (0.00,0.02) | 0.03 | (0.01,0.05) | 0.02 | (0.01,0.05) |
| Mattapan | Clap | 0.01 | (0.00,0.02) | | | | |
| Mattapan | Condon | 0.01 | (0.00,0.02) | | | | |
| Mattapan | Conley | | | 0.01 | (0.00,0.03) | 0.01 | (0.00,0.02) |
| Mattapan | Curley | 0.01 | (0.00,0.02) | 0.00 | (0.00,0.01) | 0.00 | (0.00,0.01) |
| Mattapan | Dever | 0.04 | (0.02,0.07) | 0.01 | (0.00,0.03) | 0.02 | (0.00,0.04) |
| Mattapan | Ellison/Parks | 0.12 | (0.08,0.17) | 0.14 | (0.09,0.19) | 0.15 | (0.10,0.20) |
| Mattapan | Hale | 0.01 | (0.00,0.02) | | | | |
| Mattapan | Haley | 0.02 | (0.00,0.04) | 0.09 | (0.05,0.13) | 0.08 | (0.04,0.12) |
| Mattapan | Henderson | 0.21 | (0.15,0.27) | 0.02 | (0.01,0.05) | 0.03 | (0.01,0.06) |
| Mattapan | Hernandez | 0.01 | (0.00,0.02) | 0.05 | (0.02,0.08) | 0.05 | (0.02,0.08) |
| Mattapan | Holland | 0.01 | (0.00,0.03) | 0.00 | (0.00,0.01) | 0.00 | (0.00,0.01) |
| Mattapan | Holmes | 0.01 | (0.00,0.02) | 0.01 | (0.00,0.03) | 0.01 | (0.00,0.03) |
| Mattapan | Jackson/Mann | | | 0.01 | (0.00,0.02) | 0.02 | (0.00,0.04) |
| Mattapan | Kenny | 0.01 | (0.00,0.03) | 0.01 | (0.00,0.03) | 0.01 | (0.00,0.03) |
| Mattapan | Lee | 0.02 | (0.00,0.03) | 0.07 | (0.01,0.15) | 0.06 | (0.00,0.14) |
| Mattapan | Mason | 0.01 | (0.00,0.02) | | | | |
| Mattapan | Mather | 0.01 | (0.00,0.02) | 0.00 | (0.00,0.01) | 0.00 | (0.00,0.01) |

Continued on next page

**Table 10 – continued from previous page**

| Neighborhood | School | Naive mean | Naive (95% C.I.) | Logit mean | Logit (95% C.I.) | Mixed Logit mean | Mixed Logit (95% C.I.) |
|---|---|---|---|---|---|---|---|
| Mattapan | Mattahunt | 0.02 | (0.01,0.04) | 0.05 | (0.02,0.08) | 0.05 | (0.02,0.08) |
| Mattapan | Mendell | 0.01 | (0.00,0.02) | | | | |
| Mattapan | Mission Hill | | | 0.01 | (0.00,0.01) | 0.00 | (0.00,0.01) |
| Mattapan | Murphy | | | 0.03 | (0.01,0.06) | 0.04 | (0.01,0.07) |
| Mattapan | Otis | 0.01 | (0.00,0.02) | | | | |
| Mattapan | Perry | 0.01 | (0.00,0.02) | | | | |
| Mattapan | Philbrick | 0.24 | (0.18,0.31) | 0.03 | (0.01,0.06) | 0.03 | (0.01,0.05) |
| Mattapan | Roosevelt | 0.01 | (0.00,0.02) | 0.00 | (0.00,0.01) | 0.00 | (0.00,0.01) |
| Mattapan | Russell | 0.01 | (0.00,0.03) | 0.00 | (0.00,0.01) | 0.00 | (0.00,0.02) |
| Mattapan | S. Greenwood | 0.06 | (0.02,0.09) | 0.06 | (0.03,0.10) | 0.05 | (0.02,0.09) |
| Mattapan | Sumner | 0.01 | (0.00,0.02) | 0.01 | (0.00,0.02) | 0.01 | (0.00,0.02) |
| Mattapan | Taylor | 0.04 | (0.01,0.07) | 0.06 | (0.03,0.10) | 0.05 | (0.02,0.09) |
| Mattapan | Tobin | 0.01 | (0.00,0.02) | | | | |
| Mattapan | Tynan | 0.01 | (0.00,0.02) | | | | |
| Mattapan | Young Achievers | 0.04 | (0.01,0.06) | 0.16 | (0.11,0.23) | 0.17 | (0.12,0.22) |
| North Dorchester | Adams | 0.01 | (0.00,0.02) | | | | |
| North Dorchester | Blackstone | | | 0.01 | (0.00,0.03) | 0.01 | (0.00,0.03) |
| North Dorchester | Clap | 0.02 | (0.00,0.05) | 0.18 | (0.11,0.24) | 0.17 | (0.11,0.23) |
| North Dorchester | Condon | 0.05 | (0.01,0.08) | 0.03 | (0.01,0.06) | 0.03 | (0.01,0.06) |
| North Dorchester | Dever | 0.04 | (0.01,0.07) | 0.08 | (0.03,0.12) | 0.07 | (0.03,0.12) |
| North Dorchester | Edison | 0.01 | (0.00,0.03) | | | | |
| North Dorchester | Ellison/Parks | 0.04 | (0.01,0.07) | 0.00 | (0.00,0.02) | 0.01 | (0.00,0.02) |
| North Dorchester | Everett | 0.02 | (0.00,0.05) | 0.12 | (0.07,0.18) | 0.12 | (0.06,0.17) |
| North Dorchester | Hale | | | 0.00 | (0.00,0.01) | 0.00 | (0.00,0.01) |
| North Dorchester | Harvard/Kent | 0.01 | (0.00,0.03) | 0.00 | (0.00,0.01) | 0.00 | (0.00,0.01) |
| North Dorchester | Haynes | 0.29 | (0.22,0.36) | 0.08 | (0.04,0.12) | 0.09 | (0.05,0.14) |
| North Dorchester | Henderson | 0.05 | (0.02,0.08) | 0.03 | (0.01,0.06) | 0.04 | (0.01,0.07) |
| North Dorchester | Hernandez | | | 0.03 | (0.01,0.07) | 0.04 | (0.01,0.07) |
| North Dorchester | Higginson/Lewis | 0.01 | (0.00,0.03) | 0.00 | (0.00,0.01) | | |
| North Dorchester | Holland | 0.03 | (0.01,0.06) | 0.04 | (0.01,0.07) | 0.03 | (0.01,0.06) |
| North Dorchester | Hurley | | | 0.01 | (0.00,0.03) | 0.01 | (0.00,0.04) |
| North Dorchester | Jackson/Mann | | | 0.01 | (0.00,0.04) | 0.02 | (0.00,0.05) |
| North Dorchester | King | | | 0.03 | (0.01,0.06) | 0.02 | (0.00,0.05) |
| North Dorchester | Lee | 0.01 | (0.00,0.03) | 0.00 | (0.00,0.01) | 0.00 | (0.00,0.01) |
| North Dorchester | Mason | 0.19 | (0.14,0.25) | 0.05 | (0.02,0.09) | 0.04 | (0.01,0.08) |
| North Dorchester | Mather | 0.02 | (0.00,0.05) | 0.07 | (0.04,0.12) | 0.07 | (0.03,0.12) |
| North Dorchester | Murphy | 0.03 | (0.01,0.06) | 0.04 | (0.02,0.08) | 0.05 | (0.01,0.08) |
| North Dorchester | Orchard Gardens | 0.01 | (0.00,0.03) | 0.04 | (0.01,0.07) | 0.04 | (0.01,0.08) |
| North Dorchester | Perry | 0.01 | (0.00,0.02) | 0.01 | (0.00,0.03) | 0.01 | (0.00,0.03) |
| North Dorchester | Russell | 0.09 | (0.04,0.13) | 0.09 | (0.04,0.14) | 0.09 | (0.04,0.14) |
| North Dorchester | S. Greenwood | 0.01 | (0.00,0.03) | 0.00 | (0.00,0.01) | 0.00 | (0.00,0.02) |
| North Dorchester | Taylor | 0.01 | (0.00,0.02) | | | | |
| North Dorchester | Tobin | 0.01 | (0.00,0.02) | | | 0.00 | (0.00,0.01) |
| North Dorchester | Tynan | 0.02 | (0.00,0.05) | 0.01 | (0.00,0.03) | 0.01 | (0.00,0.03) |
| North Dorchester | Winthrop | 0.01 | (0.00,0.03) | 0.03 | (0.01,0.06) | 0.02 | (0.00,0.05) |
| North Dorchester | Young Achievers | 0.02 | (0.00,0.04) | 0.01 | (0.00,0.02) | 0.00 | (0.00,0.02) |
| Roslindale | BTU | 0.01 | (0.00,0.03) | 0.14 | (0.10,0.18) | 0.14 | (0.10,0.19) |
| Roslindale | Bates | 0.02 | (0.00,0.03) | 0.10 | (0.06,0.14) | 0.10 | (0.06,0.14) |
| Roslindale | Beethoven | 0.02 | (0.00,0.03) | 0.02 | (0.01,0.04) | 0.02 | (0.01,0.04) |
| Roslindale | Channing | 0.00 | (0.00,0.01) | 0.01 | (0.00,0.02) | 0.01 | (0.00,0.02) |
| Roslindale | Chittick | 0.00 | (0.00,0.01) | 0.01 | (0.00,0.03) | 0.01 | (0.00,0.02) |
| Roslindale | Conley | 0.13 | (0.09,0.17) | 0.07 | (0.04,0.11) | 0.06 | (0.03,0.09) |
| Roslindale | Curley | 0.02 | (0.00,0.03) | 0.02 | (0.00,0.03) | 0.02 | (0.00,0.04) |
| Roslindale | East Boston EEC | 0.00 | (0.00,0.01) | | | | |
| Roslindale | Ellis | 0.00 | (0.00,0.01) | | | | |

Continued on next page

**Table 10 – continued from previous page**

| Neighborhood | School | Naive mean | Naive (95% C.I.) | Logit mean | Logit (95% C.I.) | Mixed Logit mean | Mixed Logit (95% C.I.) |
|---|---|---|---|---|---|---|---|
| Roslindale | Ellison/Parks | | | 0.02 | (0.00,0.04) | 0.02 | (0.00,0.04) |
| Roslindale | Haley | 0.04 | (0.02,0.06) | 0.08 | (0.05,0.11) | 0.09 | (0.06,0.13) |
| Roslindale | Hernandez | 0.01 | (0.00,0.02) | 0.04 | (0.02,0.07) | 0.04 | (0.02,0.07) |
| Roslindale | Higginson/Lewis | 0.00 | (0.00,0.01) | | | | |
| Roslindale | Jackson/Mann | 0.00 | (0.00,0.01) | | | | |
| Roslindale | Kenny | 0.01 | (0.00,0.02) | | | | |
| Roslindale | Kilmer | 0.03 | (0.01,0.05) | 0.03 | (0.01,0.05) | 0.03 | (0.01,0.05) |
| Roslindale | King | 0.00 | (0.00,0.01) | | | | |
| Roslindale | Lyndon | 0.04 | (0.02,0.07) | 0.06 | (0.03,0.09) | 0.05 | (0.03,0.08) |
| Roslindale | Manning | 0.01 | (0.00,0.03) | 0.03 | (0.01,0.05) | 0.03 | (0.01,0.05) |
| Roslindale | Mason | 0.01 | (0.00,0.02) | | | | |
| Roslindale | Mattahunt | | | 0.02 | (0.01,0.04) | 0.03 | (0.01,0.05) |
| Roslindale | Mendell | 0.01 | (0.00,0.02) | 0.00 | (0.00,0.01) | 0.00 | (0.00,0.01) |
| Roslindale | Mission Hill | 0.01 | (0.00,0.02) | 0.03 | (0.01,0.05) | 0.03 | (0.01,0.05) |
| Roslindale | Mozart | 0.04 | (0.02,0.07) | 0.11 | (0.07,0.15) | 0.11 | (0.07,0.15) |
| Roslindale | Philbrick | 0.22 | (0.17,0.27) | 0.09 | (0.06,0.12) | 0.07 | (0.05,0.11) |
| Roslindale | Sumner | 0.31 | (0.26,0.37) | 0.09 | (0.05,0.12) | 0.09 | (0.05,0.13) |
| Roslindale | Trotter | 0.01 | (0.00,0.02) | | | | |
| Roslindale | Young Achievers | 0.03 | (0.01,0.05) | 0.03 | (0.01,0.06) | 0.04 | (0.02,0.06) |
| Roxbury | BTU | 0.01 | (0.00,0.02) | 0.01 | (0.00,0.02) | 0.01 | (0.00,0.02) |
| Roxbury | Baldwin | 0.01 | (0.00,0.02) | 0.01 | (0.00,0.02) | 0.01 | (0.00,0.01) |
| Roxbury | Beethoven | 0.00 | (0.00,0.01) | | | | |
| Roxbury | Blackstone | | | 0.03 | (0.01,0.04) | 0.02 | (0.01,0.04) |
| Roxbury | Channing | 0.00 | (0.00,0.01) | | | | |
| Roxbury | Clap | 0.00 | (0.00,0.01) | 0.03 | (0.01,0.04) | 0.02 | (0.01,0.04) |
| Roxbury | Conley | 0.00 | (0.00,0.01) | | | | |
| Roxbury | Curley | 0.02 | (0.01,0.04) | 0.06 | (0.04,0.09) | 0.06 | (0.04,0.09) |
| Roxbury | Dever | 0.00 | (0.00,0.01) | 0.01 | (0.00,0.02) | 0.01 | (0.00,0.02) |
| Roxbury | Edison | 0.01 | (0.00,0.02) | | | | |
| Roxbury | Eliot | 0.00 | (0.00,0.01) | | | | |
| Roxbury | Ellis | 0.01 | (0.00,0.02) | 0.04 | (0.02,0.07) | 0.04 | (0.02,0.06) |
| Roxbury | Ellison/Parks | 0.01 | (0.00,0.03) | 0.01 | (0.00,0.02) | 0.01 | (0.00,0.01) |
| Roxbury | Everett | 0.00 | (0.00,0.01) | 0.03 | (0.01,0.04) | 0.03 | (0.01,0.04) |
| Roxbury | Hale | 0.25 | (0.21,0.30) | 0.03 | (0.01,0.05) | 0.03 | (0.01,0.05) |
| Roxbury | Haley | 0.02 | (0.01,0.03) | 0.01 | (0.00,0.02) | 0.01 | (0.00,0.02) |
| Roxbury | Harvard/Kent | 0.01 | (0.00,0.02) | | | | |
| Roxbury | Haynes | 0.09 | (0.06,0.12) | 0.07 | (0.04,0.10) | 0.08 | (0.05,0.11) |
| Roxbury | Henderson | 0.07 | (0.04,0.10) | 0.01 | (0.00,0.02) | 0.01 | (0.00,0.02) |
| Roxbury | Hernandez | 0.01 | (0.00,0.02) | 0.09 | (0.06,0.12) | 0.11 | (0.08,0.15) |
| Roxbury | Higginson/Lewis | 0.01 | (0.00,0.02) | 0.02 | (0.01,0.04) | 0.02 | (0.01,0.04) |
| Roxbury | Holland | 0.02 | (0.00,0.04) | 0.03 | (0.01,0.05) | 0.03 | (0.01,0.05) |
| Roxbury | Holmes | 0.00 | (0.00,0.01) | 0.01 | (0.00,0.02) | 0.01 | (0.00,0.02) |
| Roxbury | Hurley | 0.05 | (0.03,0.07) | 0.03 | (0.01,0.05) | 0.03 | (0.01,0.05) |
| Roxbury | J.F. Kennedy | 0.02 | (0.01,0.04) | 0.03 | (0.02,0.06) | 0.03 | (0.01,0.05) |
| Roxbury | Jackson/Mann | 0.01 | (0.00,0.02) | 0.03 | (0.01,0.05) | 0.03 | (0.01,0.05) |
| Roxbury | King | 0.01 | (0.00,0.02) | 0.03 | (0.01,0.05) | 0.03 | (0.01,0.04) |
| Roxbury | Lee | 0.00 | (0.00,0.01) | 0.01 | (0.00,0.02) | 0.01 | (0.00,0.03) |
| Roxbury | Lyndon | 0.01 | (0.00,0.02) | | | | |
| Roxbury | Manning | 0.00 | (0.00,0.01) | | | | |
| Roxbury | Mason | 0.10 | (0.07,0.14) | 0.04 | (0.02,0.06) | 0.04 | (0.02,0.06) |
| Roxbury | Mather | 0.01 | (0.00,0.03) | 0.02 | (0.01,0.04) | 0.02 | (0.01,0.04) |
| Roxbury | Mattahunt | 0.00 | (0.00,0.01) | | | | |
| Roxbury | Mendell | | | 0.02 | (0.01,0.04) | 0.02 | (0.01,0.04) |
| Roxbury | Mission Hill | 0.01 | (0.01,0.03) | 0.03 | (0.02,0.05) | 0.03 | (0.02,0.05) |
| Roxbury | Murphy | | | 0.01 | (0.00,0.02) | 0.01 | (0.00,0.02) |

Continued on next page

**Table 10 – continued from previous page**

| Neighborhood | School | Naive mean | Naive (95% C.I.) | Logit mean | Logit (95% C.I.) | Mixed Logit mean | Mixed Logit (95% C.I.) |
|---|---|---|---|---|---|---|---|
| Roxbury | Orchard Gardens | 0.02 | (0.00,0.03) | 0.06 | (0.03,0.08) | 0.06 | (0.03,0.08) |
| Roxbury | Philbrick | 0.00 | (0.00,0.01) | | | | |
| Roxbury | Quincy | 0.01 | (0.00,0.02) | 0.00 | (0.00,0.01) | 0.00 | (0.00,0.01) |
| Roxbury | Roosevelt | 0.01 | (0.00,0.02) | | | | |
| Roxbury | Russell | 0.03 | (0.01,0.05) | 0.03 | (0.01,0.04) | 0.03 | (0.01,0.05) |
| Roxbury | S. Greenwood | 0.03 | (0.02,0.05) | 0.03 | (0.01,0.05) | 0.03 | (0.01,0.05) |
| Roxbury | Sumner | 0.01 | (0.00,0.02) | | | | |
| Roxbury | Taylor | 0.01 | (0.00,0.02) | | | | |
| Roxbury | Tobin | 0.01 | (0.00,0.02) | 0.02 | (0.00,0.03) | 0.02 | (0.00,0.03) |
| Roxbury | Trotter | 0.04 | (0.02,0.06) | 0.04 | (0.02,0.06) | 0.04 | (0.02,0.07) |
| Roxbury | West Zone ELC | 0.01 | (0.00,0.02) | 0.02 | (0.01,0.03) | 0.02 | (0.01,0.03) |
| Roxbury | Winship | 0.00 | (0.00,0.01) | | | | |
| Roxbury | Winthrop | 0.02 | (0.00,0.03) | 0.03 | (0.01,0.05) | 0.03 | (0.01,0.04) |
| Roxbury | Young Achievers | 0.01 | (0.00,0.02) | 0.01 | (0.00,0.01) | 0.01 | (0.00,0.01) |
| South Boston | Blackstone | | | 0.05 | (0.00,0.09) | 0.05 | (0.01,0.10) |
| South Boston | Chittick | 0.01 | (0.00,0.04) | | | 0.00 | (0.00,0.01) |
| South Boston | Clap | 0.04 | (0.00,0.10) | 0.10 | (0.04,0.17) | 0.10 | (0.03,0.17) |
| South Boston | Condon | 0.10 | (0.04,0.17) | 0.17 | (0.10,0.26) | 0.16 | (0.08,0.24) |
| South Boston | Dever | | | 0.06 | (0.01,0.12) | 0.06 | (0.01,0.12) |
| South Boston | East Boston EEC | | | 0.00 | (0.00,0.01) | 0.00 | (0.00,0.02) |
| South Boston | Eliot | | | 0.02 | (0.00,0.06) | 0.02 | (0.00,0.06) |
| South Boston | Ellison/Parks | 0.01 | (0.00,0.01) | 0.00 | (0.00,0.01) | 0.00 | (0.00,0.01) |
| South Boston | Everett | | | 0.02 | (0.00,0.06) | 0.01 | (0.00,0.04) |
| South Boston | Harvard/Kent | | | 0.00 | (0.00,0.01) | 0.00 | (0.00,0.01) |
| South Boston | Haynes | 0.12 | (0.05,0.19) | 0.01 | (0.00,0.05) | 0.02 | (0.00,0.06) |
| South Boston | Hernandez | | | 0.02 | (0.00,0.06) | 0.02 | (0.00,0.06) |
| South Boston | Hurley | | | 0.02 | (0.00,0.06) | 0.03 | (0.00,0.07) |
| South Boston | Jackson/Mann | | | 0.01 | (0.00,0.04) | 0.01 | (0.00,0.04) |
| South Boston | Lee | 0.01 | (0.00,0.04) | 0.00 | (0.00,0.01) | 0.00 | (0.00,0.01) |
| South Boston | Manning | 0.01 | (0.00,0.05) | 0.00 | (0.00,0.01) | 0.00 | (0.00,0.01) |
| South Boston | Mason | 0.15 | (0.07,0.22) | 0.02 | (0.00,0.06) | 0.02 | (0.00,0.06) |
| South Boston | Mather | | | 0.00 | (0.00,0.02) | 0.00 | (0.00,0.03) |
| South Boston | Murphy | 0.03 | (0.00,0.07) | 0.01 | (0.00,0.04) | 0.01 | (0.00,0.04) |
| South Boston | Orchard Gardens | | | 0.02 | (0.00,0.05) | 0.03 | (0.00,0.06) |
| South Boston | Perry | 0.05 | (0.01,0.10) | 0.17 | (0.09,0.26) | 0.18 | (0.10,0.26) |
| South Boston | Quincy | 0.35 | (0.24,0.46) | 0.17 | (0.09,0.27) | 0.17 | (0.09,0.27) |
| South Boston | Russell | 0.11 | (0.05,0.19) | 0.05 | (0.01,0.11) | 0.04 | (0.00,0.09) |
| South Boston | Tynan | | | 0.06 | (0.01,0.11) | 0.06 | (0.01,0.11) |
| South Boston | Winthrop | | | 0.00 | (0.00,0.02) | 0.00 | (0.00,0.02) |
| South Dorchester | Channing | 0.01 | (0.00,0.01) | | | | |
| South Dorchester | Clap | 0.01 | (0.00,0.02) | 0.01 | (0.00,0.02) | 0.01 | (0.00,0.02) |
| South Dorchester | Condon | 0.02 | (0.01,0.04) | 0.01 | (0.00,0.02) | 0.01 | (0.00,0.02) |
| South Dorchester | Dever | 0.01 | (0.00,0.03) | 0.00 | (0.00,0.01) | 0.00 | (0.00,0.01) |
| South Dorchester | Ellison/Parks | 0.15 | (0.12,0.19) | 0.05 | (0.03,0.07) | 0.06 | (0.03,0.08) |
| South Dorchester | Everett | 0.01 | (0.00,0.02) | 0.03 | (0.01,0.04) | 0.02 | (0.01,0.04) |
| South Dorchester | Haynes | | | 0.02 | (0.01,0.04) | 0.02 | (0.01,0.04) |
| South Dorchester | Henderson | 0.29 | (0.24,0.34) | 0.09 | (0.07,0.12) | 0.08 | (0.06,0.12) |
| South Dorchester | Hernandez | 0.01 | (0.00,0.01) | 0.04 | (0.02,0.06) | 0.04 | (0.02,0.07) |
| South Dorchester | Holland | 0.02 | (0.01,0.04) | 0.05 | (0.03,0.08) | 0.05 | (0.03,0.08) |
| South Dorchester | Holmes | 0.01 | (0.00,0.03) | 0.03 | (0.01,0.05) | 0.03 | (0.01,0.04) |
| South Dorchester | Jackson/Mann | | | 0.01 | (0.00,0.02) | 0.02 | (0.01,0.03) |
| South Dorchester | Kenny | 0.02 | (0.01,0.04) | 0.03 | (0.02,0.05) | 0.03 | (0.01,0.05) |
| South Dorchester | King | | | 0.01 | (0.01,0.03) | 0.01 | (0.00,0.03) |
| South Dorchester | Lee | 0.01 | (0.00,0.02) | 0.05 | (0.01,0.11) | 0.04 | (0.00,0.10) |
| South Dorchester | Mather | 0.11 | (0.08,0.14) | 0.07 | (0.05,0.10) | 0.07 | (0.04,0.10) |

Continued on next page

**Table 10 – continued from previous page**

| Neighborhood | School | Naive mean | Naive (95% C.I.) | Logit mean | Logit (95% C.I.) | Mixed Logit mean | Mixed Logit (95% C.I.) |
|---|---|---|---|---|---|---|---|
| South Dorchester | Mattahunt | 0.01 | (0.00,0.03) | | | | |
| South Dorchester | Mendell | 0.01 | (0.00,0.01) | | | | |
| South Dorchester | Mission Hill | 0.01 | (0.00,0.01) | | | | |
| South Dorchester | Murphy | 0.13 | (0.10,0.17) | 0.33 | (0.28,0.37) | 0.34 | (0.29,0.39) |
| South Dorchester | Orchard Gardens | 0.00 | (0.00,0.01) | | | | |
| South Dorchester | Perry | 0.01 | (0.00,0.01) | | | | |
| South Dorchester | Russell | 0.01 | (0.01,0.03) | 0.01 | (0.00,0.02) | 0.01 | (0.00,0.02) |
| South Dorchester | S. Greenwood | 0.05 | (0.03,0.08) | 0.05 | (0.03,0.08) | 0.05 | (0.03,0.07) |
| South Dorchester | Taylor | 0.02 | (0.01,0.04) | 0.02 | (0.01,0.04) | 0.02 | (0.01,0.04) |
| South Dorchester | Tobin | 0.01 | (0.00,0.01) | | | | |
| South Dorchester | Tynan | 0.02 | (0.01,0.03) | | | | |
| South Dorchester | Young Achievers | 0.01 | (0.00,0.02) | 0.02 | (0.01,0.03) | 0.02 | (0.01,0.03) |
| South End | Baldwin | 0.01 | (0.00,0.02) | 0.01 | (0.00,0.02) | 0.01 | (0.00,0.02) |
| South End | Blackstone | 0.03 | (0.00,0.06) | 0.15 | (0.08,0.21) | 0.14 | (0.08,0.21) |
| South End | Clap | | | 0.01 | (0.00,0.03) | 0.01 | (0.00,0.03) |
| South End | Condon | 0.01 | (0.00,0.03) | 0.04 | (0.01,0.08) | 0.04 | (0.01,0.08) |
| South End | Curley | | | 0.01 | (0.00,0.02) | 0.01 | (0.00,0.03) |
| South End | Dever | | | 0.00 | (0.00,0.02) | 0.00 | (0.00,0.02) |
| South End | Edison | 0.05 | (0.01,0.09) | 0.00 | (0.00,0.02) | 0.01 | (0.00,0.02) |
| South End | Eliot | 0.03 | (0.01,0.06) | 0.03 | (0.00,0.06) | 0.03 | (0.00,0.06) |
| South End | Ellis | | | | | 0.00 | (0.00,0.01) |
| South End | Gardner | 0.02 | (0.00,0.05) | 0.00 | (0.00,0.02) | 0.01 | (0.00,0.02) |
| South End | Hale | 0.01 | (0.00,0.03) | 0.01 | (0.00,0.04) | 0.01 | (0.00,0.03) |
| South End | Harvard/Kent | 0.01 | (0.00,0.03) | 0.00 | (0.00,0.01) | 0.00 | (0.00,0.01) |
| South End | Haynes | 0.13 | (0.07,0.19) | 0.01 | (0.00,0.04) | 0.02 | (0.00,0.04) |
| South End | Hernandez | | | 0.03 | (0.00,0.06) | 0.03 | (0.00,0.06) |
| South End | Higginson/Lewis | 0.01 | (0.00,0.03) | 0.01 | (0.00,0.03) | 0.01 | (0.00,0.03) |
| South End | Hurley | 0.38 | (0.29,0.47) | 0.15 | (0.09,0.22) | 0.15 | (0.09,0.22) |
| South End | Jackson/Mann | 0.02 | (0.00,0.05) | 0.02 | (0.00,0.04) | 0.02 | (0.00,0.04) |
| South End | Mason | 0.01 | (0.00,0.03) | 0.03 | (0.00,0.06) | 0.02 | (0.00,0.05) |
| South End | Orchard Gardens | 0.02 | (0.00,0.05) | 0.07 | (0.03,0.12) | 0.07 | (0.03,0.12) |
| South End | Quincy | 0.19 | (0.11,0.27) | 0.38 | (0.27,0.46) | 0.39 | (0.30,0.48) |
| South End | Russell | 0.06 | (0.02,0.11) | 0.00 | (0.00,0.02) | 0.00 | (0.00,0.02) |
| South End | Sumner | 0.01 | (0.00,0.03) | | | 0.00 | (0.00,0.01) |
| South End | Tobin | | | 0.02 | (0.00,0.06) | 0.02 | (0.00,0.05) |
| South End | Tynan | | | 0.00 | (0.00,0.02) | 0.00 | (0.00,0.02) |
| South End | West Zone ELC | | | 0.01 | (0.00,0.03) | 0.01 | (0.00,0.04) |
| South End | Winship | 0.01 | (0.00,0.03) | | | | |
| South End | Winthrop | 0.01 | (0.00,0.03) | 0.01 | (0.00,0.03) | 0.01 | (0.00,0.03) |
| West Roxbury | BTU | 0.01 | (0.00,0.03) | 0.01 | (0.00,0.03) | 0.01 | (0.00,0.03) |
| West Roxbury | Baldwin | | | 0.00 | (0.00,0.01) | 0.00 | (0.00,0.01) |
| West Roxbury | Bates | 0.04 | (0.01,0.06) | 0.04 | (0.02,0.07) | 0.04 | (0.02,0.07) |
| West Roxbury | Beethoven | 0.09 | (0.05,0.13) | 0.21 | (0.16,0.26) | 0.21 | (0.16,0.26) |
| West Roxbury | Channing | 0.01 | (0.00,0.02) | 0.03 | (0.01,0.06) | 0.04 | (0.02,0.07) |
| West Roxbury | Conley | 0.02 | (0.00,0.03) | 0.02 | (0.00,0.04) | 0.02 | (0.00,0.03) |
| West Roxbury | Curley | 0.00 | (0.00,0.02) | | | | |
| West Roxbury | Ellison/Parks | | | 0.01 | (0.00,0.02) | 0.01 | (0.00,0.02) |
| West Roxbury | Haley | 0.01 | (0.00,0.01) | | | | |
| West Roxbury | Haynes | 0.01 | (0.00,0.02) | | | | |
| West Roxbury | Henderson | 0.01 | (0.00,0.02) | | | | |
| West Roxbury | Hernandez | 0.00 | (0.00,0.01) | 0.01 | (0.00,0.02) | 0.02 | (0.00,0.03) |
| West Roxbury | J.F. Kennedy | 0.01 | (0.00,0.03) | | | | |
| West Roxbury | Kilmer | 0.31 | (0.26,0.37) | 0.30 | (0.25,0.36) | 0.33 | (0.26,0.39) |
| West Roxbury | Lyndon | 0.34 | (0.28,0.40) | 0.22 | (0.18,0.27) | 0.20 | (0.14,0.26) |
| West Roxbury | Manning | 0.03 | (0.01,0.06) | 0.02 | (0.01,0.04) | 0.02 | (0.00,0.04) |

Continued on next page

**Table 10 – continued from previous page**

| Neighborhood | School | Naive mean | Naive (95% C.I.) | Logit mean | Logit (95% C.I.) | Mixed Logit mean | Mixed Logit (95% C.I.) |
|---|---|---|---|---|---|---|---|
| West Roxbury | Mendell | 0.00 | (0.00,0.02) | | | | |
| West Roxbury | Mission Hill | 0.01 | (0.00,0.03) | 0.00 | (0.00,0.01) | 0.00 | (0.00,0.01) |
| West Roxbury | Mozart | 0.01 | (0.00,0.03) | 0.06 | (0.03,0.09) | 0.05 | (0.03,0.09) |
| West Roxbury | Philbrick | 0.01 | (0.00,0.02) | | | | |
| West Roxbury | Roosevelt | | | 0.02 | (0.01,0.04) | 0.02 | (0.01,0.05) |
| West Roxbury | Sumner | 0.07 | (0.04,0.10) | 0.02 | (0.00,0.03) | 0.02 | (0.00,0.04) |
| West Roxbury | Taylor | 0.00 | (0.00,0.02) | | | | |
| West Roxbury | West Zone ELC | 0.01 | (0.00,0.01) | | | | |

Table 11: Top 2 Choices Market Share Predictions for 2014 K1

| Neighborhood | School | Naive mean | Naive (95% C.I.) | Logit mean | Logit (95% C.I.) | Mixed Logit mean | Mixed Logit (95% C.I.) |
|---|---|---|---|---|---|---|---|
| Allston-Brighton | Baldwin | 0.07 | (0.06,0.09) | 0.23 | (0.18,0.27) | 0.23 | (0.18,0.27) |
| Allston-Brighton | Blackstone | 0.01 | (0.00,0.03) | 0.01 | (0.00,0.03) | 0.01 | (0.00,0.03) |
| Allston-Brighton | Curley | 0.01 | (0.00,0.01) | 0.02 | (0.01,0.05) | 0.02 | (0.01,0.04) |
| Allston-Brighton | Edison | 0.33 | (0.29,0.38) | 0.20 | (0.15,0.26) | 0.19 | (0.14,0.25) |
| Allston-Brighton | Gardner | 0.03 | (0.01,0.05) | 0.14 | (0.10,0.19) | 0.16 | (0.12,0.20) |
| Allston-Brighton | Hale | 0.06 | (0.04,0.09) | | | | |
| Allston-Brighton | Hernandez | 0.06 | (0.03,0.10) | 0.03 | (0.01,0.05) | 0.03 | (0.01,0.06) |
| Allston-Brighton | Hurley | 0.03 | (0.01,0.06) | 0.00 | (0.00,0.01) | 0.00 | (0.00,0.01) |
| Allston-Brighton | J.F. Kennedy | 0.01 | (0.00,0.01) | 0.00 | (0.00,0.01) | | |
| Allston-Brighton | Jackson/Mann | 0.15 | (0.09,0.20) | 0.17 | (0.13,0.23) | 0.17 | (0.12,0.22) |
| Allston-Brighton | Manning | 0.20 | (0.16,0.24) | 0.01 | (0.00,0.02) | 0.01 | (0.00,0.02) |
| Allston-Brighton | Mendell | | | 0.01 | (0.00,0.02) | 0.01 | (0.00,0.02) |
| Allston-Brighton | Tobin | | | 0.01 | (0.00,0.02) | 0.01 | (0.00,0.02) |
| Allston-Brighton | Winship | 0.03 | (0.02,0.06) | 0.16 | (0.12,0.20) | 0.16 | (0.11,0.20) |
| Charlestown | Adams | 0.05 | (0.02,0.08) | 0.00 | (0.00,0.01) | 0.00 | (0.00,0.01) |
| Charlestown | Baldwin | 0.02 | (0.00,0.03) | 0.01 | (0.00,0.02) | 0.01 | (0.00,0.02) |
| Charlestown | Blackstone | 0.02 | (0.00,0.05) | 0.03 | (0.01,0.06) | 0.03 | (0.01,0.06) |
| Charlestown | East Boston EEC | | | 0.02 | (0.00,0.05) | 0.03 | (0.01,0.07) |
| Charlestown | Eliot | 0.41 | (0.35,0.46) | 0.47 | (0.40,0.54) | 0.48 | (0.41,0.56) |
| Charlestown | Harvard/Kent | 0.42 | (0.38,0.47) | 0.26 | (0.21,0.33) | 0.26 | (0.20,0.32) |
| Charlestown | Hernandez | 0.02 | (0.00,0.04) | 0.01 | (0.00,0.02) | 0.01 | (0.00,0.03) |
| Charlestown | O'Donnell | | | 0.02 | (0.00,0.04) | 0.01 | (0.00,0.03) |
| Charlestown | Otis | 0.06 | (0.03,0.10) | 0.02 | (0.00,0.04) | 0.02 | (0.00,0.04) |
| Charlestown | Quincy | 0.02 | (0.00,0.05) | 0.15 | (0.10,0.20) | 0.14 | (0.09,0.20) |
| Charlestown | Tynan | | | 0.01 | (0.00,0.03) | 0.01 | (0.00,0.02) |
| Downtown | Adams | 0.06 | (0.03,0.10) | | | 0.00 | (0.00,0.01) |
| Downtown | Baldwin | 0.01 | (0.00,0.01) | 0.01 | (0.00,0.01) | 0.00 | (0.00,0.01) |
| Downtown | Blackstone | | | 0.06 | (0.03,0.10) | 0.05 | (0.02,0.09) |
| Downtown | Condon | | | 0.02 | (0.00,0.04) | 0.02 | (0.00,0.04) |
| Downtown | Curley | | | 0.01 | (0.00,0.02) | 0.00 | (0.00,0.02) |
| Downtown | Dever | 0.01 | (0.00,0.02) | | | | |
| Downtown | East Boston EEC | | | 0.01 | (0.00,0.02) | 0.02 | (0.00,0.04) |
| Downtown | Edison | 0.10 | (0.06,0.15) | 0.01 | (0.00,0.02) | 0.01 | (0.00,0.03) |
| Downtown | Eliot | 0.34 | (0.25,0.44) | 0.39 | (0.31,0.47) | 0.39 | (0.31,0.48) |
| Downtown | Gardner | | | 0.00 | (0.00,0.01) | 0.00 | (0.00,0.01) |
| Downtown | Hale | 0.01 | (0.00,0.03) | 0.01 | (0.00,0.02) | 0.00 | (0.00,0.02) |
| Downtown | Harvard/Kent | 0.01 | (0.00,0.04) | 0.04 | (0.01,0.07) | 0.03 | (0.01,0.06) |
| Downtown | Haynes | 0.01 | (0.00,0.02) | | | | |
| Downtown | Hernandez | 0.02 | (0.00,0.04) | 0.02 | (0.00,0.04) | 0.02 | (0.00,0.04) |

Continued on next page

**Table 11 – continued from previous page**

| | | Naive | | Logit | | Mixed Logit | |
|---|---|---|---|---|---|---|---|
| Neighborhood | School | mean | (95% C.I.) | mean | (95% C.I.) | mean | (95% C.I.) |
| Downtown | Hurley | 0.10 | (0.06,0.15) | 0.06 | (0.02,0.09) | 0.05 | (0.02,0.09) |
| Downtown | J.F. Kennedy | | | 0.00 | (0.00,0.01) | 0.00 | (0.00,0.01) |
| Downtown | Jackson/Mann | | | 0.01 | (0.00,0.02) | 0.01 | (0.00,0.02) |
| Downtown | Mason | | | 0.01 | (0.00,0.02) | 0.00 | (0.00,0.02) |
| Downtown | Orchard Gardens | 0.01 | (0.00,0.02) | 0.02 | (0.01,0.05) | 0.02 | (0.01,0.04) |
| Downtown | Otis | 0.05 | (0.02,0.09) | 0.00 | (0.00,0.01) | 0.00 | (0.00,0.01) |
| Downtown | Quincy | 0.27 | (0.20,0.35) | 0.31 | (0.24,0.39) | 0.32 | (0.24,0.40) |
| Downtown | Russell | 0.01 | (0.00,0.02) | | | | |
| Downtown | Tobin | | | 0.01 | (0.00,0.03) | 0.01 | (0.00,0.03) |
| Downtown | Tynan | | | 0.01 | (0.00,0.03) | 0.01 | (0.00,0.03) |
| Downtown | West Zone ELC | | | 0.01 | (0.00,0.03) | 0.01 | (0.00,0.03) |
| East Boston | Adams | 0.35 | (0.32,0.38) | 0.13 | (0.10,0.16) | 0.12 | (0.09,0.14) |
| East Boston | Blackstone | 0.02 | (0.01,0.04) | 0.01 | (0.00,0.01) | 0.01 | (0.00,0.02) |
| East Boston | Bradley | 0.07 | (0.05,0.10) | 0.16 | (0.12,0.19) | 0.18 | (0.14,0.21) |
| East Boston | East Boston EEC | 0.06 | (0.04,0.08) | 0.25 | (0.22,0.29) | 0.25 | (0.22,0.29) |
| East Boston | Edison | 0.00 | (0.00,0.01) | | | | |
| East Boston | Eliot | | | 0.01 | (0.01,0.02) | 0.01 | (0.01,0.02) |
| East Boston | Harvard/Kent | 0.01 | (0.00,0.01) | 0.01 | (0.00,0.01) | 0.01 | (0.00,0.01) |
| East Boston | Hernandez | 0.21 | (0.18,0.24) | 0.01 | (0.00,0.01) | 0.02 | (0.01,0.04) |
| East Boston | Hurley | 0.00 | (0.00,0.01) | | | | |
| East Boston | Jackson/Mann | 0.01 | (0.00,0.02) | | | | |
| East Boston | Kennedy Patrick | 0.01 | (0.01,0.02) | 0.11 | (0.09,0.14) | 0.10 | (0.08,0.12) |
| East Boston | O'Donnell | 0.01 | (0.01,0.02) | 0.09 | (0.07,0.12) | 0.08 | (0.06,0.10) |
| East Boston | Otis | 0.20 | (0.17,0.24) | 0.22 | (0.18,0.26) | 0.21 | (0.17,0.24) |
| East Boston | Quincy | 0.01 | (0.00,0.02) | | | | |
| East Boston | Tynan | | | | | 0.00 | (0.00,0.01) |
| Hyde Park | Bates | | | 0.07 | (0.05,0.10) | 0.06 | (0.04,0.09) |
| Hyde Park | Beethoven | 0.01 | (0.00,0.01) | 0.11 | (0.08,0.13) | 0.10 | (0.07,0.12) |
| Hyde Park | Channing | 0.01 | (0.00,0.02) | 0.08 | (0.06,0.11) | 0.09 | (0.07,0.12) |
| Hyde Park | Chittick | 0.06 | (0.03,0.09) | 0.08 | (0.05,0.11) | 0.07 | (0.04,0.10) |
| Hyde Park | Clap | 0.01 | (0.00,0.02) | | | | |
| Hyde Park | Condon | 0.01 | (0.00,0.02) | | | | |
| Hyde Park | Conley | 0.34 | (0.31,0.37) | 0.09 | (0.06,0.12) | 0.09 | (0.06,0.12) |
| Hyde Park | Ellison/Parks | | | 0.06 | (0.04,0.08) | 0.05 | (0.03,0.08) |
| Hyde Park | Haley | | | 0.04 | (0.02,0.05) | 0.04 | (0.02,0.07) |
| Hyde Park | Hernandez | 0.06 | (0.03,0.08) | 0.04 | (0.02,0.06) | 0.04 | (0.02,0.06) |
| Hyde Park | Kilmer | 0.03 | (0.01,0.05) | 0.04 | (0.03,0.07) | 0.05 | (0.03,0.07) |
| Hyde Park | Lee | 0.00 | (0.00,0.01) | | | | |
| Hyde Park | Mattahunt | 0.02 | (0.00,0.04) | 0.03 | (0.02,0.05) | 0.04 | (0.02,0.06) |
| Hyde Park | Mozart | | | 0.05 | (0.03,0.08) | 0.05 | (0.03,0.07) |
| Hyde Park | Philbrick | 0.13 | (0.10,0.16) | 0.04 | (0.02,0.07) | 0.03 | (0.02,0.06) |
| Hyde Park | Roosevelt | 0.23 | (0.19,0.26) | 0.19 | (0.16,0.23) | 0.20 | (0.17,0.24) |
| Hyde Park | S. Greenwood | 0.01 | (0.00,0.02) | | | | |
| Hyde Park | Sumner | 0.03 | (0.01,0.05) | 0.02 | (0.01,0.04) | 0.02 | (0.01,0.04) |
| Hyde Park | Taylor | | | 0.00 | (0.00,0.01) | 0.00 | (0.00,0.01) |
| Hyde Park | Young Achievers | 0.05 | (0.03,0.08) | 0.03 | (0.01,0.05) | 0.03 | (0.02,0.05) |
| Jamaica Plain | BTU | 0.01 | (0.00,0.02) | 0.07 | (0.05,0.10) | 0.06 | (0.04,0.09) |
| Jamaica Plain | Bates | 0.00 | (0.00,0.01) | | | | |
| Jamaica Plain | Blackstone | 0.01 | (0.00,0.01) | 0.01 | (0.00,0.01) | 0.01 | (0.00,0.01) |
| Jamaica Plain | Curley | 0.11 | (0.07,0.15) | 0.26 | (0.21,0.30) | 0.25 | (0.21,0.30) |
| Jamaica Plain | Ellis | 0.02 | (0.00,0.03) | 0.03 | (0.01,0.05) | 0.03 | (0.01,0.04) |
| Jamaica Plain | Ellison/Parks | 0.02 | (0.01,0.04) | 0.00 | (0.00,0.01) | 0.01 | (0.00,0.01) |
| Jamaica Plain | Hale | 0.24 | (0.21,0.28) | 0.02 | (0.01,0.03) | 0.02 | (0.01,0.03) |
| Jamaica Plain | Haley | | | 0.01 | (0.00,0.02) | 0.01 | (0.00,0.02) |
| Jamaica Plain | Hernandez | 0.01 | (0.00,0.02) | 0.07 | (0.04,0.10) | 0.09 | (0.06,0.12) |

Continued on next page

**Table 11 – continued from previous page**

| Neighborhood | School | Naive mean | Naive (95% C.I.) | Logit mean | Logit (95% C.I.) | Mixed Logit mean | Mixed Logit (95% C.I.) |
|---|---|---|---|---|---|---|---|
| Jamaica Plain | Higginson/Lewis | | | 0.01 | (0.00,0.01) | 0.00 | (0.00,0.01) |
| Jamaica Plain | Hurley | 0.09 | (0.07,0.12) | 0.03 | (0.01,0.05) | 0.03 | (0.02,0.05) |
| Jamaica Plain | J.F. Kennedy | 0.01 | (0.00,0.02) | 0.06 | (0.04,0.09) | 0.06 | (0.03,0.08) |
| Jamaica Plain | Jackson/Mann | 0.01 | (0.00,0.03) | 0.03 | (0.01,0.05) | 0.03 | (0.02,0.06) |
| Jamaica Plain | Kilmer | 0.00 | (0.00,0.01) | | | | |
| Jamaica Plain | Manning | 0.25 | (0.21,0.28) | 0.08 | (0.06,0.11) | 0.08 | (0.06,0.11) |
| Jamaica Plain | Mason | 0.04 | (0.02,0.06) | 0.00 | (0.00,0.01) | 0.00 | (0.00,0.01) |
| Jamaica Plain | Mendell | 0.01 | (0.00,0.02) | 0.06 | (0.04,0.08) | 0.05 | (0.03,0.07) |
| Jamaica Plain | Mission Hill | 0.02 | (0.01,0.03) | 0.12 | (0.09,0.15) | 0.12 | (0.09,0.15) |
| Jamaica Plain | Orchard Gardens | | | 0.02 | (0.01,0.04) | 0.02 | (0.01,0.04) |
| Jamaica Plain | Philbrick | 0.06 | (0.04,0.08) | 0.01 | (0.00,0.02) | 0.01 | (0.00,0.02) |
| Jamaica Plain | Quincy | 0.00 | (0.00,0.02) | 0.00 | (0.00,0.01) | 0.00 | (0.00,0.01) |
| Jamaica Plain | S. Greenwood | 0.01 | (0.00,0.03) | | | 0.00 | (0.00,0.01) |
| Jamaica Plain | Sumner | 0.04 | (0.02,0.06) | | | | |
| Jamaica Plain | Tobin | 0.01 | (0.00,0.02) | 0.03 | (0.02,0.05) | 0.03 | (0.02,0.05) |
| Jamaica Plain | Trotter | | | 0.01 | (0.00,0.01) | 0.01 | (0.00,0.01) |
| Jamaica Plain | West Zone ELC | | | 0.05 | (0.03,0.07) | 0.06 | (0.04,0.08) |
| Mattapan | BTU | 0.01 | (0.00,0.01) | 0.05 | (0.03,0.07) | 0.05 | (0.03,0.07) |
| Mattapan | Channing | 0.01 | (0.00,0.02) | 0.01 | (0.00,0.02) | 0.01 | (0.00,0.02) |
| Mattapan | Chittick | 0.01 | (0.00,0.02) | 0.03 | (0.01,0.05) | 0.03 | (0.01,0.04) |
| Mattapan | Clap | 0.01 | (0.00,0.02) | | | | |
| Mattapan | Condon | 0.01 | (0.00,0.02) | | | | |
| Mattapan | Conley | 0.06 | (0.04,0.09) | 0.01 | (0.00,0.02) | 0.01 | (0.00,0.02) |
| Mattapan | Curley | 0.01 | (0.00,0.02) | 0.00 | (0.00,0.01) | 0.00 | (0.00,0.01) |
| Mattapan | Dever | 0.03 | (0.01,0.06) | 0.01 | (0.00,0.03) | 0.01 | (0.00,0.03) |
| Mattapan | Ellison/Parks | 0.07 | (0.04,0.10) | 0.13 | (0.10,0.17) | 0.14 | (0.11,0.17) |
| Mattapan | Haley | 0.01 | (0.00,0.02) | 0.09 | (0.06,0.11) | 0.08 | (0.05,0.11) |
| Mattapan | Henderson | 0.25 | (0.22,0.28) | 0.03 | (0.01,0.04) | 0.03 | (0.01,0.05) |
| Mattapan | Hernandez | 0.03 | (0.02,0.05) | 0.05 | (0.03,0.08) | 0.05 | (0.03,0.08) |
| Mattapan | Holland | 0.01 | (0.00,0.01) | | | | |
| Mattapan | Holmes | | | 0.01 | (0.00,0.03) | 0.01 | (0.00,0.02) |
| Mattapan | Jackson/Mann | | | 0.01 | (0.00,0.02) | 0.02 | (0.01,0.03) |
| Mattapan | Kenny | 0.01 | (0.00,0.02) | 0.01 | (0.00,0.02) | 0.01 | (0.00,0.02) |
| Mattapan | Lee | 0.01 | (0.00,0.03) | 0.07 | (0.01,0.13) | 0.06 | (0.01,0.13) |
| Mattapan | Mason | 0.00 | (0.00,0.01) | | | | |
| Mattapan | Mather | 0.01 | (0.00,0.01) | | | | |
| Mattapan | Mattahunt | 0.02 | (0.01,0.04) | 0.05 | (0.03,0.08) | 0.05 | (0.03,0.08) |
| Mattapan | Murphy | 0.04 | (0.02,0.06) | 0.03 | (0.02,0.05) | 0.04 | (0.02,0.06) |
| Mattapan | Otis | 0.01 | (0.00,0.02) | | | | |
| Mattapan | Philbrick | 0.21 | (0.18,0.25) | 0.03 | (0.02,0.05) | 0.03 | (0.01,0.05) |
| Mattapan | Roosevelt | 0.00 | (0.00,0.01) | | | | |
| Mattapan | Russell | 0.01 | (0.00,0.02) | 0.00 | (0.00,0.01) | 0.00 | (0.00,0.01) |
| Mattapan | S. Greenwood | 0.04 | (0.02,0.06) | 0.06 | (0.03,0.08) | 0.06 | (0.04,0.08) |
| Mattapan | Sumner | 0.03 | (0.01,0.05) | 0.01 | (0.00,0.02) | 0.01 | (0.00,0.02) |
| Mattapan | Taylor | 0.03 | (0.01,0.04) | 0.06 | (0.04,0.09) | 0.06 | (0.04,0.08) |
| Mattapan | Tobin | 0.00 | (0.00,0.01) | | | | |
| Mattapan | Young Achievers | 0.03 | (0.01,0.05) | 0.16 | (0.12,0.20) | 0.16 | (0.12,0.20) |
| North Dorchester | Adams | 0.00 | (0.00,0.01) | | | | |
| North Dorchester | Blackstone | | | 0.01 | (0.00,0.02) | 0.01 | (0.00,0.02) |
| North Dorchester | Clap | 0.03 | (0.01,0.05) | 0.18 | (0.14,0.22) | 0.17 | (0.13,0.22) |
| North Dorchester | Condon | 0.05 | (0.01,0.08) | 0.03 | (0.01,0.05) | 0.03 | (0.01,0.05) |
| North Dorchester | Dever | 0.05 | (0.03,0.07) | 0.08 | (0.05,0.11) | 0.07 | (0.04,0.10) |
| North Dorchester | Edison | 0.00 | (0.00,0.01) | | | | |
| North Dorchester | Ellison/Parks | 0.02 | (0.01,0.04) | 0.00 | (0.00,0.01) | 0.01 | (0.00,0.01) |
| North Dorchester | Everett | 0.01 | (0.00,0.02) | 0.12 | (0.08,0.15) | 0.12 | (0.08,0.15) |

Continued on next page

**Table 11 – continued from previous page**

| Neighborhood | School | Naive mean | Naive (95% C.I.) | Logit mean | Logit (95% C.I.) | Mixed Logit mean | Mixed Logit (95% C.I.) |
|---|---|---|---|---|---|---|---|
| North Dorchester | Hale | 0.02 | (0.01,0.03) | | | 0.00 | (0.00,0.01) |
| North Dorchester | Harvard/Kent | 0.01 | (0.00,0.02) | | | | |
| North Dorchester | Haynes | 0.18 | (0.14,0.22) | 0.07 | (0.04,0.11) | 0.08 | (0.05,0.12) |
| North Dorchester | Henderson | 0.10 | (0.07,0.12) | 0.03 | (0.01,0.05) | 0.03 | (0.02,0.06) |
| North Dorchester | Hernandez | | | 0.04 | (0.02,0.06) | 0.04 | (0.02,0.06) |
| North Dorchester | Higginson/Lewis | 0.00 | (0.00,0.01) | | | | |
| North Dorchester | Holland | 0.02 | (0.00,0.04) | 0.04 | (0.01,0.06) | 0.03 | (0.01,0.05) |
| North Dorchester | Hurley | 0.03 | (0.01,0.05) | 0.01 | (0.00,0.03) | 0.01 | (0.00,0.03) |
| North Dorchester | Jackson/Mann | | | 0.01 | (0.00,0.03) | 0.02 | (0.01,0.04) |
| North Dorchester | King | | | 0.03 | (0.01,0.05) | 0.02 | (0.01,0.04) |
| North Dorchester | Lee | 0.01 | (0.00,0.01) | | | 0.00 | (0.00,0.01) |
| North Dorchester | Mason | 0.30 | (0.27,0.34) | 0.04 | (0.02,0.07) | 0.04 | (0.02,0.07) |
| North Dorchester | Mather | 0.02 | (0.00,0.04) | 0.07 | (0.04,0.10) | 0.08 | (0.05,0.11) |
| North Dorchester | Murphy | 0.05 | (0.02,0.09) | 0.04 | (0.02,0.07) | 0.04 | (0.02,0.08) |
| North Dorchester | Orchard Gardens | 0.00 | (0.00,0.01) | 0.04 | (0.02,0.06) | 0.04 | (0.02,0.07) |
| North Dorchester | Perry | 0.00 | (0.00,0.01) | 0.01 | (0.00,0.02) | 0.01 | (0.00,0.02) |
| North Dorchester | Russell | 0.05 | (0.02,0.07) | 0.09 | (0.06,0.12) | 0.09 | (0.06,0.12) |
| North Dorchester | S. Greenwood | 0.01 | (0.00,0.02) | 0.00 | (0.00,0.01) | 0.00 | (0.00,0.01) |
| North Dorchester | Taylor | 0.00 | (0.00,0.01) | | | | |
| North Dorchester | Tobin | 0.00 | (0.00,0.01) | | | | |
| North Dorchester | Tynan | 0.01 | (0.00,0.02) | 0.01 | (0.00,0.02) | 0.01 | (0.00,0.02) |
| North Dorchester | Winship | 0.00 | (0.00,0.01) | | | | |
| North Dorchester | Winthrop | 0.00 | (0.00,0.01) | 0.03 | (0.01,0.05) | 0.02 | (0.01,0.04) |
| North Dorchester | Young Achievers | 0.01 | (0.00,0.02) | 0.00 | (0.00,0.01) | 0.00 | (0.00,0.01) |
| Roslindale | BTU | 0.01 | (0.00,0.01) | 0.13 | (0.10,0.16) | 0.13 | (0.10,0.16) |
| Roslindale | Bates | 0.01 | (0.00,0.02) | 0.11 | (0.08,0.13) | 0.11 | (0.08,0.13) |
| Roslindale | Beethoven | 0.01 | (0.00,0.02) | 0.02 | (0.01,0.03) | 0.02 | (0.01,0.03) |
| Roslindale | Channing | | | 0.00 | (0.00,0.01) | 0.01 | (0.00,0.01) |
| Roslindale | Chittick | 0.00 | (0.00,0.01) | 0.01 | (0.00,0.03) | 0.01 | (0.00,0.02) |
| Roslindale | Conley | 0.16 | (0.13,0.19) | 0.08 | (0.06,0.10) | 0.07 | (0.05,0.09) |
| Roslindale | Curley | 0.02 | (0.01,0.04) | 0.02 | (0.01,0.03) | 0.02 | (0.01,0.03) |
| Roslindale | East Boston EEC | 0.00 | (0.00,0.01) | | | | |
| Roslindale | Ellis | 0.00 | (0.00,0.01) | | | | |
| Roslindale | Ellison/Parks | | | 0.02 | (0.01,0.04) | 0.02 | (0.01,0.04) |
| Roslindale | Haley | 0.02 | (0.01,0.03) | 0.08 | (0.06,0.10) | 0.08 | (0.06,0.11) |
| Roslindale | Hernandez | 0.03 | (0.01,0.04) | 0.04 | (0.03,0.06) | 0.05 | (0.03,0.07) |
| Roslindale | Jackson/Mann | 0.00 | (0.00,0.01) | | | | |
| Roslindale | Kenny | 0.00 | (0.00,0.01) | | | | |
| Roslindale | Kilmer | 0.02 | (0.01,0.03) | 0.02 | (0.01,0.03) | 0.02 | (0.01,0.03) |
| Roslindale | King | 0.00 | (0.00,0.01) | | | | |
| Roslindale | Lyndon | 0.04 | (0.02,0.06) | 0.06 | (0.04,0.08) | 0.05 | (0.03,0.07) |
| Roslindale | Manning | 0.03 | (0.02,0.05) | 0.03 | (0.02,0.04) | 0.03 | (0.01,0.04) |
| Roslindale | Mason | 0.00 | (0.00,0.01) | | | | |
| Roslindale | Mattahunt | | | 0.03 | (0.01,0.04) | 0.03 | (0.02,0.05) |
| Roslindale | Mendell | 0.00 | (0.00,0.01) | | | 0.00 | (0.00,0.01) |
| Roslindale | Mission Hill | 0.01 | (0.00,0.01) | 0.02 | (0.01,0.04) | 0.02 | (0.01,0.04) |
| Roslindale | Mozart | 0.02 | (0.01,0.04) | 0.11 | (0.08,0.13) | 0.11 | (0.08,0.14) |
| Roslindale | Philbrick | 0.20 | (0.17,0.23) | 0.10 | (0.07,0.12) | 0.08 | (0.06,0.11) |
| Roslindale | Sumner | 0.36 | (0.33,0.39) | 0.09 | (0.07,0.11) | 0.09 | (0.06,0.12) |
| Roslindale | Young Achievers | 0.02 | (0.01,0.03) | 0.03 | (0.02,0.05) | 0.04 | (0.02,0.05) |
| Roxbury | BTU | | | 0.01 | (0.00,0.01) | 0.01 | (0.00,0.01) |
| Roxbury | Blackstone | | | 0.02 | (0.01,0.04) | 0.02 | (0.01,0.04) |
| Roxbury | Clap | 0.00 | (0.00,0.01) | 0.03 | (0.01,0.04) | 0.03 | (0.01,0.04) |
| Roxbury | Curley | 0.04 | (0.02,0.06) | 0.07 | (0.05,0.09) | 0.06 | (0.04,0.08) |
| Roxbury | Dever | 0.02 | (0.01,0.03) | 0.01 | (0.00,0.02) | 0.01 | (0.00,0.02) |

Continued on next page

**Table 11 – continued from previous page**

| Neighborhood | School | Naive mean | Naive (95% C.I.) | Logit mean | Logit (95% C.I.) | Mixed Logit mean | Mixed Logit (95% C.I.) |
|---|---|---|---|---|---|---|---|
| Roxbury | Edison | 0.00 | (0.00,0.01) | | | | |
| Roxbury | Eliot | 0.00 | (0.00,0.01) | | | | |
| Roxbury | Ellis | 0.01 | (0.01,0.03) | 0.04 | (0.03,0.06) | 0.04 | (0.03,0.06) |
| Roxbury | Ellison/Parks | 0.01 | (0.00,0.02) | 0.01 | (0.00,0.01) | 0.01 | (0.00,0.01) |
| Roxbury | Everett | | | 0.03 | (0.01,0.04) | 0.03 | (0.01,0.04) |
| Roxbury | Hale | 0.23 | (0.21,0.26) | 0.03 | (0.02,0.05) | 0.03 | (0.02,0.04) |
| Roxbury | Haley | 0.01 | (0.00,0.02) | 0.01 | (0.00,0.02) | 0.01 | (0.00,0.01) |
| Roxbury | Haynes | 0.06 | (0.05,0.08) | 0.07 | (0.05,0.09) | 0.08 | (0.05,0.10) |
| Roxbury | Henderson | 0.05 | (0.03,0.07) | 0.01 | (0.00,0.01) | 0.01 | (0.00,0.02) |
| Roxbury | Hernandez | 0.02 | (0.01,0.04) | 0.09 | (0.07,0.11) | 0.11 | (0.09,0.13) |
| Roxbury | Higginson/Lewis | 0.01 | (0.00,0.01) | 0.02 | (0.01,0.04) | 0.02 | (0.01,0.03) |
| Roxbury | Holland | 0.01 | (0.00,0.02) | 0.03 | (0.02,0.04) | 0.03 | (0.02,0.04) |
| Roxbury | Holmes | | | 0.01 | (0.00,0.02) | 0.01 | (0.00,0.02) |
| Roxbury | Hurley | 0.06 | (0.04,0.08) | 0.03 | (0.02,0.04) | 0.03 | (0.02,0.04) |
| Roxbury | J.F. Kennedy | 0.01 | (0.00,0.02) | 0.03 | (0.02,0.05) | 0.03 | (0.02,0.05) |
| Roxbury | Jackson/Mann | 0.01 | (0.00,0.02) | 0.03 | (0.02,0.04) | 0.03 | (0.02,0.05) |
| Roxbury | King | 0.01 | (0.00,0.02) | 0.03 | (0.02,0.05) | 0.03 | (0.02,0.04) |
| Roxbury | Lee | | | 0.01 | (0.00,0.02) | 0.01 | (0.00,0.02) |
| Roxbury | Manning | 0.01 | (0.01,0.02) | | | | |
| Roxbury | Mason | 0.22 | (0.19,0.24) | 0.03 | (0.02,0.05) | 0.03 | (0.02,0.05) |
| Roxbury | Mather | 0.01 | (0.00,0.01) | 0.02 | (0.01,0.03) | 0.02 | (0.01,0.03) |
| Roxbury | Mattahunt | 0.00 | (0.00,0.01) | | | | |
| Roxbury | Mendell | | | 0.03 | (0.01,0.04) | 0.02 | (0.01,0.04) |
| Roxbury | Mission Hill | 0.01 | (0.00,0.01) | 0.03 | (0.02,0.04) | 0.03 | (0.02,0.04) |
| Roxbury | Murphy | 0.01 | (0.01,0.02) | 0.01 | (0.00,0.02) | 0.01 | (0.00,0.02) |
| Roxbury | Orchard Gardens | 0.01 | (0.00,0.02) | 0.06 | (0.04,0.07) | 0.05 | (0.04,0.07) |
| Roxbury | Philbrick | 0.00 | (0.00,0.01) | | | | |
| Roxbury | Quincy | 0.01 | (0.00,0.02) | | | 0.00 | (0.00,0.01) |
| Roxbury | Russell | 0.03 | (0.01,0.04) | 0.03 | (0.02,0.04) | 0.03 | (0.02,0.04) |
| Roxbury | S. Greenwood | 0.02 | (0.01,0.03) | 0.03 | (0.02,0.05) | 0.03 | (0.02,0.05) |
| Roxbury | Sumner | 0.01 | (0.00,0.01) | | | | |
| Roxbury | Tobin | | | 0.02 | (0.01,0.03) | 0.02 | (0.01,0.03) |
| Roxbury | Trotter | 0.02 | (0.01,0.03) | 0.04 | (0.02,0.05) | 0.04 | (0.03,0.06) |
| Roxbury | West Zone ELC | 0.01 | (0.00,0.01) | 0.02 | (0.01,0.03) | 0.02 | (0.01,0.03) |
| Roxbury | Winthrop | 0.01 | (0.00,0.02) | 0.03 | (0.02,0.04) | 0.03 | (0.01,0.04) |
| Roxbury | Young Achievers | 0.01 | (0.00,0.02) | 0.00 | (0.00,0.01) | 0.00 | (0.00,0.01) |
| South Boston | Blackstone | | | 0.05 | (0.02,0.09) | 0.05 | (0.02,0.09) |
| South Boston | Chittick | 0.01 | (0.00,0.04) | | | | |
| South Boston | Clap | 0.04 | (0.00,0.10) | 0.10 | (0.05,0.15) | 0.10 | (0.05,0.15) |
| South Boston | Condon | 0.10 | (0.04,0.17) | 0.18 | (0.12,0.24) | 0.17 | (0.11,0.23) |
| South Boston | Dever | 0.05 | (0.02,0.09) | 0.06 | (0.03,0.10) | 0.06 | (0.03,0.10) |
| South Boston | East Boston EEC | | | | | 0.00 | (0.00,0.02) |
| South Boston | Eliot | | | 0.02 | (0.00,0.05) | 0.02 | (0.00,0.05) |
| South Boston | Everett | | | 0.02 | (0.00,0.04) | 0.01 | (0.00,0.03) |
| South Boston | Haynes | 0.06 | (0.02,0.10) | 0.02 | (0.00,0.04) | 0.02 | (0.00,0.04) |
| South Boston | Hernandez | | | 0.02 | (0.00,0.05) | 0.02 | (0.01,0.05) |
| South Boston | Hurley | 0.04 | (0.01,0.08) | 0.03 | (0.01,0.06) | 0.03 | (0.01,0.05) |
| South Boston | Jackson/Mann | | | 0.01 | (0.00,0.03) | 0.01 | (0.00,0.03) |
| South Boston | Lee | 0.01 | (0.01,0.03) | | | | |
| South Boston | Manning | 0.01 | (0.00,0.03) | | | | |
| South Boston | Mason | 0.10 | (0.05,0.14) | 0.02 | (0.01,0.04) | 0.02 | (0.00,0.04) |
| South Boston | Mather | | | 0.00 | (0.00,0.02) | 0.00 | (0.00,0.02) |
| South Boston | Murphy | 0.03 | (0.00,0.07) | 0.01 | (0.00,0.04) | 0.01 | (0.00,0.03) |
| South Boston | Orchard Gardens | | | 0.02 | (0.00,0.04) | 0.02 | (0.01,0.05) |
| South Boston | Perry | 0.03 | (0.01,0.05) | 0.14 | (0.09,0.19) | 0.14 | (0.09,0.19) |

Continued on next page

**Table 11 – continued from previous page**

| Neighborhood | School | Naive mean | Naive (95% C.I.) | Logit mean | Logit (95% C.I.) | Mixed Logit mean | Mixed Logit (95% C.I.) |
|---|---|---|---|---|---|---|---|
| South Boston | Quincy | 0.44 | (0.34,0.55) | 0.18 | (0.11,0.24) | 0.18 | (0.12,0.26) |
| South Boston | Russell | 0.07 | (0.04,0.12) | 0.05 | (0.02,0.09) | 0.04 | (0.01,0.07) |
| South Boston | Tynan | | | 0.06 | (0.03,0.10) | 0.07 | (0.03,0.11) |
| South Boston | Winthrop | | | 0.00 | (0.00,0.01) | 0.00 | (0.00,0.01) |
| South Dorchester | Clap | 0.01 | (0.00,0.02) | 0.01 | (0.00,0.01) | 0.01 | (0.00,0.01) |
| South Dorchester | Condon | 0.02 | (0.01,0.04) | 0.01 | (0.00,0.01) | 0.01 | (0.00,0.01) |
| South Dorchester | Dever | 0.01 | (0.00,0.01) | | | | |
| South Dorchester | Ellison/Parks | 0.09 | (0.07,0.11) | 0.04 | (0.03,0.06) | 0.05 | (0.04,0.07) |
| South Dorchester | Everett | 0.01 | (0.00,0.01) | 0.03 | (0.02,0.04) | 0.02 | (0.01,0.04) |
| South Dorchester | Haynes | | | 0.02 | (0.01,0.03) | 0.02 | (0.01,0.04) |
| South Dorchester | Henderson | 0.27 | (0.24,0.29) | 0.09 | (0.07,0.12) | 0.08 | (0.07,0.10) |
| South Dorchester | Hernandez | 0.03 | (0.02,0.04) | 0.04 | (0.03,0.06) | 0.05 | (0.03,0.06) |
| South Dorchester | Holland | 0.05 | (0.04,0.07) | 0.05 | (0.04,0.07) | 0.05 | (0.04,0.07) |
| South Dorchester | Holmes | 0.01 | (0.00,0.01) | 0.03 | (0.02,0.04) | 0.03 | (0.02,0.04) |
| South Dorchester | Jackson/Mann | | | 0.01 | (0.00,0.02) | 0.02 | (0.01,0.03) |
| South Dorchester | Kenny | 0.01 | (0.01,0.02) | 0.04 | (0.02,0.05) | 0.03 | (0.02,0.04) |
| South Dorchester | King | | | 0.02 | (0.01,0.03) | 0.01 | (0.01,0.02) |
| South Dorchester | Lee | 0.01 | (0.00,0.02) | 0.05 | (0.01,0.10) | 0.04 | (0.01,0.09) |
| South Dorchester | Mason | 0.01 | (0.00,0.02) | | | | |
| South Dorchester | Mather | 0.07 | (0.05,0.09) | 0.07 | (0.05,0.09) | 0.07 | (0.05,0.09) |
| South Dorchester | Mattahunt | 0.01 | (0.00,0.03) | | | | |
| South Dorchester | Murphy | 0.29 | (0.25,0.32) | 0.32 | (0.29,0.35) | 0.33 | (0.30,0.38) |
| South Dorchester | Russell | 0.01 | (0.00,0.02) | 0.01 | (0.00,0.02) | 0.01 | (0.00,0.02) |
| South Dorchester | S. Greenwood | 0.04 | (0.02,0.05) | 0.05 | (0.04,0.07) | 0.05 | (0.03,0.06) |
| South Dorchester | Taylor | 0.02 | (0.01,0.03) | 0.02 | (0.01,0.03) | 0.02 | (0.01,0.03) |
| South Dorchester | Tynan | 0.01 | (0.00,0.02) | | | | |
| South Dorchester | Young Achievers | 0.01 | (0.00,0.02) | 0.02 | (0.01,0.03) | 0.02 | (0.01,0.03) |
| South End | Baldwin | 0.01 | (0.00,0.01) | 0.00 | (0.00,0.01) | 0.00 | (0.00,0.01) |
| South End | Blackstone | 0.03 | (0.01,0.07) | 0.15 | (0.10,0.20) | 0.14 | (0.10,0.20) |
| South End | Clap | | | 0.01 | (0.00,0.02) | 0.01 | (0.00,0.03) |
| South End | Condon | 0.01 | (0.00,0.03) | 0.05 | (0.02,0.07) | 0.04 | (0.01,0.07) |
| South End | Curley | 0.01 | (0.00,0.03) | 0.01 | (0.00,0.02) | 0.01 | (0.00,0.02) |
| South End | Dever | 0.03 | (0.01,0.05) | 0.00 | (0.00,0.01) | 0.01 | (0.00,0.02) |
| South End | Edison | 0.03 | (0.01,0.06) | 0.00 | (0.00,0.01) | 0.00 | (0.00,0.02) |
| South End | Eliot | 0.03 | (0.01,0.06) | 0.03 | (0.01,0.06) | 0.03 | (0.01,0.06) |
| South End | Gardner | 0.01 | (0.00,0.02) | 0.00 | (0.00,0.01) | 0.00 | (0.00,0.01) |
| South End | Hale | 0.03 | (0.01,0.06) | 0.01 | (0.00,0.03) | 0.01 | (0.00,0.03) |
| South End | Harvard/Kent | 0.00 | (0.00,0.01) | | | | |
| South End | Haynes | 0.07 | (0.04,0.10) | 0.01 | (0.00,0.03) | 0.02 | (0.00,0.04) |
| South End | Hernandez | | | 0.03 | (0.01,0.05) | 0.03 | (0.01,0.05) |
| South End | Higginson/Lewis | 0.00 | (0.00,0.02) | 0.01 | (0.00,0.02) | 0.01 | (0.00,0.02) |
| South End | Hurley | 0.27 | (0.23,0.32) | 0.14 | (0.10,0.20) | 0.14 | (0.10,0.18) |
| South End | Jackson/Mann | 0.02 | (0.00,0.05) | 0.02 | (0.00,0.04) | 0.02 | (0.00,0.04) |
| South End | Mason | 0.04 | (0.02,0.07) | 0.03 | (0.01,0.05) | 0.02 | (0.01,0.04) |
| South End | Orchard Gardens | 0.01 | (0.00,0.02) | 0.07 | (0.04,0.11) | 0.07 | (0.04,0.10) |
| South End | Quincy | 0.34 | (0.26,0.41) | 0.37 | (0.30,0.44) | 0.39 | (0.31,0.46) |
| South End | Russell | 0.03 | (0.01,0.05) | 0.00 | (0.00,0.01) | 0.00 | (0.00,0.02) |
| South End | Sumner | 0.00 | (0.00,0.02) | | | | |
| South End | Tobin | | | 0.02 | (0.01,0.05) | 0.02 | (0.00,0.04) |
| South End | Tynan | | | 0.00 | (0.00,0.01) | 0.00 | (0.00,0.01) |
| South End | West Zone ELC | | | 0.01 | (0.00,0.02) | 0.01 | (0.00,0.03) |
| South End | Winship | 0.00 | (0.00,0.01) | | | | |
| South End | Winthrop | 0.00 | (0.00,0.01) | 0.01 | (0.00,0.02) | 0.01 | (0.00,0.02) |
| West Roxbury | BTU | 0.01 | (0.00,0.02) | 0.01 | (0.00,0.02) | 0.01 | (0.00,0.02) |
| West Roxbury | Baldwin | | | | | 0.00 | (0.00,0.01) |

Continued on next page

**Table 11 – continued from previous page**

| Neighborhood | School | Naive mean | Naive (95% C.I.) | Logit mean | Logit (95% C.I.) | Mixed Logit mean | Mixed Logit (95% C.I.) |
|---|---|---|---|---|---|---|---|
| West Roxbury | Bates | 0.02 | (0.01,0.03) | 0.05 | (0.04,0.07) | 0.05 | (0.03,0.07) |
| West Roxbury | Beethoven | 0.04 | (0.03,0.06) | 0.19 | (0.16,0.23) | 0.19 | (0.16,0.22) |
| West Roxbury | Channing | 0.01 | (0.00,0.02) | 0.04 | (0.02,0.05) | 0.04 | (0.02,0.06) |
| West Roxbury | Conley | 0.02 | (0.01,0.03) | 0.02 | (0.01,0.04) | 0.02 | (0.01,0.03) |
| West Roxbury | Curley | 0.00 | (0.00,0.02) | | | | |
| West Roxbury | Ellison/Parks | | | 0.01 | (0.00,0.02) | 0.01 | (0.00,0.02) |
| West Roxbury | Hernandez | 0.02 | (0.01,0.03) | 0.01 | (0.01,0.02) | 0.02 | (0.01,0.03) |
| West Roxbury | J.F. Kennedy | 0.01 | (0.00,0.02) | | | | |
| West Roxbury | Kilmer | 0.33 | (0.30,0.36) | 0.27 | (0.24,0.31) | 0.28 | (0.25,0.32) |
| West Roxbury | Lyndon | 0.34 | (0.31,0.37) | 0.23 | (0.20,0.26) | 0.23 | (0.19,0.26) |
| West Roxbury | Manning | 0.03 | (0.01,0.04) | 0.02 | (0.01,0.04) | 0.02 | (0.01,0.04) |
| West Roxbury | Mission Hill | 0.01 | (0.00,0.01) | | | | |
| West Roxbury | Mozart | 0.01 | (0.00,0.02) | 0.07 | (0.05,0.10) | 0.07 | (0.05,0.09) |
| West Roxbury | Roosevelt | 0.04 | (0.03,0.07) | 0.02 | (0.01,0.04) | 0.03 | (0.01,0.04) |
| West Roxbury | Sumner | 0.09 | (0.07,0.12) | 0.02 | (0.01,0.03) | 0.02 | (0.01,0.03) |

Table 12: Top 3 Choices Market Share Predictions for 2014 K1

| Neighborhood | School | Naive mean | Naive (95% C.I.) | Logit mean | Logit (95% C.I.) | Mixed Logit mean | Mixed Logit (95% C.I.) |
|---|---|---|---|---|---|---|---|
| Allston-Brighton | Baldwin | 0.05 | (0.04,0.07) | 0.20 | (0.17,0.23) | 0.19 | (0.16,0.22) |
| Allston-Brighton | Blackstone | 0.01 | (0.00,0.03) | 0.01 | (0.00,0.03) | 0.01 | (0.00,0.03) |
| Allston-Brighton | Curley | 0.01 | (0.00,0.02) | 0.03 | (0.01,0.05) | 0.03 | (0.01,0.05) |
| Allston-Brighton | Edison | 0.30 | (0.26,0.34) | 0.21 | (0.17,0.24) | 0.20 | (0.16,0.24) |
| Allston-Brighton | Gardner | 0.02 | (0.01,0.03) | 0.14 | (0.11,0.17) | 0.16 | (0.13,0.19) |
| Allston-Brighton | Hale | 0.09 | (0.07,0.12) | | | | |
| Allston-Brighton | Hernandez | 0.05 | (0.03,0.08) | 0.03 | (0.01,0.05) | 0.03 | (0.01,0.05) |
| Allston-Brighton | Hurley | 0.03 | (0.01,0.04) | 0.00 | (0.00,0.01) | | |
| Allston-Brighton | J.F. Kennedy | 0.00 | (0.00,0.01) | | | | |
| Allston-Brighton | Jackson/Mann | 0.23 | (0.19,0.28) | 0.18 | (0.15,0.22) | 0.19 | (0.14,0.23) |
| Allston-Brighton | Manning | 0.16 | (0.13,0.19) | 0.01 | (0.00,0.02) | 0.01 | (0.00,0.02) |
| Allston-Brighton | Mendell | | | 0.01 | (0.00,0.02) | 0.01 | (0.00,0.02) |
| Allston-Brighton | Tobin | | | 0.01 | (0.00,0.02) | 0.01 | (0.00,0.02) |
| Allston-Brighton | Winship | 0.03 | (0.01,0.04) | 0.16 | (0.13,0.19) | 0.16 | (0.13,0.19) |
| Allston-Brighton | Winthrop | 0.00 | (0.00,0.01) | | | | |
| Charlestown | Adams | 0.06 | (0.03,0.08) | 0.00 | (0.00,0.01) | 0.00 | (0.00,0.01) |
| Charlestown | Baldwin | 0.01 | (0.00,0.02) | 0.01 | (0.00,0.01) | 0.01 | (0.00,0.01) |
| Charlestown | Blackstone | 0.02 | (0.00,0.05) | 0.03 | (0.01,0.06) | 0.03 | (0.01,0.06) |
| Charlestown | East Boston EEC | 0.02 | (0.00,0.03) | 0.03 | (0.01,0.05) | 0.04 | (0.01,0.06) |
| Charlestown | Eliot | 0.51 | (0.46,0.57) | 0.45 | (0.40,0.50) | 0.46 | (0.41,0.52) |
| Charlestown | Harvard/Kent | 0.30 | (0.27,0.33) | 0.25 | (0.21,0.29) | 0.25 | (0.20,0.28) |
| Charlestown | Hernandez | 0.02 | (0.00,0.03) | 0.01 | (0.00,0.02) | 0.01 | (0.00,0.02) |
| Charlestown | O'Donnell | | | 0.02 | (0.00,0.04) | 0.01 | (0.00,0.03) |
| Charlestown | Otis | 0.06 | (0.03,0.08) | 0.02 | (0.00,0.04) | 0.02 | (0.00,0.04) |
| Charlestown | Quincy | 0.01 | (0.00,0.03) | 0.17 | (0.13,0.22) | 0.16 | (0.11,0.21) |
| Charlestown | Tynan | | | 0.01 | (0.00,0.03) | 0.01 | (0.00,0.02) |
| Downtown | Adams | 0.04 | (0.02,0.07) | | | 0.00 | (0.00,0.01) |
| Downtown | Blackstone | 0.00 | (0.00,0.01) | 0.06 | (0.04,0.10) | 0.06 | (0.04,0.09) |
| Downtown | Condon | | | 0.03 | (0.01,0.04) | 0.02 | (0.01,0.04) |
| Downtown | Curley | | | 0.01 | (0.00,0.02) | 0.01 | (0.00,0.02) |
| Downtown | Dever | 0.00 | (0.00,0.01) | | | | |
| Downtown | East Boston EEC | 0.04 | (0.01,0.06) | 0.01 | (0.00,0.02) | 0.02 | (0.00,0.04) |

Continued on next page

**Table 12 – continued from previous page**

| Neighborhood | School | Naive mean | Naive (95% C.I.) | Logit mean | Logit (95% C.I.) | Mixed Logit mean | Mixed Logit (95% C.I.) |
|---|---|---|---|---|---|---|---|
| Downtown | Edison | 0.09 | (0.06,0.12) | 0.01 | (0.00,0.02) | 0.01 | (0.00,0.02) |
| Downtown | Eliot | 0.25 | (0.19,0.32) | 0.34 | (0.28,0.40) | 0.34 | (0.28,0.40) |
| Downtown | Hale | 0.02 | (0.00,0.03) | 0.01 | (0.00,0.02) | 0.01 | (0.00,0.01) |
| Downtown | Harvard/Kent | 0.06 | (0.04,0.09) | 0.05 | (0.03,0.08) | 0.05 | (0.02,0.07) |
| Downtown | Haynes | 0.00 | (0.00,0.01) | | | | |
| Downtown | Hernandez | 0.02 | (0.01,0.04) | 0.02 | (0.01,0.04) | 0.02 | (0.01,0.04) |
| Downtown | Hurley | 0.08 | (0.05,0.11) | 0.06 | (0.03,0.09) | 0.06 | (0.03,0.08) |
| Downtown | J.F. Kennedy | 0.01 | (0.00,0.02) | 0.00 | (0.00,0.01) | 0.00 | (0.00,0.01) |
| Downtown | Jackson/Mann | 0.00 | (0.00,0.01) | 0.01 | (0.00,0.02) | 0.01 | (0.00,0.02) |
| Downtown | Mason | | | 0.01 | (0.00,0.02) | 0.01 | (0.00,0.02) |
| Downtown | Orchard Gardens | 0.00 | (0.00,0.01) | 0.02 | (0.01,0.04) | 0.02 | (0.01,0.04) |
| Downtown | Otis | 0.05 | (0.02,0.07) | | | 0.00 | (0.00,0.01) |
| Downtown | Quincy | 0.32 | (0.26,0.38) | 0.32 | (0.27,0.38) | 0.32 | (0.27,0.38) |
| Downtown | Russell | 0.00 | (0.00,0.01) | | | | |
| Downtown | Tobin | | | 0.01 | (0.00,0.03) | 0.01 | (0.00,0.03) |
| Downtown | Tynan | | | 0.01 | (0.00,0.03) | 0.01 | (0.00,0.03) |
| Downtown | West Zone ELC | | | 0.01 | (0.00,0.03) | 0.01 | (0.00,0.02) |
| East Boston | Adams | 0.25 | (0.23,0.27) | 0.13 | (0.11,0.16) | 0.12 | (0.10,0.14) |
| East Boston | Blackstone | 0.02 | (0.01,0.03) | 0.01 | (0.00,0.01) | 0.01 | (0.01,0.02) |
| East Boston | Bradley | 0.08 | (0.06,0.10) | 0.15 | (0.13,0.18) | 0.17 | (0.14,0.19) |
| East Boston | East Boston EEC | 0.09 | (0.07,0.11) | 0.25 | (0.22,0.28) | 0.25 | (0.22,0.28) |
| East Boston | Eliot | | | 0.01 | (0.01,0.02) | 0.01 | (0.01,0.02) |
| East Boston | Harvard/Kent | | | 0.01 | (0.00,0.01) | 0.01 | (0.00,0.01) |
| East Boston | Hernandez | 0.16 | (0.14,0.18) | 0.01 | (0.00,0.01) | 0.02 | (0.01,0.03) |
| East Boston | Jackson/Mann | 0.01 | (0.00,0.01) | | | | |
| East Boston | Kennedy Patrick | 0.01 | (0.01,0.02) | 0.11 | (0.09,0.14) | 0.10 | (0.09,0.12) |
| East Boston | O'Donnell | 0.01 | (0.01,0.02) | 0.09 | (0.07,0.11) | 0.08 | (0.06,0.10) |
| East Boston | Otis | 0.34 | (0.32,0.36) | 0.22 | (0.19,0.25) | 0.21 | (0.18,0.24) |
| East Boston | Quincy | 0.00 | (0.00,0.01) | | | | |
| East Boston | Tynan | | | | | 0.01 | (0.00,0.01) |
| Hyde Park | Bates | | | 0.08 | (0.06,0.10) | 0.07 | (0.05,0.09) |
| Hyde Park | Beethoven | | | 0.11 | (0.09,0.13) | 0.10 | (0.08,0.13) |
| Hyde Park | Channing | 0.01 | (0.00,0.01) | 0.09 | (0.07,0.11) | 0.09 | (0.07,0.12) |
| Hyde Park | Chittick | 0.04 | (0.02,0.06) | 0.08 | (0.05,0.10) | 0.07 | (0.05,0.10) |
| Hyde Park | Clap | 0.00 | (0.00,0.01) | | | | |
| Hyde Park | Condon | 0.00 | (0.00,0.01) | | | | |
| Hyde Park | Conley | 0.30 | (0.28,0.31) | 0.09 | (0.07,0.12) | 0.10 | (0.07,0.12) |
| Hyde Park | Curley | 0.00 | (0.00,0.01) | | | | |
| Hyde Park | Ellison/Parks | | | 0.06 | (0.04,0.08) | 0.06 | (0.04,0.08) |
| Hyde Park | Haley | | | 0.04 | (0.03,0.05) | 0.04 | (0.03,0.06) |
| Hyde Park | Hernandez | 0.04 | (0.02,0.06) | 0.04 | (0.02,0.06) | 0.04 | (0.02,0.06) |
| Hyde Park | Kilmer | 0.10 | (0.08,0.12) | 0.05 | (0.03,0.07) | 0.05 | (0.03,0.07) |
| Hyde Park | Mattahunt | 0.01 | (0.00,0.03) | 0.04 | (0.02,0.05) | 0.04 | (0.02,0.06) |
| Hyde Park | Mozart | | | 0.06 | (0.04,0.08) | 0.06 | (0.04,0.08) |
| Hyde Park | Philbrick | 0.16 | (0.14,0.18) | 0.05 | (0.03,0.06) | 0.04 | (0.02,0.06) |
| Hyde Park | Roosevelt | 0.18 | (0.15,0.20) | 0.16 | (0.13,0.18) | 0.16 | (0.13,0.18) |
| Hyde Park | S. Greenwood | 0.00 | (0.00,0.01) | | | | |
| Hyde Park | Sumner | 0.09 | (0.08,0.12) | 0.03 | (0.01,0.04) | 0.03 | (0.01,0.04) |
| Hyde Park | Taylor | | | 0.00 | (0.00,0.01) | 0.00 | (0.00,0.01) |
| Hyde Park | Young Achievers | 0.04 | (0.03,0.06) | 0.03 | (0.02,0.04) | 0.03 | (0.02,0.04) |
| Jamaica Plain | BTU | 0.01 | (0.00,0.02) | 0.07 | (0.05,0.09) | 0.06 | (0.05,0.08) |
| Jamaica Plain | Blackstone | | | 0.01 | (0.00,0.01) | 0.01 | (0.00,0.01) |
| Jamaica Plain | Curley | 0.13 | (0.10,0.17) | 0.25 | (0.22,0.28) | 0.25 | (0.22,0.28) |
| Jamaica Plain | Ellis | 0.01 | (0.00,0.03) | 0.03 | (0.02,0.05) | 0.03 | (0.01,0.04) |
| Jamaica Plain | Ellison/Parks | 0.02 | (0.01,0.04) | 0.00 | (0.00,0.01) | 0.01 | (0.00,0.01) |

Continued on next page

**Table 12 – continued from previous page**

| Neighborhood | School | Naive mean | Naive (95% C.I.) | Logit mean | Logit (95% C.I.) | Mixed Logit mean | Mixed Logit (95% C.I.) |
|---|---|---|---|---|---|---|---|
| Jamaica Plain | Hale | 0.19 | (0.17,0.21) | 0.02 | (0.01,0.03) | 0.02 | (0.01,0.03) |
| Jamaica Plain | Haley | | | 0.01 | (0.00,0.02) | 0.01 | (0.00,0.02) |
| Jamaica Plain | Hernandez | 0.04 | (0.02,0.05) | 0.07 | (0.05,0.09) | 0.09 | (0.07,0.11) |
| Jamaica Plain | Higginson/Lewis | | | 0.01 | (0.00,0.01) | 0.00 | (0.00,0.01) |
| Jamaica Plain | Hurley | 0.07 | (0.05,0.09) | 0.03 | (0.02,0.04) | 0.03 | (0.02,0.05) |
| Jamaica Plain | J.F. Kennedy | 0.08 | (0.06,0.10) | 0.06 | (0.04,0.08) | 0.06 | (0.04,0.08) |
| Jamaica Plain | Jackson/Mann | 0.01 | (0.00,0.02) | 0.03 | (0.02,0.05) | 0.04 | (0.02,0.05) |
| Jamaica Plain | Manning | 0.19 | (0.17,0.21) | 0.08 | (0.06,0.10) | 0.07 | (0.05,0.09) |
| Jamaica Plain | Mason | 0.03 | (0.02,0.05) | | | | |
| Jamaica Plain | Mendell | 0.01 | (0.00,0.02) | 0.06 | (0.04,0.08) | 0.05 | (0.03,0.07) |
| Jamaica Plain | Mission Hill | 0.08 | (0.06,0.10) | 0.12 | (0.09,0.14) | 0.12 | (0.09,0.14) |
| Jamaica Plain | Orchard Gardens | | | 0.02 | (0.01,0.04) | 0.02 | (0.01,0.04) |
| Jamaica Plain | Philbrick | 0.05 | (0.04,0.07) | 0.01 | (0.00,0.02) | 0.01 | (0.00,0.02) |
| Jamaica Plain | Quincy | 0.00 | (0.00,0.01) | | | | |
| Jamaica Plain | S. Greenwood | 0.01 | (0.00,0.02) | | | 0.00 | (0.00,0.01) |
| Jamaica Plain | Sumner | 0.03 | (0.02,0.04) | | | | |
| Jamaica Plain | Tobin | 0.01 | (0.00,0.02) | 0.03 | (0.02,0.05) | 0.03 | (0.02,0.05) |
| Jamaica Plain | Trotter | | | 0.01 | (0.00,0.01) | 0.01 | (0.00,0.01) |
| Jamaica Plain | West Zone ELC | | | 0.05 | (0.04,0.07) | 0.06 | (0.04,0.08) |
| Mattapan | BTU | | | 0.05 | (0.03,0.07) | 0.05 | (0.03,0.07) |
| Mattapan | Channing | 0.01 | (0.00,0.02) | 0.01 | (0.00,0.01) | 0.01 | (0.00,0.01) |
| Mattapan | Chittick | 0.01 | (0.00,0.02) | 0.03 | (0.02,0.05) | 0.03 | (0.01,0.04) |
| Mattapan | Clap | 0.00 | (0.00,0.01) | | | | |
| Mattapan | Condon | 0.00 | (0.00,0.01) | | | | |
| Mattapan | Conley | 0.05 | (0.04,0.07) | 0.01 | (0.00,0.02) | 0.01 | (0.00,0.02) |
| Mattapan | Curley | 0.01 | (0.00,0.02) | | | | |
| Mattapan | Dever | 0.02 | (0.01,0.04) | 0.01 | (0.00,0.02) | 0.01 | (0.00,0.02) |
| Mattapan | Ellison/Parks | 0.07 | (0.05,0.09) | 0.13 | (0.10,0.15) | 0.13 | (0.11,0.16) |
| Mattapan | Haley | 0.01 | (0.00,0.01) | 0.09 | (0.06,0.11) | 0.08 | (0.06,0.10) |
| Mattapan | Henderson | 0.19 | (0.16,0.21) | 0.03 | (0.01,0.04) | 0.03 | (0.02,0.05) |
| Mattapan | Hernandez | 0.03 | (0.02,0.05) | 0.06 | (0.04,0.07) | 0.06 | (0.04,0.07) |
| Mattapan | Holmes | | | 0.01 | (0.01,0.03) | 0.01 | (0.00,0.02) |
| Mattapan | Jackson/Mann | | | 0.01 | (0.00,0.02) | 0.02 | (0.01,0.03) |
| Mattapan | Kenny | 0.00 | (0.00,0.01) | 0.01 | (0.00,0.02) | 0.01 | (0.00,0.02) |
| Mattapan | King | 0.00 | (0.00,0.01) | | | | |
| Mattapan | Lee | 0.01 | (0.01,0.02) | 0.07 | (0.02,0.13) | 0.06 | (0.01,0.13) |
| Mattapan | Mattahunt | 0.02 | (0.00,0.03) | 0.06 | (0.04,0.08) | 0.05 | (0.03,0.08) |
| Mattapan | Murphy | 0.08 | (0.06,0.11) | 0.03 | (0.02,0.05) | 0.04 | (0.02,0.06) |
| Mattapan | Otis | 0.00 | (0.00,0.01) | | | | |
| Mattapan | Philbrick | 0.20 | (0.17,0.22) | 0.04 | (0.02,0.05) | 0.03 | (0.02,0.05) |
| Mattapan | Russell | 0.01 | (0.00,0.01) | | | | |
| Mattapan | S. Greenwood | 0.07 | (0.05,0.09) | 0.06 | (0.04,0.08) | 0.06 | (0.04,0.08) |
| Mattapan | Sumner | 0.05 | (0.03,0.07) | 0.01 | (0.00,0.02) | 0.01 | (0.00,0.02) |
| Mattapan | Taylor | 0.10 | (0.07,0.12) | 0.06 | (0.04,0.08) | 0.06 | (0.04,0.07) |
| Mattapan | Young Achievers | 0.02 | (0.01,0.03) | 0.15 | (0.12,0.18) | 0.15 | (0.12,0.18) |
| North Dorchester | Blackstone | 0.02 | (0.01,0.03) | 0.01 | (0.00,0.02) | 0.01 | (0.00,0.02) |
| North Dorchester | Clap | 0.05 | (0.03,0.08) | 0.18 | (0.15,0.22) | 0.18 | (0.14,0.21) |
| North Dorchester | Condon | 0.03 | (0.01,0.06) | 0.03 | (0.01,0.05) | 0.03 | (0.01,0.05) |
| North Dorchester | Dever | 0.04 | (0.02,0.05) | 0.07 | (0.05,0.10) | 0.07 | (0.05,0.10) |
| North Dorchester | Ellison/Parks | 0.01 | (0.00,0.03) | 0.00 | (0.00,0.01) | 0.00 | (0.00,0.01) |
| North Dorchester | Everett | 0.01 | (0.00,0.02) | 0.11 | (0.09,0.14) | 0.12 | (0.09,0.14) |
| North Dorchester | Hale | 0.03 | (0.02,0.05) | | | | |
| North Dorchester | Harvard/Kent | 0.00 | (0.00,0.01) | | | | |
| North Dorchester | Haynes | 0.14 | (0.12,0.17) | 0.07 | (0.05,0.10) | 0.08 | (0.05,0.11) |
| North Dorchester | Henderson | 0.14 | (0.11,0.17) | 0.03 | (0.02,0.05) | 0.03 | (0.02,0.05) |

Continued on next page

**Table 12 – continued from previous page**

| Neighborhood | School | Naive mean | Naive (95% C.I.) | Logit mean | Logit (95% C.I.) | Mixed Logit mean | Mixed Logit (95% C.I.) |
|---|---|---|---|---|---|---|---|
| North Dorchester | Hernandez | 0.01 | (0.00,0.02) | 0.04 | (0.02,0.05) | 0.04 | (0.02,0.06) |
| North Dorchester | Holland | 0.02 | (0.00,0.03) | 0.04 | (0.02,0.05) | 0.03 | (0.01,0.05) |
| North Dorchester | Hurley | 0.04 | (0.03,0.06) | 0.01 | (0.00,0.02) | 0.01 | (0.00,0.03) |
| North Dorchester | Jackson/Mann | | | 0.02 | (0.01,0.03) | 0.02 | (0.01,0.04) |
| North Dorchester | King | | | 0.03 | (0.02,0.05) | 0.03 | (0.01,0.04) |
| North Dorchester | Lee | 0.01 | (0.00,0.02) | | | | |
| North Dorchester | Mason | 0.27 | (0.25,0.29) | 0.04 | (0.03,0.06) | 0.04 | (0.03,0.06) |
| North Dorchester | Mather | 0.05 | (0.03,0.07) | 0.07 | (0.05,0.10) | 0.08 | (0.06,0.10) |
| North Dorchester | Murphy | 0.06 | (0.03,0.09) | 0.04 | (0.02,0.06) | 0.04 | (0.02,0.07) |
| North Dorchester | Orchard Gardens | | | 0.04 | (0.02,0.06) | 0.04 | (0.02,0.06) |
| North Dorchester | Perry | | | 0.01 | (0.00,0.02) | 0.01 | (0.00,0.02) |
| North Dorchester | Russell | 0.03 | (0.01,0.05) | 0.09 | (0.06,0.12) | 0.09 | (0.06,0.11) |
| North Dorchester | S. Greenwood | 0.01 | (0.00,0.01) | | | | |
| North Dorchester | Tynan | 0.01 | (0.00,0.02) | 0.01 | (0.00,0.01) | 0.01 | (0.00,0.02) |
| North Dorchester | Winthrop | | | 0.03 | (0.02,0.05) | 0.03 | (0.01,0.04) |
| North Dorchester | Young Achievers | 0.01 | (0.00,0.01) | 0.00 | (0.00,0.01) | | |
| Roslindale | BTU | 0.01 | (0.00,0.01) | 0.12 | (0.10,0.14) | 0.12 | (0.10,0.14) |
| Roslindale | Bates | 0.01 | (0.00,0.02) | 0.11 | (0.09,0.13) | 0.11 | (0.09,0.13) |
| Roslindale | Beethoven | 0.01 | (0.00,0.01) | 0.02 | (0.01,0.03) | 0.02 | (0.01,0.03) |
| Roslindale | Channing | | | | | 0.00 | (0.00,0.01) |
| Roslindale | Chittick | | | 0.01 | (0.01,0.02) | 0.01 | (0.00,0.02) |
| Roslindale | Conley | 0.20 | (0.18,0.22) | 0.08 | (0.06,0.10) | 0.08 | (0.06,0.09) |
| Roslindale | Curley | 0.02 | (0.01,0.04) | 0.02 | (0.01,0.03) | 0.02 | (0.01,0.03) |
| Roslindale | Ellis | 0.00 | (0.00,0.01) | | | | |
| Roslindale | Ellison/Parks | | | 0.02 | (0.01,0.04) | 0.03 | (0.01,0.04) |
| Roslindale | Haley | 0.01 | (0.01,0.02) | 0.07 | (0.06,0.09) | 0.08 | (0.06,0.10) |
| Roslindale | Hernandez | 0.03 | (0.02,0.04) | 0.04 | (0.03,0.06) | 0.05 | (0.03,0.06) |
| Roslindale | Kilmer | 0.01 | (0.01,0.02) | 0.02 | (0.01,0.03) | 0.02 | (0.01,0.03) |
| Roslindale | Lyndon | 0.05 | (0.03,0.06) | 0.05 | (0.04,0.07) | 0.05 | (0.04,0.06) |
| Roslindale | Manning | 0.07 | (0.05,0.08) | 0.03 | (0.02,0.04) | 0.03 | (0.02,0.04) |
| Roslindale | Mattahunt | | | 0.03 | (0.02,0.04) | 0.03 | (0.02,0.05) |
| Roslindale | Mission Hill | | | 0.02 | (0.01,0.04) | 0.02 | (0.01,0.03) |
| Roslindale | Mozart | 0.01 | (0.01,0.02) | 0.10 | (0.08,0.12) | 0.10 | (0.09,0.12) |
| Roslindale | Philbrick | 0.21 | (0.20,0.23) | 0.10 | (0.08,0.12) | 0.09 | (0.07,0.11) |
| Roslindale | Sumner | 0.31 | (0.30,0.33) | 0.09 | (0.07,0.11) | 0.09 | (0.07,0.11) |
| Roslindale | Young Achievers | 0.02 | (0.01,0.03) | 0.03 | (0.02,0.04) | 0.03 | (0.02,0.05) |
| Roxbury | BTU | | | 0.01 | (0.00,0.01) | 0.01 | (0.00,0.01) |
| Roxbury | Blackstone | 0.01 | (0.00,0.01) | 0.02 | (0.02,0.04) | 0.02 | (0.01,0.03) |
| Roxbury | Clap | 0.01 | (0.00,0.01) | 0.03 | (0.02,0.04) | 0.03 | (0.02,0.04) |
| Roxbury | Curley | 0.04 | (0.03,0.06) | 0.06 | (0.05,0.08) | 0.06 | (0.04,0.08) |
| Roxbury | Dever | 0.02 | (0.01,0.03) | 0.01 | (0.00,0.01) | 0.01 | (0.00,0.01) |
| Roxbury | Eliot | 0.00 | (0.00,0.01) | | | | |
| Roxbury | Ellis | 0.02 | (0.01,0.03) | 0.05 | (0.03,0.06) | 0.04 | (0.03,0.06) |
| Roxbury | Ellison/Parks | 0.01 | (0.01,0.02) | 0.01 | (0.00,0.01) | 0.01 | (0.00,0.01) |
| Roxbury | Everett | | | 0.03 | (0.02,0.04) | 0.03 | (0.02,0.04) |
| Roxbury | Hale | 0.21 | (0.20,0.23) | 0.03 | (0.02,0.05) | 0.03 | (0.02,0.04) |
| Roxbury | Haley | 0.01 | (0.00,0.01) | 0.01 | (0.00,0.01) | 0.01 | (0.00,0.01) |
| Roxbury | Haynes | 0.04 | (0.03,0.06) | 0.07 | (0.05,0.09) | 0.07 | (0.06,0.09) |
| Roxbury | Henderson | 0.04 | (0.03,0.05) | 0.01 | (0.00,0.01) | 0.01 | (0.00,0.01) |
| Roxbury | Hernandez | 0.02 | (0.01,0.04) | 0.09 | (0.07,0.11) | 0.11 | (0.09,0.13) |
| Roxbury | Higginson/Lewis | | | 0.03 | (0.02,0.04) | 0.02 | (0.01,0.03) |
| Roxbury | Holland | 0.01 | (0.00,0.01) | 0.03 | (0.02,0.04) | 0.03 | (0.02,0.04) |
| Roxbury | Holmes | | | 0.01 | (0.01,0.02) | 0.01 | (0.00,0.02) |
| Roxbury | Hurley | 0.06 | (0.05,0.07) | 0.03 | (0.02,0.04) | 0.03 | (0.02,0.04) |
| Roxbury | J.F. Kennedy | 0.05 | (0.04,0.07) | 0.03 | (0.02,0.04) | 0.03 | (0.02,0.04) |

Continued on next page

**Table 12 – continued from previous page**

| Neighborhood | School | Naive mean | Naive (95% C.I.) | Logit mean | Logit (95% C.I.) | Mixed Logit mean | Mixed Logit (95% C.I.) |
|---|---|---|---|---|---|---|---|
| Roxbury | Jackson/Mann | 0.01 | (0.00,0.01) | 0.03 | (0.02,0.04) | 0.03 | (0.02,0.05) |
| Roxbury | King | 0.01 | (0.00,0.01) | 0.04 | (0.02,0.05) | 0.03 | (0.02,0.04) |
| Roxbury | Lee | | | 0.01 | (0.00,0.02) | 0.01 | (0.00,0.02) |
| Roxbury | Manning | 0.01 | (0.01,0.02) | | | | |
| Roxbury | Mason | 0.19 | (0.17,0.21) | 0.03 | (0.02,0.05) | 0.04 | (0.02,0.05) |
| Roxbury | Mather | 0.01 | (0.01,0.02) | 0.02 | (0.01,0.03) | 0.02 | (0.01,0.03) |
| Roxbury | Mendell | | | 0.03 | (0.02,0.04) | 0.02 | (0.01,0.03) |
| Roxbury | Mission Hill | 0.01 | (0.01,0.01) | 0.03 | (0.02,0.04) | 0.03 | (0.02,0.04) |
| Roxbury | Murphy | 0.02 | (0.01,0.04) | 0.01 | (0.00,0.01) | 0.01 | (0.00,0.02) |
| Roxbury | Orchard Gardens | 0.02 | (0.01,0.03) | 0.06 | (0.04,0.07) | 0.05 | (0.04,0.07) |
| Roxbury | Quincy | 0.01 | (0.00,0.01) | | | | |
| Roxbury | Russell | 0.02 | (0.01,0.03) | 0.03 | (0.02,0.04) | 0.03 | (0.02,0.04) |
| Roxbury | S. Greenwood | 0.05 | (0.04,0.06) | 0.03 | (0.02,0.04) | 0.03 | (0.02,0.04) |
| Roxbury | Tobin | | | 0.02 | (0.01,0.03) | 0.02 | (0.01,0.03) |
| Roxbury | Trotter | 0.01 | (0.01,0.02) | 0.04 | (0.03,0.05) | 0.04 | (0.03,0.06) |
| Roxbury | West Zone ELC | | | 0.02 | (0.01,0.03) | 0.02 | (0.01,0.03) |
| Roxbury | Winthrop | 0.01 | (0.00,0.01) | 0.03 | (0.02,0.04) | 0.03 | (0.02,0.04) |
| Roxbury | Young Achievers | 0.01 | (0.00,0.01) | 0.00 | (0.00,0.01) | | |
| South Boston | Blackstone | 0.03 | (0.01,0.06) | 0.05 | (0.02,0.08) | 0.05 | (0.03,0.09) |
| South Boston | Chittick | 0.01 | (0.00,0.03) | | | | |
| South Boston | Clap | 0.06 | (0.03,0.10) | 0.11 | (0.07,0.14) | 0.11 | (0.06,0.15) |
| South Boston | Condon | 0.07 | (0.02,0.12) | 0.18 | (0.13,0.23) | 0.17 | (0.13,0.22) |
| South Boston | Dever | 0.04 | (0.02,0.07) | 0.06 | (0.04,0.09) | 0.06 | (0.03,0.09) |
| South Boston | East Boston EEC | | | | | 0.00 | (0.00,0.01) |
| South Boston | Eliot | 0.01 | (0.00,0.03) | 0.02 | (0.00,0.04) | 0.02 | (0.00,0.05) |
| South Boston | Everett | | | 0.02 | (0.00,0.04) | 0.01 | (0.00,0.03) |
| South Boston | Haynes | 0.06 | (0.03,0.09) | 0.02 | (0.00,0.03) | 0.02 | (0.00,0.04) |
| South Boston | Hernandez | | | 0.02 | (0.01,0.04) | 0.02 | (0.01,0.04) |
| South Boston | Hurley | 0.06 | (0.04,0.10) | 0.03 | (0.01,0.05) | 0.03 | (0.01,0.05) |
| South Boston | Jackson/Mann | | | 0.01 | (0.00,0.03) | 0.01 | (0.00,0.03) |
| South Boston | Lee | 0.01 | (0.00,0.03) | | | | |
| South Boston | Manning | 0.00 | (0.00,0.02) | | | | |
| South Boston | Mason | 0.15 | (0.12,0.19) | 0.02 | (0.01,0.04) | 0.02 | (0.00,0.04) |
| South Boston | Mather | | | 0.01 | (0.00,0.01) | 0.01 | (0.00,0.02) |
| South Boston | Murphy | 0.02 | (0.00,0.05) | 0.01 | (0.00,0.03) | 0.01 | (0.00,0.03) |
| South Boston | Orchard Gardens | | | 0.02 | (0.01,0.04) | 0.03 | (0.01,0.05) |
| South Boston | Perry | 0.02 | (0.00,0.04) | 0.12 | (0.08,0.15) | 0.12 | (0.08,0.15) |
| South Boston | Quincy | 0.39 | (0.32,0.46) | 0.18 | (0.12,0.23) | 0.18 | (0.12,0.24) |
| South Boston | Russell | 0.05 | (0.03,0.08) | 0.05 | (0.03,0.08) | 0.04 | (0.02,0.07) |
| South Boston | Tynan | 0.00 | (0.00,0.01) | 0.07 | (0.04,0.10) | 0.07 | (0.04,0.10) |
| South Boston | Winthrop | | | 0.00 | (0.00,0.01) | 0.00 | (0.00,0.01) |
| South Dorchester | Clap | 0.01 | (0.00,0.02) | 0.01 | (0.00,0.01) | 0.01 | (0.00,0.01) |
| South Dorchester | Condon | 0.02 | (0.01,0.03) | 0.01 | (0.00,0.01) | 0.01 | (0.00,0.01) |
| South Dorchester | Ellison/Parks | 0.11 | (0.09,0.12) | 0.04 | (0.03,0.06) | 0.05 | (0.04,0.07) |
| South Dorchester | Everett | | | 0.03 | (0.02,0.04) | 0.03 | (0.02,0.04) |
| South Dorchester | Haynes | | | 0.02 | (0.01,0.03) | 0.02 | (0.01,0.03) |
| South Dorchester | Henderson | 0.24 | (0.22,0.26) | 0.10 | (0.08,0.12) | 0.10 | (0.08,0.12) |
| South Dorchester | Hernandez | 0.02 | (0.01,0.03) | 0.04 | (0.03,0.06) | 0.05 | (0.03,0.06) |
| South Dorchester | Holland | 0.04 | (0.03,0.06) | 0.05 | (0.04,0.07) | 0.05 | (0.04,0.07) |
| South Dorchester | Holmes | | | 0.03 | (0.02,0.04) | 0.03 | (0.02,0.04) |
| South Dorchester | Jackson/Mann | | | 0.01 | (0.01,0.02) | 0.02 | (0.01,0.03) |
| South Dorchester | Kenny | 0.01 | (0.00,0.01) | 0.04 | (0.03,0.05) | 0.04 | (0.03,0.05) |
| South Dorchester | King | | | 0.02 | (0.01,0.03) | 0.01 | (0.01,0.02) |
| South Dorchester | Lee | 0.01 | (0.00,0.02) | 0.05 | (0.01,0.10) | 0.05 | (0.01,0.09) |
| South Dorchester | Mason | 0.01 | (0.00,0.01) | | | | |

Continued on next page

**Table 12 – continued from previous page**

| Neighborhood | School | Naive mean | Naive (95% C.I.) | Logit mean | Logit (95% C.I.) | Mixed Logit mean | Mixed Logit (95% C.I.) |
|---|---|---|---|---|---|---|---|
| South Dorchester | Mather | 0.05 | (0.04,0.07) | 0.07 | (0.06,0.09) | 0.07 | (0.05,0.08) |
| South Dorchester | Mattahunt | 0.01 | (0.00,0.02) | | | | |
| South Dorchester | Murphy | 0.38 | (0.35,0.40) | 0.30 | (0.27,0.33) | 0.30 | (0.28,0.34) |
| South Dorchester | Russell | 0.01 | (0.00,0.01) | 0.01 | (0.01,0.02) | 0.01 | (0.01,0.02) |
| South Dorchester | S. Greenwood | 0.03 | (0.02,0.04) | 0.05 | (0.04,0.06) | 0.05 | (0.04,0.06) |
| South Dorchester | Taylor | 0.01 | (0.01,0.02) | 0.02 | (0.01,0.03) | 0.02 | (0.01,0.03) |
| South Dorchester | Tynan | 0.01 | (0.00,0.01) | | | | |
| South Dorchester | Young Achievers | 0.00 | (0.00,0.01) | 0.02 | (0.01,0.02) | 0.02 | (0.01,0.02) |
| South End | Baldwin | | | 0.00 | (0.00,0.01) | 0.00 | (0.00,0.01) |
| South End | Blackstone | 0.05 | (0.02,0.08) | 0.16 | (0.12,0.20) | 0.15 | (0.12,0.20) |
| South End | Clap | | | 0.01 | (0.00,0.02) | 0.01 | (0.00,0.03) |
| South End | Condon | 0.01 | (0.00,0.02) | 0.05 | (0.03,0.08) | 0.05 | (0.03,0.08) |
| South End | Curley | 0.02 | (0.01,0.03) | 0.01 | (0.00,0.02) | 0.01 | (0.00,0.02) |
| South End | Dever | 0.02 | (0.01,0.04) | 0.00 | (0.00,0.01) | 0.01 | (0.00,0.01) |
| South End | Edison | 0.03 | (0.02,0.05) | 0.00 | (0.00,0.01) | 0.00 | (0.00,0.01) |
| South End | Eliot | 0.02 | (0.01,0.04) | 0.03 | (0.01,0.05) | 0.03 | (0.01,0.05) |
| South End | Ellis | 0.01 | (0.00,0.02) | | | | |
| South End | Gardner | 0.01 | (0.00,0.02) | 0.00 | (0.00,0.01) | 0.00 | (0.00,0.01) |
| South End | Hale | 0.03 | (0.02,0.06) | 0.02 | (0.00,0.03) | 0.01 | (0.00,0.03) |
| South End | Haynes | 0.06 | (0.04,0.09) | 0.01 | (0.00,0.03) | 0.02 | (0.01,0.04) |
| South End | Hernandez | | | 0.03 | (0.02,0.05) | 0.03 | (0.01,0.05) |
| South End | Higginson/Lewis | 0.00 | (0.00,0.01) | 0.01 | (0.00,0.02) | 0.01 | (0.00,0.02) |
| South End | Hurley | 0.24 | (0.21,0.27) | 0.14 | (0.11,0.18) | 0.15 | (0.11,0.18) |
| South End | Jackson/Mann | 0.02 | (0.00,0.04) | 0.02 | (0.01,0.04) | 0.02 | (0.01,0.04) |
| South End | Mason | 0.06 | (0.04,0.08) | 0.03 | (0.01,0.05) | 0.02 | (0.01,0.04) |
| South End | Orchard Gardens | 0.01 | (0.00,0.02) | 0.08 | (0.05,0.10) | 0.07 | (0.04,0.10) |
| South End | Quincy | 0.38 | (0.32,0.43) | 0.33 | (0.27,0.38) | 0.33 | (0.27,0.39) |
| South End | Russell | 0.02 | (0.01,0.04) | 0.00 | (0.00,0.01) | 0.01 | (0.00,0.01) |
| South End | Sumner | 0.00 | (0.00,0.01) | | | | |
| South End | Tobin | | | 0.02 | (0.01,0.04) | 0.02 | (0.01,0.04) |
| South End | Tynan | | | 0.00 | (0.00,0.01) | 0.01 | (0.00,0.01) |
| South End | West Zone ELC | | | 0.01 | (0.00,0.02) | 0.01 | (0.00,0.03) |
| South End | Winthrop | 0.00 | (0.00,0.01) | 0.01 | (0.00,0.02) | 0.01 | (0.00,0.02) |
| West Roxbury | BTU | 0.01 | (0.00,0.01) | 0.01 | (0.01,0.02) | 0.01 | (0.00,0.02) |
| West Roxbury | Baldwin | | | 0.00 | (0.00,0.01) | 0.01 | (0.00,0.01) |
| West Roxbury | Bates | 0.01 | (0.01,0.02) | 0.07 | (0.05,0.09) | 0.07 | (0.05,0.09) |
| West Roxbury | Beethoven | 0.03 | (0.02,0.04) | 0.18 | (0.16,0.21) | 0.19 | (0.17,0.21) |
| West Roxbury | Channing | 0.01 | (0.00,0.01) | 0.04 | (0.03,0.05) | 0.04 | (0.03,0.06) |
| West Roxbury | Conley | 0.12 | (0.10,0.14) | 0.03 | (0.01,0.04) | 0.02 | (0.01,0.04) |
| West Roxbury | Curley | 0.00 | (0.00,0.01) | | | | |
| West Roxbury | Ellison/Parks | | | 0.01 | (0.00,0.02) | 0.01 | (0.00,0.02) |
| West Roxbury | Hernandez | 0.02 | (0.01,0.03) | 0.02 | (0.01,0.03) | 0.02 | (0.01,0.03) |
| West Roxbury | J.F. Kennedy | 0.00 | (0.00,0.01) | | | | |
| West Roxbury | Kilmer | 0.28 | (0.26,0.29) | 0.23 | (0.21,0.25) | 0.23 | (0.21,0.25) |
| West Roxbury | Lyndon | 0.27 | (0.25,0.28) | 0.22 | (0.20,0.23) | 0.21 | (0.19,0.24) |
| West Roxbury | Manning | 0.04 | (0.02,0.05) | 0.03 | (0.02,0.04) | 0.03 | (0.02,0.04) |
| West Roxbury | Mozart | 0.01 | (0.00,0.01) | 0.10 | (0.08,0.12) | 0.10 | (0.07,0.12) |
| West Roxbury | Philbrick | 0.01 | (0.00,0.01) | | | | |
| West Roxbury | Roosevelt | 0.04 | (0.03,0.05) | 0.02 | (0.01,0.03) | 0.03 | (0.01,0.04) |
| West Roxbury | Sumner | 0.14 | (0.12,0.16) | 0.02 | (0.01,0.03) | 0.02 | (0.01,0.04) |
| West Roxbury | Taylor | 0.00 | (0.00,0.01) | | | | |
